# Supplementary material for: Context-Aware Sentence/Passage Term Importance Estimation For First Stage Retrieval
Source: arXiv:1910.10687 source file (2019-11-26)
Supplement: Supplementary file 1 [file appendix.tex]

query: what constitutional clause prohibits a state from drawing unreasonable distinctions between its own residents and those of persons living in other states

\begin{CJK*}{UTF8}{gbsn}
{\setlength{\fboxsep}{0pt}\colorbox{white!0}{\parbox{0.9\textwidth}{
\colorbox{red!0}{\strut Chapter} \colorbox{red!0}{\strut 4} \colorbox{red!6}{\strut Government} \colorbox{red!0}{\strut Quiz} \colorbox{red!0}{\strut .} \colorbox{red!0}{\strut 47} \colorbox{red!0}{\strut terms} \colorbox{red!0}{\strut hannahmcclary8Chapter} \colorbox{red!0}{\strut 4} \colorbox{red!6}{\strut Government} \colorbox{red!0}{\strut QuizLearn} \colorbox{red!0}{\strut Flashcards} \colorbox{red!0}{\strut Write} \colorbox{red!0}{\strut Spell} \colorbox{red!0}{\strut Test} \colorbox{red!0}{\strut MatchGravityAdvertisementUpgrade} \colorbox{red!0}{\strut to} \colorbox{red!0}{\strut remove} \colorbox{red!0}{\strut adsLike} \colorbox{red!0}{\strut this} \colorbox{red!0}{\strut study} \colorbox{red!0}{\strut set} \colorbox{red!0}{\strut ?} \colorbox{red!0}{\strut Create} \colorbox{red!0}{\strut a} \colorbox{red!0}{\strut free} \colorbox{red!0}{\strut account} \colorbox{red!0}{\strut to} \colorbox{red!0}{\strut save} \colorbox{red!0}{\strut it.Create} \colorbox{red!0}{\strut a} \colorbox{red!0}{\strut free} \colorbox{red!0}{\strut accountMaybe} \colorbox{red!0}{\strut laterSortThe} \colorbox{red!0}{\strut 10th} \colorbox{red!0}{\strut Amendment} \colorbox{red!0}{\strut provides} \colorbox{red!0}{\strut for} \colorbox{red!0}{\strut .} \colorbox{red!0}{\strut between} \colorbox{red!0}{\strut the} \colorbox{red!1}{\strut National} \colorbox{red!6}{\strut Government} \colorbox{red!0}{\strut and} \colorbox{red!0}{\strut the} \colorbox{red!1}{\strut States} \colorbox{red!0}{\strut division} \colorbox{red!0}{\strut of} \colorbox{red!0}{\strut powersFederalism} \colorbox{red!0}{\strut is} \colorbox{red!0}{\strut a} \colorbox{red!0}{\strut system} \colorbox{red!0}{\strut of} \colorbox{red!6}{\strut government} \colorbox{red!0}{\strut in} \colorbox{red!1}{\strut which} \colorbox{red!0}{\strut a} \colorbox{red!0}{\strut written} \colorbox{red!1}{\strut constitution} \colorbox{red!0}{\strut does} \colorbox{red!4}{\strut what} \colorbox{red!0}{\strut ?} \colorbox{red!0}{\strut divides} \colorbox{red!0}{\strut the} \colorbox{red!6}{\strut powers} \colorbox{red!0}{\strut of} \colorbox{red!6}{\strut government} \colorbox{red!0}{\strut between} \colorbox{red!0}{\strut a} \colorbox{red!1}{\strut national} \colorbox{red!6}{\strut government} \colorbox{red!0}{\strut and} \colorbox{red!0}{\strut several} \colorbox{red!0}{\strut regional} \colorbox{red!0}{\strut governmentsWhat} \colorbox{red!6}{\strut powers} \colorbox{red!3}{\strut given} \colorbox{red!0}{\strut to} \colorbox{red!0}{\strut the} \colorbox{red!1}{\strut National} \colorbox{red!6}{\strut Government} \colorbox{red!0}{\strut are} \colorbox{red!0}{\strut spelled} \colorbox{red!0}{\strut out} \colorbox{red!0}{\strut in} \colorbox{red!0}{\strut the} \colorbox{red!1}{\strut Constitution} \colorbox{red!0}{\strut ?} \colorbox{red!0}{\strut expressed} \colorbox{red!0}{\strut powersWhich} \colorbox{red!0}{\strut was} \colorbox{red!0}{\strut NOT} \colorbox{red!0}{\strut a} \colorbox{red!0}{\strut concern} \colorbox{red!0}{\strut of} \colorbox{red!0}{\strut the} \colorbox{red!0}{\strut Framers} \colorbox{red!0}{\strut about} \colorbox{red!0}{\strut limited} \colorbox{red!6}{\strut government} \colorbox{red!0}{\strut ?} \colorbox{red!0}{\strut A} \colorbox{red!0}{\strut strong} \colorbox{red!0}{\strut central} \colorbox{red!6}{\strut government} \colorbox{red!0}{\strut helps} \colorbox{red!0}{\strut ensure} \colorbox{red!0}{\strut personal} \colorbox{red!0}{\strut freedom.The} \colorbox{red!0}{\strut three} \colorbox{red!0}{\strut types} \colorbox{red!0}{\strut of} \colorbox{red!0}{\strut .} \colorbox{red!6}{\strut powers} \colorbox{red!0}{\strut are} \colorbox{red!0}{\strut expressed} \colorbox{red!0}{\strut ,} \colorbox{red!0}{\strut implied} \colorbox{red!0}{\strut ,} \colorbox{red!0}{\strut and} \colorbox{red!0}{\strut inherent} \colorbox{red!0}{\strut .} \colorbox{red!0}{\strut delegatedWhat} \colorbox{red!6}{\strut powers} \colorbox{red!0}{\strut can} \colorbox{red!0}{\strut be} \colorbox{red!0}{\strut exercised} \colorbox{red!0}{\strut only} \colorbox{red!0}{\strut by} \colorbox{red!0}{\strut the} \colorbox{red!1}{\strut National} \colorbox{red!6}{\strut Government} \colorbox{red!0}{\strut ?} \colorbox{red!0}{\strut exclusive} \colorbox{red!0}{\strut powersWhat} \colorbox{red!6}{\strut powers} \colorbox{red!0}{\strut are} \colorbox{red!3}{\strut given} \colorbox{red!0}{\strut to} \colorbox{red!0}{\strut the} \colorbox{red!1}{\strut National} \colorbox{red!6}{\strut Government} \colorbox{red!0}{\strut because} \colorbox{red!0}{\strut it} \colorbox{red!0}{\strut is} \colorbox{red!0}{\strut the} \colorbox{red!1}{\strut national} \colorbox{red!6}{\strut government} \colorbox{red!0}{\strut of} \colorbox{red!0}{\strut a} \colorbox{red!0}{\strut sovereign} \colorbox{red!1}{\strut state} \colorbox{red!0}{\strut in} \colorbox{red!0}{\strut the} \colorbox{red!0}{\strut world} \colorbox{red!0}{\strut community} \colorbox{red!0}{\strut ?} \colorbox{red!0}{\strut inherent} \colorbox{red!0}{\strut powersWhat} \colorbox{red!6}{\strut powers} \colorbox{red!3}{\strut given} \colorbox{red!0}{\strut to} \colorbox{red!0}{\strut the} \colorbox{red!1}{\strut National} \colorbox{red!6}{\strut Government} \colorbox{red!0}{\strut are} \colorbox{red!0}{\strut reasonably} \colorbox{red!0}{\strut suggested} \colorbox{red!0}{\strut by} \colorbox{red!0}{\strut the} \colorbox{red!1}{\strut Constitution} \colorbox{red!0}{\strut ?} \colorbox{red!0}{\strut implied} \colorbox{red!0}{\strut powersWhat} \colorbox{red!6}{\strut powers} \colorbox{red!0}{\strut can} \colorbox{red!0}{\strut be} \colorbox{red!0}{\strut exercised} \colorbox{red!0}{\strut by} \colorbox{red!0}{\strut both} \colorbox{red!0}{\strut the} \colorbox{red!1}{\strut National} \colorbox{red!6}{\strut Government} \colorbox{red!0}{\strut and} \colorbox{red!0}{\strut the} \colorbox{red!1}{\strut States} \colorbox{red!0}{\strut ?} \colorbox{red!0}{\strut concurrent} \colorbox{red!0}{\strut powersWhat} \colorbox{red!0}{\strut are} \colorbox{red!0}{\strut the} \colorbox{red!6}{\strut powers} \colorbox{red!0}{\strut that} \colorbox{red!0}{\strut the} \colorbox{red!1}{\strut Constitution} \colorbox{red!0}{\strut does} \colorbox{red!0}{\strut not} \colorbox{red!1}{\strut grant} \colorbox{red!0}{\strut to} \colorbox{red!0}{\strut the} \colorbox{red!1}{\strut National} \colorbox{red!6}{\strut Government} \colorbox{red!0}{\strut and} \colorbox{red!0}{\strut does} \colorbox{red!0}{\strut not} \colorbox{red!0}{\strut deny} \colorbox{red!0}{\strut to} \colorbox{red!0}{\strut the} \colorbox{red!1}{\strut States} \colorbox{red!0}{\strut ?} \colorbox{red!0}{\strut reserved} \colorbox{red!0}{\strut powersWhich} \colorbox{red!0}{\strut of} \colorbox{red!0}{\strut the} \colorbox{red!0}{\strut following} \colorbox{red!0}{\strut would} \colorbox{red!0}{\strut NOT} \colorbox{red!0}{\strut be} \colorbox{red!0}{\strut an} \colorbox{red!0}{\strut example} \colorbox{red!0}{\strut of} \colorbox{red!0}{\strut .} \colorbox{red!0}{\strut .} \colorbox{red!0}{\strut domestic} \colorbox{red!0}{\strut Violence} \colorbox{red!0}{\strut .} \colorbox{red!0}{\strut .} \colorbox{red!0}{\strut as} \colorbox{red!0}{\strut intended} \colorbox{red!0}{\strut by} \colorbox{red!0}{\strut the} \colorbox{red!1}{\strut Constitution} \colorbox{red!0}{\strut ?} \colorbox{red!0}{\strut invasionWhat} \colorbox{red!0}{\strut are} \colorbox{red!0}{\strut the} \colorbox{red!0}{\strut grants} \colorbox{red!0}{\strut of} \colorbox{red!0}{\strut federal} \colorbox{red!0}{\strut money} \colorbox{red!0}{\strut or} \colorbox{red!0}{\strut other} \colorbox{red!0}{\strut resources} \colorbox{red!0}{\strut to} \colorbox{red!0}{\strut the} \colorbox{red!1}{\strut States} \colorbox{red!0}{\strut andor} \colorbox{red!0}{\strut their} \colorbox{red!0}{\strut cities} \colorbox{red!0}{\strut ,} \colorbox{red!0}{\strut counties} \colorbox{red!0}{\strut ,} \colorbox{red!0}{\strut or} \colorbox{red!0}{\strut other} \colorbox{red!0}{\strut local} \colorbox{red!0}{\strut units} \colorbox{red!0}{\strut called} \colorbox{red!0}{\strut ?} \colorbox{red!0}{\strut grants-in-aid} \colorbox{red!0}{\strut programsWhat} \colorbox{red!0}{\strut are} \colorbox{red!0}{\strut grants} \colorbox{red!0}{\strut intended} \colorbox{red!0}{\strut for} \colorbox{red!0}{\strut a} \colorbox{red!0}{\strut broadly} \colorbox{red!0}{\strut defined} \colorbox{red!0}{\strut purpose} \colorbox{red!0}{\strut such} \colorbox{red!0}{\strut as} \colorbox{red!0}{\strut health} \colorbox{red!0}{\strut care} \colorbox{red!0}{\strut ,} \colorbox{red!0}{\strut social} \colorbox{red!0}{\strut services} \colorbox{red!0}{\strut ,} \colorbox{red!0}{\strut or} \colorbox{red!0}{\strut welfare} \colorbox{red!0}{\strut ?} \colorbox{red!0}{\strut block} \colorbox{red!0}{\strut grantsWhat} \colorbox{red!0}{\strut is} \colorbox{red!0}{\strut the} \colorbox{red!0}{\strut one} \colorbox{red!0}{\strut restriction} \colorbox{red!0}{\strut that} \colorbox{red!0}{\strut the} \colorbox{red!1}{\strut Constitution} \colorbox{red!0}{\strut places} \colorbox{red!0}{\strut on} \colorbox{red!0}{\strut the} \colorbox{red!1}{\strut National} \colorbox{red!6}{\strut Government} \colorbox{red!0}{\strut in} \colorbox{red!0}{\strut the} \colorbox{red!0}{\strut admission} \colorbox{red!0}{\strut of} \colorbox{red!0}{\strut new} \colorbox{red!1}{\strut states} \colorbox{red!0}{\strut into} 
}}}
\end{CJK*}

\begin{CJK*}{UTF8}{gbsn}
{\setlength{\fboxsep}{0pt}\colorbox{white!0}{\parbox{0.9\textwidth}{
\colorbox{red!0}{\strut List} \colorbox{red!0}{\strut of} \colorbox{red!5}{\strut clauses} \colorbox{red!0}{\strut of} \colorbox{red!0}{\strut the} \colorbox{red!1}{\strut United} \colorbox{red!1}{\strut States} \colorbox{red!5}{\strut Constitution} \colorbox{red!0}{\strut .} \colorbox{red!0}{\strut From} \colorbox{red!0}{\strut Wikipedia} \colorbox{red!0}{\strut ,} \colorbox{red!0}{\strut the} \colorbox{red!0}{\strut free} \colorbox{red!0}{\strut encyclopedianavigation} \colorbox{red!0}{\strut searchThis} \colorbox{red!0}{\strut article} \colorbox{red!0}{\strut needs} \colorbox{red!0}{\strut additional} \colorbox{red!0}{\strut citations} \colorbox{red!0}{\strut for} \colorbox{red!0}{\strut verification} \colorbox{red!0}{\strut .} \colorbox{red!0}{\strut Please} \colorbox{red!0}{\strut help} \colorbox{red!0}{\strut improve} \colorbox{red!0}{\strut this} \colorbox{red!0}{\strut article} \colorbox{red!0}{\strut by} \colorbox{red!0}{\strut adding} \colorbox{red!0}{\strut citations} \colorbox{red!0}{\strut to} \colorbox{red!0}{\strut reliable} \colorbox{red!0}{\strut sources} \colorbox{red!0}{\strut .} \colorbox{red!0}{\strut Unsourced} \colorbox{red!0}{\strut material} \colorbox{red!0}{\strut may} \colorbox{red!0}{\strut be} \colorbox{red!0}{\strut challenged} \colorbox{red!0}{\strut and} \colorbox{red!0}{\strut removed} \colorbox{red!0}{\strut .} \colorbox{red!0}{\strut .} \colorbox{red!0}{\strut February} \colorbox{red!0}{\strut 2017} \colorbox{red!0}{\strut .} \colorbox{red!0}{\strut .} \colorbox{red!0}{\strut Learn} \colorbox{red!1}{\strut how} \colorbox{red!0}{\strut and} \colorbox{red!0}{\strut when} \colorbox{red!0}{\strut to} \colorbox{red!0}{\strut remove} \colorbox{red!0}{\strut this} \colorbox{red!0}{\strut template} \colorbox{red!0}{\strut message} \colorbox{red!0}{\strut .} \colorbox{red!0}{\strut The} \colorbox{red!1}{\strut United} \colorbox{red!1}{\strut States} \colorbox{red!5}{\strut Constitution} \colorbox{red!0}{\strut and} \colorbox{red!0}{\strut its} \colorbox{red!2}{\strut amendments} \colorbox{red!0}{\strut comprise} \colorbox{red!0}{\strut hundreds} \colorbox{red!0}{\strut of} \colorbox{red!5}{\strut clauses} \colorbox{red!0}{\strut which} \colorbox{red!0}{\strut outline} \colorbox{red!0}{\strut the} \colorbox{red!0}{\strut functioning} \colorbox{red!0}{\strut of} \colorbox{red!0}{\strut the} \colorbox{red!1}{\strut United} \colorbox{red!1}{\strut States} \colorbox{red!1}{\strut Federal} \colorbox{red!1}{\strut Government} \colorbox{red!0}{\strut ,} \colorbox{red!0}{\strut the} \colorbox{red!0}{\strut political} \colorbox{red!0}{\strut relationship} \colorbox{red!0}{\strut between} \colorbox{red!0}{\strut the} \colorbox{red!1}{\strut states} \colorbox{red!0}{\strut and} \colorbox{red!0}{\strut the} \colorbox{red!0}{\strut national} \colorbox{red!1}{\strut government} \colorbox{red!0}{\strut ,} \colorbox{red!0}{\strut and} \colorbox{red!0}{\strut affect} \colorbox{red!1}{\strut how} \colorbox{red!0}{\strut the} \colorbox{red!1}{\strut United} \colorbox{red!1}{\strut States} \colorbox{red!1}{\strut federal} \colorbox{red!0}{\strut court} \colorbox{red!0}{\strut system} \colorbox{red!0}{\strut interprets} \colorbox{red!0}{\strut the} \colorbox{red!1}{\strut law} \colorbox{red!0}{\strut .} \colorbox{red!0}{\strut When} \colorbox{red!0}{\strut a} \colorbox{red!0}{\strut particular} \colorbox{red!5}{\strut clause} \colorbox{red!0}{\strut becomes} \colorbox{red!0}{\strut an} \colorbox{red!0}{\strut important} \colorbox{red!0}{\strut or} \colorbox{red!0}{\strut contentious} \colorbox{red!0}{\strut issue} \colorbox{red!0}{\strut of} \colorbox{red!1}{\strut law} \colorbox{red!0}{\strut ,} \colorbox{red!0}{\strut it} \colorbox{red!0}{\strut is} \colorbox{red!0}{\strut given} \colorbox{red!0}{\strut a} \colorbox{red!0}{\strut name} \colorbox{red!0}{\strut for} \colorbox{red!0}{\strut ease} \colorbox{red!0}{\strut of} \colorbox{red!0}{\strut reference.Contents} \colorbox{red!0}{\strut .} \colorbox{red!0}{\strut hide} \colorbox{red!0}{\strut .} \colorbox{red!0}{\strut 1} \colorbox{red!5}{\strut Clauses} \colorbox{red!0}{\strut within} \colorbox{red!0}{\strut the} \colorbox{red!0}{\strut Articles2} \colorbox{red!5}{\strut Clauses} \colorbox{red!0}{\strut within} \colorbox{red!0}{\strut the} \colorbox{red!0}{\strut Amendments2.1} \colorbox{red!0}{\strut First} \colorbox{red!0}{\strut Amendment2.2} \colorbox{red!0}{\strut Fourth} \colorbox{red!0}{\strut Amendment2.3} \colorbox{red!0}{\strut Fifth} \colorbox{red!0}{\strut Amendment2.4} \colorbox{red!0}{\strut Sixth} \colorbox{red!0}{\strut Amendment2.5} \colorbox{red!0}{\strut Eighth} \colorbox{red!0}{\strut Amendment2.6} \colorbox{red!0}{\strut Fourteenth} \colorbox{red!0}{\strut Amendment2.7} \colorbox{red!0}{\strut Recurring} \colorbox{red!0}{\strut Clauses3} \colorbox{red!0}{\strut References4} \colorbox{red!0}{\strut NotesClauses} \colorbox{red!0}{\strut within} \colorbox{red!0}{\strut the} \colorbox{red!0}{\strut Articles} \colorbox{red!0}{\strut .} \colorbox{red!0}{\strut edit} \colorbox{red!0}{\strut .} \colorbox{red!5}{\strut Clause} \colorbox{red!0}{\strut Name} \colorbox{red!0}{\strut Article} \colorbox{red!0}{\strut Section} \colorbox{red!0}{\strut Clause1808} \colorbox{red!5}{\strut Clause} \colorbox{red!0}{\strut .} \colorbox{red!0}{\strut 1} \colorbox{red!0}{\strut .} \colorbox{red!0}{\strut I} \colorbox{red!0}{\strut 9} \colorbox{red!0}{\strut 1Admissions} \colorbox{red!5}{\strut Clause} \colorbox{red!0}{\strut IV} \colorbox{red!0}{\strut 3} \colorbox{red!0}{\strut 1Advice} \colorbox{red!0}{\strut and} \colorbox{red!0}{\strut Consent} \colorbox{red!5}{\strut Clause} \colorbox{red!0}{\strut II} \colorbox{red!0}{\strut 2} \colorbox{red!0}{\strut 2Appointments} \colorbox{red!5}{\strut Clause} \colorbox{red!0}{\strut II} \colorbox{red!0}{\strut 2} \colorbox{red!0}{\strut 2Arisings} \colorbox{red!5}{\strut Clause} \colorbox{red!0}{\strut .} \colorbox{red!0}{\strut 1} \colorbox{red!0}{\strut .} \colorbox{red!0}{\strut III} \colorbox{red!0}{\strut 2} \colorbox{red!0}{\strut 1Basket} \colorbox{red!5}{\strut Clause} \colorbox{red!0}{\strut I} \colorbox{red!0}{\strut 8} \colorbox{red!0}{\strut 18Case} \colorbox{red!0}{\strut or} \colorbox{red!0}{\strut Controversy} \colorbox{red!5}{\strut Clause} \colorbox{red!0}{\strut III} \colorbox{red!0}{\strut 2} \colorbox{red!0}{\strut 1Coefficient} \colorbox{red!5}{\strut Clause} \colorbox{red!5}{\strut Clause} \colorbox{red!0}{\strut I} \colorbox{red!0}{\strut 8} \colorbox{red!0}{\strut 18Comity} \colorbox{red!5}{\strut Clause} \colorbox{red!0}{\strut IV} \colorbox{red!0}{\strut 2} \colorbox{red!0}{\strut 1Commerce} \colorbox{red!5}{\strut Clause} \colorbox{red!0}{\strut I} \colorbox{red!0}{\strut 8} \colorbox{red!0}{\strut 3Compact} \colorbox{red!5}{\strut Clause} \colorbox{red!0}{\strut I} \colorbox{red!0}{\strut 10} \colorbox{red!0}{\strut 3Contract} \colorbox{red!5}{\strut Clause} \colorbox{red!0}{\strut I} \colorbox{red!0}{\strut 10} \colorbox{red!0}{\strut 1Copyright} \colorbox{red!5}{\strut Clause} \colorbox{red!0}{\strut I} \colorbox{red!0}{\strut 8} \colorbox{red!0}{\strut 8Diversity} \colorbox{red!0}{\strut .} \colorbox{red!0}{\strut of} \colorbox{red!0}{\strut Citizenship} \colorbox{red!0}{\strut .} \colorbox{red!5}{\strut Clause} \colorbox{red!0}{\strut .} \colorbox{red!0}{\strut 1} \colorbox{red!0}{\strut .} \colorbox{red!0}{\strut III} \colorbox{red!0}{\strut 2} \colorbox{red!0}{\strut 1Elastic} \colorbox{red!5}{\strut Clause} \colorbox{red!0}{\strut I} \colorbox{red!0}{\strut 8} \colorbox{red!0}{\strut 18Emoluments} \colorbox{red!5}{\strut Clause} \colorbox{red!0}{\strut I} \colorbox{red!0}{\strut 6} \colorbox{red!0}{\strut 2Emolument} \colorbox{red!5}{\strut Clause} \colorbox{red!0}{\strut I} \colorbox{red!0}{\strut 9} \colorbox{red!0}{\strut 8Enclave} \colorbox{red!5}{\strut Clause} \colorbox{red!0}{\strut .} \colorbox{red!0}{\strut 1} \colorbox{red!0}{\strut .} \colorbox{red!0}{\strut I} \colorbox{red!0}{\strut 8} \colorbox{red!0}{\strut 17Excepting} \colorbox{red!5}{\strut Clause} \colorbox{red!0}{\strut .} \colorbox{red!0}{\strut 1} \colorbox{red!0}{\strut .} \colorbox{red!0}{\strut II} \colorbox{red!0}{\strut 2} \colorbox{red!0}{\strut 2Exceptions} \colorbox{red!5}{\strut Clause} \colorbox{red!0}{\strut III} \colorbox{red!0}{\strut 2} \colorbox{red!0}{\strut 2Export} \colorbox{red!5}{\strut Clause} \colorbox{red!0}{\strut I} \colorbox{red!0}{\strut 10} \colorbox{red!0}{\strut 2Extradition} \colorbox{red!5}{\strut Clause} \colorbox{red!0}{\strut IV} \colorbox{red!0}{\strut 2} \colorbox{red!0}{\strut 2Faithful} \colorbox{red!0}{\strut Execution} \colorbox{red!5}{\strut Clause} \colorbox{red!0}{\strut II} \colorbox{red!0}{\strut 3Faithfully} \colorbox{red!0}{\strut Executed} \colorbox{red!5}{\strut Clause} \colorbox{red!0}{\strut II} \colorbox{red!0}{\strut 3Foreign} \colorbox{red!0}{\strut Commerce} \colorbox{red!5}{\strut Clause} \colorbox{red!0}{\strut .} \colorbox{red!0}{\strut 1} \colorbox{red!0}{\strut .} \colorbox{red!0}{\strut I} \colorbox{red!0}{\strut 8} \colorbox{red!0}{\strut 3Fugitive} \colorbox{red!0}{\strut Slave} \colorbox{red!5}{\strut Clause} \colorbox{red!0}{\strut IV} \colorbox{red!0}{\strut 2} \colorbox{red!0}{\strut 3Full} \colorbox{red!0}{\strut Faith} \colorbox{red!0}{\strut and} 
}}}
\end{CJK*}

query: what is diflorasone diacetate cream used for

\begin{CJK*}{UTF8}{gbsn}
{\setlength{\fboxsep}{0pt}\colorbox{white!0}{\parbox{0.9\textwidth}{
\colorbox{red!0}{\strut Diflorasone} \colorbox{red!0}{\strut Diacetate} \colorbox{red!0}{\strut Uses} \colorbox{red!0}{\strut .} \colorbox{red!37}{\strut Skin} \colorbox{red!0}{\strut ChannelTopicsAllergic} \colorbox{red!4}{\strut Contact} \colorbox{red!0}{\strut DermatitisAlopecia} \colorbox{red!0}{\strut AreataAtopic} \colorbox{red!0}{\strut DermatitisBody} \colorbox{red!0}{\strut LiceBreast} \colorbox{red!0}{\strut CellulitisCellulitisContact} \colorbox{red!0}{\strut DermatitisDermatitis} \colorbox{red!0}{\strut HerpetiformisFacial} \colorbox{red!0}{\strut CellulitisHot} \colorbox{red!0}{\strut Tub} \colorbox{red!0}{\strut RashImpetigoIrritant} \colorbox{red!4}{\strut Contact} \colorbox{red!0}{\strut DermatitisLeg} \colorbox{red!0}{\strut CellulitisLiceLichen} \colorbox{red!0}{\strut SclerosusOrbital} \colorbox{red!0}{\strut CellulitisPerianal} \colorbox{red!0}{\strut CellulitisPeriorbital} \colorbox{red!0}{\strut CellulitisSkinSkin} \colorbox{red!0}{\strut ExamStaph} \colorbox{red!0}{\strut InfectionSwimmer} \colorbox{red!0}{\strut s} \colorbox{red!0}{\strut ItchVitiligoMedicationsAbobotulinumtoxinAAcitretinAdapaleneBenzoyl} \colorbox{red!0}{\strut PeroxideAlclometasoneAlefaceptAltabaxAmcinonideAquaphorAvageAzelaic} \colorbox{red!0}{\strut Acid} \colorbox{red!0}{\strut GelAzficel-TBenzyl} \colorbox{red!0}{\strut Alcohol} \colorbox{red!0}{\strut LotionBetamethasone} \colorbox{red!0}{\strut Valerate} \colorbox{red!0}{\strut FoamBotulinum} \colorbox{red!4}{\strut Toxin} \colorbox{red!4}{\strut Type} \colorbox{red!0}{\strut ABrimonidine} \colorbox{red!0}{\strut GelCalcipotrieneCalcipotrieneBetamethasone} \colorbox{red!0}{\strut DipropionateCalcitriol} \colorbox{red!0}{\strut OintmentCapexCinryzeClemastineClindamycinBenzoyl} \colorbox{red!0}{\strut PeroxideClobetasol} \colorbox{red!0}{\strut PropionateClobetasol} \colorbox{red!0}{\strut Propionate} \colorbox{red!0}{\strut FoamClobexCordran} \colorbox{red!0}{\strut SP} \colorbox{red!0}{\strut CreamCutivate} \colorbox{red!0}{\strut LotionDacarbazineDecadronDenileukin} \colorbox{red!0}{\strut DiftitoxDermatopDesonateDesonide} \colorbox{red!0}{\strut CreamDesoximetasoneDesoximetasone} \colorbox{red!0}{\strut SprayDiclofenac} \colorbox{red!0}{\strut GelDiflorasone} \colorbox{red!0}{\strut DiacetateDiflorasone} \colorbox{red!0}{\strut Emollient} \colorbox{red!0}{\strut CreamElidelErythromycinBenzoyl} \colorbox{red!0}{\strut PeroxideExtinaFirazyrFluocinolone} \colorbox{red!0}{\strut OilFluocinonideFlurandrenolide} \colorbox{red!0}{\strut LotionFluticasone} \colorbox{red!0}{\strut Propionate} \colorbox{red!0}{\strut CreamHalogHydrocortisone} \colorbox{red!0}{\strut ButyrateHydrogen} \colorbox{red!0}{\strut PeroxideHydroxyzineImiquimodIncobotulinumtoxinAInjectable} \colorbox{red!0}{\strut Poly-L} \colorbox{red!0}{\strut Lactic} \colorbox{red!0}{\strut AcidIstodaxIvermectin} \colorbox{red!0}{\strut LotionKalbitorKenalog} \colorbox{red!0}{\strut OintmentLamisilLidexMangosteenMetronidazole} \colorbox{red!0}{\strut GelMometasoneMometasone} \colorbox{red!0}{\strut Furoate} \colorbox{red!0}{\strut OintmentMupirocinNeosporinOnabotulinumtoxinAPicatoPromethazineProtopicRheumatrexSpinosadTazarotene} \colorbox{red!0}{\strut FoamTerbinafineTopical} \colorbox{red!0}{\strut Fluticasone} \colorbox{red!0}{\strut PropionateTriamcinoloneTriamcinolone} \colorbox{red!0}{\strut Acetonide} \colorbox{red!0}{\strut CreamUltravateUstekinumabVerdesoVorinostatXolegelZyclaraAdvertisementQuicklinksSkinLiceCellulitisVitiligoAlopecia} \colorbox{red!0}{\strut AreataLichen} \colorbox{red!0}{\strut SclerosisAtopic} \colorbox{red!0}{\strut DermatitisContact} \colorbox{red!0}{\strut DermatitisBody} \colorbox{red!0}{\strut LiceLamisilTriamcinoloneMangosteenHydroxyzinePromethazineStaph} \colorbox{red!0}{\strut InfectionImpetigoHydrogen} \colorbox{red!0}{\strut PeroxideRelated} \colorbox{red!0}{\strut ChannelsPsoriasisRosaceaSkin} \colorbox{red!0}{\strut CancerScabiesKidsPregnancyAdvertisementTweetSkin} \colorbox{red!0}{\strut Home} \colorbox{red!0}{\strut .} \colorbox{red!0}{\strut Diflorasone} \colorbox{red!0}{\strut Diacetate} \colorbox{red!0}{\strut UsesDiflorasone} \colorbox{red!0}{\strut Diacetate} \colorbox{red!0}{\strut UsesYour} \colorbox{red!0}{\strut healthcare} \colorbox{red!0}{\strut provider} \colorbox{red!0}{\strut may} \colorbox{red!0}{\strut recommend} \colorbox{red!0}{\strut using} \colorbox{red!0}{\strut diflorasone} \colorbox{red!0}{\strut diacetate} \colorbox{red!0}{\strut to} \colorbox{red!0}{\strut help} \colorbox{red!0}{\strut relieve} \colorbox{red!0}{\strut inflammation} \colorbox{red!0}{\strut and} \colorbox{red!0}{\strut itching} \colorbox{red!0}{\strut caused} \colorbox{red!0}{\strut by} \colorbox{red!0}{\strut various} \colorbox{red!37}{\strut skin} \colorbox{red!0}{\strut conditions} \colorbox{red!0}{\strut .} \colorbox{red!0}{\strut Specifically} \colorbox{red!0}{\strut ,} \colorbox{red!0}{\strut this} \colorbox{red!0}{\strut topical} \colorbox{red!37}{\strut skin} \colorbox{red!0}{\strut medicine} \colorbox{red!0}{\strut is} \colorbox{red!0}{\strut approved} \colorbox{red!0}{\strut for} \colorbox{red!0}{\strut treating} \colorbox{red!0}{\strut problems} \colorbox{red!0}{\strut such} \colorbox{red!0}{\strut as} \colorbox{red!0}{\strut dermatitis} \colorbox{red!0}{\strut ,} \colorbox{red!0}{\strut eczema} \colorbox{red!0}{\strut ,} \colorbox{red!0}{\strut and} \colorbox{red!0}{\strut poison} \colorbox{red!0}{\strut ivy} \colorbox{red!0}{\strut ,} \colorbox{red!0}{\strut just} \colorbox{red!0}{\strut to} \colorbox{red!0}{\strut name} \colorbox{red!0}{\strut a} \colorbox{red!0}{\strut few} \colorbox{red!0}{\strut .} \colorbox{red!0}{\strut It} \colorbox{red!0}{\strut works} \colorbox{red!0}{\strut by} \colorbox{red!0}{\strut suppressing} \colorbox{red!0}{\strut an} \colorbox{red!0}{\strut overactive} \colorbox{red!0}{\strut immune} \colorbox{red!0}{\strut system} \colorbox{red!0}{\strut and} \colorbox{red!0}{\strut reducing} \colorbox{red!0}{\strut inflammation} \colorbox{red!0}{\strut .} \colorbox{red!0}{\strut This} \colorbox{red!0}{\strut product} \colorbox{red!0}{\strut is} \colorbox{red!0}{\strut approved} \colorbox{red!0}{\strut for} \colorbox{red!0}{\strut use} \colorbox{red!0}{\strut in} \colorbox{red!0}{\strut adults} \colorbox{red!0}{\strut only.Interested} \colorbox{red!0}{\strut in} \colorbox{red!0}{\strut a} \colorbox{red!0}{\strut Discount} \colorbox{red!0}{\strut on} \colorbox{red!0}{\strut Diflorasone} \colorbox{red!0}{\strut Diacetate} \colorbox{red!0}{\strut ?} \colorbox{red!0}{\strut Our} \colorbox{red!0}{\strut free} \colorbox{red!0}{\strut DiscountRx} \colorbox{red!0}{\strut savings} \colorbox{red!0}{\strut card} \colorbox{red!0}{\strut can} \colorbox{red!0}{\strut help} \colorbox{red!0}{\strut you} \colorbox{red!0}{\strut and} \colorbox{red!0}{\strut your} \colorbox{red!0}{\strut family} \colorbox{red!0}{\strut save} \colorbox{red!0}{\strut money} \colorbox{red!0}{\strut on} \colorbox{red!0}{\strut your} \colorbox{red!0}{\strut prescriptions} \colorbox{red!0}{\strut .} \colorbox{red!0}{\strut This} \colorbox{red!0}{\strut card} \colorbox{red!0}{\strut is} \colorbox{red!0}{\strut accepted} \colorbox{red!0}{\strut at} \colorbox{red!0}{\strut all} \colorbox{red!0}{\strut major} \colorbox{red!0}{\strut chain} \colorbox{red!0}{\strut pharmacies} \colorbox{red!0}{\strut ,} \colorbox{red!0}{\strut nationwide} \colorbox{red!0}{\strut .} \colorbox{red!0}{\strut Enter} \colorbox{red!0}{\strut your} \colorbox{red!0}{\strut name} \colorbox{red!0}{\strut and} \colorbox{red!0}{\strut email} \colorbox{red!0}{\strut address} \colorbox{red!0}{\strut to} \colorbox{red!0}{\strut receive} \colorbox{red!0}{\strut your} \colorbox{red!0}{\strut free} \colorbox{red!0}{\strut savings} \colorbox{red!0}{\strut card.Enter} \colorbox{red!0}{\strut Your} \colorbox{red!0}{\strut NameEnter} \colorbox{red!0}{\strut Your} \colorbox{red!0}{\strut Email} \colorbox{red!0}{\strut AddressCLICK} \colorbox{red!0}{\strut HERE} \colorbox{red!0}{\strut to} \colorbox{red!0}{\strut learn} \colorbox{red!0}{\strut more} \colorbox{red!0}{\strut about} \colorbox{red!0}{\strut from} \colorbox{red!0}{\strut eMedTV.comWhat} \colorbox{red!0}{\strut Is} \colorbox{red!0}{\strut Diflorasone} \colorbox{red!0}{\strut Diacetate} \colorbox{red!0}{\strut Used} \colorbox{red!0}{\strut For} \colorbox{red!0}{\strut ?} \colorbox{red!0}{\strut Diflorasone} \colorbox{red!0}{\strut diacetate} \colorbox{red!0}{\strut is} \colorbox{red!0}{\strut a} \colorbox{red!0}{\strut prescription} \colorbox{red!37}{\strut skin} \colorbox{red!0}{\strut medication} \colorbox{red!0}{\strut used} \colorbox{red!0}{\strut to} \colorbox{red!0}{\strut treat} \colorbox{red!0}{\strut inflammation} \colorbox{red!0}{\strut and} \colorbox{red!0}{\strut itching} \colorbox{red!0}{\strut due} \colorbox{red!0}{\strut to} \colorbox{red!0}{\strut a} \colorbox{red!0}{\strut wide} \colorbox{red!0}{\strut variety} \colorbox{red!0}{\strut of} \colorbox{red!0}{\strut different} \colorbox{red!0}{\strut conditions} \colorbox{red!0}{\strut .} \colorbox{red!0}{\strut Such} \colorbox{red!0}{\strut conditions} \colorbox{red!0}{\strut include} \colorbox{red!0}{\strut but} \colorbox{red!0}{\strut are} \colorbox{red!0}{\strut not} \colorbox{red!0}{\strut limited} \colorbox{red!0}{\strut to} \colorbox{red!0}{\strut .} \colorbox{red!0}{\strut Atopic} \colorbox{red!0}{\strut dermatitisContact} \colorbox{red!0}{\strut dermatitisEczemaPsoriasisPoison} \colorbox{red!0}{\strut ivySeborrhea.Specifically} \colorbox{red!0}{\strut ,} \colorbox{red!0}{\strut diflorasone} \colorbox{red!0}{\strut diacetate} \colorbox{red!0}{\strut is} \colorbox{red!0}{\strut approved} \colorbox{red!0}{\strut to} \colorbox{red!0}{\strut treat} \colorbox{red!0}{\strut any} \colorbox{red!37}{\strut skin} \colorbox{red!0}{\strut condition} \colorbox{red!0}{\strut that} \colorbox{red!0}{\strut is} \colorbox{red!0}{\strut responsive} \colorbox{red!0}{\strut to} \colorbox{red!0}{\strut corticosteroids} \colorbox{red!0}{\strut .} \colorbox{red!0}{\strut diflorasone} \colorbox{red!0}{\strut diacetate} \colorbox{red!0}{\strut is} \colorbox{red!0}{\strut a} \colorbox{red!0}{\strut corticosteroid} \colorbox{red!0}{\strut .} \colorbox{red!0}{\strut .} \colorbox{red!0}{\strut This} \colorbox{red!0}{\strut is} \colorbox{red!0}{\strut a} \colorbox{red!0}{\strut broad} \colorbox{red!0}{\strut indication} \colorbox{red!0}{\strut .} \colorbox{red!0}{\strut This} \colorbox{red!0}{\strut medication} \colorbox{red!0}{\strut is} \colorbox{red!0}{\strut probably} \colorbox{red!0}{\strut used} \colorbox{red!0}{\strut most} \colorbox{red!0}{\strut often} \colorbox{red!0}{\strut for} \colorbox{red!0}{\strut treating} \colorbox{red!0}{\strut psoriasis} \colorbox{red!0}{\strut or} \colorbox{red!0}{\strut severe} 
}}}
\end{CJK*}

\begin{CJK*}{UTF8}{gbsn}
{\setlength{\fboxsep}{0pt}\colorbox{white!0}{\parbox{0.9\textwidth}{
\colorbox{red!1}{\strut Label} \colorbox{red!0}{\strut .} \colorbox{red!9}{\strut DIFLORASONE} \colorbox{red!0}{\strut DIACETATE-} \colorbox{red!9}{\strut diflorasone} \colorbox{red!8}{\strut diacetate} \colorbox{red!5}{\strut cream} \colorbox{red!0}{\strut NDC} \colorbox{red!0}{\strut Code} \colorbox{red!0}{\strut .} \colorbox{red!0}{\strut s} \colorbox{red!0}{\strut .} \colorbox{red!0}{\strut .} \colorbox{red!0}{\strut 51672-1296-1} \colorbox{red!0}{\strut ,} \colorbox{red!0}{\strut 51672-1296-2} \colorbox{red!0}{\strut ,} \colorbox{red!0}{\strut 51672-1296-3Packager} \colorbox{red!0}{\strut .} \colorbox{red!1}{\strut Taro} \colorbox{red!0}{\strut Pharmaceuticals} \colorbox{red!0}{\strut U.S.A.} \colorbox{red!0}{\strut ,} \colorbox{red!0}{\strut Inc.Category} \colorbox{red!0}{\strut .} \colorbox{red!0}{\strut HUMAN} \colorbox{red!1}{\strut PRESCRIPTION} \colorbox{red!1}{\strut DRUG} \colorbox{red!0}{\strut LABELDEA} \colorbox{red!0}{\strut Schedule} \colorbox{red!0}{\strut .} \colorbox{red!0}{\strut NoneMarketing} \colorbox{red!0}{\strut Status} \colorbox{red!0}{\strut .} \colorbox{red!0}{\strut Abbreviated} \colorbox{red!0}{\strut New} \colorbox{red!1}{\strut Drug} \colorbox{red!0}{\strut ApplicationDrug} \colorbox{red!1}{\strut Label} \colorbox{red!0}{\strut InformationUpdated} \colorbox{red!0}{\strut August} \colorbox{red!0}{\strut 31} \colorbox{red!0}{\strut ,} \colorbox{red!0}{\strut 2015If} \colorbox{red!0}{\strut you} \colorbox{red!0}{\strut are} \colorbox{red!0}{\strut a} \colorbox{red!0}{\strut consumer} \colorbox{red!0}{\strut or} \colorbox{red!0}{\strut patient} \colorbox{red!0}{\strut please} \colorbox{red!0}{\strut visit} \colorbox{red!0}{\strut this} \colorbox{red!0}{\strut version.Download} \colorbox{red!1}{\strut DRUG} \colorbox{red!1}{\strut LABEL} \colorbox{red!0}{\strut INFO} \colorbox{red!0}{\strut .} \colorbox{red!0}{\strut PDF} \colorbox{red!0}{\strut XML} \colorbox{red!0}{\strut Official} \colorbox{red!1}{\strut Label} \colorbox{red!0}{\strut .} \colorbox{red!0}{\strut Printer} \colorbox{red!0}{\strut Friendly} \colorbox{red!0}{\strut .} \colorbox{red!0}{\strut View} \colorbox{red!0}{\strut All} \colorbox{red!0}{\strut SectionsSPL} \colorbox{red!0}{\strut UNCLASSIFIED} \colorbox{red!0}{\strut SECTIONRx} \colorbox{red!0}{\strut only} \colorbox{red!0}{\strut For} \colorbox{red!0}{\strut External} \colorbox{red!0}{\strut Use} \colorbox{red!0}{\strut Only} \colorbox{red!0}{\strut -} \colorbox{red!0}{\strut Not} \colorbox{red!0}{\strut for} \colorbox{red!0}{\strut Ophthalmic} \colorbox{red!0}{\strut Use.DESCRIPTIONDiflorasone} \colorbox{red!8}{\strut diacetate} \colorbox{red!5}{\strut cream} \colorbox{red!1}{\strut USP} \colorbox{red!0}{\strut ,} \colorbox{red!0}{\strut 0.05} \colorbox{red!0}{\strut .} \colorbox{red!0}{\strut contains} \colorbox{red!0}{\strut the} \colorbox{red!0}{\strut active} \colorbox{red!0}{\strut compound} \colorbox{red!9}{\strut diflorasone} \colorbox{red!8}{\strut diacetate} \colorbox{red!0}{\strut ,} \colorbox{red!0}{\strut a} \colorbox{red!0}{\strut synthetic} \colorbox{red!2}{\strut corticosteroid} \colorbox{red!0}{\strut for} \colorbox{red!1}{\strut topical} \colorbox{red!0}{\strut dermatological} \colorbox{red!0}{\strut use} \colorbox{red!0}{\strut .} \colorbox{red!1}{\strut Chemically} \colorbox{red!0}{\strut ,} \colorbox{red!9}{\strut diflorasone} \colorbox{red!8}{\strut diacetate} \colorbox{red!0}{\strut is} \colorbox{red!0}{\strut ...} \colorbox{red!0}{\strut CLINICAL} \colorbox{red!0}{\strut PHARMACOLOGYLike} \colorbox{red!0}{\strut other} \colorbox{red!1}{\strut topical} \colorbox{red!1}{\strut corticosteroids} \colorbox{red!0}{\strut ,} \colorbox{red!9}{\strut diflorasone} \colorbox{red!8}{\strut diacetate} \colorbox{red!0}{\strut has} \colorbox{red!0}{\strut anti-inflammatory} \colorbox{red!0}{\strut ,} \colorbox{red!0}{\strut anti-pruritic} \colorbox{red!0}{\strut ,} \colorbox{red!0}{\strut and} \colorbox{red!0}{\strut vasoconstrictive} \colorbox{red!0}{\strut actions} \colorbox{red!0}{\strut .} \colorbox{red!0}{\strut The} \colorbox{red!0}{\strut mechanism} \colorbox{red!0}{\strut of} \colorbox{red!0}{\strut the} \colorbox{red!0}{\strut anti-inflammatory} \colorbox{red!0}{\strut activity} \colorbox{red!0}{\strut of} \colorbox{red!0}{\strut the} \colorbox{red!1}{\strut topical} \colorbox{red!0}{\strut ...} \colorbox{red!0}{\strut INDICATION} \colorbox{red!0}{\strut AND} \colorbox{red!0}{\strut USAGEDiflorasone} \colorbox{red!8}{\strut diacetate} \colorbox{red!5}{\strut cream} \colorbox{red!1}{\strut USP} \colorbox{red!0}{\strut ,} \colorbox{red!0}{\strut 0.05} \colorbox{red!0}{\strut .} \colorbox{red!0}{\strut is} \colorbox{red!0}{\strut a} \colorbox{red!0}{\strut high} \colorbox{red!0}{\strut potency} \colorbox{red!2}{\strut corticosteroid} \colorbox{red!0}{\strut indicated} \colorbox{red!0}{\strut for} \colorbox{red!0}{\strut the} \colorbox{red!0}{\strut relief} \colorbox{red!0}{\strut of} \colorbox{red!0}{\strut the} \colorbox{red!1}{\strut inflammatory} \colorbox{red!0}{\strut and} \colorbox{red!1}{\strut pruritic} \colorbox{red!0}{\strut manifestations} \colorbox{red!0}{\strut of} \colorbox{red!0}{\strut corticosteroid-responsive} \colorbox{red!0}{\strut dermatoses} \colorbox{red!0}{\strut ...} \colorbox{red!0}{\strut CONTRAINDICATIONSDiflorasone} \colorbox{red!8}{\strut diacetate} \colorbox{red!5}{\strut cream} \colorbox{red!1}{\strut USP} \colorbox{red!0}{\strut is} \colorbox{red!0}{\strut contraindicated} \colorbox{red!0}{\strut in} \colorbox{red!0}{\strut those} \colorbox{red!0}{\strut patients} \colorbox{red!0}{\strut with} \colorbox{red!0}{\strut a} \colorbox{red!0}{\strut history} \colorbox{red!0}{\strut of} \colorbox{red!0}{\strut hypersensitivity} \colorbox{red!0}{\strut to} \colorbox{red!0}{\strut any} \colorbox{red!0}{\strut of} \colorbox{red!0}{\strut the} \colorbox{red!0}{\strut components} \colorbox{red!0}{\strut of} \colorbox{red!0}{\strut the} \colorbox{red!0}{\strut preparation.PRECAUTIONSGeneral} \colorbox{red!0}{\strut -} \colorbox{red!0}{\strut Systemic} \colorbox{red!0}{\strut absorption} \colorbox{red!0}{\strut of} \colorbox{red!1}{\strut topical} \colorbox{red!1}{\strut corticosteroids} \colorbox{red!0}{\strut can} \colorbox{red!0}{\strut produce} \colorbox{red!0}{\strut reversible} \colorbox{red!0}{\strut hypothalamic-pituitary-adrenal} \colorbox{red!0}{\strut .} \colorbox{red!0}{\strut HPA} \colorbox{red!0}{\strut .} \colorbox{red!0}{\strut axis} \colorbox{red!0}{\strut suppression} \colorbox{red!0}{\strut with} \colorbox{red!0}{\strut the} \colorbox{red!0}{\strut potential} \colorbox{red!0}{\strut for} \colorbox{red!0}{\strut ...} \colorbox{red!1}{\strut ADVERSE} \colorbox{red!0}{\strut REACTIONSThe} \colorbox{red!0}{\strut following} \colorbox{red!0}{\strut local} \colorbox{red!1}{\strut adverse} \colorbox{red!0}{\strut reactions} \colorbox{red!0}{\strut have} \colorbox{red!0}{\strut been} \colorbox{red!0}{\strut reported} \colorbox{red!0}{\strut infrequently} \colorbox{red!0}{\strut with} \colorbox{red!0}{\strut other} \colorbox{red!1}{\strut topical} \colorbox{red!1}{\strut corticosteroids} \colorbox{red!0}{\strut ,} \colorbox{red!0}{\strut and} \colorbox{red!0}{\strut they} \colorbox{red!0}{\strut may} \colorbox{red!0}{\strut occur} \colorbox{red!0}{\strut more} \colorbox{red!0}{\strut frequently} \colorbox{red!0}{\strut with} \colorbox{red!0}{\strut the} \colorbox{red!0}{\strut use} \colorbox{red!0}{\strut of} \colorbox{red!1}{\strut occlusive} \colorbox{red!0}{\strut dressings} \colorbox{red!0}{\strut ,} \colorbox{red!0}{\strut especially} \colorbox{red!0}{\strut ...} \colorbox{red!0}{\strut OVERDOSAGETopically} \colorbox{red!0}{\strut applied} \colorbox{red!9}{\strut diflorasone} \colorbox{red!8}{\strut diacetate} \colorbox{red!5}{\strut cream} \colorbox{red!1}{\strut USP} \colorbox{red!0}{\strut ,} \colorbox{red!0}{\strut 0.05} \colorbox{red!0}{\strut .} \colorbox{red!0}{\strut can} \colorbox{red!0}{\strut be} \colorbox{red!0}{\strut absorbed} \colorbox{red!0}{\strut in} \colorbox{red!0}{\strut sufficient} \colorbox{red!0}{\strut amounts} \colorbox{red!0}{\strut to} \colorbox{red!0}{\strut produce} \colorbox{red!0}{\strut systemic} \colorbox{red!0}{\strut effects} \colorbox{red!0}{\strut .} \colorbox{red!0}{\strut see} \colorbox{red!0}{\strut PRECAUTIONS} \colorbox{red!0}{\strut .} \colorbox{red!0}{\strut .DOSAGE} \colorbox{red!0}{\strut AND} \colorbox{red!0}{\strut ADMINISTRATIONDiflorasone} \colorbox{red!8}{\strut diacetate} \colorbox{red!5}{\strut cream} \colorbox{red!1}{\strut USP} \colorbox{red!0}{\strut ,} \colorbox{red!0}{\strut 0.05} \colorbox{red!0}{\strut .} \colorbox{red!0}{\strut should} \colorbox{red!0}{\strut be} \colorbox{red!0}{\strut applied} \colorbox{red!0}{\strut to} \colorbox{red!0}{\strut the} \colorbox{red!0}{\strut affected} \colorbox{red!0}{\strut area} \colorbox{red!0}{\strut twice} \colorbox{red!0}{\strut daily.HOW} \colorbox{red!0}{\strut SUPPLIEDDiflorasone} \colorbox{red!8}{\strut diacetate} \colorbox{red!5}{\strut cream} \colorbox{red!1}{\strut USP} \colorbox{red!0}{\strut ,} \colorbox{red!0}{\strut 0.05} \colorbox{red!0}{\strut .} \colorbox{red!0}{\strut is} \colorbox{red!0}{\strut available} \colorbox{red!0}{\strut in} \colorbox{red!0}{\strut 15} \colorbox{red!0}{\strut g} \colorbox{red!0}{\strut .} \colorbox{red!0}{\strut NDC} \colorbox{red!0}{\strut 51672-1296-1} \colorbox{red!0}{\strut .} \colorbox{red!0}{\strut ,} \colorbox{red!0}{\strut 30} \colorbox{red!0}{\strut g} \colorbox{red!0}{\strut .} \colorbox{red!0}{\strut NDC} \colorbox{red!0}{\strut 51672-1296-2} \colorbox{red!0}{\strut .} \colorbox{red!0}{\strut and} 
}}}
\end{CJK*}

query: general izzam

\begin{CJK*}{UTF8}{gbsn}
{\setlength{\fboxsep}{0pt}\colorbox{white!0}{\parbox{0.9\textwidth}{
\colorbox{red!2}{\strut Board} \colorbox{red!0}{\strut of} \colorbox{red!1}{\strut Directors} \colorbox{red!2}{\strut Board} \colorbox{red!0}{\strut of} \colorbox{red!0}{\strut DirectorsAmir} \colorbox{red!0}{\strut AhamedChairman} \colorbox{red!0}{\strut ,} \colorbox{red!1}{\strut President} \colorbox{red!0}{\strut .} \colorbox{red!0}{\strut CEOAmir} \colorbox{red!0}{\strut Ahamed} \colorbox{red!2}{\strut founded} \colorbox{red!0}{\strut The} \colorbox{red!21}{\strut Regency} \colorbox{red!8}{\strut Group} \colorbox{red!0}{\strut in} \colorbox{red!0}{\strut August} \colorbox{red!0}{\strut 1983} \colorbox{red!0}{\strut and} \colorbox{red!0}{\strut is} \colorbox{red!0}{\strut the} \colorbox{red!0}{\strut firm} \colorbox{red!0}{\strut .} \colorbox{red!0}{\strut s} \colorbox{red!1}{\strut President} \colorbox{red!0}{\strut .} \colorbox{red!4}{\strut CEO} \colorbox{red!0}{\strut .} \colorbox{red!0}{\strut Amir} \colorbox{red!0}{\strut is} \colorbox{red!0}{\strut responsible} \colorbox{red!0}{\strut for} \colorbox{red!0}{\strut the} \colorbox{red!0}{\strut all} \colorbox{red!0}{\strut operations} \colorbox{red!0}{\strut of} \colorbox{red!0}{\strut the} \colorbox{red!0}{\strut Group.He} \colorbox{red!0}{\strut has} \colorbox{red!0}{\strut since} \colorbox{red!0}{\strut grown} \colorbox{red!0}{\strut the} \colorbox{red!0}{\strut business} \colorbox{red!0}{\strut to} \colorbox{red!0}{\strut include} \colorbox{red!0}{\strut various} \colorbox{red!0}{\strut real} \colorbox{red!0}{\strut estate} \colorbox{red!0}{\strut holdings} \colorbox{red!0}{\strut .} \colorbox{red!0}{\strut multi-family} \colorbox{red!0}{\strut residential} \colorbox{red!0}{\strut ,} \colorbox{red!0}{\strut commercial} \colorbox{red!0}{\strut ,} \colorbox{red!0}{\strut retail} \colorbox{red!0}{\strut ,} \colorbox{red!0}{\strut development} \colorbox{red!0}{\strut .} \colorbox{red!0}{\strut ,} \colorbox{red!0}{\strut up} \colorbox{red!0}{\strut to} \colorbox{red!0}{\strut 14} \colorbox{red!0}{\strut OEM} \colorbox{red!0}{\strut franchises} \colorbox{red!0}{\strut across} \colorbox{red!0}{\strut 9} \colorbox{red!0}{\strut dealerships} \colorbox{red!0}{\strut at} \colorbox{red!0}{\strut the} \colorbox{red!0}{\strut peak} \colorbox{red!0}{\strut of} \colorbox{red!21}{\strut Regency} \colorbox{red!8}{\strut Auto} \colorbox{red!0}{\strut ,} \colorbox{red!0}{\strut and} \colorbox{red!2}{\strut managing} \colorbox{red!0}{\strut various} \colorbox{red!0}{\strut other} \colorbox{red!0}{\strut investments} \colorbox{red!0}{\strut in} \colorbox{red!0}{\strut operating} \colorbox{red!1}{\strut companies} \colorbox{red!0}{\strut .} \colorbox{red!0}{\strut Amir} \colorbox{red!0}{\strut has} \colorbox{red!0}{\strut held} \colorbox{red!0}{\strut principal} \colorbox{red!0}{\strut responsibility} \colorbox{red!0}{\strut for} \colorbox{red!0}{\strut all} \colorbox{red!0}{\strut operations} \colorbox{red!0}{\strut of} \colorbox{red!21}{\strut Regency} \colorbox{red!8}{\strut Auto} \colorbox{red!0}{\strut since} \colorbox{red!0}{\strut 1983} \colorbox{red!0}{\strut and} \colorbox{red!0}{\strut has} \colorbox{red!0}{\strut been} \colorbox{red!0}{\strut the} \colorbox{red!0}{\strut driving} \colorbox{red!0}{\strut force} \colorbox{red!0}{\strut of} \colorbox{red!0}{\strut The} \colorbox{red!21}{\strut Regency} \colorbox{red!0}{\strut Group.In} \colorbox{red!0}{\strut 1998} \colorbox{red!0}{\strut ,} \colorbox{red!0}{\strut Amir} \colorbox{red!0}{\strut was} \colorbox{red!0}{\strut awarded} \colorbox{red!0}{\strut the} \colorbox{red!0}{\strut Ernst} \colorbox{red!0}{\strut .} \colorbox{red!0}{\strut Young} \colorbox{red!0}{\strut Entrepreneur} \colorbox{red!0}{\strut of} \colorbox{red!0}{\strut the} \colorbox{red!0}{\strut Year} \colorbox{red!0}{\strut award} \colorbox{red!0}{\strut for} \colorbox{red!0}{\strut his} \colorbox{red!0}{\strut work} \colorbox{red!0}{\strut with} \colorbox{red!21}{\strut Regency} \colorbox{red!8}{\strut Auto} \colorbox{red!0}{\strut .} \colorbox{red!0}{\strut Amir} \colorbox{red!0}{\strut has} \colorbox{red!0}{\strut chaired} \colorbox{red!0}{\strut the} \colorbox{red!0}{\strut Lexus} \colorbox{red!0}{\strut Communications} \colorbox{red!0}{\strut Team} \colorbox{red!0}{\strut .} \colorbox{red!0}{\strut Canada} \colorbox{red!0}{\strut .} \colorbox{red!0}{\strut and} \colorbox{red!0}{\strut was} \colorbox{red!0}{\strut an} \colorbox{red!0}{\strut active} \colorbox{red!2}{\strut board} \colorbox{red!0}{\strut member} \colorbox{red!0}{\strut of} \colorbox{red!0}{\strut both} \colorbox{red!0}{\strut the} \colorbox{red!0}{\strut BC} \colorbox{red!0}{\strut Cancer} \colorbox{red!0}{\strut Foundation} \colorbox{red!0}{\strut as} \colorbox{red!0}{\strut well} \colorbox{red!0}{\strut as} \colorbox{red!0}{\strut Collingwood} \colorbox{red!0}{\strut School} \colorbox{red!0}{\strut .} \colorbox{red!0}{\strut Vice} \colorbox{red!0}{\strut Chairman} \colorbox{red!0}{\strut .} \colorbox{red!0}{\strut Chairman} \colorbox{red!0}{\strut of} \colorbox{red!0}{\strut Building} \colorbox{red!0}{\strut Committee} \colorbox{red!0}{\strut for} \colorbox{red!0}{\strut new} \colorbox{red!0}{\strut campus} \colorbox{red!0}{\strut at} \colorbox{red!0}{\strut Wentworth} \colorbox{red!0}{\strut .} \colorbox{red!0}{\strut .Aleem} \colorbox{red!0}{\strut AhamedManaging} \colorbox{red!0}{\strut DirectorAleem} \colorbox{red!0}{\strut Ahamed} \colorbox{red!0}{\strut is} \colorbox{red!2}{\strut Managing} \colorbox{red!2}{\strut Director} \colorbox{red!0}{\strut and} \colorbox{red!0}{\strut holds} \colorbox{red!0}{\strut responsibility} \colorbox{red!0}{\strut for} \colorbox{red!2}{\strut managing} \colorbox{red!0}{\strut the} \colorbox{red!0}{\strut existing} \colorbox{red!0}{\strut investment} \colorbox{red!0}{\strut portfolio} \colorbox{red!0}{\strut as} \colorbox{red!0}{\strut well} \colorbox{red!0}{\strut as} \colorbox{red!0}{\strut sourcing} \colorbox{red!0}{\strut new} \colorbox{red!0}{\strut opportunities.Aleem} \colorbox{red!0}{\strut joined} \colorbox{red!0}{\strut The} \colorbox{red!21}{\strut Regency} \colorbox{red!8}{\strut Group} \colorbox{red!0}{\strut in} \colorbox{red!0}{\strut 2013} \colorbox{red!0}{\strut after} \colorbox{red!0}{\strut spending} \colorbox{red!0}{\strut nearly} \colorbox{red!0}{\strut 10} \colorbox{red!0}{\strut years} \colorbox{red!0}{\strut in} \colorbox{red!0}{\strut the} \colorbox{red!0}{\strut financial} \colorbox{red!0}{\strut services} \colorbox{red!0}{\strut industry} \colorbox{red!0}{\strut .} \colorbox{red!0}{\strut Aleem} \colorbox{red!0}{\strut worked} \colorbox{red!0}{\strut for} \colorbox{red!1}{\strut Bank} \colorbox{red!0}{\strut of} \colorbox{red!0}{\strut Montreal} \colorbox{red!0}{\strut in} \colorbox{red!0}{\strut various} \colorbox{red!0}{\strut capacities} \colorbox{red!0}{\strut in} \colorbox{red!0}{\strut both} \colorbox{red!0}{\strut Vancouver} \colorbox{red!0}{\strut and} \colorbox{red!0}{\strut Toronto} \colorbox{red!0}{\strut including} \colorbox{red!0}{\strut Commercial} \colorbox{red!0}{\strut Banking} \colorbox{red!0}{\strut ,} \colorbox{red!0}{\strut Real} \colorbox{red!0}{\strut Estate} \colorbox{red!0}{\strut Finance} \colorbox{red!0}{\strut ,} \colorbox{red!0}{\strut and} \colorbox{red!1}{\strut Corporate} \colorbox{red!0}{\strut Finance} \colorbox{red!0}{\strut as} \colorbox{red!0}{\strut well} \colorbox{red!0}{\strut as} \colorbox{red!0}{\strut spending} \colorbox{red!0}{\strut time} \colorbox{red!0}{\strut in} \colorbox{red!0}{\strut Chicago} \colorbox{red!0}{\strut ,} \colorbox{red!0}{\strut IL} \colorbox{red!0}{\strut and} \colorbox{red!0}{\strut Milwaukee} \colorbox{red!0}{\strut ,} \colorbox{red!0}{\strut WI} \colorbox{red!1}{\strut where} \colorbox{red!0}{\strut he} \colorbox{red!0}{\strut worked} \colorbox{red!0}{\strut on} \colorbox{red!0}{\strut the} \colorbox{red!0}{\strut acquisition} \colorbox{red!0}{\strut and} \colorbox{red!0}{\strut integration} \colorbox{red!0}{\strut of} \colorbox{red!0}{\strut Marshall} \colorbox{red!0}{\strut .} \colorbox{red!0}{\strut Ilsley} \colorbox{red!1}{\strut Bank} \colorbox{red!0}{\strut ,} \colorbox{red!0}{\strut which} \colorbox{red!0}{\strut closed} \colorbox{red!0}{\strut in} \colorbox{red!0}{\strut 2012} \colorbox{red!0}{\strut .} \colorbox{red!0}{\strut Following} \colorbox{red!0}{\strut his} \colorbox{red!0}{\strut time} \colorbox{red!0}{\strut at} \colorbox{red!1}{\strut Bank} \colorbox{red!0}{\strut of} \colorbox{red!0}{\strut Montreal} \colorbox{red!0}{\strut ,} \colorbox{red!0}{\strut Aleem} \colorbox{red!0}{\strut worked} \colorbox{red!0}{\strut at} \colorbox{red!0}{\strut Aver} \colorbox{red!0}{\strut Media} \colorbox{red!0}{\strut LP} \colorbox{red!0}{\strut ,} \colorbox{red!0}{\strut a} \colorbox{red!0}{\strut media} \colorbox{red!1}{\strut bank} \colorbox{red!2}{\strut founded} \colorbox{red!0}{\strut in} \colorbox{red!0}{\strut 2006} \colorbox{red!0}{\strut .} \colorbox{red!0}{\strut partially} \colorbox{red!0}{\strut owned} \colorbox{red!0}{\strut by} \colorbox{red!0}{\strut a} \colorbox{red!0}{\strut pension} \colorbox{red!0}{\strut fund} \colorbox{red!0}{\strut .} \colorbox{red!0}{\strut ,} \colorbox{red!1}{\strut where} \colorbox{red!0}{\strut he} \colorbox{red!0}{\strut had} \colorbox{red!0}{\strut responsibilities} 
}}}
\end{CJK*}

\begin{CJK*}{UTF8}{gbsn}
{\setlength{\fboxsep}{0pt}\colorbox{white!0}{\parbox{0.9\textwidth}{
\colorbox{red!13}{\strut generalize} \colorbox{red!13}{\strut generalize} \colorbox{red!0}{\strut .} \colorbox{red!0}{\strut jen} \colorbox{red!0}{\strut -er-} \colorbox{red!0}{\strut uh} \colorbox{red!0}{\strut -lahyz} \colorbox{red!0}{\strut .} \colorbox{red!0}{\strut SpellSyllablesExamples} \colorbox{red!1}{\strut Word} \colorbox{red!0}{\strut OriginSee} \colorbox{red!0}{\strut more} \colorbox{red!0}{\strut synonyms} \colorbox{red!0}{\strut on} \colorbox{red!0}{\strut Thesaurus.comverb} \colorbox{red!0}{\strut .} \colorbox{red!0}{\strut used} \colorbox{red!0}{\strut with} \colorbox{red!1}{\strut object} \colorbox{red!0}{\strut .} \colorbox{red!0}{\strut ,} \colorbox{red!2}{\strut generalized} \colorbox{red!0}{\strut ,} \colorbox{red!0}{\strut generalizing.1} \colorbox{red!0}{\strut .} \colorbox{red!0}{\strut to} \colorbox{red!1}{\strut infer} \colorbox{red!0}{\strut .} \colorbox{red!0}{\strut a} \colorbox{red!12}{\strut general} \colorbox{red!1}{\strut principle} \colorbox{red!0}{\strut ,} \colorbox{red!0}{\strut trend} \colorbox{red!0}{\strut ,} \colorbox{red!0}{\strut etc} \colorbox{red!0}{\strut .} \colorbox{red!0}{\strut .} \colorbox{red!0}{\strut from} \colorbox{red!0}{\strut particular} \colorbox{red!0}{\strut facts} \colorbox{red!0}{\strut ,} \colorbox{red!0}{\strut statistics} \colorbox{red!0}{\strut ,} \colorbox{red!0}{\strut or} \colorbox{red!0}{\strut the} \colorbox{red!0}{\strut like.2} \colorbox{red!0}{\strut .} \colorbox{red!0}{\strut to} \colorbox{red!1}{\strut infer} \colorbox{red!0}{\strut or} \colorbox{red!0}{\strut form} \colorbox{red!0}{\strut .} \colorbox{red!0}{\strut a} \colorbox{red!12}{\strut general} \colorbox{red!1}{\strut principle} \colorbox{red!0}{\strut ,} \colorbox{red!0}{\strut opinion} \colorbox{red!0}{\strut ,} \colorbox{red!0}{\strut conclusion} \colorbox{red!0}{\strut ,} \colorbox{red!0}{\strut etc} \colorbox{red!0}{\strut .} \colorbox{red!0}{\strut .} \colorbox{red!0}{\strut from} \colorbox{red!0}{\strut only} \colorbox{red!0}{\strut a} \colorbox{red!0}{\strut few} \colorbox{red!0}{\strut facts} \colorbox{red!0}{\strut ,} \colorbox{red!0}{\strut examples} \colorbox{red!0}{\strut ,} \colorbox{red!0}{\strut or} \colorbox{red!0}{\strut the} \colorbox{red!0}{\strut like.3} \colorbox{red!0}{\strut .} \colorbox{red!0}{\strut to} \colorbox{red!0}{\strut give} \colorbox{red!0}{\strut a} \colorbox{red!12}{\strut general} \colorbox{red!0}{\strut rather} \colorbox{red!0}{\strut than} \colorbox{red!0}{\strut a} \colorbox{red!0}{\strut specific} \colorbox{red!0}{\strut or} \colorbox{red!0}{\strut special} \colorbox{red!0}{\strut character} \colorbox{red!0}{\strut or} \colorbox{red!0}{\strut form} \colorbox{red!0}{\strut to.4} \colorbox{red!0}{\strut .} \colorbox{red!0}{\strut to} \colorbox{red!0}{\strut make} \colorbox{red!12}{\strut general} \colorbox{red!0}{\strut .} \colorbox{red!0}{\strut bring} \colorbox{red!0}{\strut into} \colorbox{red!12}{\strut general} \colorbox{red!0}{\strut use} \colorbox{red!0}{\strut or} \colorbox{red!0}{\strut knowledge.verb} \colorbox{red!0}{\strut .} \colorbox{red!0}{\strut used} \colorbox{red!0}{\strut without} \colorbox{red!1}{\strut object} \colorbox{red!0}{\strut .} \colorbox{red!0}{\strut ,} \colorbox{red!2}{\strut generalized} \colorbox{red!0}{\strut ,} \colorbox{red!0}{\strut generalizing.5} \colorbox{red!0}{\strut .} \colorbox{red!0}{\strut to} \colorbox{red!0}{\strut form} \colorbox{red!12}{\strut general} \colorbox{red!1}{\strut principles} \colorbox{red!0}{\strut ,} \colorbox{red!0}{\strut opinions} \colorbox{red!0}{\strut ,} \colorbox{red!0}{\strut etc.6} \colorbox{red!0}{\strut .} \colorbox{red!0}{\strut to} \colorbox{red!0}{\strut deal} \colorbox{red!0}{\strut ,} \colorbox{red!0}{\strut think} \colorbox{red!0}{\strut ,} \colorbox{red!0}{\strut or} \colorbox{red!1}{\strut speak} \colorbox{red!0}{\strut in} \colorbox{red!0}{\strut generalities.7} \colorbox{red!0}{\strut .} \colorbox{red!0}{\strut to} \colorbox{red!0}{\strut make} \colorbox{red!12}{\strut general} \colorbox{red!0}{\strut inferences.ExpandAlso} \colorbox{red!0}{\strut ,} \colorbox{red!0}{\strut especially} \colorbox{red!0}{\strut British} \colorbox{red!0}{\strut ,} \colorbox{red!0}{\strut generalise.Origin} \colorbox{red!0}{\strut of} \colorbox{red!0}{\strut generalizeExpand1745-1755First} \colorbox{red!0}{\strut recorded} \colorbox{red!0}{\strut in} \colorbox{red!0}{\strut 1745-55} \colorbox{red!0}{\strut .} \colorbox{red!12}{\strut general} \colorbox{red!0}{\strut .} \colorbox{red!0}{\strut -izeRelated} \colorbox{red!0}{\strut formsExpandgeneralizable} \colorbox{red!0}{\strut ,} \colorbox{red!0}{\strut adjectivegeneralizer} \colorbox{red!0}{\strut ,} \colorbox{red!0}{\strut nounnongeneralized} \colorbox{red!0}{\strut ,} \colorbox{red!0}{\strut adjectiveungeneralized} \colorbox{red!0}{\strut ,} \colorbox{red!0}{\strut adjectiveungeneralizing} \colorbox{red!0}{\strut ,} \colorbox{red!0}{\strut adjectiveDictionary.com} \colorbox{red!0}{\strut Unabridged} \colorbox{red!0}{\strut Based} \colorbox{red!0}{\strut on} \colorbox{red!0}{\strut the} \colorbox{red!0}{\strut Random} \colorbox{red!0}{\strut House} \colorbox{red!0}{\strut Dictionary} \colorbox{red!0}{\strut ,} \colorbox{red!0}{\strut .} \colorbox{red!0}{\strut Random} \colorbox{red!0}{\strut House} \colorbox{red!0}{\strut ,} \colorbox{red!0}{\strut Inc.} \colorbox{red!0}{\strut 2018} \colorbox{red!0}{\strut .} \colorbox{red!0}{\strut Cite} \colorbox{red!0}{\strut This} \colorbox{red!0}{\strut SourceExamples} \colorbox{red!0}{\strut from} \colorbox{red!0}{\strut the} \colorbox{red!0}{\strut Web} \colorbox{red!0}{\strut for} \colorbox{red!0}{\strut generalizeExpandContemporary} \colorbox{red!0}{\strut ExamplesTel} \colorbox{red!0}{\strut Aviv} \colorbox{red!0}{\strut ,} \colorbox{red!0}{\strut to} \colorbox{red!13}{\strut generalize} \colorbox{red!0}{\strut but} \colorbox{red!0}{\strut slightly} \colorbox{red!0}{\strut ,} \colorbox{red!0}{\strut dislikes} \colorbox{red!0}{\strut Netanyahu} \colorbox{red!0}{\strut and} \colorbox{red!0}{\strut fears} \colorbox{red!0}{\strut the} \colorbox{red!0}{\strut future} \colorbox{red!0}{\strut he} \colorbox{red!0}{\strut personifies.Resigned} \colorbox{red!0}{\strut To} \colorbox{red!0}{\strut Loss} \colorbox{red!0}{\strut ,} \colorbox{red!0}{\strut But} \colorbox{red!0}{\strut Optimism} \colorbox{red!0}{\strut On} \colorbox{red!0}{\strut The} \colorbox{red!0}{\strut Center-LeftFania} \colorbox{red!0}{\strut Oz-SalzbergerJanuary} \colorbox{red!0}{\strut 22} \colorbox{red!0}{\strut ,} \colorbox{red!0}{\strut 2013I} \colorbox{red!0}{\strut do} \colorbox{red!0}{\strut nt} \colorbox{red!0}{\strut think} \colorbox{red!0}{\strut it} \colorbox{red!0}{\strut s} \colorbox{red!0}{\strut safe} \colorbox{red!0}{\strut to} \colorbox{red!13}{\strut generalize} \colorbox{red!0}{\strut about} \colorbox{red!0}{\strut any} \colorbox{red!0}{\strut industry} \colorbox{red!0}{\strut or} \colorbox{red!0}{\strut the} \colorbox{red!0}{\strut people} \colorbox{red!0}{\strut therein.Jennie} \colorbox{red!0}{\strut Ketcham} \colorbox{red!0}{\strut Interview} \colorbox{red!0}{\strut .} \colorbox{red!0}{\strut Recovering} \colorbox{red!0}{\strut From} \colorbox{red!0}{\strut Sex} \colorbox{red!0}{\strut AddictionRachel} \colorbox{red!0}{\strut Kramer} \colorbox{red!0}{\strut BusselJuly} \colorbox{red!0}{\strut 27} \colorbox{red!0}{\strut ,} \colorbox{red!0}{\strut 2012It} \colorbox{red!0}{\strut is} \colorbox{red!0}{\strut impossible} \colorbox{red!0}{\strut to} \colorbox{red!13}{\strut generalize} \colorbox{red!0}{\strut on} \colorbox{red!0}{\strut the} \colorbox{red!0}{\strut issue} \colorbox{red!0}{\strut of} \colorbox{red!0}{\strut Jewish} \colorbox{red!0}{\strut councils.Claude} \colorbox{red!0}{\strut Lanzmann} \colorbox{red!0}{\strut on} \colorbox{red!0}{\strut Shoah} \colorbox{red!0}{\strut .} \colorbox{red!0}{\strut ,} \colorbox{red!0}{\strut His} \colorbox{red!0}{\strut Memoir} \colorbox{red!0}{\strut ,} \colorbox{red!0}{\strut and} \colorbox{red!0}{\strut the} \colorbox{red!0}{\strut Banality} \colorbox{red!0}{\strut of} \colorbox{red!0}{\strut EvilClmence} \colorbox{red!0}{\strut BoulouqueJune} \colorbox{red!0}{\strut 11} \colorbox{red!0}{\strut ,} \colorbox{red!0}{\strut 2012Not} \colorbox{red!0}{\strut to} \colorbox{red!13}{\strut generalize} \colorbox{red!0}{\strut or} \colorbox{red!0}{\strut anything} \colorbox{red!0}{\strut ,} \colorbox{red!0}{\strut but} \colorbox{red!0}{\strut in} \colorbox{red!0}{\strut our} \colorbox{red!0}{\strut very} \colorbox{red!0}{\strut limited} \colorbox{red!0}{\strut world} \colorbox{red!0}{\strut ,} \colorbox{red!0}{\strut it} \colorbox{red!0}{\strut seems} \colorbox{red!0}{\strut like} \colorbox{red!0}{\strut everyone} \colorbox{red!0}{\strut drinks} \colorbox{red!0}{\strut .} \colorbox{red!0}{\strut or} \colorbox{red!0}{\strut at} \colorbox{red!0}{\strut one} \colorbox{red!0}{\strut point} \colorbox{red!0}{\strut has} \colorbox{red!0}{\strut drunk} \colorbox{red!0}{\strut .} \colorbox{red!0}{\strut vodka.Lights} \colorbox{red!0}{\strut ,} \colorbox{red!0}{\strut Camera} \colorbox{red!0}{\strut ,} \colorbox{red!0}{\strut CocktailsBrody} \colorbox{red!0}{\strut BrownOctober} \colorbox{red!0}{\strut 29} \colorbox{red!0}{\strut ,} \colorbox{red!0}{\strut 2011Can} \colorbox{red!0}{\strut we} \colorbox{red!13}{\strut generalize} \colorbox{red!0}{\strut about} 
}}}
\end{CJK*}

query: what in skin care is linked to thyroid problems

\begin{CJK*}{UTF8}{gbsn}
{\setlength{\fboxsep}{0pt}\colorbox{white!0}{\parbox{0.9\textwidth}{
\colorbox{red!0}{\strut Thyroid} \colorbox{red!0}{\strut Health} \colorbox{red!0}{\strut Solutions} \colorbox{red!0}{\strut .} \colorbox{red!0}{\strut 7} \colorbox{red!1}{\strut Reasons} \colorbox{red!0}{\strut To} \colorbox{red!2}{\strut Ditch} \colorbox{red!5}{\strut Toxic} \colorbox{red!13}{\strut Dryer} \colorbox{red!12}{\strut Sheets} \colorbox{red!0}{\strut Thyroid} \colorbox{red!0}{\strut Health} \colorbox{red!0}{\strut Solutions} \colorbox{red!0}{\strut .} \colorbox{red!0}{\strut 7} \colorbox{red!1}{\strut Reasons} \colorbox{red!0}{\strut To} \colorbox{red!2}{\strut Ditch} \colorbox{red!5}{\strut Toxic} \colorbox{red!13}{\strut Dryer} \colorbox{red!0}{\strut SheetsBy} \colorbox{red!0}{\strut kim} \colorbox{red!0}{\strut ,} \colorbox{red!0}{\strut on} \colorbox{red!0}{\strut April} \colorbox{red!0}{\strut 16th} \colorbox{red!0}{\strut ,} \colorbox{red!0}{\strut 2014} \colorbox{red!0}{\strut .} \colorbox{red!0}{\strut Freshly} \colorbox{red!0}{\strut dried} \colorbox{red!0}{\strut ,} \colorbox{red!0}{\strut awesomely} \colorbox{red!0}{\strut clean} \colorbox{red!0}{\strut and} \colorbox{red!0}{\strut nice} \colorbox{red!0}{\strut smelling} \colorbox{red!0}{\strut clothes} \colorbox{red!0}{\strut are} \colorbox{red!0}{\strut lovely} \colorbox{red!0}{\strut .} \colorbox{red!0}{\strut Yea} \colorbox{red!0}{\strut !} \colorbox{red!0}{\strut And} \colorbox{red!0}{\strut ,} \colorbox{red!0}{\strut making} \colorbox{red!0}{\strut these} \colorbox{red!0}{\strut lovely} \colorbox{red!0}{\strut fresh} \colorbox{red!0}{\strut washed} \colorbox{red!0}{\strut and} \colorbox{red!0}{\strut dried} \colorbox{red!0}{\strut clothes} \colorbox{red!0}{\strut reeeeeaaally} \colorbox{red!0}{\strut soft} \colorbox{red!0}{\strut to} \colorbox{red!0}{\strut our} \colorbox{red!0}{\strut skin} \colorbox{red!0}{\strut is} \colorbox{red!0}{\strut great} \colorbox{red!0}{\strut !} \colorbox{red!2}{\strut What} \colorbox{red!0}{\strut do} \colorbox{red!0}{\strut you} \colorbox{red!0}{\strut use} \colorbox{red!0}{\strut to} \colorbox{red!0}{\strut accomplish} \colorbox{red!0}{\strut the} \colorbox{red!0}{\strut softening} \colorbox{red!0}{\strut effect} \colorbox{red!0}{\strut .} \colorbox{red!0}{\strut in} \colorbox{red!0}{\strut the} \colorbox{red!2}{\strut washer} \colorbox{red!0}{\strut or} \colorbox{red!0}{\strut the} \colorbox{red!13}{\strut dryer} \colorbox{red!0}{\strut ?} \colorbox{red!0}{\strut In} \colorbox{red!0}{\strut the} \colorbox{red!13}{\strut dryer} \colorbox{red!0}{\strut ,} \colorbox{red!0}{\strut probably} \colorbox{red!13}{\strut dryer} \colorbox{red!12}{\strut sheets} \colorbox{red!0}{\strut ,} \colorbox{red!0}{\strut right} \colorbox{red!0}{\strut ?} \colorbox{red!0}{\strut THE} \colorbox{red!0}{\strut BAD} \colorbox{red!0}{\strut .} \colorbox{red!0}{\strut .} \colorbox{red!0}{\strut .} \colorbox{red!0}{\strut .} \colorbox{red!0}{\strut Read} \colorbox{red!0}{\strut More} \colorbox{red!0}{\strut .} \colorbox{red!0}{\strut Thyroid} \colorbox{red!0}{\strut Health} \colorbox{red!0}{\strut Solutions} \colorbox{red!0}{\strut .} \colorbox{red!0}{\strut 7} \colorbox{red!1}{\strut Reasons} \colorbox{red!0}{\strut To} \colorbox{red!2}{\strut Ditch} \colorbox{red!5}{\strut Toxic} \colorbox{red!13}{\strut Dryer} \colorbox{red!0}{\strut SheetsLeave} \colorbox{red!0}{\strut a} \colorbox{red!0}{\strut comment} \colorbox{red!0}{\strut Nervous} \colorbox{red!0}{\strut System} \colorbox{red!0}{\strut ,} \colorbox{red!0}{\strut Thyroid} \colorbox{red!0}{\strut ,} \colorbox{red!0}{\strut Thyroid} \colorbox{red!0}{\strut and} \colorbox{red!0}{\strut Skin} \colorbox{red!0}{\strut Care} \colorbox{red!0}{\strut ,} \colorbox{red!0}{\strut Thyroid} \colorbox{red!0}{\strut Problems} \colorbox{red!0}{\strut ,} \colorbox{red!2}{\strut Toxins} \colorbox{red!0}{\strut healthy} \colorbox{red!0}{\strut lifestyle} \colorbox{red!0}{\strut ,} \colorbox{red!0}{\strut the} \colorbox{red!0}{\strut bad} \colorbox{red!0}{\strut news} \colorbox{red!0}{\strut about} \colorbox{red!13}{\strut dryer} \colorbox{red!12}{\strut sheets} \colorbox{red!0}{\strut and} \colorbox{red!0}{\strut your} \colorbox{red!0}{\strut thyroid} \colorbox{red!0}{\strut health} \colorbox{red!0}{\strut ,} \colorbox{red!0}{\strut thyroid} \colorbox{red!0}{\strut problems} \colorbox{red!0}{\strut ,} \colorbox{red!0}{\strut thyroid} \colorbox{red!1}{\strut symptoms} \colorbox{red!0}{\strut ,} \colorbox{red!0}{\strut toxinsThyroid} \colorbox{red!0}{\strut Health} \colorbox{red!0}{\strut .} \colorbox{red!1}{\strut Avoid} \colorbox{red!5}{\strut Toxic} \colorbox{red!3}{\strut Deodorants} \colorbox{red!0}{\strut By} \colorbox{red!0}{\strut Switching} \colorbox{red!0}{\strut to} \colorbox{red!0}{\strut Limes} \colorbox{red!0}{\strut and} \colorbox{red!0}{\strut Lemons} \colorbox{red!0}{\strut !} \colorbox{red!0}{\strut By} \colorbox{red!0}{\strut kim} \colorbox{red!0}{\strut ,} \colorbox{red!0}{\strut on} \colorbox{red!0}{\strut July} \colorbox{red!0}{\strut 7th} \colorbox{red!0}{\strut ,} \colorbox{red!0}{\strut 2013} \colorbox{red!0}{\strut .} \colorbox{red!0}{\strut Thyroid} \colorbox{red!0}{\strut health} \colorbox{red!0}{\strut depends} \colorbox{red!0}{\strut on} \colorbox{red!0}{\strut a} \colorbox{red!0}{\strut multitude} \colorbox{red!0}{\strut of} \colorbox{red!0}{\strut things} \colorbox{red!0}{\strut ,} \colorbox{red!0}{\strut one} \colorbox{red!0}{\strut of} \colorbox{red!0}{\strut which} \colorbox{red!0}{\strut is} \colorbox{red!0}{\strut not} \colorbox{red!0}{\strut adding} \colorbox{red!0}{\strut more} \colorbox{red!2}{\strut toxins} \colorbox{red!0}{\strut to} \colorbox{red!0}{\strut your} \colorbox{red!0}{\strut skin} \colorbox{red!0}{\strut than} \colorbox{red!0}{\strut pollutants} \colorbox{red!0}{\strut that} \colorbox{red!0}{\strut you} \colorbox{red!0}{\strut can} \colorbox{red!0}{\strut .} \colorbox{red!0}{\strut t} \colorbox{red!0}{\strut escape} \colorbox{red!0}{\strut .} \colorbox{red!0}{\strut like} \colorbox{red!0}{\strut air} \colorbox{red!0}{\strut pollutions} \colorbox{red!0}{\strut ,} \colorbox{red!0}{\strut smoke} \colorbox{red!0}{\strut ,} \colorbox{red!0}{\strut etc} \colorbox{red!0}{\strut .} \colorbox{red!0}{\strut .} \colorbox{red!0}{\strut already} \colorbox{red!0}{\strut add} \colorbox{red!0}{\strut .} \colorbox{red!0}{\strut Right} \colorbox{red!0}{\strut up} \colorbox{red!0}{\strut there} \colorbox{red!0}{\strut with} \colorbox{red!0}{\strut make} \colorbox{red!0}{\strut up} \colorbox{red!0}{\strut and} \colorbox{red!0}{\strut lotions} \colorbox{red!0}{\strut is} \colorbox{red!0}{\strut deodorant.It} \colorbox{red!0}{\strut .} \colorbox{red!0}{\strut s} \colorbox{red!0}{\strut great} \colorbox{red!0}{\strut to} \colorbox{red!0}{\strut feel} \colorbox{red!0}{\strut free} \colorbox{red!0}{\strut to} \colorbox{red!0}{\strut raise} \colorbox{red!0}{\strut your} \colorbox{red!0}{\strut sleeveless} \colorbox{red!0}{\strut arms} \colorbox{red!0}{\strut in} \colorbox{red!0}{\strut public} \colorbox{red!0}{\strut and} \colorbox{red!0}{\strut know} \colorbox{red!0}{\strut .} \colorbox{red!0}{\strut .} \colorbox{red!0}{\strut .} \colorbox{red!0}{\strut .} \colorbox{red!0}{\strut Read} \colorbox{red!0}{\strut More} \colorbox{red!0}{\strut .} \colorbox{red!0}{\strut Thyroid} \colorbox{red!0}{\strut Health} \colorbox{red!0}{\strut .} \colorbox{red!1}{\strut Avoid} \colorbox{red!5}{\strut Toxic} \colorbox{red!3}{\strut Deodorants} \colorbox{red!0}{\strut By} \colorbox{red!0}{\strut Switching} \colorbox{red!0}{\strut to} \colorbox{red!0}{\strut Limes} \colorbox{red!0}{\strut and} \colorbox{red!0}{\strut Lemons} \colorbox{red!0}{\strut !} \colorbox{red!0}{\strut 13} \colorbox{red!0}{\strut comments} \colorbox{red!0}{\strut Hypothyroidism} \colorbox{red!0}{\strut in} \colorbox{red!0}{\strut Women} \colorbox{red!0}{\strut ,} \colorbox{red!0}{\strut Thyroid} \colorbox{red!0}{\strut ,} \colorbox{red!0}{\strut Thyroid} \colorbox{red!0}{\strut and} \colorbox{red!0}{\strut Skin} \colorbox{red!0}{\strut Care} \colorbox{red!0}{\strut healthy} \colorbox{red!0}{\strut lifestyle} \colorbox{red!0}{\strut ,} \colorbox{red!0}{\strut lemon} \colorbox{red!3}{\strut deodorant} \colorbox{red!0}{\strut ,} \colorbox{red!0}{\strut lime} \colorbox{red!3}{\strut deodorant} \colorbox{red!0}{\strut ,} \colorbox{red!0}{\strut non-toxic} \colorbox{red!0}{\strut natural} \colorbox{red!3}{\strut deodorant} \colorbox{red!0}{\strut ,} \colorbox{red!0}{\strut toxinsThyroid} \colorbox{red!0}{\strut Health} \colorbox{red!0}{\strut .} \colorbox{red!0}{\strut The} \colorbox{red!0}{\strut Affects} \colorbox{red!0}{\strut of} \colorbox{red!0}{\strut Iron} \colorbox{red!0}{\strut on} \colorbox{red!0}{\strut Your} \colorbox{red!0}{\strut Thyroid} \colorbox{red!0}{\strut ,} \colorbox{red!0}{\strut T4} \colorbox{red!0}{\strut and} \colorbox{red!0}{\strut T3By} \colorbox{red!0}{\strut kim} \colorbox{red!0}{\strut ,} \colorbox{red!0}{\strut on} \colorbox{red!0}{\strut December} \colorbox{red!0}{\strut 21st} \colorbox{red!0}{\strut ,} \colorbox{red!0}{\strut 2012} \colorbox{red!0}{\strut .} 
}}}
\end{CJK*}

\begin{CJK*}{UTF8}{gbsn}
{\setlength{\fboxsep}{0pt}\colorbox{white!0}{\parbox{0.9\textwidth}{
\colorbox{red!6}{\strut Skin} \colorbox{red!1}{\strut Conditions} \colorbox{red!0}{\strut and} \colorbox{red!6}{\strut Thyroid} \colorbox{red!1}{\strut Health} \colorbox{red!6}{\strut Skin} \colorbox{red!1}{\strut Conditions} \colorbox{red!0}{\strut and} \colorbox{red!6}{\strut Thyroid} \colorbox{red!0}{\strut HealthPublished} \colorbox{red!0}{\strut January} \colorbox{red!0}{\strut 27} \colorbox{red!0}{\strut 2014It} \colorbox{red!0}{\strut .} \colorbox{red!0}{\strut s} \colorbox{red!0}{\strut quite} \colorbox{red!2}{\strut common} \colorbox{red!0}{\strut for} \colorbox{red!1}{\strut people} \colorbox{red!0}{\strut with} \colorbox{red!6}{\strut thyroid} \colorbox{red!0}{\strut and} \colorbox{red!1}{\strut autoimmune} \colorbox{red!6}{\strut thyroid} \colorbox{red!1}{\strut conditions} \colorbox{red!0}{\strut to} \colorbox{red!0}{\strut have} \colorbox{red!2}{\strut dry} \colorbox{red!6}{\strut skin} \colorbox{red!0}{\strut .} \colorbox{red!0}{\strut But} \colorbox{red!0}{\strut in} \colorbox{red!0}{\strut addition} \colorbox{red!0}{\strut to} \colorbox{red!2}{\strut dry} \colorbox{red!6}{\strut skin} \colorbox{red!0}{\strut ,} \colorbox{red!0}{\strut other} \colorbox{red!1}{\strut problems} \colorbox{red!0}{\strut with} \colorbox{red!0}{\strut the} \colorbox{red!6}{\strut skin} \colorbox{red!0}{\strut are} \colorbox{red!2}{\strut common} \colorbox{red!0}{\strut ,} \colorbox{red!0}{\strut such} \colorbox{red!0}{\strut as} \colorbox{red!1}{\strut acne} \colorbox{red!0}{\strut ,} \colorbox{red!0}{\strut eczema} \colorbox{red!0}{\strut ,} \colorbox{red!0}{\strut and} \colorbox{red!0}{\strut psoriasis} \colorbox{red!0}{\strut .} \colorbox{red!6}{\strut Skin} \colorbox{red!1}{\strut conditions} \colorbox{red!0}{\strut are} \colorbox{red!2}{\strut common} \colorbox{red!0}{\strut in} \colorbox{red!1}{\strut hypothyroidism} \colorbox{red!0}{\strut and} \colorbox{red!0}{\strut Hashimoto} \colorbox{red!0}{\strut .} \colorbox{red!0}{\strut s} \colorbox{red!5}{\strut Thyroiditis} \colorbox{red!0}{\strut ,} \colorbox{red!0}{\strut as} \colorbox{red!0}{\strut well} \colorbox{red!0}{\strut as} \colorbox{red!0}{\strut in} \colorbox{red!1}{\strut hyperthyroidism} \colorbox{red!0}{\strut and} \colorbox{red!1}{\strut Graves} \colorbox{red!0}{\strut .} \colorbox{red!1}{\strut Disease} \colorbox{red!0}{\strut .} \colorbox{red!0}{\strut In} \colorbox{red!0}{\strut this} \colorbox{red!0}{\strut article} \colorbox{red!0}{\strut I} \colorbox{red!0}{\strut .} \colorbox{red!0}{\strut ll} \colorbox{red!0}{\strut discuss} \colorbox{red!0}{\strut the} \colorbox{red!0}{\strut relationship} \colorbox{red!0}{\strut of} \colorbox{red!0}{\strut some} \colorbox{red!0}{\strut of} \colorbox{red!0}{\strut the} \colorbox{red!0}{\strut more} \colorbox{red!2}{\strut common} \colorbox{red!6}{\strut skin} \colorbox{red!1}{\strut conditions} \colorbox{red!0}{\strut with} \colorbox{red!6}{\strut thyroid} \colorbox{red!0}{\strut health.Dry} \colorbox{red!6}{\strut Skin} \colorbox{red!0}{\strut .} \colorbox{red!0}{\strut Although} \colorbox{red!0}{\strut some} \colorbox{red!0}{\strut of} \colorbox{red!0}{\strut my} \colorbox{red!0}{\strut patients} \colorbox{red!0}{\strut with} \colorbox{red!1}{\strut hyperthyroid} \colorbox{red!1}{\strut conditions} \colorbox{red!0}{\strut experience} \colorbox{red!2}{\strut dry} \colorbox{red!6}{\strut skin} \colorbox{red!0}{\strut ,} \colorbox{red!0}{\strut this} \colorbox{red!0}{\strut is} \colorbox{red!0}{\strut more} \colorbox{red!2}{\strut common} \colorbox{red!0}{\strut in} \colorbox{red!1}{\strut people} \colorbox{red!0}{\strut with} \colorbox{red!1}{\strut hypothyroid} \colorbox{red!1}{\strut conditions} \colorbox{red!0}{\strut .} \colorbox{red!6}{\strut Thyroid} \colorbox{red!1}{\strut hormone} \colorbox{red!0}{\strut plays} \colorbox{red!0}{\strut an} \colorbox{red!0}{\strut important} \colorbox{red!0}{\strut role} \colorbox{red!0}{\strut in} \colorbox{red!0}{\strut maintaining} \colorbox{red!0}{\strut the} \colorbox{red!1}{\strut health} \colorbox{red!0}{\strut of} \colorbox{red!0}{\strut the} \colorbox{red!6}{\strut skin} \colorbox{red!0}{\strut .} \colorbox{red!0}{\strut So} \colorbox{red!0}{\strut as} \colorbox{red!0}{\strut the} \colorbox{red!6}{\strut thyroid} \colorbox{red!1}{\strut hormone} \colorbox{red!0}{\strut levels} \colorbox{red!0}{\strut begin} \colorbox{red!0}{\strut to} \colorbox{red!0}{\strut decrease} \colorbox{red!0}{\strut ,} \colorbox{red!0}{\strut the} \colorbox{red!0}{\strut integrity} \colorbox{red!0}{\strut of} \colorbox{red!0}{\strut the} \colorbox{red!6}{\strut skin} \colorbox{red!0}{\strut will} \colorbox{red!0}{\strut be} \colorbox{red!1}{\strut affected} \colorbox{red!0}{\strut .} \colorbox{red!0}{\strut As} \colorbox{red!0}{\strut a} \colorbox{red!0}{\strut result} \colorbox{red!0}{\strut ,} \colorbox{red!0}{\strut with} \colorbox{red!1}{\strut hypothyroidism} \colorbox{red!0}{\strut and} \colorbox{red!0}{\strut Hashimoto} \colorbox{red!0}{\strut .} \colorbox{red!0}{\strut s} \colorbox{red!5}{\strut Thyroiditis} \colorbox{red!0}{\strut ,} \colorbox{red!0}{\strut balancing} \colorbox{red!0}{\strut the} \colorbox{red!6}{\strut thyroid} \colorbox{red!1}{\strut hormone} \colorbox{red!0}{\strut levels} \colorbox{red!0}{\strut usually} \colorbox{red!0}{\strut will} \colorbox{red!1}{\strut help} \colorbox{red!0}{\strut with} \colorbox{red!2}{\strut dry} \colorbox{red!0}{\strut skin.When} \colorbox{red!0}{\strut someone} \colorbox{red!0}{\strut with} \colorbox{red!1}{\strut Graves} \colorbox{red!0}{\strut .} \colorbox{red!1}{\strut Disease} \colorbox{red!0}{\strut has} \colorbox{red!2}{\strut dry} \colorbox{red!6}{\strut skin} \colorbox{red!0}{\strut ,} \colorbox{red!0}{\strut this} \colorbox{red!0}{\strut typically} \colorbox{red!0}{\strut is} \colorbox{red!0}{\strut due} \colorbox{red!0}{\strut to} \colorbox{red!0}{\strut the} \colorbox{red!1}{\strut autoimmune} \colorbox{red!0}{\strut component} \colorbox{red!0}{\strut of} \colorbox{red!0}{\strut the} \colorbox{red!1}{\strut condition} \colorbox{red!0}{\strut ,} \colorbox{red!0}{\strut and} \colorbox{red!0}{\strut not} \colorbox{red!0}{\strut the} \colorbox{red!0}{\strut imbalance} \colorbox{red!0}{\strut in} \colorbox{red!6}{\strut thyroid} \colorbox{red!1}{\strut hormone} \colorbox{red!0}{\strut levels} \colorbox{red!0}{\strut .} \colorbox{red!0}{\strut 1} \colorbox{red!0}{\strut .} \colorbox{red!0}{\strut .} \colorbox{red!0}{\strut But} \colorbox{red!0}{\strut many} \colorbox{red!1}{\strut people} \colorbox{red!0}{\strut with} \colorbox{red!1}{\strut hyperthyroid} \colorbox{red!1}{\strut conditions} \colorbox{red!0}{\strut have} \colorbox{red!0}{\strut the} \colorbox{red!0}{\strut opposite} \colorbox{red!0}{\strut problem} \colorbox{red!0}{\strut ,} \colorbox{red!0}{\strut as} \colorbox{red!0}{\strut their} \colorbox{red!6}{\strut skin} \colorbox{red!0}{\strut might} \colorbox{red!0}{\strut appear} \colorbox{red!0}{\strut to} \colorbox{red!0}{\strut be} \colorbox{red!0}{\strut more} \colorbox{red!0}{\strut moist} \colorbox{red!0}{\strut due} \colorbox{red!0}{\strut to} \colorbox{red!0}{\strut the} \colorbox{red!0}{\strut excessive} \colorbox{red!0}{\strut sweating} \colorbox{red!0}{\strut .} \colorbox{red!0}{\strut hyperhydrosis} \colorbox{red!0}{\strut .} \colorbox{red!0}{\strut which} \colorbox{red!0}{\strut of} \colorbox{red!0}{\strut course} \colorbox{red!0}{\strut is} \colorbox{red!0}{\strut a} \colorbox{red!0}{\strut result} \colorbox{red!0}{\strut of} \colorbox{red!0}{\strut the} \colorbox{red!0}{\strut increase} \colorbox{red!0}{\strut in} \colorbox{red!0}{\strut metabolism} \colorbox{red!0}{\strut .} \colorbox{red!0}{\strut In} \colorbox{red!0}{\strut most} \colorbox{red!0}{\strut cases} \colorbox{red!0}{\strut ,} \colorbox{red!0}{\strut addressing} \colorbox{red!0}{\strut the} \colorbox{red!1}{\strut autoimmune} \colorbox{red!0}{\strut component} \colorbox{red!0}{\strut is} \colorbox{red!0}{\strut the} \colorbox{red!0}{\strut key} \colorbox{red!0}{\strut in} \colorbox{red!1}{\strut helping} \colorbox{red!0}{\strut someone} \colorbox{red!0}{\strut with} \colorbox{red!1}{\strut Graves} \colorbox{red!0}{\strut .} \colorbox{red!1}{\strut Disease} \colorbox{red!0}{\strut who} \colorbox{red!0}{\strut has} \colorbox{red!6}{\strut skin} \colorbox{red!0}{\strut problems.Acne} \colorbox{red!0}{\strut .} \colorbox{red!1}{\strut Acne} \colorbox{red!0}{\strut vulgaris} \colorbox{red!0}{\strut is} \colorbox{red!0}{\strut the} \colorbox{red!0}{\strut most} \colorbox{red!2}{\strut common} \colorbox{red!6}{\strut skin} \colorbox{red!1}{\strut disorder} \colorbox{red!0}{\strut .} \colorbox{red!0}{\strut Conventional} \colorbox{red!1}{\strut medical} \colorbox{red!1}{\strut treatment} \colorbox{red!0}{\strut involves} \colorbox{red!0}{\strut topical} \colorbox{red!0}{\strut retinoids} \colorbox{red!0}{\strut ,} \colorbox{red!0}{\strut topical} \colorbox{red!0}{\strut antimicrobials} \colorbox{red!0}{\strut ,} \colorbox{red!0}{\strut azelaic} \colorbox{red!0}{\strut acid} \colorbox{red!0}{\strut ,} \colorbox{red!0}{\strut oral} \colorbox{red!0}{\strut antibiotics} \colorbox{red!0}{\strut ,} \colorbox{red!0}{\strut and} \colorbox{red!0}{\strut hormonal} \colorbox{red!0}{\strut therapies} 
}}}
\end{CJK*}

query: highest dose of glimepiride

\begin{CJK*}{UTF8}{gbsn}
{\setlength{\fboxsep}{0pt}\colorbox{white!0}{\parbox{0.9\textwidth}{
\colorbox{red!0}{\strut Glimepiride} \colorbox{red!0}{\strut Dosing} \colorbox{red!40}{\strut Endocrine} \colorbox{red!32}{\strut System} \colorbox{red!0}{\strut ChannelTopicsAcromegalyAddison} \colorbox{red!0}{\strut s} \colorbox{red!0}{\strut DiseaseAddisonian} \colorbox{red!0}{\strut CrisisAdrenal} \colorbox{red!0}{\strut InsufficiencyCortisolCushing} \colorbox{red!0}{\strut s} \colorbox{red!0}{\strut DiseaseCushing} \colorbox{red!0}{\strut s} \colorbox{red!0}{\strut SyndromeEmpty} \colorbox{red!0}{\strut Sella} \colorbox{red!0}{\strut SyndromeHigh} \colorbox{red!8}{\strut Prolactin} \colorbox{red!0}{\strut LevelsHyperthyroidismHypothyroidismPituitary} \colorbox{red!0}{\strut AdenomaPituitary} \colorbox{red!0}{\strut MacroadenomaPituitary} \colorbox{red!0}{\strut MicroadenomaPituitary} \colorbox{red!0}{\strut TumorProlactinomaMedicationsAcarboseActoplus} \colorbox{red!0}{\strut Met} \colorbox{red!0}{\strut XRAlogliptinAlogliptin} \colorbox{red!0}{\strut and} \colorbox{red!0}{\strut MetforminAlogliptin} \colorbox{red!0}{\strut and} \colorbox{red!0}{\strut PioglitazoneArmour} \colorbox{red!0}{\strut ThyroidCanagliflozinCytomelExenatideExtended-Release} \colorbox{red!0}{\strut ExenatideGlimepirideGlipizide} \colorbox{red!0}{\strut and} \colorbox{red!0}{\strut MetforminGlucaGenGlucophageGlucophage} \colorbox{red!0}{\strut XRGlucotrolGlyburide} \colorbox{red!0}{\strut and} \colorbox{red!0}{\strut MetforminHumalog} \colorbox{red!0}{\strut Mix7525Inhaled} \colorbox{red!0}{\strut InsulinInsulin} \colorbox{red!0}{\strut AspartInsulin} \colorbox{red!0}{\strut DetemirInsulin} \colorbox{red!0}{\strut GlargineInsulin} \colorbox{red!0}{\strut GlulisineInsulin} \colorbox{red!0}{\strut LisproInsulin} \colorbox{red!0}{\strut Lispro} \colorbox{red!0}{\strut ProtamineInsulin} \colorbox{red!0}{\strut LisproJanumetKorlymLevothyroxineLinagliptinLinagliptinMetforminLiraglutideMethimazoleMetoclopramideNateglinideNovolin} \colorbox{red!0}{\strut NNovoLog} \colorbox{red!0}{\strut Mix} \colorbox{red!0}{\strut 7030NPH} \colorbox{red!0}{\strut InsulinRegular} \colorbox{red!0}{\strut InsulinPioglitazonePioglitazone} \colorbox{red!0}{\strut and} \colorbox{red!0}{\strut GlimepiridePioglitazone} \colorbox{red!0}{\strut and} \colorbox{red!0}{\strut MetforminPramlintidePropylthiouracilRegular} \colorbox{red!0}{\strut InsulinRepaglinideRepaglinide} \colorbox{red!0}{\strut and} \colorbox{red!0}{\strut MetforminRosiglitazoneRosiglitazone} \colorbox{red!0}{\strut and} \colorbox{red!0}{\strut GlimepirideRosiglitazone} \colorbox{red!0}{\strut and} \colorbox{red!0}{\strut MetforminSaxagliptinSaxagliptinMetformin} \colorbox{red!0}{\strut ERSitagliptinSitagliptin} \colorbox{red!0}{\strut and} \colorbox{red!32}{\strut Metformin} \colorbox{red!0}{\strut Extended-ReleaseSynthroidTestosterone} \colorbox{red!0}{\strut Topical} \colorbox{red!0}{\strut SolutionTirosintWesthroidAdvertisementQuicklinksCushing} \colorbox{red!0}{\strut s} \colorbox{red!0}{\strut DiseaseAddison} \colorbox{red!0}{\strut s} \colorbox{red!0}{\strut DiseaseAcromegalyProlactinomaAdrenal} \colorbox{red!0}{\strut InsufficiencyPituitary} \colorbox{red!0}{\strut TumorEmpty} \colorbox{red!0}{\strut Sella} \colorbox{red!0}{\strut SyndromeGlucophageExenatideSynthroidLevothyroxineCytomelMetoclopramideHypothyroidismHypothyroidism} \colorbox{red!0}{\strut DietHyperthyroidismRelated} \colorbox{red!0}{\strut ChannelsDiabetesDepressionHeart} \colorbox{red!0}{\strut DiseaseBlood} \colorbox{red!0}{\strut PressureCholesterolAdvertisementTweetEndocrine} \colorbox{red!32}{\strut System} \colorbox{red!0}{\strut Home} \colorbox{red!0}{\strut .} \colorbox{red!0}{\strut Glimepiride} \colorbox{red!0}{\strut DosingGlimepiride} \colorbox{red!0}{\strut DosingThe} \colorbox{red!0}{\strut recommended} \colorbox{red!0}{\strut starting} \colorbox{red!0}{\strut glimepiride} \colorbox{red!0}{\strut dose} \colorbox{red!0}{\strut is} \colorbox{red!0}{\strut generally} \colorbox{red!0}{\strut 1} \colorbox{red!0}{\strut mg} \colorbox{red!0}{\strut or} \colorbox{red!0}{\strut 2} \colorbox{red!0}{\strut mg} \colorbox{red!0}{\strut once} \colorbox{red!0}{\strut a} \colorbox{red!0}{\strut day} \colorbox{red!0}{\strut .} \colorbox{red!0}{\strut Your} \colorbox{red!0}{\strut healthcare} \colorbox{red!0}{\strut provider} \colorbox{red!0}{\strut will} \colorbox{red!0}{\strut determine} \colorbox{red!0}{\strut your} \colorbox{red!0}{\strut glimepiride} \colorbox{red!0}{\strut dosing} \colorbox{red!0}{\strut guidelines} \colorbox{red!0}{\strut based} \colorbox{red!0}{\strut on} \colorbox{red!0}{\strut a} \colorbox{red!0}{\strut number} \colorbox{red!0}{\strut of} \colorbox{red!0}{\strut factors} \colorbox{red!0}{\strut ,} \colorbox{red!0}{\strut such} \colorbox{red!0}{\strut as} \colorbox{red!0}{\strut your} \colorbox{red!0}{\strut age} \colorbox{red!0}{\strut ,} \colorbox{red!0}{\strut other} \colorbox{red!0}{\strut medical} \colorbox{red!0}{\strut conditions} \colorbox{red!0}{\strut you} \colorbox{red!0}{\strut may} \colorbox{red!0}{\strut have} \colorbox{red!0}{\strut ,} \colorbox{red!0}{\strut and} \colorbox{red!0}{\strut other} \colorbox{red!0}{\strut medications} \colorbox{red!0}{\strut you} \colorbox{red!0}{\strut may} \colorbox{red!0}{\strut be} \colorbox{red!0}{\strut taking} \colorbox{red!0}{\strut .} \colorbox{red!0}{\strut Glimepiride} \colorbox{red!0}{\strut is} \colorbox{red!0}{\strut usually} \colorbox{red!0}{\strut started} \colorbox{red!0}{\strut at} \colorbox{red!0}{\strut a} \colorbox{red!0}{\strut lower} \colorbox{red!0}{\strut dose} \colorbox{red!0}{\strut and} \colorbox{red!0}{\strut then} \colorbox{red!0}{\strut slowly} \colorbox{red!0}{\strut increased} \colorbox{red!0}{\strut every} \colorbox{red!0}{\strut one} \colorbox{red!0}{\strut to} \colorbox{red!0}{\strut two} \colorbox{red!0}{\strut weeks} \colorbox{red!0}{\strut if} \colorbox{red!0}{\strut necessary} \colorbox{red!0}{\strut .} \colorbox{red!0}{\strut The} \colorbox{red!0}{\strut medication} \colorbox{red!0}{\strut can} \colorbox{red!0}{\strut also} \colorbox{red!0}{\strut be} \colorbox{red!0}{\strut used} \colorbox{red!0}{\strut in} \colorbox{red!0}{\strut combination} \colorbox{red!0}{\strut with} \colorbox{red!56}{\strut insulin} \colorbox{red!0}{\strut injections.Your} \colorbox{red!0}{\strut Guide} \colorbox{red!0}{\strut to} \colorbox{red!0}{\strut Healthy} \colorbox{red!0}{\strut Living} \colorbox{red!0}{\strut With} \colorbox{red!0}{\strut DiabetesGet} \colorbox{red!0}{\strut tips} \colorbox{red!0}{\strut ,} \colorbox{red!0}{\strut read} \colorbox{red!0}{\strut articles} \colorbox{red!0}{\strut ,} \colorbox{red!0}{\strut and} \colorbox{red!0}{\strut learn} \colorbox{red!0}{\strut about} \colorbox{red!0}{\strut healthy} \colorbox{red!0}{\strut living} \colorbox{red!0}{\strut with} \colorbox{red!0}{\strut diabetes} \colorbox{red!0}{\strut ,} \colorbox{red!0}{\strut in-depth} \colorbox{red!0}{\strut ,} \colorbox{red!0}{\strut from} \colorbox{red!0}{\strut eMedTV} \colorbox{red!0}{\strut s} \colorbox{red!0}{\strut experts.Click} \colorbox{red!0}{\strut here} \colorbox{red!0}{\strut to} \colorbox{red!0}{\strut learn} \colorbox{red!0}{\strut more} \colorbox{red!0}{\strut .} \colorbox{red!0}{\strut An} \colorbox{red!0}{\strut Overview} \colorbox{red!0}{\strut of} \colorbox{red!0}{\strut Glimepiride} \colorbox{red!0}{\strut DosingThe} \colorbox{red!0}{\strut dose} \colorbox{red!0}{\strut of} \colorbox{red!0}{\strut glimepiride} \colorbox{red!0}{\strut .} \colorbox{red!0}{\strut Amaryl} \colorbox{red!0}{\strut .} \colorbox{red!0}{\strut .} \colorbox{red!0}{\strut your} \colorbox{red!0}{\strut healthcare} \colorbox{red!0}{\strut provider} \colorbox{red!0}{\strut prescribes} \colorbox{red!0}{\strut will} \colorbox{red!0}{\strut vary} \colorbox{red!0}{\strut depending} \colorbox{red!0}{\strut on} \colorbox{red!0}{\strut a} \colorbox{red!0}{\strut number} \colorbox{red!0}{\strut of} \colorbox{red!0}{\strut factors} \colorbox{red!0}{\strut ,} \colorbox{red!0}{\strut including} \colorbox{red!0}{\strut .} \colorbox{red!0}{\strut Your} \colorbox{red!0}{\strut ageOther} \colorbox{red!0}{\strut medical} \colorbox{red!0}{\strut conditions} \colorbox{red!0}{\strut you} \colorbox{red!0}{\strut may} \colorbox{red!0}{\strut haveOther} \colorbox{red!0}{\strut medications} \colorbox{red!0}{\strut you} \colorbox{red!0}{\strut may} \colorbox{red!0}{\strut currently} \colorbox{red!0}{\strut be} \colorbox{red!0}{\strut taking.As} \colorbox{red!0}{\strut is} \colorbox{red!0}{\strut always} \colorbox{red!0}{\strut the} \colorbox{red!0}{\strut case} \colorbox{red!0}{\strut ,} \colorbox{red!0}{\strut do} \colorbox{red!0}{\strut not} \colorbox{red!0}{\strut adjust} \colorbox{red!0}{\strut your} \colorbox{red!0}{\strut dose} \colorbox{red!0}{\strut unless} \colorbox{red!0}{\strut your} \colorbox{red!0}{\strut healthcare} \colorbox{red!0}{\strut provider} \colorbox{red!0}{\strut specifically} \colorbox{red!0}{\strut instructs} \colorbox{red!0}{\strut you} \colorbox{red!0}{\strut to} \colorbox{red!0}{\strut do} \colorbox{red!0}{\strut so.Glimepiride} \colorbox{red!0}{\strut Dosage} \colorbox{red!0}{\strut for} \colorbox{red!0}{\strut Type} \colorbox{red!0}{\strut 2} \colorbox{red!0}{\strut DiabetesGlimepiride} \colorbox{red!0}{\strut is} \colorbox{red!0}{\strut usually} \colorbox{red!0}{\strut started} \colorbox{red!0}{\strut at} \colorbox{red!0}{\strut a} \colorbox{red!0}{\strut low} \colorbox{red!0}{\strut dose} \colorbox{red!0}{\strut and} \colorbox{red!0}{\strut increased} \colorbox{red!0}{\strut slowly} \colorbox{red!0}{\strut ,} \colorbox{red!0}{\strut with} \colorbox{red!0}{\strut the} \colorbox{red!0}{\strut following} \colorbox{red!0}{\strut instructions} \colorbox{red!0}{\strut .} \colorbox{red!0}{\strut The} \colorbox{red!0}{\strut recommended} \colorbox{red!0}{\strut starting} \colorbox{red!0}{\strut does} \colorbox{red!0}{\strut is} \colorbox{red!0}{\strut glimepiride} \colorbox{red!0}{\strut 1} \colorbox{red!0}{\strut mg} \colorbox{red!0}{\strut or} \colorbox{red!0}{\strut glimepiride} \colorbox{red!0}{\strut 2} \colorbox{red!0}{\strut mg} \colorbox{red!0}{\strut once} \colorbox{red!0}{\strut a} \colorbox{red!0}{\strut day.The} \colorbox{red!0}{\strut recommended} \colorbox{red!0}{\strut starting} \colorbox{red!0}{\strut dose} \colorbox{red!0}{\strut for} \colorbox{red!0}{\strut elderly} \colorbox{red!0}{\strut people} \colorbox{red!0}{\strut and} \colorbox{red!0}{\strut people} 
}}}
\end{CJK*}

\begin{CJK*}{UTF8}{gbsn}
{\setlength{\fboxsep}{0pt}\colorbox{white!0}{\parbox{0.9\textwidth}{
\colorbox{red!28}{\strut Glimepiride} \colorbox{red!0}{\strut GlimepirideDosage} \colorbox{red!0}{\strut Form} \colorbox{red!0}{\strut .} \colorbox{red!0}{\strut tabletOverview} \colorbox{red!6}{\strut Side} \colorbox{red!4}{\strut Effects} \colorbox{red!6}{\strut Dosage} \colorbox{red!0}{\strut Professional} \colorbox{red!0}{\strut Tips} \colorbox{red!0}{\strut Interactions} \colorbox{red!3}{\strut Pregnancy} \colorbox{red!0}{\strut WarningsMoreBreastfeeding} \colorbox{red!0}{\strut WarningsUser} \colorbox{red!0}{\strut ReviewsDrug} \colorbox{red!0}{\strut ImagesSupport} \colorbox{red!0}{\strut Group} \colorbox{red!0}{\strut Q} \colorbox{red!0}{\strut .} \colorbox{red!0}{\strut APricing} \colorbox{red!0}{\strut .} \colorbox{red!0}{\strut CouponsOn} \colorbox{red!0}{\strut This} \colorbox{red!0}{\strut PageIndications} \colorbox{red!0}{\strut and} \colorbox{red!0}{\strut UsageDosage} \colorbox{red!0}{\strut and} \colorbox{red!0}{\strut AdministrationDosage} \colorbox{red!0}{\strut Forms} \colorbox{red!0}{\strut and} \colorbox{red!0}{\strut StrengthsContraindicationsWarnings} \colorbox{red!0}{\strut and} \colorbox{red!0}{\strut PrecautionsAdverse} \colorbox{red!0}{\strut ReactionsDrug} \colorbox{red!0}{\strut InteractionsUse} \colorbox{red!0}{\strut In} \colorbox{red!0}{\strut Specific} \colorbox{red!0}{\strut PopulationsOverdosageDescriptionClinical} \colorbox{red!0}{\strut PharmacologyNonclinical} \colorbox{red!0}{\strut ToxicologyClinical} \colorbox{red!0}{\strut StudiesHow} \colorbox{red!0}{\strut SuppliedStorage} \colorbox{red!0}{\strut and} \colorbox{red!0}{\strut HandlingPatient} \colorbox{red!0}{\strut Counseling} \colorbox{red!0}{\strut InformationOn} \colorbox{red!0}{\strut This} \colorbox{red!0}{\strut PageIndications} \colorbox{red!0}{\strut and} \colorbox{red!0}{\strut UsageDosage} \colorbox{red!0}{\strut and} \colorbox{red!0}{\strut AdministrationDosage} \colorbox{red!0}{\strut Forms} \colorbox{red!0}{\strut and} \colorbox{red!0}{\strut StrengthsContraindicationsWarnings} \colorbox{red!0}{\strut and} \colorbox{red!0}{\strut PrecautionsAdverse} \colorbox{red!0}{\strut ReactionsDrug} \colorbox{red!0}{\strut InteractionsUse} \colorbox{red!0}{\strut In} \colorbox{red!0}{\strut Specific} \colorbox{red!0}{\strut PopulationsOverdosageDescriptionClinical} \colorbox{red!0}{\strut PharmacologyNonclinical} \colorbox{red!0}{\strut ToxicologyClinical} \colorbox{red!0}{\strut StudiesHow} \colorbox{red!0}{\strut SuppliedStorage} \colorbox{red!0}{\strut and} \colorbox{red!0}{\strut HandlingPatient} \colorbox{red!0}{\strut Counseling} \colorbox{red!0}{\strut InformationIndications} \colorbox{red!0}{\strut and} \colorbox{red!3}{\strut Usage} \colorbox{red!0}{\strut for} \colorbox{red!0}{\strut GlimepirideGlimepiride} \colorbox{red!3}{\strut tablets} \colorbox{red!0}{\strut are} \colorbox{red!3}{\strut indicated} \colorbox{red!0}{\strut as} \colorbox{red!0}{\strut an} \colorbox{red!0}{\strut adjunct} \colorbox{red!0}{\strut to} \colorbox{red!0}{\strut diet} \colorbox{red!0}{\strut and} \colorbox{red!0}{\strut exercise} \colorbox{red!0}{\strut to} \colorbox{red!0}{\strut improve} \colorbox{red!6}{\strut glycemic} \colorbox{red!0}{\strut control} \colorbox{red!0}{\strut in} \colorbox{red!0}{\strut adults} \colorbox{red!0}{\strut with} \colorbox{red!0}{\strut type} \colorbox{red!0}{\strut 2} \colorbox{red!3}{\strut diabetes} \colorbox{red!0}{\strut mellitus} \colorbox{red!0}{\strut .} \colorbox{red!0}{\strut see} \colorbox{red!0}{\strut Clinical} \colorbox{red!0}{\strut Studies} \colorbox{red!0}{\strut .} \colorbox{red!0}{\strut 14.1} \colorbox{red!0}{\strut .} \colorbox{red!0}{\strut .} \colorbox{red!0}{\strut .Important} \colorbox{red!0}{\strut Limitations} \colorbox{red!0}{\strut of} \colorbox{red!0}{\strut UseGlimepiride} \colorbox{red!3}{\strut tablets} \colorbox{red!0}{\strut should} \colorbox{red!0}{\strut not} \colorbox{red!0}{\strut be} \colorbox{red!0}{\strut used} \colorbox{red!0}{\strut for} \colorbox{red!0}{\strut the} \colorbox{red!3}{\strut treatment} \colorbox{red!0}{\strut of} \colorbox{red!0}{\strut type} \colorbox{red!0}{\strut 1} \colorbox{red!3}{\strut diabetes} \colorbox{red!0}{\strut mellitus} \colorbox{red!0}{\strut or} \colorbox{red!0}{\strut diabetic} \colorbox{red!0}{\strut ketoacidosis} \colorbox{red!0}{\strut ,} \colorbox{red!0}{\strut as} \colorbox{red!0}{\strut it} \colorbox{red!0}{\strut would} \colorbox{red!0}{\strut not} \colorbox{red!0}{\strut be} \colorbox{red!3}{\strut effective} \colorbox{red!0}{\strut in} \colorbox{red!0}{\strut these} \colorbox{red!0}{\strut settings.SlideshowAging} \colorbox{red!0}{\strut Issues} \colorbox{red!0}{\strut .} \colorbox{red!0}{\strut 12} \colorbox{red!0}{\strut of} \colorbox{red!0}{\strut the} \colorbox{red!0}{\strut Most} \colorbox{red!0}{\strut Common} \colorbox{red!0}{\strut Health} \colorbox{red!0}{\strut Concerns} \colorbox{red!0}{\strut Affecting} \colorbox{red!0}{\strut SeniorsGlimepiride} \colorbox{red!6}{\strut Dosage} \colorbox{red!0}{\strut and} \colorbox{red!0}{\strut AdministrationRecommended} \colorbox{red!0}{\strut DosingGlimepiride} \colorbox{red!3}{\strut tablets} \colorbox{red!0}{\strut should} \colorbox{red!0}{\strut be} \colorbox{red!0}{\strut administered} \colorbox{red!0}{\strut with} \colorbox{red!0}{\strut breakfast} \colorbox{red!0}{\strut or} \colorbox{red!0}{\strut the} \colorbox{red!0}{\strut first} \colorbox{red!0}{\strut main} \colorbox{red!0}{\strut meal} \colorbox{red!0}{\strut of} \colorbox{red!0}{\strut the} \colorbox{red!0}{\strut day.The} \colorbox{red!5}{\strut recommended} \colorbox{red!3}{\strut starting} \colorbox{red!13}{\strut dose} \colorbox{red!0}{\strut of} \colorbox{red!28}{\strut Glimepiride} \colorbox{red!3}{\strut tablets} \colorbox{red!0}{\strut is} \colorbox{red!0}{\strut 1} \colorbox{red!0}{\strut mg} \colorbox{red!0}{\strut or} \colorbox{red!0}{\strut 2} \colorbox{red!0}{\strut mg} \colorbox{red!0}{\strut once} \colorbox{red!4}{\strut daily} \colorbox{red!0}{\strut .} \colorbox{red!0}{\strut Patients} \colorbox{red!0}{\strut at} \colorbox{red!0}{\strut increased} \colorbox{red!0}{\strut risk} \colorbox{red!0}{\strut for} \colorbox{red!0}{\strut hypoglycemia} \colorbox{red!0}{\strut .} \colorbox{red!0}{\strut e.g.} \colorbox{red!0}{\strut ,} \colorbox{red!0}{\strut the} \colorbox{red!0}{\strut elderly} \colorbox{red!0}{\strut or} \colorbox{red!0}{\strut patients} \colorbox{red!0}{\strut with} \colorbox{red!0}{\strut renal} \colorbox{red!0}{\strut impairment} \colorbox{red!0}{\strut .} \colorbox{red!0}{\strut should} \colorbox{red!0}{\strut be} \colorbox{red!0}{\strut started} \colorbox{red!0}{\strut on} \colorbox{red!0}{\strut 1} \colorbox{red!0}{\strut mg} \colorbox{red!0}{\strut once} \colorbox{red!4}{\strut daily} \colorbox{red!0}{\strut .} \colorbox{red!0}{\strut see} \colorbox{red!0}{\strut Warnings} \colorbox{red!0}{\strut and} \colorbox{red!4}{\strut Precautions} \colorbox{red!0}{\strut .} \colorbox{red!0}{\strut 5.1} \colorbox{red!0}{\strut .} \colorbox{red!0}{\strut and} \colorbox{red!0}{\strut Use} \colorbox{red!0}{\strut in} \colorbox{red!0}{\strut Specific} \colorbox{red!0}{\strut Populations} \colorbox{red!0}{\strut .} \colorbox{red!0}{\strut 8.5} \colorbox{red!0}{\strut ,} \colorbox{red!0}{\strut 8.6} \colorbox{red!0}{\strut .} \colorbox{red!0}{\strut .} \colorbox{red!0}{\strut .After} \colorbox{red!0}{\strut reaching} \colorbox{red!0}{\strut a} \colorbox{red!4}{\strut daily} \colorbox{red!13}{\strut dose} \colorbox{red!0}{\strut of} \colorbox{red!0}{\strut 2} \colorbox{red!0}{\strut mg} \colorbox{red!0}{\strut ,} \colorbox{red!0}{\strut further} \colorbox{red!13}{\strut dose} \colorbox{red!3}{\strut increases} \colorbox{red!0}{\strut can} \colorbox{red!0}{\strut be} \colorbox{red!0}{\strut made} \colorbox{red!0}{\strut in} \colorbox{red!0}{\strut increments} \colorbox{red!0}{\strut of} \colorbox{red!0}{\strut 1} \colorbox{red!0}{\strut mg} \colorbox{red!0}{\strut or} \colorbox{red!0}{\strut 2} \colorbox{red!0}{\strut mg} \colorbox{red!0}{\strut based} \colorbox{red!0}{\strut upon} \colorbox{red!0}{\strut the} \colorbox{red!0}{\strut patient} \colorbox{red!0}{\strut .} \colorbox{red!0}{\strut s} \colorbox{red!6}{\strut glycemic} \colorbox{red!0}{\strut response} \colorbox{red!0}{\strut .} \colorbox{red!0}{\strut Uptitration} \colorbox{red!0}{\strut should} \colorbox{red!0}{\strut not} \colorbox{red!0}{\strut occur} \colorbox{red!0}{\strut more} \colorbox{red!0}{\strut frequently} \colorbox{red!0}{\strut than} \colorbox{red!0}{\strut every} \colorbox{red!0}{\strut 1} \colorbox{red!0}{\strut to} \colorbox{red!0}{\strut 2} \colorbox{red!0}{\strut weeks} \colorbox{red!0}{\strut .} \colorbox{red!0}{\strut A} \colorbox{red!0}{\strut conservative} \colorbox{red!0}{\strut titration} \colorbox{red!0}{\strut scheme} \colorbox{red!0}{\strut is} \colorbox{red!5}{\strut recommended} \colorbox{red!0}{\strut for} \colorbox{red!0}{\strut patients} \colorbox{red!0}{\strut at} \colorbox{red!0}{\strut increased} \colorbox{red!0}{\strut risk} \colorbox{red!0}{\strut for} \colorbox{red!0}{\strut hypoglycemia} \colorbox{red!0}{\strut .} \colorbox{red!0}{\strut see} \colorbox{red!0}{\strut Warnings} \colorbox{red!0}{\strut and} \colorbox{red!4}{\strut Precautions} \colorbox{red!0}{\strut .} \colorbox{red!0}{\strut 5.1} \colorbox{red!0}{\strut .} \colorbox{red!0}{\strut and} \colorbox{red!0}{\strut Use} \colorbox{red!0}{\strut in} \colorbox{red!0}{\strut Specific} \colorbox{red!0}{\strut Populations} \colorbox{red!0}{\strut .} \colorbox{red!0}{\strut 8.5} \colorbox{red!0}{\strut ,} \colorbox{red!0}{\strut 8.6} \colorbox{red!0}{\strut .} \colorbox{red!0}{\strut .} \colorbox{red!0}{\strut .The} \colorbox{red!4}{\strut maximum} 
}}}
\end{CJK*}

query: who starred in movie reckless?

\begin{CJK*}{UTF8}{gbsn}
{\setlength{\fboxsep}{0pt}\colorbox{white!0}{\parbox{0.9\textwidth}{
\colorbox{red!0}{\strut Reckless} \colorbox{red!0}{\strut 1984} \colorbox{red!0}{\strut .} \colorbox{red!0}{\strut By} \colorbox{red!0}{\strut placing} \colorbox{red!0}{\strut your} \colorbox{red!0}{\strut order} \colorbox{red!0}{\strut or} \colorbox{red!0}{\strut playing} \colorbox{red!0}{\strut a} \colorbox{red!1}{\strut video} \colorbox{red!0}{\strut ,} \colorbox{red!0}{\strut you} \colorbox{red!0}{\strut agree} \colorbox{red!0}{\strut to} \colorbox{red!0}{\strut our} \colorbox{red!0}{\strut Terms} \colorbox{red!0}{\strut of} \colorbox{red!0}{\strut Use} \colorbox{red!0}{\strut .} \colorbox{red!0}{\strut Sold} \colorbox{red!0}{\strut by} \colorbox{red!0}{\strut Amazon} \colorbox{red!0}{\strut Digital} \colorbox{red!0}{\strut Services} \colorbox{red!0}{\strut LLC} \colorbox{red!0}{\strut .} \colorbox{red!0}{\strut Additional} \colorbox{red!0}{\strut taxes} \colorbox{red!0}{\strut may} \colorbox{red!0}{\strut apply.Customers} \colorbox{red!15}{\strut who} \colorbox{red!0}{\strut watched} \colorbox{red!0}{\strut this} \colorbox{red!0}{\strut item} \colorbox{red!0}{\strut also} \colorbox{red!0}{\strut watchedFire} \colorbox{red!0}{\strut with} \colorbox{red!1}{\strut Fire} \colorbox{red!0}{\strut Thief} \colorbox{red!0}{\strut Of} \colorbox{red!0}{\strut Hearts} \colorbox{red!0}{\strut The} \colorbox{red!0}{\strut New} \colorbox{red!0}{\strut Kids} \colorbox{red!0}{\strut Tuff} \colorbox{red!0}{\strut Turf} \colorbox{red!0}{\strut Afterburn} \colorbox{red!0}{\strut Aftershock} \colorbox{red!0}{\strut Hollywood} \colorbox{red!0}{\strut Dirt} \colorbox{red!0}{\strut Blink} \colorbox{red!0}{\strut Dogfight} \colorbox{red!0}{\strut Ribbons} \colorbox{red!0}{\strut Permanent} \colorbox{red!0}{\strut Record} \colorbox{red!0}{\strut Moving} \colorbox{red!0}{\strut In} \colorbox{red!0}{\strut .} \colorbox{red!0}{\strut First} \colorbox{red!1}{\strut Born} \colorbox{red!0}{\strut .} \colorbox{red!0}{\strut The} \colorbox{red!0}{\strut Accident} \colorbox{red!0}{\strut Perfect} \colorbox{red!0}{\strut Commandments} \colorbox{red!2}{\strut Jersey} \colorbox{red!4}{\strut Girl} \colorbox{red!0}{\strut Tomboy} \colorbox{red!0}{\strut The} \colorbox{red!0}{\strut Trouble} \colorbox{red!0}{\strut With} \colorbox{red!0}{\strut Mistletoe} \colorbox{red!0}{\strut The} \colorbox{red!0}{\strut Night} \colorbox{red!0}{\strut Before} \colorbox{red!0}{\strut Vision} \colorbox{red!0}{\strut Quest} \colorbox{red!0}{\strut No} \colorbox{red!0}{\strut Small} \colorbox{red!0}{\strut AffairProduct} \colorbox{red!0}{\strut detailsGenres} \colorbox{red!0}{\strut DramaDirector} \colorbox{red!0}{\strut James} \colorbox{red!0}{\strut FoleyStarring} \colorbox{red!6}{\strut Aidan} \colorbox{red!4}{\strut Quinn} \colorbox{red!0}{\strut ,} \colorbox{red!11}{\strut Daryl} \colorbox{red!6}{\strut Hannah} \colorbox{red!0}{\strut ,} \colorbox{red!0}{\strut Kenneth} \colorbox{red!0}{\strut McmillanSupporting} \colorbox{red!2}{\strut actors} \colorbox{red!0}{\strut Cliff} \colorbox{red!0}{\strut De} \colorbox{red!0}{\strut YoungStudio} \colorbox{red!0}{\strut MGMMPAA} \colorbox{red!0}{\strut rating} \colorbox{red!0}{\strut R} \colorbox{red!0}{\strut .} \colorbox{red!0}{\strut Restricted} \colorbox{red!0}{\strut .} \colorbox{red!0}{\strut Captions} \colorbox{red!0}{\strut and} \colorbox{red!0}{\strut subtitles} \colorbox{red!0}{\strut English} \colorbox{red!0}{\strut .} \colorbox{red!0}{\strut CC} \colorbox{red!0}{\strut .} \colorbox{red!0}{\strut DetailsAudio} \colorbox{red!0}{\strut EnglishPurchase} \colorbox{red!0}{\strut rights} \colorbox{red!0}{\strut Stream} \colorbox{red!0}{\strut instantly} \colorbox{red!0}{\strut DetailsFormat} \colorbox{red!1}{\strut Prime} \colorbox{red!1}{\strut Video} \colorbox{red!0}{\strut .} \colorbox{red!0}{\strut streaming} \colorbox{red!0}{\strut online} \colorbox{red!1}{\strut video} \colorbox{red!0}{\strut .} \colorbox{red!0}{\strut Devices} \colorbox{red!0}{\strut Available} \colorbox{red!0}{\strut to} \colorbox{red!0}{\strut watch} \colorbox{red!0}{\strut on} \colorbox{red!0}{\strut supported} \colorbox{red!0}{\strut devicesOther} \colorbox{red!0}{\strut formatsDVD} \colorbox{red!0}{\strut .} \colorbox{red!0}{\strut 13.72Customer} \colorbox{red!0}{\strut Reviews4.6} \colorbox{red!0}{\strut out} \colorbox{red!0}{\strut of} \colorbox{red!0}{\strut 5} \colorbox{red!1}{\strut stars} \colorbox{red!0}{\strut 1304.6} \colorbox{red!0}{\strut out} \colorbox{red!0}{\strut of} \colorbox{red!0}{\strut 5} \colorbox{red!0}{\strut stars5} \colorbox{red!1}{\strut star} \colorbox{red!0}{\strut 72} \colorbox{red!0}{\strut .} \colorbox{red!0}{\strut 4} \colorbox{red!1}{\strut star} \colorbox{red!0}{\strut 22} \colorbox{red!0}{\strut .} \colorbox{red!0}{\strut 3} \colorbox{red!1}{\strut star} \colorbox{red!0}{\strut 5} \colorbox{red!0}{\strut .} \colorbox{red!0}{\strut 2} \colorbox{red!0}{\strut star2} \colorbox{red!1}{\strut star} \colorbox{red!0}{\strut .} \colorbox{red!0}{\strut 0} \colorbox{red!0}{\strut .} \colorbox{red!0}{\strut .} \colorbox{red!0}{\strut 0} \colorbox{red!0}{\strut .} \colorbox{red!0}{\strut 1} \colorbox{red!1}{\strut star} \colorbox{red!0}{\strut 1} \colorbox{red!0}{\strut .} \colorbox{red!0}{\strut Share} \colorbox{red!0}{\strut your} \colorbox{red!0}{\strut thoughts} \colorbox{red!0}{\strut with} \colorbox{red!0}{\strut other} \colorbox{red!0}{\strut customersWrite} \colorbox{red!0}{\strut a} \colorbox{red!0}{\strut customer} \colorbox{red!0}{\strut reviewSee} \colorbox{red!0}{\strut all} \colorbox{red!0}{\strut 130} \colorbox{red!0}{\strut customer} \colorbox{red!0}{\strut reviewsRead} \colorbox{red!0}{\strut reviews} \colorbox{red!0}{\strut that} \colorbox{red!0}{\strut mentionquinn} \colorbox{red!6}{\strut hannah} \colorbox{red!6}{\strut aidan} \colorbox{red!1}{\strut dvd} \colorbox{red!11}{\strut daryl} \colorbox{red!28}{\strut movies} \colorbox{red!0}{\strut youngschool} \colorbox{red!0}{\strut scene} \colorbox{red!0}{\strut classic} \colorbox{red!0}{\strut saw} \colorbox{red!0}{\strut soundtrack} \colorbox{red!0}{\strut johnnydance} \colorbox{red!0}{\strut early} \colorbox{red!0}{\strut teen} \colorbox{red!0}{\strut scenes} \colorbox{red!0}{\strut void} \colorbox{red!4}{\strut girl} \colorbox{red!0}{\strut rebelTop} \colorbox{red!0}{\strut customer} \colorbox{red!0}{\strut reviewsClaire4.0} \colorbox{red!0}{\strut out} \colorbox{red!0}{\strut of} \colorbox{red!0}{\strut 5} \colorbox{red!1}{\strut stars} \colorbox{red!0}{\strut Better} \colorbox{red!0}{\strut in} \colorbox{red!0}{\strut some} \colorbox{red!0}{\strut ways} \colorbox{red!0}{\strut but} \colorbox{red!0}{\strut less} \colorbox{red!0}{\strut in} \colorbox{red!0}{\strut others} \colorbox{red!0}{\strut ...} \colorbox{red!0}{\strut August} \colorbox{red!0}{\strut 24} \colorbox{red!0}{\strut ,} \colorbox{red!0}{\strut 2012Format} \colorbox{red!0}{\strut .} \colorbox{red!1}{\strut DVD} \colorbox{red!0}{\strut Verified} \colorbox{red!0}{\strut PurchaseI} \colorbox{red!0}{\strut saw} \colorbox{red!0}{\strut this} \colorbox{red!26}{\strut movie} \colorbox{red!0}{\strut while} \colorbox{red!0}{\strut in} \colorbox{red!0}{\strut high} \colorbox{red!1}{\strut school} \colorbox{red!0}{\strut in} \colorbox{red!0}{\strut 1988} \colorbox{red!0}{\strut .} \colorbox{red!0}{\strut 4} \colorbox{red!0}{\strut years} \colorbox{red!0}{\strut after} \colorbox{red!0}{\strut it} \colorbox{red!0}{\strut came} \colorbox{red!0}{\strut out} \colorbox{red!0}{\strut .} \colorbox{red!0}{\strut on} \colorbox{red!1}{\strut tv} \colorbox{red!0}{\strut and} \colorbox{red!0}{\strut it} \colorbox{red!0}{\strut was} \colorbox{red!0}{\strut of} \colorbox{red!0}{\strut course} \colorbox{red!0}{\strut edited} \colorbox{red!0}{\strut for} \colorbox{red!1}{\strut nudity} \colorbox{red!0}{\strut .} \colorbox{red!0}{\strut Just} \colorbox{red!0}{\strut the} \colorbox{red!0}{\strut same} \colorbox{red!0}{\strut ,} \colorbox{red!0}{\strut though} \colorbox{red!0}{\strut ,} \colorbox{red!0}{\strut the} \colorbox{red!0}{\strut editing} \colorbox{red!0}{\strut did} \colorbox{red!0}{\strut nt} \colorbox{red!0}{\strut take} \colorbox{red!3}{\strut away} \colorbox{red!0}{\strut from} \colorbox{red!0}{\strut the} \colorbox{red!26}{\strut movie} \colorbox{red!0}{\strut s} \colorbox{red!0}{\strut .} \colorbox{red!0}{\strut .} \colorbox{red!3}{\strut Rebel} \colorbox{red!0}{\strut Without} \colorbox{red!0}{\strut A} \colorbox{red!1}{\strut Cause} \colorbox{red!0}{\strut .} \colorbox{red!0}{\strut .} \colorbox{red!0}{\strut .} \colorbox{red!0}{\strut Romeo} \colorbox{red!0}{\strut .} \colorbox{red!0}{\strut Juliet} \colorbox{red!0}{\strut love} \colorbox{red!0}{\strut story} \colorbox{red!1}{\strut which} \colorbox{red!0}{\strut inspired} \colorbox{red!0}{\strut me} \colorbox{red!0}{\strut to} \colorbox{red!0}{\strut wish} \colorbox{red!0}{\strut I} \colorbox{red!0}{\strut could} \colorbox{red!0}{\strut be} \colorbox{red!11}{\strut Daryl} \colorbox{red!6}{\strut Hannah} \colorbox{red!3}{\strut running} \colorbox{red!3}{\strut away} \colorbox{red!0}{\strut on} \colorbox{red!0}{\strut the} \colorbox{red!0}{\strut back} \colorbox{red!0}{\strut of} \colorbox{red!0}{\strut a} \colorbox{red!0}{\strut motorcycle} \colorbox{red!0}{\strut wrapped} 
}}}
\end{CJK*}

\begin{CJK*}{UTF8}{gbsn}
{\setlength{\fboxsep}{0pt}\colorbox{white!0}{\parbox{0.9\textwidth}{
\colorbox{red!40}{\strut Zipper} \colorbox{red!3}{\strut .} \colorbox{red!0}{\strut 2015} \colorbox{red!0}{\strut .} \colorbox{red!0}{\strut .} \colorbox{red!0}{\strut FULL} \colorbox{red!5}{\strut CAST} \colorbox{red!0}{\strut AND} \colorbox{red!0}{\strut CREW} \colorbox{red!0}{\strut .} \colorbox{red!0}{\strut TRIVIA} \colorbox{red!0}{\strut .} \colorbox{red!0}{\strut USER} \colorbox{red!0}{\strut REVIEWS} \colorbox{red!0}{\strut .} \colorbox{red!0}{\strut IMDbPro} \colorbox{red!0}{\strut .} \colorbox{red!0}{\strut MORESHARE5.7} \colorbox{red!0}{\strut 105,536Rate} \colorbox{red!0}{\strut ThisZipper} \colorbox{red!3}{\strut .} \colorbox{red!0}{\strut 2015} \colorbox{red!0}{\strut .} \colorbox{red!0}{\strut R} \colorbox{red!0}{\strut .} \colorbox{red!0}{\strut 1h} \colorbox{red!0}{\strut 52min} \colorbox{red!0}{\strut .} \colorbox{red!0}{\strut Drama} \colorbox{red!0}{\strut ,} \colorbox{red!0}{\strut Thriller} \colorbox{red!0}{\strut .} \colorbox{red!0}{\strut 28} \colorbox{red!0}{\strut August} \colorbox{red!0}{\strut 2015} \colorbox{red!3}{\strut .} \colorbox{red!0}{\strut USA} \colorbox{red!0}{\strut .} \colorbox{red!0}{\strut 221} \colorbox{red!0}{\strut .} \colorbox{red!0}{\strut Trailer3} \colorbox{red!0}{\strut VIDEOS} \colorbox{red!0}{\strut 22} \colorbox{red!0}{\strut IMAGESWatch} \colorbox{red!0}{\strut NowFrom} \colorbox{red!0}{\strut .} \colorbox{red!0}{\strut 3.99} \colorbox{red!3}{\strut .} \colorbox{red!0}{\strut SD} \colorbox{red!0}{\strut .} \colorbox{red!0}{\strut on} \colorbox{red!0}{\strut Prime} \colorbox{red!0}{\strut VideoA} \colorbox{red!0}{\strut successful} \colorbox{red!0}{\strut family} \colorbox{red!0}{\strut man} \colorbox{red!0}{\strut with} \colorbox{red!0}{\strut a} \colorbox{red!0}{\strut blossoming} \colorbox{red!0}{\strut political} \colorbox{red!0}{\strut career} \colorbox{red!0}{\strut loses} \colorbox{red!0}{\strut all} \colorbox{red!0}{\strut sense} \colorbox{red!0}{\strut of} \colorbox{red!0}{\strut morality} \colorbox{red!3}{\strut when} \colorbox{red!0}{\strut he} \colorbox{red!0}{\strut becomes} \colorbox{red!0}{\strut addicted} \colorbox{red!0}{\strut to} \colorbox{red!0}{\strut using} \colorbox{red!0}{\strut an} \colorbox{red!0}{\strut escort} \colorbox{red!0}{\strut agency.Director} \colorbox{red!0}{\strut .} \colorbox{red!3}{\strut Mora} \colorbox{red!0}{\strut StephensWriters} \colorbox{red!0}{\strut .} \colorbox{red!3}{\strut Mora} \colorbox{red!0}{\strut Stephens} \colorbox{red!0}{\strut ,} \colorbox{red!0}{\strut Joel} \colorbox{red!0}{\strut Viertel} \colorbox{red!0}{\strut .} \colorbox{red!0}{\strut 2} \colorbox{red!0}{\strut more} \colorbox{red!0}{\strut credits} \colorbox{red!0}{\strut .} \colorbox{red!3}{\strut Stars} \colorbox{red!0}{\strut .} \colorbox{red!3}{\strut Patrick} \colorbox{red!0}{\strut Wilson} \colorbox{red!0}{\strut ,} \colorbox{red!0}{\strut Lena} \colorbox{red!0}{\strut Headey} \colorbox{red!0}{\strut ,} \colorbox{red!0}{\strut Ray} \colorbox{red!0}{\strut Winstone} \colorbox{red!0}{\strut .} \colorbox{red!0}{\strut See} \colorbox{red!0}{\strut full} \colorbox{red!5}{\strut cast} \colorbox{red!0}{\strut .} \colorbox{red!0}{\strut crew} \colorbox{red!0}{\strut .} \colorbox{red!0}{\strut 39MetascoreFrom} \colorbox{red!0}{\strut metacritic.comReviews26} \colorbox{red!0}{\strut user} \colorbox{red!0}{\strut .} \colorbox{red!0}{\strut 39} \colorbox{red!0}{\strut criticAre} \colorbox{red!0}{\strut You} \colorbox{red!0}{\strut Team} \colorbox{red!0}{\strut Emily} \colorbox{red!0}{\strut or} \colorbox{red!0}{\strut Team} \colorbox{red!0}{\strut John} \colorbox{red!0}{\strut ?} \colorbox{red!0}{\strut Emily} \colorbox{red!0}{\strut Blunt} \colorbox{red!0}{\strut or} \colorbox{red!0}{\strut John} \colorbox{red!0}{\strut Krasinski} \colorbox{red!0}{\strut .} \colorbox{red!9}{\strut Who} \colorbox{red!0}{\strut would} \colorbox{red!3}{\strut survive} \colorbox{red!0}{\strut in} \colorbox{red!0}{\strut a} \colorbox{red!0}{\strut post-apocalyptic} \colorbox{red!0}{\strut world} \colorbox{red!0}{\strut ?} \colorbox{red!0}{\strut The} \colorbox{red!5}{\strut cast} \colorbox{red!0}{\strut of} \colorbox{red!0}{\strut A} \colorbox{red!0}{\strut Quiet} \colorbox{red!0}{\strut Place} \colorbox{red!0}{\strut place} \colorbox{red!0}{\strut their} \colorbox{red!0}{\strut bets.Watch} \colorbox{red!0}{\strut nowRelated} \colorbox{red!0}{\strut NewsJohn} \colorbox{red!0}{\strut Cho} \colorbox{red!0}{\strut Joins} \colorbox{red!0}{\strut the} \colorbox{red!5}{\strut Cast} \colorbox{red!0}{\strut of} \colorbox{red!0}{\strut Fox} \colorbox{red!0}{\strut .} \colorbox{red!0}{\strut s} \colorbox{red!0}{\strut The} \colorbox{red!3}{\strut Exorcist} \colorbox{red!0}{\strut Season} \colorbox{red!0}{\strut 2} \colorbox{red!0}{\strut ,} \colorbox{red!0}{\strut New} \colorbox{red!0}{\strut Plot} \colorbox{red!0}{\strut Details} \colorbox{red!0}{\strut Revealed08} \colorbox{red!0}{\strut July} \colorbox{red!0}{\strut 2017} \colorbox{red!0}{\strut .} \colorbox{red!0}{\strut DailyDeadDVD} \colorbox{red!0}{\strut Review} \colorbox{red!0}{\strut .} \colorbox{red!16}{\strut Reckless} \colorbox{red!3}{\strut .} \colorbox{red!0}{\strut 2015} \colorbox{red!0}{\strut .} \colorbox{red!0}{\strut 25} \colorbox{red!0}{\strut July} \colorbox{red!0}{\strut 2016} \colorbox{red!0}{\strut .} \colorbox{red!0}{\strut FlickeringmythGlee} \colorbox{red!0}{\strut .} \colorbox{red!3}{\strut star} \colorbox{red!0}{\strut Dianna} \colorbox{red!0}{\strut Agron} \colorbox{red!0}{\strut thriller} \colorbox{red!3}{\strut heads} \colorbox{red!0}{\strut to} \colorbox{red!0}{\strut WestEnd12} \colorbox{red!0}{\strut February} \colorbox{red!0}{\strut 2016} \colorbox{red!0}{\strut .} \colorbox{red!0}{\strut ScreenDailySee} \colorbox{red!0}{\strut all} \colorbox{red!0}{\strut related} \colorbox{red!0}{\strut articles} \colorbox{red!0}{\strut .} \colorbox{red!0}{\strut Around} \colorbox{red!0}{\strut The} \colorbox{red!0}{\strut WebPowered} \colorbox{red!0}{\strut by} \colorbox{red!0}{\strut ZergNetEditorial} \colorbox{red!0}{\strut ListsRelated} \colorbox{red!3}{\strut lists} \colorbox{red!0}{\strut from} \colorbox{red!0}{\strut IMDb} \colorbox{red!0}{\strut editorsSundance} \colorbox{red!0}{\strut 2015} \colorbox{red!0}{\strut .} \colorbox{red!0}{\strut Distribution} \colorbox{red!0}{\strut Dealsa} \colorbox{red!3}{\strut list} \colorbox{red!0}{\strut of} \colorbox{red!0}{\strut 33} \colorbox{red!3}{\strut titles} \colorbox{red!0}{\strut updated} \colorbox{red!0}{\strut 09} \colorbox{red!0}{\strut Feb} \colorbox{red!0}{\strut 2015Sundance} \colorbox{red!0}{\strut 2015} \colorbox{red!0}{\strut .} \colorbox{red!0}{\strut Premieresa} \colorbox{red!3}{\strut list} \colorbox{red!0}{\strut of} \colorbox{red!0}{\strut 18} \colorbox{red!0}{\strut images} \colorbox{red!0}{\strut updated} \colorbox{red!0}{\strut 20} \colorbox{red!0}{\strut Jan} \colorbox{red!0}{\strut 2015Sundance} \colorbox{red!0}{\strut 2015} \colorbox{red!0}{\strut .} \colorbox{red!0}{\strut Premieresa} \colorbox{red!3}{\strut list} \colorbox{red!0}{\strut of} \colorbox{red!0}{\strut 18} \colorbox{red!3}{\strut titles} \colorbox{red!0}{\strut updated} \colorbox{red!0}{\strut 16} \colorbox{red!0}{\strut Dec} \colorbox{red!0}{\strut 2014Create} \colorbox{red!0}{\strut a} \colorbox{red!3}{\strut list} \colorbox{red!0}{\strut .} \colorbox{red!0}{\strut User} \colorbox{red!0}{\strut ListsRelated} \colorbox{red!3}{\strut lists} \colorbox{red!0}{\strut from} \colorbox{red!0}{\strut IMDb} \colorbox{red!0}{\strut users2017} \colorbox{red!12}{\strut Movies} \colorbox{red!0}{\strut watcheda} \colorbox{red!3}{\strut list} \colorbox{red!0}{\strut of} \colorbox{red!0}{\strut 43} \colorbox{red!3}{\strut titles} \colorbox{red!0}{\strut created} \colorbox{red!0}{\strut 02} \colorbox{red!0}{\strut Jan} \colorbox{red!0}{\strut 20175.7} \colorbox{red!3}{\strut Rated} \colorbox{red!0}{\strut Filmsa} \colorbox{red!3}{\strut list} \colorbox{red!0}{\strut of} \colorbox{red!0}{\strut 24} \colorbox{red!3}{\strut titles} \colorbox{red!0}{\strut created} \colorbox{red!0}{\strut 11} \colorbox{red!0}{\strut months} \colorbox{red!0}{\strut agoRay} \colorbox{red!0}{\strut Winstone} \colorbox{red!0}{\strut Moviesa} \colorbox{red!3}{\strut list} \colorbox{red!0}{\strut of} \colorbox{red!0}{\strut 49} \colorbox{red!3}{\strut titles} \colorbox{red!0}{\strut created} \colorbox{red!0}{\strut 9} \colorbox{red!0}{\strut months} \colorbox{red!0}{\strut agoJune} \colorbox{red!0}{\strut 16a} \colorbox{red!3}{\strut list} \colorbox{red!0}{\strut of} \colorbox{red!0}{\strut 24} \colorbox{red!3}{\strut titles} \colorbox{red!0}{\strut created} \colorbox{red!0}{\strut 04} \colorbox{red!0}{\strut Jun} \colorbox{red!0}{\strut 2016Favourite} \colorbox{red!5}{\strut Films} \colorbox{red!0}{\strut of} \colorbox{red!0}{\strut 2015a} \colorbox{red!3}{\strut list} \colorbox{red!0}{\strut of} \colorbox{red!0}{\strut 30} \colorbox{red!3}{\strut titles} \colorbox{red!0}{\strut created} \colorbox{red!0}{\strut 07} \colorbox{red!0}{\strut Jan} \colorbox{red!0}{\strut 2016See} \colorbox{red!0}{\strut all} \colorbox{red!0}{\strut related} \colorbox{red!3}{\strut lists} \colorbox{red!0}{\strut .} \colorbox{red!0}{\strut Related} 
}}}
\end{CJK*}

query: where is the corral club located in reliant stadium

\begin{CJK*}{UTF8}{gbsn}
{\setlength{\fboxsep}{0pt}\colorbox{white!0}{\parbox{0.9\textwidth}{
\colorbox{red!15}{\strut NRG} \colorbox{red!14}{\strut Stadium} \colorbox{red!0}{\strut .} \colorbox{red!0}{\strut Formerly} \colorbox{red!0}{\strut Reliant} \colorbox{red!14}{\strut Stadium} \colorbox{red!0}{\strut .} \colorbox{red!15}{\strut Seating} \colorbox{red!0}{\strut Chart} \colorbox{red!0}{\strut .} \colorbox{red!0}{\strut Ticket} \colorbox{red!0}{\strut Info} \colorbox{red!0}{\strut .} \colorbox{red!0}{\strut A3} \colorbox{red!0}{\strut A4} \colorbox{red!0}{\strut A2} \colorbox{red!0}{\strut A5} \colorbox{red!0}{\strut A1} \colorbox{red!0}{\strut A6} \colorbox{red!0}{\strut B3} \colorbox{red!0}{\strut B4} \colorbox{red!0}{\strut 109} \colorbox{red!0}{\strut 124} \colorbox{red!0}{\strut 108} \colorbox{red!0}{\strut 125} \colorbox{red!0}{\strut 107} \colorbox{red!0}{\strut 126} \colorbox{red!0}{\strut B2} \colorbox{red!0}{\strut B5} \colorbox{red!0}{\strut 106} \colorbox{red!0}{\strut 127} \colorbox{red!0}{\strut B1} \colorbox{red!0}{\strut B6} \colorbox{red!0}{\strut 105} \colorbox{red!0}{\strut 128} \colorbox{red!0}{\strut 104} \colorbox{red!0}{\strut 129} \colorbox{red!0}{\strut 110} \colorbox{red!0}{\strut 123} \colorbox{red!0}{\strut 103} \colorbox{red!0}{\strut 130} \colorbox{red!0}{\strut 312} \colorbox{red!0}{\strut 335} \colorbox{red!0}{\strut 311} \colorbox{red!0}{\strut 336} \colorbox{red!0}{\strut 102} \colorbox{red!0}{\strut 131} \colorbox{red!0}{\strut 310} \colorbox{red!0}{\strut 337} \colorbox{red!0}{\strut 309} \colorbox{red!0}{\strut 338} \colorbox{red!0}{\strut 101} \colorbox{red!0}{\strut 132} \colorbox{red!0}{\strut 308} \colorbox{red!0}{\strut 339} \colorbox{red!0}{\strut 307} \colorbox{red!0}{\strut 340} \colorbox{red!0}{\strut 133} \colorbox{red!0}{\strut 140} \colorbox{red!0}{\strut C3} \colorbox{red!0}{\strut C4} \colorbox{red!0}{\strut 306} \colorbox{red!0}{\strut C2} \colorbox{red!0}{\strut C5} \colorbox{red!0}{\strut 334} \colorbox{red!0}{\strut 341} \colorbox{red!0}{\strut 305} \colorbox{red!0}{\strut C1} \colorbox{red!0}{\strut C6} \colorbox{red!0}{\strut 134} \colorbox{red!0}{\strut 139} \colorbox{red!0}{\strut 342} \colorbox{red!0}{\strut 304} \colorbox{red!0}{\strut 510} \colorbox{red!0}{\strut 532} \colorbox{red!0}{\strut 343} \colorbox{red!0}{\strut 111} \colorbox{red!0}{\strut 122} \colorbox{red!0}{\strut 509} \colorbox{red!0}{\strut 135} \colorbox{red!0}{\strut 136} \colorbox{red!0}{\strut 137} \colorbox{red!0}{\strut 138} \colorbox{red!0}{\strut 303} \colorbox{red!0}{\strut 533} \colorbox{red!0}{\strut 344} \colorbox{red!0}{\strut 508} \colorbox{red!0}{\strut 534} \colorbox{red!0}{\strut 302} \colorbox{red!0}{\strut 313} \colorbox{red!0}{\strut 345} \colorbox{red!0}{\strut 507} \colorbox{red!0}{\strut 535} \colorbox{red!0}{\strut 301} \colorbox{red!0}{\strut 346} \colorbox{red!0}{\strut 506} \colorbox{red!0}{\strut 536} \colorbox{red!0}{\strut 356} \colorbox{red!0}{\strut 333} \colorbox{red!0}{\strut 505} \colorbox{red!0}{\strut 347} \colorbox{red!0}{\strut 537} \colorbox{red!0}{\strut 531} \colorbox{red!0}{\strut 355} \colorbox{red!0}{\strut 504} \colorbox{red!0}{\strut 633} \colorbox{red!0}{\strut 610} \colorbox{red!0}{\strut 348} \colorbox{red!0}{\strut 538} \colorbox{red!0}{\strut 609} \colorbox{red!0}{\strut 634} \colorbox{red!0}{\strut 354} \colorbox{red!0}{\strut 503} \colorbox{red!0}{\strut 539} \colorbox{red!0}{\strut 349} \colorbox{red!0}{\strut 608} \colorbox{red!0}{\strut 635} \colorbox{red!0}{\strut 502} \colorbox{red!0}{\strut 350} \colorbox{red!0}{\strut 351} \colorbox{red!0}{\strut 352} \colorbox{red!0}{\strut 353} \colorbox{red!0}{\strut 540} \colorbox{red!0}{\strut 607} \colorbox{red!0}{\strut 636} \colorbox{red!0}{\strut 501} \colorbox{red!0}{\strut 511} \colorbox{red!0}{\strut 606} \colorbox{red!0}{\strut 541} \colorbox{red!0}{\strut 637} \colorbox{red!0}{\strut 632} \colorbox{red!0}{\strut 605} \colorbox{red!0}{\strut 552} \colorbox{red!0}{\strut 638} \colorbox{red!0}{\strut 542} \colorbox{red!0}{\strut 604} \colorbox{red!0}{\strut 530} \colorbox{red!0}{\strut 639} \colorbox{red!0}{\strut 551} \colorbox{red!0}{\strut 543} \colorbox{red!0}{\strut 603} \colorbox{red!0}{\strut 611} \colorbox{red!0}{\strut 332} \colorbox{red!0}{\strut 112} \colorbox{red!0}{\strut 640} \colorbox{red!0}{\strut 121} \colorbox{red!0}{\strut 550} \colorbox{red!0}{\strut 544} \colorbox{red!0}{\strut 602} \colorbox{red!0}{\strut 641} \colorbox{red!0}{\strut 545} \colorbox{red!0}{\strut 546} \colorbox{red!0}{\strut 547} \colorbox{red!0}{\strut 548} \colorbox{red!0}{\strut 549} \colorbox{red!0}{\strut 601} \colorbox{red!0}{\strut 631} \colorbox{red!0}{\strut 642} \colorbox{red!0}{\strut 314} \colorbox{red!0}{\strut 652} \colorbox{red!0}{\strut 643} \colorbox{red!0}{\strut 651} \colorbox{red!0}{\strut 644} \colorbox{red!0}{\strut 650} \colorbox{red!0}{\strut 645} \colorbox{red!0}{\strut 529} \colorbox{red!0}{\strut 646} \colorbox{red!0}{\strut 647} \colorbox{red!0}{\strut 648} \colorbox{red!0}{\strut 649} \colorbox{red!0}{\strut 630} \colorbox{red!0}{\strut 612} \colorbox{red!0}{\strut 512} \colorbox{red!0}{\strut 331} \colorbox{red!0}{\strut 717} \colorbox{red!0}{\strut 718} \colorbox{red!0}{\strut 719} \colorbox{red!0}{\strut 720} \colorbox{red!0}{\strut 721} \colorbox{red!0}{\strut 722} \colorbox{red!0}{\strut 723} \colorbox{red!0}{\strut 724} \colorbox{red!0}{\strut 725} \colorbox{red!0}{\strut 726} \colorbox{red!0}{\strut 743} \colorbox{red!0}{\strut 744} \colorbox{red!0}{\strut 746} \colorbox{red!0}{\strut 747} \colorbox{red!0}{\strut 748} \colorbox{red!0}{\strut 749} \colorbox{red!0}{\strut 750} \colorbox{red!0}{\strut 751} \colorbox{red!0}{\strut 752} \colorbox{red!0}{\strut 745} \colorbox{red!0}{\strut 629} \colorbox{red!0}{\strut 528} \colorbox{red!0}{\strut 613} \colorbox{red!0}{\strut 113} \colorbox{red!0}{\strut 114} \colorbox{red!0}{\strut 115} \colorbox{red!0}{\strut 116} \colorbox{red!0}{\strut 117} \colorbox{red!0}{\strut 118} \colorbox{red!0}{\strut 119} \colorbox{red!0}{\strut 120} \colorbox{red!0}{\strut 628} \colorbox{red!0}{\strut 315} \colorbox{red!0}{\strut 316} \colorbox{red!0}{\strut 317} \colorbox{red!0}{\strut 318} \colorbox{red!0}{\strut 319} \colorbox{red!0}{\strut 320} \colorbox{red!0}{\strut 321} \colorbox{red!0}{\strut 322} \colorbox{red!0}{\strut 323} \colorbox{red!0}{\strut 324} \colorbox{red!0}{\strut 325} \colorbox{red!0}{\strut 326} \colorbox{red!0}{\strut 327} \colorbox{red!0}{\strut 328} \colorbox{red!0}{\strut 329} \colorbox{red!0}{\strut 330} \colorbox{red!0}{\strut 513} \colorbox{red!0}{\strut 514} \colorbox{red!0}{\strut 515} \colorbox{red!0}{\strut 516} \colorbox{red!0}{\strut 517} \colorbox{red!0}{\strut 518} \colorbox{red!0}{\strut 519} \colorbox{red!0}{\strut 520} \colorbox{red!0}{\strut 521} \colorbox{red!0}{\strut 522} \colorbox{red!0}{\strut 523} \colorbox{red!0}{\strut 524} \colorbox{red!0}{\strut 525} \colorbox{red!0}{\strut 526} \colorbox{red!0}{\strut 527} \colorbox{red!0}{\strut 620} \colorbox{red!0}{\strut 621} \colorbox{red!0}{\strut 622} \colorbox{red!0}{\strut 623} \colorbox{red!0}{\strut 624} \colorbox{red!0}{\strut 625} \colorbox{red!0}{\strut 626} \colorbox{red!0}{\strut 627} \colorbox{red!0}{\strut 614} \colorbox{red!0}{\strut 615} \colorbox{red!0}{\strut 616} \colorbox{red!0}{\strut 617} \colorbox{red!0}{\strut 618} \colorbox{red!0}{\strut 619Seating} \colorbox{red!0}{\strut ConfigurationsStandard} \colorbox{red!0}{\strut Concert} \colorbox{red!0}{\strut Basketball} \colorbox{red!1}{\strut Houston} \colorbox{red!0}{\strut TexansHouston} \colorbox{red!1}{\strut Texans} \colorbox{red!15}{\strut Seating} \colorbox{red!0}{\strut Chart} \colorbox{red!0}{\strut .} \colorbox{red!15}{\strut NRG} \colorbox{red!14}{\strut Stadium} \colorbox{red!14}{\strut Seat} \colorbox{red!0}{\strut ViewsWelcome} \colorbox{red!0}{\strut to} \colorbox{red!0}{\strut TickPick} \colorbox{red!0}{\strut .} \colorbox{red!0}{\strut s} \colorbox{red!1}{\strut Houston} \colorbox{red!1}{\strut Texans} \colorbox{red!15}{\strut Seating} \colorbox{red!0}{\strut Chart} \colorbox{red!0}{\strut .} \colorbox{red!0}{\strut Here} \colorbox{red!0}{\strut we} \colorbox{red!0}{\strut will} \colorbox{red!0}{\strut cover} \colorbox{red!0}{\strut everything} \colorbox{red!0}{\strut you} \colorbox{red!0}{\strut need} \colorbox{red!0}{\strut to} \colorbox{red!0}{\strut knwo} \colorbox{red!0}{\strut before} \colorbox{red!0}{\strut purchasing} \colorbox{red!0}{\strut Cheap} \colorbox{red!1}{\strut Houston} \colorbox{red!1}{\strut Texans} \colorbox{red!1}{\strut Tickets} \colorbox{red!0}{\strut ,} \colorbox{red!0}{\strut including} \colorbox{red!15}{\strut NRG} \colorbox{red!14}{\strut Stadium} \colorbox{red!0}{\strut row} \colorbox{red!0}{\strut and} \colorbox{red!14}{\strut seat} \colorbox{red!4}{\strut numbers} \colorbox{red!0}{\strut ,} \colorbox{red!1}{\strut Texans} \colorbox{red!14}{\strut seat} \colorbox{red!0}{\strut views} 
}}}
\end{CJK*}

\begin{CJK*}{UTF8}{gbsn}
{\setlength{\fboxsep}{0pt}\colorbox{white!0}{\parbox{0.9\textwidth}{
\colorbox{red!5}{\strut club} \colorbox{red!3}{\strut seats} \colorbox{red!0}{\strut at} \colorbox{red!0}{\strut the} \colorbox{red!2}{\strut texans} \colorbox{red!5}{\strut club} \colorbox{red!3}{\strut seats} \colorbox{red!0}{\strut at} \colorbox{red!0}{\strut the} \colorbox{red!0}{\strut texansRam} \colorbox{red!0}{\strut KingSubscribe} \colorbox{red!0}{\strut 7Add} \colorbox{red!0}{\strut toShareMore3,855} \colorbox{red!0}{\strut views02Published} \colorbox{red!0}{\strut on} \colorbox{red!0}{\strut Nov} \colorbox{red!0}{\strut 7} \colorbox{red!0}{\strut ,} \colorbox{red!0}{\strut 2010This} \colorbox{red!0}{\strut is} \colorbox{red!0}{\strut the} \colorbox{red!1}{\strut view} \colorbox{red!0}{\strut from} \colorbox{red!0}{\strut the} \colorbox{red!5}{\strut Club} \colorbox{red!2}{\strut Seat} \colorbox{red!1}{\strut section} \colorbox{red!0}{\strut in} \colorbox{red!2}{\strut Reliant} \colorbox{red!0}{\strut StadiumShow} \colorbox{red!0}{\strut moreLoading} \colorbox{red!0}{\strut ...} \colorbox{red!0}{\strut AutoplayUp} \colorbox{red!0}{\strut nextHouston} \colorbox{red!0}{\strut 20-25} \colorbox{red!0}{\strut Oakland} \colorbox{red!0}{\strut .} \colorbox{red!2}{\strut Reliant} \colorbox{red!8}{\strut Stadium} \colorbox{red!0}{\strut ,} \colorbox{red!4}{\strut Houston} \colorbox{red!0}{\strut .} \colorbox{red!5}{\strut Club} \colorbox{red!0}{\strut Section.aldjazairi11,899} \colorbox{red!0}{\strut views244Inside} \colorbox{red!2}{\strut Reliant} \colorbox{red!8}{\strut Stadium} \colorbox{red!0}{\strut IEPA0000124,718} \colorbox{red!0}{\strut views302Reliant} \colorbox{red!8}{\strut Stadium} \colorbox{red!0}{\strut in} \colorbox{red!0}{\strut One} \colorbox{red!0}{\strut Minuteminutemaps20,646} \colorbox{red!0}{\strut views116Club} \colorbox{red!3}{\strut Seats} \colorbox{red!1}{\strut Pats} \colorbox{red!0}{\strut GameGene} \colorbox{red!0}{\strut Brown1,703} \colorbox{red!0}{\strut views033NRG} \colorbox{red!8}{\strut Stadium} \colorbox{red!0}{\strut .} \colorbox{red!0}{\strut Walking} \colorbox{red!0}{\strut Into} \colorbox{red!1}{\strut Section} \colorbox{red!0}{\strut 606DoktorStrangelove3,487} \colorbox{red!0}{\strut views028TEXANS} \colorbox{red!1}{\strut BULLS} \colorbox{red!0}{\strut ON} \colorbox{red!0}{\strut PARADE} \colorbox{red!0}{\strut COMING} \colorbox{red!0}{\strut OUT} \colorbox{red!0}{\strut OF} \colorbox{red!0}{\strut THE} \colorbox{red!0}{\strut TUNNEL} \colorbox{red!0}{\strut LIVE} \colorbox{red!0}{\strut SATELLITE} \colorbox{red!0}{\strut FEEDsatellite} \colorbox{red!0}{\strut pro30,288} \colorbox{red!0}{\strut views550121110} \colorbox{red!2}{\strut Reliant} \colorbox{red!8}{\strut Stadium} \colorbox{red!0}{\strut turf} \colorbox{red!0}{\strut lapseMarc} \colorbox{red!0}{\strut Herklotz26,296} \colorbox{red!0}{\strut views145Reliant} \colorbox{red!8}{\strut Stadium} \colorbox{red!0}{\strut ,} \colorbox{red!4}{\strut Houston} \colorbox{red!0}{\strut ,} \colorbox{red!1}{\strut Texas} \colorbox{red!0}{\strut Not} \colorbox{red!0}{\strut a} \colorbox{red!0}{\strut bad} \colorbox{red!2}{\strut seat} \colorbox{red!0}{\strut in} \colorbox{red!0}{\strut theHouse} \colorbox{red!0}{\strut !} \colorbox{red!0}{\strut Elmer} \colorbox{red!0}{\strut Mudguaard1,332} \colorbox{red!0}{\strut views041Panoramic} \colorbox{red!1}{\strut view} \colorbox{red!0}{\strut of} \colorbox{red!2}{\strut Reliant} \colorbox{red!0}{\strut StadiumJCLIVE325877} \colorbox{red!0}{\strut views039Monster} \colorbox{red!0}{\strut Jam} \colorbox{red!0}{\strut 2014} \colorbox{red!0}{\strut 1414} \colorbox{red!1}{\strut Relient} \colorbox{red!8}{\strut Stadium} \colorbox{red!0}{\strut .} \colorbox{red!4}{\strut Houston} \colorbox{red!0}{\strut ,} \colorbox{red!1}{\strut Texas} \colorbox{red!0}{\strut .} \colorbox{red!0}{\strut WhosZappo7,171} \colorbox{red!0}{\strut views1236NRG} \colorbox{red!8}{\strut Stadium} \colorbox{red!0}{\strut -} \colorbox{red!4}{\strut Houston} \colorbox{red!2}{\strut Texans} \colorbox{red!0}{\strut .} \colorbox{red!2}{\strut NFL} \colorbox{red!0}{\strut .} \colorbox{red!8}{\strut Stadium} \colorbox{red!0}{\strut Zone19,528} \colorbox{red!0}{\strut views119Panthers} \colorbox{red!8}{\strut Stadium} \colorbox{red!0}{\strut Tours} \colorbox{red!0}{\strut and} \colorbox{red!5}{\strut Club} \colorbox{red!0}{\strut Seatschiefkeith14,758} \colorbox{red!0}{\strut views622Houston} \colorbox{red!2}{\strut Texans} \colorbox{red!0}{\strut 360} \colorbox{red!0}{\strut Player} \colorbox{red!0}{\strut EntranceFamous} \colorbox{red!0}{\strut Group1,798} \colorbox{red!0}{\strut views360107NRG} \colorbox{red!8}{\strut Stadium} \colorbox{red!0}{\strut History} \colorbox{red!0}{\strut on} \colorbox{red!0}{\strut The} \colorbox{red!1}{\strut Rich} \colorbox{red!0}{\strut Eisen} \colorbox{red!0}{\strut Show} \colorbox{red!0}{\strut 10914The} \colorbox{red!1}{\strut Rich} \colorbox{red!0}{\strut Eisen} \colorbox{red!0}{\strut Show2,214} \colorbox{red!0}{\strut views201FSU} \colorbox{red!5}{\strut Club} \colorbox{red!3}{\strut Seats} \colorbox{red!0}{\strut 60} \colorbox{red!0}{\strut secChampions} \colorbox{red!0}{\strut Campaign14,285} \colorbox{red!0}{\strut views101View} \colorbox{red!0}{\strut from} \colorbox{red!0}{\strut the} \colorbox{red!0}{\strut Suite} \colorbox{red!0}{\strut Level} \colorbox{red!0}{\strut of} \colorbox{red!0}{\strut the} \colorbox{red!1}{\strut Cowboys} \colorbox{red!0}{\strut Stadiumhoutexusa23,420} \colorbox{red!0}{\strut views055Walking} \colorbox{red!0}{\strut down} \colorbox{red!0}{\strut to} \colorbox{red!0}{\strut our} \colorbox{red!3}{\strut seats} \colorbox{red!0}{\strut at} \colorbox{red!1}{\strut Lexus} \colorbox{red!0}{\strut Diamond} \colorbox{red!5}{\strut Club} \colorbox{red!0}{\strut ...} \colorbox{red!0}{\strut woahjophill2460} \colorbox{red!0}{\strut views031BASE} \colorbox{red!0}{\strut jump} \colorbox{red!0}{\strut inside} \colorbox{red!2}{\strut Reliant} \colorbox{red!0}{\strut Stadiumredbullusa123,880} \colorbox{red!0}{\strut views1218} \colorbox{red!0}{\strut 13} \colorbox{red!0}{\strut 13} \colorbox{red!2}{\strut Texans} \colorbox{red!0}{\strut Video} \colorbox{red!0}{\strut Board} \colorbox{red!0}{\strut PrezoMichael} \colorbox{red!0}{\strut Williams4,411} \colorbox{red!0}{\strut views406A} \colorbox{red!0}{\strut walk} \colorbox{red!0}{\strut through} \colorbox{red!0}{\strut the} \colorbox{red!5}{\strut Club} \colorbox{red!0}{\strut level} \colorbox{red!0}{\strut at} \colorbox{red!4}{\strut Houston} \colorbox{red!0}{\strut Rodeo} \colorbox{red!0}{\strut 2012Bandit44TA1,278} \colorbox{red!0}{\strut views035Show} \colorbox{red!0}{\strut more} 
}}}
\end{CJK*}

query: what is the charter of french liberties

\begin{CJK*}{UTF8}{gbsn}
{\setlength{\fboxsep}{0pt}\colorbox{white!0}{\parbox{0.9\textwidth}{
\colorbox{red!1}{\strut Charter} \colorbox{red!0}{\strut of} \colorbox{red!2}{\strut 1814} \colorbox{red!0}{\strut Alternative} \colorbox{red!0}{\strut Title} \colorbox{red!0}{\strut .} \colorbox{red!2}{\strut Charte} \colorbox{red!0}{\strut ConstitutionnelleCharter} \colorbox{red!0}{\strut of} \colorbox{red!2}{\strut 1814} \colorbox{red!0}{\strut ,} \colorbox{red!3}{\strut French} \colorbox{red!2}{\strut Charte} \colorbox{red!1}{\strut Constitutionnelle} \colorbox{red!0}{\strut ,} \colorbox{red!3}{\strut French} \colorbox{red!20}{\strut constitution} \colorbox{red!1}{\strut issued} \colorbox{red!0}{\strut by} \colorbox{red!4}{\strut Louis} \colorbox{red!2}{\strut XVIII} \colorbox{red!0}{\strut after} \colorbox{red!0}{\strut he} \colorbox{red!0}{\strut became} \colorbox{red!2}{\strut king} \colorbox{red!0}{\strut .} \colorbox{red!0}{\strut see} \colorbox{red!3}{\strut Bourbon} \colorbox{red!2}{\strut Restoration} \colorbox{red!0}{\strut .} \colorbox{red!0}{\strut .} \colorbox{red!0}{\strut The} \colorbox{red!1}{\strut charter} \colorbox{red!0}{\strut ,} \colorbox{red!1}{\strut which} \colorbox{red!0}{\strut was} \colorbox{red!0}{\strut revised} \colorbox{red!0}{\strut in} \colorbox{red!0}{\strut 1830} \colorbox{red!0}{\strut and} \colorbox{red!0}{\strut remained} \colorbox{red!0}{\strut in} \colorbox{red!1}{\strut effect} \colorbox{red!0}{\strut until} \colorbox{red!0}{\strut 1848} \colorbox{red!0}{\strut ,} \colorbox{red!0}{\strut preserved} \colorbox{red!0}{\strut many} \colorbox{red!0}{\strut liberties} \colorbox{red!0}{\strut won} \colorbox{red!0}{\strut by} \colorbox{red!0}{\strut the} \colorbox{red!3}{\strut French} \colorbox{red!1}{\strut Revolution} \colorbox{red!0}{\strut .} \colorbox{red!0}{\strut It} \colorbox{red!1}{\strut established} \colorbox{red!0}{\strut a} \colorbox{red!18}{\strut constitutional} \colorbox{red!1}{\strut monarchy} \colorbox{red!0}{\strut with} \colorbox{red!0}{\strut a} \colorbox{red!0}{\strut bicameral} \colorbox{red!0}{\strut parliament} \colorbox{red!0}{\strut ,} \colorbox{red!0}{\strut guaranteed} \colorbox{red!0}{\strut civil} \colorbox{red!0}{\strut liberties} \colorbox{red!0}{\strut ,} \colorbox{red!0}{\strut proclaimed} \colorbox{red!0}{\strut religious} \colorbox{red!0}{\strut toleration} \colorbox{red!0}{\strut ,} \colorbox{red!0}{\strut and} \colorbox{red!0}{\strut acknowledged} \colorbox{red!0}{\strut Catholicism} \colorbox{red!0}{\strut as} \colorbox{red!0}{\strut the} \colorbox{red!0}{\strut state} \colorbox{red!0}{\strut religion.Learn} \colorbox{red!0}{\strut More} \colorbox{red!0}{\strut in} \colorbox{red!0}{\strut these} \colorbox{red!0}{\strut related} \colorbox{red!0}{\strut articles} \colorbox{red!0}{\strut .} \colorbox{red!3}{\strut Bourbon} \colorbox{red!0}{\strut RestorationBourbon} \colorbox{red!2}{\strut Restoration} \colorbox{red!0}{\strut ,} \colorbox{red!0}{\strut .} \colorbox{red!0}{\strut 181430} \colorbox{red!0}{\strut .} \colorbox{red!0}{\strut in} \colorbox{red!3}{\strut France} \colorbox{red!0}{\strut ,} \colorbox{red!0}{\strut the} \colorbox{red!0}{\strut period} \colorbox{red!0}{\strut that} \colorbox{red!0}{\strut began} \colorbox{red!4}{\strut when} \colorbox{red!2}{\strut Napoleon} \colorbox{red!0}{\strut I} \colorbox{red!0}{\strut abdicated} \colorbox{red!0}{\strut and} \colorbox{red!0}{\strut the} \colorbox{red!3}{\strut Bourbon} \colorbox{red!0}{\strut monarchs} \colorbox{red!0}{\strut were} \colorbox{red!1}{\strut restored} \colorbox{red!0}{\strut to} \colorbox{red!0}{\strut the} \colorbox{red!0}{\strut throne} \colorbox{red!0}{\strut .} \colorbox{red!0}{\strut The} \colorbox{red!0}{\strut First} \colorbox{red!2}{\strut Restoration} \colorbox{red!0}{\strut occurred} \colorbox{red!4}{\strut when} \colorbox{red!2}{\strut Napoleon} \colorbox{red!0}{\strut fell} \colorbox{red!0}{\strut from} \colorbox{red!0}{\strut power} \colorbox{red!0}{\strut and} \colorbox{red!4}{\strut Louis} \colorbox{red!2}{\strut XVIII} \colorbox{red!0}{\strut became} \colorbox{red!2}{\strut king} \colorbox{red!0}{\strut .} \colorbox{red!4}{\strut Louis} \colorbox{red!0}{\strut .} \colorbox{red!0}{\strut reign} \colorbox{red!0}{\strut was} \colorbox{red!0}{\strut interrupted} \colorbox{red!0}{\strut by} \colorbox{red!2}{\strut Napoleon} \colorbox{red!0}{\strut .} \colorbox{red!0}{\strut s} \colorbox{red!0}{\strut return} \colorbox{red!0}{\strut to} \colorbox{red!3}{\strut France} \colorbox{red!0}{\strut .} \colorbox{red!0}{\strut see} \colorbox{red!0}{\strut Hundred} \colorbox{red!0}{\strut Days} \colorbox{red!0}{\strut .} \colorbox{red!0}{\strut ,} \colorbox{red!0}{\strut but} \colorbox{red!0}{\strut NapoleonRead} \colorbox{red!0}{\strut MoreFrance} \colorbox{red!0}{\strut .} \colorbox{red!4}{\strut Louis} \colorbox{red!2}{\strut XVIII} \colorbox{red!0}{\strut ,} \colorbox{red!0}{\strut 181524refused} \colorbox{red!0}{\strut ,} \colorbox{red!0}{\strut however} \colorbox{red!0}{\strut ,} \colorbox{red!0}{\strut to} \colorbox{red!0}{\strut scrap} \colorbox{red!0}{\strut the} \colorbox{red!1}{\strut Charter} \colorbox{red!0}{\strut of} \colorbox{red!2}{\strut 1814} \colorbox{red!0}{\strut ,} \colorbox{red!0}{\strut in} \colorbox{red!0}{\strut spite} \colorbox{red!0}{\strut of} \colorbox{red!0}{\strut ultra} \colorbox{red!0}{\strut pressure} \colorbox{red!0}{\strut .} \colorbox{red!4}{\strut When} \colorbox{red!0}{\strut a} \colorbox{red!0}{\strut new} \colorbox{red!0}{\strut Chamber} \colorbox{red!0}{\strut of} \colorbox{red!0}{\strut Deputies} \colorbox{red!0}{\strut was} \colorbox{red!0}{\strut elected} \colorbox{red!0}{\strut in} \colorbox{red!0}{\strut August} \colorbox{red!0}{\strut 1815} \colorbox{red!0}{\strut ,} \colorbox{red!0}{\strut the} \colorbox{red!0}{\strut ultras} \colorbox{red!0}{\strut scored} \colorbox{red!0}{\strut a} \colorbox{red!0}{\strut sweeping} \colorbox{red!0}{\strut victory} \colorbox{red!0}{\strut .} \colorbox{red!0}{\strut the} \colorbox{red!0}{\strut surprised} \colorbox{red!2}{\strut king} \colorbox{red!0}{\strut ,} \colorbox{red!7}{\strut who} \colorbox{red!0}{\strut had} \colorbox{red!0}{\strut feared} \colorbox{red!0}{\strut a} \colorbox{red!0}{\strut surge} \colorbox{red!0}{\strut of} \colorbox{red!0}{\strut antimonarchical} \colorbox{red!0}{\strut sentiment} \colorbox{red!0}{\strut ,} \colorbox{red!0}{\strut greeted} \colorbox{red!0}{\strut the} \colorbox{red!0}{\strut legislature} \colorbox{red!0}{\strut as} \colorbox{red!0}{\strut la} \colorbox{red!0}{\strut chambre} \colorbox{red!0}{\strut introuvable} \colorbox{red!0}{\strut .} \colorbox{red!0}{\strut .} \colorbox{red!0}{\strut the} \colorbox{red!0}{\strut incomparableRead} \colorbox{red!0}{\strut MoreSpain} \colorbox{red!0}{\strut .} \colorbox{red!0}{\strut The} \colorbox{red!0}{\strut failure} \colorbox{red!0}{\strut of} \colorbox{red!0}{\strut liberalismconstitution} \colorbox{red!0}{\strut ,} \colorbox{red!0}{\strut based} \colorbox{red!0}{\strut on} \colorbox{red!0}{\strut the} \colorbox{red!3}{\strut French} \colorbox{red!1}{\strut Charter} \colorbox{red!0}{\strut of} \colorbox{red!2}{\strut 1814} \colorbox{red!0}{\strut ,} \colorbox{red!1}{\strut which} \colorbox{red!0}{\strut would} \colorbox{red!0}{\strut give} \colorbox{red!0}{\strut better} \colorbox{red!0}{\strut representation} \colorbox{red!0}{\strut to} \colorbox{red!0}{\strut the} \colorbox{red!0}{\strut upper} \colorbox{red!0}{\strut classes} \colorbox{red!0}{\strut and} \colorbox{red!0}{\strut would} \colorbox{red!0}{\strut not} \colorbox{red!0}{\strut be} \colorbox{red!0}{\strut totally} \colorbox{red!0}{\strut unacceptable} \colorbox{red!0}{\strut to} \colorbox{red!0}{\strut the} \colorbox{red!2}{\strut king} \colorbox{red!0}{\strut ,} \colorbox{red!0}{\strut as} \colorbox{red!0}{\strut was} \colorbox{red!0}{\strut the} \colorbox{red!0}{\strut .} \colorbox{red!0}{\strut prison} \colorbox{red!0}{\strut .} \colorbox{red!0}{\strut of} \colorbox{red!0}{\strut the} \colorbox{red!20}{\strut constitution} \colorbox{red!0}{\strut of} \colorbox{red!0}{\strut 1812} \colorbox{red!0}{\strut .} \colorbox{red!0}{\strut The} \colorbox{red!2}{\strut king} \colorbox{red!0}{\strut gave} \colorbox{red!0}{\strut no} \colorbox{red!0}{\strut support} \colorbox{red!0}{\strut to} \colorbox{red!0}{\strut this} \colorbox{red!0}{\strut movement} \colorbox{red!0}{\strut and} \colorbox{red!0}{\strut ,} \colorbox{red!0}{\strut in} \colorbox{red!0}{\strut a} \colorbox{red!0}{\strut cowardly} \colorbox{red!0}{\strut fashion} \colorbox{red!0}{\strut ,} \colorbox{red!0}{\strut disowned} \colorbox{red!0}{\strut aRead} \colorbox{red!0}{\strut MoreLouis} \colorbox{red!0}{\strut ,} \colorbox{red!0}{\strut marquis} \colorbox{red!0}{\strut de} \colorbox{red!0}{\strut Fontanescommission} \colorbox{red!0}{\strut appointed} \colorbox{red!0}{\strut to} \colorbox{red!0}{\strut draft} \colorbox{red!0}{\strut the} \colorbox{red!2}{\strut Charte} \colorbox{red!1}{\strut Constitutionnelle} \colorbox{red!0}{\strut ,} \colorbox{red!4}{\strut Louis} \colorbox{red!0}{\strut .} \colorbox{red!0}{\strut s} \colorbox{red!20}{\strut constitution} \colorbox{red!0}{\strut .} \colorbox{red!0}{\strut In} \colorbox{red!0}{\strut 1817} \colorbox{red!0}{\strut he} \colorbox{red!0}{\strut was} \colorbox{red!0}{\strut created} \colorbox{red!0}{\strut a} 
}}}
\end{CJK*}

\begin{CJK*}{UTF8}{gbsn}
{\setlength{\fboxsep}{0pt}\colorbox{white!0}{\parbox{0.9\textwidth}{
\colorbox{red!2}{\strut 1830} \colorbox{red!0}{\strut .} \colorbox{red!4}{\strut French} \colorbox{red!11}{\strut Charter} \colorbox{red!1}{\strut of} \colorbox{red!2}{\strut 1830} \colorbox{red!0}{\strut Related} \colorbox{red!0}{\strut Links} \colorbox{red!0}{\strut .} \colorbox{red!0}{\strut Key} \colorbox{red!0}{\strut DocumentsRelated} \colorbox{red!0}{\strut Links} \colorbox{red!0}{\strut .} \colorbox{red!0}{\strut Francis} \colorbox{red!0}{\strut LieberCollection} \colorbox{red!0}{\strut .} \colorbox{red!1}{\strut Laws} \colorbox{red!0}{\strut ,} \colorbox{red!7}{\strut Charters} \colorbox{red!0}{\strut ,} \colorbox{red!8}{\strut Constitutions} \colorbox{red!0}{\strut ,} \colorbox{red!1}{\strut Bills} \colorbox{red!1}{\strut of} \colorbox{red!0}{\strut RightSource} \colorbox{red!0}{\strut .} \colorbox{red!0}{\strut Appendix} \colorbox{red!0}{\strut to} \colorbox{red!0}{\strut Francis} \colorbox{red!0}{\strut Lieber} \colorbox{red!0}{\strut ,} \colorbox{red!0}{\strut On} \colorbox{red!1}{\strut Civil} \colorbox{red!1}{\strut Liberty} \colorbox{red!0}{\strut and} \colorbox{red!0}{\strut Self-Government,3rd} \colorbox{red!0}{\strut revised} \colorbox{red!0}{\strut edition} \colorbox{red!0}{\strut ,} \colorbox{red!0}{\strut ed} \colorbox{red!0}{\strut .} \colorbox{red!0}{\strut Theodore} \colorbox{red!0}{\strut D.} \colorbox{red!0}{\strut Woolsey} \colorbox{red!0}{\strut .} \colorbox{red!0}{\strut Philadelphia} \colorbox{red!0}{\strut .} \colorbox{red!0}{\strut J.B.} \colorbox{red!0}{\strut Lippincott} \colorbox{red!0}{\strut .} \colorbox{red!0}{\strut Co.} \colorbox{red!0}{\strut ,} \colorbox{red!0}{\strut 1883} \colorbox{red!0}{\strut .} \colorbox{red!0}{\strut .APPENDIX} \colorbox{red!0}{\strut XII.french} \colorbox{red!11}{\strut charter} \colorbox{red!1}{\strut of} \colorbox{red!2}{\strut louis} \colorbox{red!1}{\strut xviii} \colorbox{red!0}{\strut .} \colorbox{red!0}{\strut and} \colorbox{red!0}{\strut that} \colorbox{red!1}{\strut adopted} \colorbox{red!0}{\strut in} \colorbox{red!0}{\strut the} \colorbox{red!0}{\strut year} \colorbox{red!0}{\strut 1830.The} \colorbox{red!1}{\strut following} \colorbox{red!0}{\strut is} \colorbox{red!0}{\strut the} \colorbox{red!11}{\strut charter} \colorbox{red!1}{\strut of} \colorbox{red!2}{\strut 1830} \colorbox{red!0}{\strut ,} \colorbox{red!0}{\strut as} \colorbox{red!0}{\strut I} \colorbox{red!0}{\strut translated} \colorbox{red!0}{\strut it} \colorbox{red!0}{\strut in} \colorbox{red!0}{\strut that} \colorbox{red!0}{\strut year} \colorbox{red!0}{\strut ,} \colorbox{red!0}{\strut for} \colorbox{red!0}{\strut a} \colorbox{red!0}{\strut work} \colorbox{red!1}{\strut published} \colorbox{red!0}{\strut in} \colorbox{red!0}{\strut Boston} \colorbox{red!0}{\strut ,} \colorbox{red!0}{\strut under} \colorbox{red!0}{\strut the} \colorbox{red!0}{\strut title} \colorbox{red!1}{\strut of} \colorbox{red!0}{\strut .} \colorbox{red!1}{\strut Events} \colorbox{red!0}{\strut in} \colorbox{red!1}{\strut Paris} \colorbox{red!0}{\strut during} \colorbox{red!0}{\strut the} \colorbox{red!1}{\strut 26th} \colorbox{red!0}{\strut ,} \colorbox{red!0}{\strut 27th} \colorbox{red!0}{\strut ,} \colorbox{red!1}{\strut 28th} \colorbox{red!0}{\strut and} \colorbox{red!1}{\strut 29th} \colorbox{red!1}{\strut of} \colorbox{red!1}{\strut July} \colorbox{red!0}{\strut .} \colorbox{red!0}{\strut translated} \colorbox{red!0}{\strut from} \colorbox{red!0}{\strut the} \colorbox{red!0}{\strut French.} \colorbox{red!0}{\strut .} \colorbox{red!0}{\strut This} \colorbox{red!11}{\strut charter} \colorbox{red!1}{\strut of} \colorbox{red!1}{\strut August} \colorbox{red!0}{\strut 8} \colorbox{red!0}{\strut ,} \colorbox{red!2}{\strut 1830} \colorbox{red!0}{\strut ,} \colorbox{red!0}{\strut is} \colorbox{red!0}{\strut in} \colorbox{red!1}{\strut substance} \colorbox{red!0}{\strut the} \colorbox{red!11}{\strut charter} \colorbox{red!1}{\strut of} \colorbox{red!2}{\strut Louis} \colorbox{red!1}{\strut XVIII} \colorbox{red!0}{\strut .} \colorbox{red!0}{\strut with} \colorbox{red!0}{\strut such} \colorbox{red!1}{\strut changes} \colorbox{red!0}{\strut as} \colorbox{red!0}{\strut the} \colorbox{red!1}{\strut chambers} \colorbox{red!1}{\strut adopted} \colorbox{red!0}{\strut in} \colorbox{red!0}{\strut favor} \colorbox{red!1}{\strut of} \colorbox{red!1}{\strut liberty} \colorbox{red!0}{\strut .} \colorbox{red!0}{\strut The} \colorbox{red!0}{\strut new} \colorbox{red!1}{\strut articles} \colorbox{red!0}{\strut ,} \colorbox{red!0}{\strut or} \colorbox{red!0}{\strut the} \colorbox{red!0}{\strut amendments} \colorbox{red!1}{\strut of} \colorbox{red!0}{\strut the} \colorbox{red!0}{\strut old} \colorbox{red!0}{\strut ones} \colorbox{red!0}{\strut ,} \colorbox{red!0}{\strut are} \colorbox{red!0}{\strut printed} \colorbox{red!0}{\strut in} \colorbox{red!0}{\strut italics} \colorbox{red!0}{\strut ,} \colorbox{red!0}{\strut and} \colorbox{red!0}{\strut the} \colorbox{red!0}{\strut old} \colorbox{red!0}{\strut readings} \colorbox{red!0}{\strut or} \colorbox{red!3}{\strut suppressed} \colorbox{red!1}{\strut articles} \colorbox{red!0}{\strut are} \colorbox{red!0}{\strut given} \colorbox{red!0}{\strut in} \colorbox{red!0}{\strut notes} \colorbox{red!0}{\strut .} \colorbox{red!0}{\strut so} \colorbox{red!0}{\strut that} \colorbox{red!0}{\strut the} \colorbox{red!0}{\strut paper} \colorbox{red!0}{\strut exhibits} \colorbox{red!0}{\strut both} \colorbox{red!0}{\strut the} \colorbox{red!0}{\strut charters.FRENCH} \colorbox{red!11}{\strut CHARTER} \colorbox{red!1}{\strut OF} \colorbox{red!0}{\strut 1830.The} \colorbox{red!0}{\strut whole} \colorbox{red!1}{\strut preamble} \colorbox{red!1}{\strut of} \colorbox{red!0}{\strut the} \colorbox{red!1}{\strut ancient} \colorbox{red!11}{\strut charter} \colorbox{red!0}{\strut was} \colorbox{red!3}{\strut suppressed} \colorbox{red!0}{\strut ,} \colorbox{red!0}{\strut as} \colorbox{red!0}{\strut containing} \colorbox{red!0}{\strut the} \colorbox{red!0}{\strut principle} \colorbox{red!1}{\strut of} \colorbox{red!0}{\strut concession} \colorbox{red!0}{\strut and} \colorbox{red!0}{\strut octroi} \colorbox{red!0}{\strut .} \colorbox{red!1}{\strut grant} \colorbox{red!0}{\strut .} \colorbox{red!0}{\strut ,} \colorbox{red!0}{\strut incompatible} \colorbox{red!0}{\strut with} \colorbox{red!0}{\strut that} \colorbox{red!1}{\strut of} \colorbox{red!0}{\strut the} \colorbox{red!0}{\strut acknowledgment} \colorbox{red!1}{\strut of} \colorbox{red!1}{\strut national} \colorbox{red!0}{\strut sovereignty.The} \colorbox{red!1}{\strut following} \colorbox{red!0}{\strut is} \colorbox{red!0}{\strut the} \colorbox{red!1}{\strut substitution} \colorbox{red!1}{\strut of} \colorbox{red!0}{\strut the} \colorbox{red!1}{\strut preamble} \colorbox{red!0}{\strut .} \colorbox{red!1}{\strut declaration} \colorbox{red!1}{\strut of} \colorbox{red!0}{\strut the} \colorbox{red!1}{\strut chamber} \colorbox{red!1}{\strut of} \colorbox{red!0}{\strut deputies.The} \colorbox{red!1}{\strut chamber} \colorbox{red!1}{\strut of} \colorbox{red!1}{\strut deputies} \colorbox{red!0}{\strut ,} \colorbox{red!0}{\strut taking} \colorbox{red!0}{\strut into} \colorbox{red!0}{\strut consideration} \colorbox{red!0}{\strut the} \colorbox{red!0}{\strut imperious} \colorbox{red!0}{\strut necessity} \colorbox{red!1}{\strut which} \colorbox{red!0}{\strut results} \colorbox{red!0}{\strut from} \colorbox{red!0}{\strut the} \colorbox{red!1}{\strut events} \colorbox{red!1}{\strut of} \colorbox{red!0}{\strut the} \colorbox{red!1}{\strut 26th} \colorbox{red!0}{\strut ,} \colorbox{red!0}{\strut 27th} \colorbox{red!0}{\strut ,} \colorbox{red!1}{\strut 28th} \colorbox{red!0}{\strut and} \colorbox{red!1}{\strut 29th} \colorbox{red!1}{\strut of} \colorbox{red!1}{\strut July} \colorbox{red!0}{\strut ,} \colorbox{red!0}{\strut and} \colorbox{red!0}{\strut the} \colorbox{red!1}{\strut following} \colorbox{red!0}{\strut days} \colorbox{red!0}{\strut .} \colorbox{red!0}{\strut and} \colorbox{red!0}{\strut from} \colorbox{red!0}{\strut the} \colorbox{red!1}{\strut situation} \colorbox{red!0}{\strut in} \colorbox{red!1}{\strut which} \colorbox{red!2}{\strut France} \colorbox{red!0}{\strut is} \colorbox{red!0}{\strut placed} \colorbox{red!0}{\strut in} \colorbox{red!1}{\strut consequence} \colorbox{red!1}{\strut of} \colorbox{red!0}{\strut the} \colorbox{red!2}{\strut violation} \colorbox{red!1}{\strut of} \colorbox{red!0}{\strut the} \colorbox{red!10}{\strut constitutional} \colorbox{red!11}{\strut charter} \colorbox{red!0}{\strut .} \colorbox{red!0}{\strut Considering} \colorbox{red!0}{\strut ,} \colorbox{red!0}{\strut moreover} \colorbox{red!0}{\strut ,} \colorbox{red!0}{\strut that} \colorbox{red!0}{\strut by} \colorbox{red!0}{\strut this} \colorbox{red!2}{\strut violation} \colorbox{red!0}{\strut ,} \colorbox{red!0}{\strut and} \colorbox{red!0}{\strut the} \colorbox{red!0}{\strut heroic} \colorbox{red!0}{\strut resistance} \colorbox{red!1}{\strut of} \colorbox{red!0}{\strut the} \colorbox{red!0}{\strut citizens} \colorbox{red!1}{\strut of} \colorbox{red!1}{\strut Paris} \colorbox{red!0}{\strut ,} \colorbox{red!0}{\strut his} \colorbox{red!0}{\strut majesty} 
}}}
\end{CJK*}

query: do clouds form in the vab

\begin{CJK*}{UTF8}{gbsn}
{\setlength{\fboxsep}{0pt}\colorbox{white!0}{\parbox{0.9\textwidth}{
\colorbox{red!0}{\strut NASA} \colorbox{red!2}{\strut Vehicle} \colorbox{red!3}{\strut Assembly} \colorbox{red!13}{\strut Building} \colorbox{red!2}{\strut Titusville} \colorbox{red!0}{\strut ,} \colorbox{red!0}{\strut FloridaNASA} \colorbox{red!2}{\strut Vehicle} \colorbox{red!3}{\strut Assembly} \colorbox{red!0}{\strut BuildingA} \colorbox{red!13}{\strut building} \colorbox{red!0}{\strut so} \colorbox{red!1}{\strut large} \colorbox{red!0}{\strut that} \colorbox{red!0}{\strut it} \colorbox{red!0}{\strut has} \colorbox{red!0}{\strut its} \colorbox{red!0}{\strut own} \colorbox{red!0}{\strut weather.Edit} \colorbox{red!0}{\strut EntryAdd} \colorbox{red!0}{\strut PhotoBeen} \colorbox{red!0}{\strut Here} \colorbox{red!0}{\strut ?} \colorbox{red!0}{\strut 691Want} \colorbox{red!0}{\strut to} \colorbox{red!0}{\strut Visit} \colorbox{red!0}{\strut ?} \colorbox{red!0}{\strut 149Exterior} \colorbox{red!0}{\strut view} \colorbox{red!0}{\strut of} \colorbox{red!0}{\strut the} \colorbox{red!2}{\strut Vehicle} \colorbox{red!3}{\strut Assembly} \colorbox{red!13}{\strut Building} \colorbox{red!0}{\strut .} \colorbox{red!0}{\strut http} \colorbox{red!0}{\strut .} \colorbox{red!0}{\strut upload.wikimedia.orgwikipediacomm} \colorbox{red!0}{\strut ...} \colorbox{red!0}{\strut The} \colorbox{red!2}{\strut Vehicle} \colorbox{red!3}{\strut Assembly} \colorbox{red!13}{\strut Building} \colorbox{red!0}{\strut .} \colorbox{red!1}{\strut VAB} \colorbox{red!0}{\strut .} \colorbox{red!0}{\strut at} \colorbox{red!0}{\strut NASA} \colorbox{red!0}{\strut .} \colorbox{red!0}{\strut s} \colorbox{red!1}{\strut Kennedy} \colorbox{red!2}{\strut Space} \colorbox{red!1}{\strut Center} \colorbox{red!0}{\strut in} \colorbox{red!2}{\strut Florida} \colorbox{red!0}{\strut is} \colorbox{red!0}{\strut the} \colorbox{red!0}{\strut world} \colorbox{red!0}{\strut .} \colorbox{red!0}{\strut s} \colorbox{red!0}{\strut fourth} \colorbox{red!12}{\strut largest} \colorbox{red!13}{\strut building} \colorbox{red!0}{\strut by} \colorbox{red!0}{\strut volume} \colorbox{red!0}{\strut .} \colorbox{red!0}{\strut Completed} \colorbox{red!0}{\strut in} \colorbox{red!0}{\strut 1966} \colorbox{red!0}{\strut ,} \colorbox{red!0}{\strut the} \colorbox{red!1}{\strut VAB} \colorbox{red!0}{\strut also} \colorbox{red!0}{\strut holds} \colorbox{red!0}{\strut the} \colorbox{red!0}{\strut record} \colorbox{red!0}{\strut of} \colorbox{red!0}{\strut the} \colorbox{red!12}{\strut largest} \colorbox{red!0}{\strut one-story} \colorbox{red!13}{\strut building} \colorbox{red!0}{\strut in} \colorbox{red!0}{\strut the} \colorbox{red!0}{\strut world} \colorbox{red!0}{\strut and} \colorbox{red!0}{\strut is} \colorbox{red!0}{\strut the} \colorbox{red!0}{\strut tallest} \colorbox{red!13}{\strut building} \colorbox{red!0}{\strut outside} \colorbox{red!0}{\strut an} \colorbox{red!0}{\strut urban} \colorbox{red!1}{\strut center} \colorbox{red!0}{\strut in} \colorbox{red!0}{\strut the} \colorbox{red!0}{\strut United} \colorbox{red!0}{\strut States.Top} \colorbox{red!0}{\strut Places} \colorbox{red!0}{\strut in} \colorbox{red!0}{\strut TitusvilleTitusville} \colorbox{red!0}{\strut ,} \colorbox{red!0}{\strut FloridaAmerican} \colorbox{red!2}{\strut Space} \colorbox{red!0}{\strut Museum28.6105} \colorbox{red!0}{\strut ,} \colorbox{red!0}{\strut -80.8087Titusville} \colorbox{red!0}{\strut ,} \colorbox{red!0}{\strut FloridaWindover} \colorbox{red!0}{\strut Archeological} \colorbox{red!0}{\strut Site28.5386} \colorbox{red!0}{\strut ,} \colorbox{red!0}{\strut -80.8433See} \colorbox{red!0}{\strut more} \colorbox{red!0}{\strut things} \colorbox{red!0}{\strut to} \colorbox{red!0}{\strut do} \colorbox{red!0}{\strut in} \colorbox{red!2}{\strut Titusville} \colorbox{red!0}{\strut .} \colorbox{red!0}{\strut At} \colorbox{red!0}{\strut an} \colorbox{red!0}{\strut astonishing} \colorbox{red!0}{\strut 160} \colorbox{red!0}{\strut meters} \colorbox{red!0}{\strut .} \colorbox{red!0}{\strut 525} \colorbox{red!0}{\strut feet} \colorbox{red!0}{\strut .} \colorbox{red!1}{\strut tall} \colorbox{red!0}{\strut ,} \colorbox{red!0}{\strut 218} \colorbox{red!0}{\strut meters} \colorbox{red!0}{\strut .} \colorbox{red!0}{\strut 716} \colorbox{red!0}{\strut feet} \colorbox{red!0}{\strut .} \colorbox{red!0}{\strut long} \colorbox{red!0}{\strut ,} \colorbox{red!0}{\strut and} \colorbox{red!0}{\strut 158} \colorbox{red!0}{\strut meters} \colorbox{red!0}{\strut .} \colorbox{red!0}{\strut 518} \colorbox{red!0}{\strut feet} \colorbox{red!0}{\strut .} \colorbox{red!0}{\strut wide} \colorbox{red!0}{\strut ,} \colorbox{red!0}{\strut the} \colorbox{red!1}{\strut VAB} \colorbox{red!0}{\strut covers} \colorbox{red!0}{\strut an} \colorbox{red!0}{\strut area} \colorbox{red!0}{\strut of} \colorbox{red!0}{\strut eight} \colorbox{red!0}{\strut acres} \colorbox{red!0}{\strut and} \colorbox{red!0}{\strut encloses} \colorbox{red!0}{\strut a} \colorbox{red!0}{\strut volume} \colorbox{red!0}{\strut of} \colorbox{red!0}{\strut about} \colorbox{red!0}{\strut 3,665,000} \colorbox{red!0}{\strut cubic} \colorbox{red!0}{\strut meters} \colorbox{red!0}{\strut .} \colorbox{red!0}{\strut 129,428,000} \colorbox{red!0}{\strut cubic} \colorbox{red!0}{\strut feet} \colorbox{red!0}{\strut .} \colorbox{red!0}{\strut .} \colorbox{red!0}{\strut To} \colorbox{red!0}{\strut get} \colorbox{red!0}{\strut an} \colorbox{red!0}{\strut idea} \colorbox{red!0}{\strut of} \colorbox{red!2}{\strut how} \colorbox{red!1}{\strut large} \colorbox{red!0}{\strut that} \colorbox{red!0}{\strut is} \colorbox{red!0}{\strut ,} \colorbox{red!0}{\strut the} \colorbox{red!0}{\strut total} \colorbox{red!0}{\strut volume} \colorbox{red!0}{\strut of} \colorbox{red!0}{\strut the} \colorbox{red!1}{\strut VAB} \colorbox{red!0}{\strut is} \colorbox{red!0}{\strut about} \colorbox{red!0}{\strut 3.75} \colorbox{red!0}{\strut times} \colorbox{red!0}{\strut that} \colorbox{red!0}{\strut of} \colorbox{red!0}{\strut Manhattan} \colorbox{red!0}{\strut .} \colorbox{red!0}{\strut s} \colorbox{red!0}{\strut Empire} \colorbox{red!0}{\strut State} \colorbox{red!13}{\strut Building} \colorbox{red!0}{\strut .} \colorbox{red!0}{\strut That} \colorbox{red!0}{\strut .} \colorbox{red!0}{\strut s} \colorbox{red!0}{\strut enough} \colorbox{red!2}{\strut space} \colorbox{red!0}{\strut to} \colorbox{red!0}{\strut fit} \colorbox{red!0}{\strut the} \colorbox{red!0}{\strut volume} \colorbox{red!0}{\strut of} \colorbox{red!0}{\strut Pentagon} \colorbox{red!0}{\strut inside} \colorbox{red!0}{\strut and} \colorbox{red!0}{\strut have} \colorbox{red!0}{\strut plenty} \colorbox{red!0}{\strut of} \colorbox{red!0}{\strut room} \colorbox{red!0}{\strut left} \colorbox{red!0}{\strut over} \colorbox{red!0}{\strut !} \colorbox{red!0}{\strut The} \colorbox{red!1}{\strut VAB} \colorbox{red!0}{\strut is} \colorbox{red!0}{\strut so} \colorbox{red!1}{\strut large} \colorbox{red!0}{\strut ,} \colorbox{red!0}{\strut in} \colorbox{red!0}{\strut fact} \colorbox{red!0}{\strut ,} \colorbox{red!0}{\strut that} \colorbox{red!0}{\strut it} \colorbox{red!0}{\strut has} \colorbox{red!0}{\strut its} \colorbox{red!0}{\strut own} \colorbox{red!0}{\strut weather} \colorbox{red!0}{\strut .} \colorbox{red!0}{\strut On} \colorbox{red!0}{\strut humid} \colorbox{red!0}{\strut days} \colorbox{red!0}{\strut ,} \colorbox{red!0}{\strut rain} \colorbox{red!0}{\strut clouds} \colorbox{red!0}{\strut can} \colorbox{red!0}{\strut form} \colorbox{red!0}{\strut below} \colorbox{red!0}{\strut the} \colorbox{red!0}{\strut ceiling} \colorbox{red!0}{\strut ,} \colorbox{red!0}{\strut requiring} \colorbox{red!0}{\strut about} \colorbox{red!0}{\strut 10,000} \colorbox{red!0}{\strut tons} \colorbox{red!0}{\strut of} \colorbox{red!0}{\strut air} \colorbox{red!0}{\strut conditioning} \colorbox{red!0}{\strut equipment} \colorbox{red!0}{\strut to} \colorbox{red!0}{\strut control} \colorbox{red!0}{\strut the} \colorbox{red!0}{\strut moisture} \colorbox{red!0}{\strut .} \colorbox{red!0}{\strut With} \colorbox{red!0}{\strut this} \colorbox{red!0}{\strut setup} \colorbox{red!0}{\strut ,} \colorbox{red!0}{\strut the} \colorbox{red!0}{\strut total} \colorbox{red!0}{\strut volume} \colorbox{red!0}{\strut of} \colorbox{red!0}{\strut air} \colorbox{red!0}{\strut in} \colorbox{red!0}{\strut the} \colorbox{red!13}{\strut building} \colorbox{red!0}{\strut can} \colorbox{red!0}{\strut be} \colorbox{red!0}{\strut replaced} \colorbox{red!0}{\strut in} \colorbox{red!0}{\strut only} \colorbox{red!0}{\strut one} \colorbox{red!0}{\strut hour.The} \colorbox{red!0}{\strut records} \colorbox{red!0}{\strut held} \colorbox{red!0}{\strut by} \colorbox{red!0}{\strut the} \colorbox{red!1}{\strut VAB} \colorbox{red!0}{\strut are} \colorbox{red!0}{\strut not} \colorbox{red!0}{\strut limited} \colorbox{red!0}{\strut to} \colorbox{red!0}{\strut its} \colorbox{red!0}{\strut interior} \colorbox{red!0}{\strut ,} \colorbox{red!0}{\strut however} \colorbox{red!0}{\strut .} \colorbox{red!0}{\strut The} \colorbox{red!0}{\strut exterior} \colorbox{red!0}{\strut boasts} \colorbox{red!0}{\strut one} \colorbox{red!0}{\strut of} \colorbox{red!0}{\strut the} \colorbox{red!12}{\strut largest} 
}}}
\end{CJK*}

\begin{CJK*}{UTF8}{gbsn}
{\setlength{\fboxsep}{0pt}\colorbox{white!0}{\parbox{0.9\textwidth}{
\colorbox{red!9}{\strut Cloud} \colorbox{red!4}{\strut Formation} \colorbox{red!0}{\strut .} \colorbox{red!0}{\strut A} \colorbox{red!0}{\strut Brief} \colorbox{red!0}{\strut Explanation} \colorbox{red!0}{\strut of} \colorbox{red!3}{\strut How} \colorbox{red!1}{\strut Do} \colorbox{red!9}{\strut Clouds} \colorbox{red!6}{\strut Form} \colorbox{red!9}{\strut Cloud} \colorbox{red!4}{\strut Formation} \colorbox{red!0}{\strut .} \colorbox{red!0}{\strut A} \colorbox{red!0}{\strut Brief} \colorbox{red!0}{\strut Explanation} \colorbox{red!0}{\strut of} \colorbox{red!3}{\strut How} \colorbox{red!1}{\strut Do} \colorbox{red!9}{\strut Clouds} \colorbox{red!0}{\strut FormClouds} \colorbox{red!0}{\strut are} \colorbox{red!0}{\strut an} \colorbox{red!0}{\strut interesting} \colorbox{red!2}{\strut natural} \colorbox{red!1}{\strut phenomenon} \colorbox{red!0}{\strut which} \colorbox{red!0}{\strut one} \colorbox{red!0}{\strut can} \colorbox{red!0}{\strut observe} \colorbox{red!0}{\strut everyday} \colorbox{red!0}{\strut .} \colorbox{red!0}{\strut Interestingly} \colorbox{red!0}{\strut ,} \colorbox{red!0}{\strut there} \colorbox{red!0}{\strut are} \colorbox{red!0}{\strut a} \colorbox{red!0}{\strut variety} \colorbox{red!0}{\strut of} \colorbox{red!9}{\strut clouds} \colorbox{red!0}{\strut and} \colorbox{red!0}{\strut they} \colorbox{red!0}{\strut are} \colorbox{red!0}{\strut all} \colorbox{red!1}{\strut made} \colorbox{red!0}{\strut up} \colorbox{red!0}{\strut of} \colorbox{red!0}{\strut the} \colorbox{red!0}{\strut same} \colorbox{red!0}{\strut substances} \colorbox{red!0}{\strut ,} \colorbox{red!1}{\strut water} \colorbox{red!0}{\strut or} \colorbox{red!0}{\strut ice} \colorbox{red!0}{\strut or} \colorbox{red!0}{\strut both} \colorbox{red!0}{\strut ,} \colorbox{red!0}{\strut in} \colorbox{red!0}{\strut a} \colorbox{red!1}{\strut condensed} \colorbox{red!0}{\strut form.Weather} \colorbox{red!0}{\strut can} \colorbox{red!0}{\strut be} \colorbox{red!0}{\strut predicted} \colorbox{red!0}{\strut to} \colorbox{red!0}{\strut a} \colorbox{red!0}{\strut certain} \colorbox{red!0}{\strut level} \colorbox{red!0}{\strut by} \colorbox{red!0}{\strut studying} \colorbox{red!0}{\strut the} \colorbox{red!9}{\strut clouds} \colorbox{red!0}{\strut .} \colorbox{red!0}{\strut Any} \colorbox{red!1}{\strut planet} \colorbox{red!0}{\strut of} \colorbox{red!0}{\strut the} \colorbox{red!0}{\strut solar} \colorbox{red!1}{\strut system} \colorbox{red!0}{\strut that} \colorbox{red!0}{\strut has} \colorbox{red!1}{\strut atmosphere} \colorbox{red!0}{\strut will} \colorbox{red!0}{\strut definitely} \colorbox{red!0}{\strut have} \colorbox{red!9}{\strut clouds} \colorbox{red!0}{\strut .} \colorbox{red!0}{\strut Besides} \colorbox{red!1}{\strut Earth} \colorbox{red!0}{\strut ,} \colorbox{red!9}{\strut clouds} \colorbox{red!1}{\strut exist} \colorbox{red!0}{\strut on} \colorbox{red!0}{\strut other} \colorbox{red!1}{\strut planets} \colorbox{red!0}{\strut like} \colorbox{red!0}{\strut Venus} \colorbox{red!0}{\strut ,} \colorbox{red!0}{\strut Mars} \colorbox{red!0}{\strut ,} \colorbox{red!0}{\strut Jupiter} \colorbox{red!0}{\strut and} \colorbox{red!0}{\strut Saturn} \colorbox{red!0}{\strut as} \colorbox{red!0}{\strut well} \colorbox{red!0}{\strut .} \colorbox{red!0}{\strut They} \colorbox{red!0}{\strut are} \colorbox{red!0}{\strut nothing} \colorbox{red!0}{\strut but} \colorbox{red!1}{\strut condensed} \colorbox{red!0}{\strut droplets} \colorbox{red!0}{\strut suspended} \colorbox{red!0}{\strut in} \colorbox{red!0}{\strut the} \colorbox{red!1}{\strut atmosphere} \colorbox{red!0}{\strut above} \colorbox{red!0}{\strut the} \colorbox{red!1}{\strut surface} \colorbox{red!0}{\strut of} \colorbox{red!0}{\strut the} \colorbox{red!0}{\strut planet.Processes} \colorbox{red!0}{\strut of} \colorbox{red!9}{\strut Cloud} \colorbox{red!0}{\strut FormationClouds} \colorbox{red!0}{\strut are} \colorbox{red!7}{\strut formed} \colorbox{red!2}{\strut when} \colorbox{red!0}{\strut the} \colorbox{red!1}{\strut air} \colorbox{red!0}{\strut in} \colorbox{red!0}{\strut the} \colorbox{red!1}{\strut atmosphere} \colorbox{red!0}{\strut is} \colorbox{red!0}{\strut so} \colorbox{red!0}{\strut saturated} \colorbox{red!0}{\strut with} \colorbox{red!1}{\strut water} \colorbox{red!1}{\strut vapor} \colorbox{red!0}{\strut that} \colorbox{red!0}{\strut it} \colorbox{red!0}{\strut can} \colorbox{red!0}{\strut not} \colorbox{red!0}{\strut hold} \colorbox{red!0}{\strut any} \colorbox{red!0}{\strut more} \colorbox{red!0}{\strut of} \colorbox{red!0}{\strut it} \colorbox{red!0}{\strut .} \colorbox{red!0}{\strut This} \colorbox{red!0}{\strut may} \colorbox{red!1}{\strut happen} \colorbox{red!0}{\strut under} \colorbox{red!0}{\strut two} \colorbox{red!0}{\strut conditions} \colorbox{red!0}{\strut viz.} \colorbox{red!0}{\strut ,} \colorbox{red!0}{\strut the} \colorbox{red!1}{\strut air} \colorbox{red!0}{\strut has} \colorbox{red!0}{\strut cooled} \colorbox{red!0}{\strut down} \colorbox{red!0}{\strut to} \colorbox{red!0}{\strut a} \colorbox{red!0}{\strut point} \colorbox{red!1}{\strut where} \colorbox{red!1}{\strut condensation} \colorbox{red!0}{\strut is} \colorbox{red!0}{\strut bound} \colorbox{red!0}{\strut to} \colorbox{red!1}{\strut take} \colorbox{red!0}{\strut place} \colorbox{red!0}{\strut because} \colorbox{red!0}{\strut the} \colorbox{red!1}{\strut air} \colorbox{red!0}{\strut has} \colorbox{red!0}{\strut expanded} \colorbox{red!0}{\strut enough} \colorbox{red!0}{\strut and} \colorbox{red!0}{\strut has} \colorbox{red!0}{\strut lost} \colorbox{red!0}{\strut a} \colorbox{red!0}{\strut considerable} \colorbox{red!0}{\strut amount} \colorbox{red!0}{\strut of} \colorbox{red!0}{\strut its} \colorbox{red!1}{\strut moisture} \colorbox{red!0}{\strut content} \colorbox{red!0}{\strut .} \colorbox{red!0}{\strut And} \colorbox{red!0}{\strut the} \colorbox{red!0}{\strut quantity} \colorbox{red!0}{\strut of} \colorbox{red!1}{\strut water} \colorbox{red!0}{\strut in} \colorbox{red!0}{\strut the} \colorbox{red!1}{\strut atmosphere} \colorbox{red!0}{\strut had} \colorbox{red!0}{\strut increased} \colorbox{red!0}{\strut to} \colorbox{red!0}{\strut such} \colorbox{red!0}{\strut an} \colorbox{red!0}{\strut extent} \colorbox{red!0}{\strut that} \colorbox{red!0}{\strut the} \colorbox{red!1}{\strut air} \colorbox{red!0}{\strut has} \colorbox{red!0}{\strut no} \colorbox{red!0}{\strut capacity} \colorbox{red!0}{\strut to} \colorbox{red!0}{\strut hold} \colorbox{red!0}{\strut any} \colorbox{red!0}{\strut more} \colorbox{red!0}{\strut of} \colorbox{red!0}{\strut it} \colorbox{red!0}{\strut .} \colorbox{red!0}{\strut The} \colorbox{red!0}{\strut amount} \colorbox{red!0}{\strut of} \colorbox{red!1}{\strut water} \colorbox{red!0}{\strut in} \colorbox{red!0}{\strut the} \colorbox{red!1}{\strut atmosphere} \colorbox{red!0}{\strut may} \colorbox{red!1}{\strut rise} \colorbox{red!0}{\strut due} \colorbox{red!0}{\strut to} \colorbox{red!0}{\strut factors} \colorbox{red!0}{\strut such} \colorbox{red!0}{\strut as} \colorbox{red!0}{\strut evaporation} \colorbox{red!0}{\strut .} \colorbox{red!0}{\strut Though} \colorbox{red!9}{\strut cloud} \colorbox{red!4}{\strut formation} \colorbox{red!0}{\strut may} \colorbox{red!0}{\strut seem} \colorbox{red!0}{\strut as} \colorbox{red!0}{\strut simple} \colorbox{red!0}{\strut as} \colorbox{red!1}{\strut condensation} \colorbox{red!0}{\strut of} \colorbox{red!1}{\strut water} \colorbox{red!1}{\strut vapor} \colorbox{red!0}{\strut in} \colorbox{red!1}{\strut air} \colorbox{red!0}{\strut ,} \colorbox{red!0}{\strut in} \colorbox{red!0}{\strut reality} \colorbox{red!0}{\strut the} \colorbox{red!0}{\strut entire} \colorbox{red!1}{\strut process} \colorbox{red!0}{\strut is} \colorbox{red!0}{\strut much} \colorbox{red!0}{\strut more} \colorbox{red!0}{\strut complicated} \colorbox{red!0}{\strut .} \colorbox{red!0}{\strut For} \colorbox{red!0}{\strut the} \colorbox{red!1}{\strut water} \colorbox{red!1}{\strut vapor} \colorbox{red!0}{\strut to} \colorbox{red!1}{\strut condense} \colorbox{red!0}{\strut at} \colorbox{red!0}{\strut a} \colorbox{red!0}{\strut particular} \colorbox{red!0}{\strut point} \colorbox{red!0}{\strut and} \colorbox{red!6}{\strut form} \colorbox{red!9}{\strut clouds} \colorbox{red!0}{\strut ,} \colorbox{red!0}{\strut the} \colorbox{red!0}{\strut moist} \colorbox{red!1}{\strut air} \colorbox{red!0}{\strut that} \colorbox{red!0}{\strut rises} \colorbox{red!0}{\strut above} \colorbox{red!0}{\strut the} \colorbox{red!1}{\strut earth} \colorbox{red!0}{\strut s} \colorbox{red!1}{\strut surface} \colorbox{red!0}{\strut has} \colorbox{red!0}{\strut to} \colorbox{red!0}{\strut undergo} \colorbox{red!0}{\strut a} \colorbox{red!0}{\strut series} \colorbox{red!0}{\strut of} \colorbox{red!1}{\strut processes} \colorbox{red!0}{\strut .} \colorbox{red!9}{\strut Clouds} \colorbox{red!0}{\strut thus} \colorbox{red!0}{\strut ,} \colorbox{red!0}{\strut may} \colorbox{red!0}{\strut be} \colorbox{red!7}{\strut formed} \colorbox{red!0}{\strut in} \colorbox{red!0}{\strut five} \colorbox{red!1}{\strut different} \colorbox{red!1}{\strut ways} 
}}}
\end{CJK*}

query: when allocating service department costs, the method which ignores serviced provided to other service departments is called

\begin{CJK*}{UTF8}{gbsn}
{\setlength{\fboxsep}{0pt}\colorbox{white!0}{\parbox{0.9\textwidth}{
\colorbox{red!0}{\strut Examining} \colorbox{red!0}{\strut methods} \colorbox{red!0}{\strut for} \colorbox{red!4}{\strut allocating} \colorbox{red!7}{\strut overhead} \colorbox{red!6}{\strut costs} \colorbox{red!0}{\strut .} \colorbox{red!0}{\strut Examining} \colorbox{red!0}{\strut methods} \colorbox{red!0}{\strut for} \colorbox{red!4}{\strut allocating} \colorbox{red!7}{\strut overhead} \colorbox{red!0}{\strut costsPrintReference} \colorbox{red!0}{\strut thisPublished} \colorbox{red!0}{\strut .} \colorbox{red!0}{\strut 23rd} \colorbox{red!0}{\strut March} \colorbox{red!0}{\strut ,} \colorbox{red!0}{\strut 2015Disclaimer} \colorbox{red!0}{\strut .} \colorbox{red!0}{\strut This} \colorbox{red!0}{\strut essay} \colorbox{red!0}{\strut has} \colorbox{red!0}{\strut been} \colorbox{red!0}{\strut submitted} \colorbox{red!0}{\strut by} \colorbox{red!0}{\strut a} \colorbox{red!0}{\strut student} \colorbox{red!0}{\strut .} \colorbox{red!0}{\strut This} \colorbox{red!0}{\strut is} \colorbox{red!0}{\strut not} \colorbox{red!0}{\strut an} \colorbox{red!0}{\strut example} \colorbox{red!0}{\strut of} \colorbox{red!0}{\strut the} \colorbox{red!0}{\strut work} \colorbox{red!0}{\strut written} \colorbox{red!0}{\strut by} \colorbox{red!0}{\strut our} \colorbox{red!0}{\strut professional} \colorbox{red!0}{\strut essay} \colorbox{red!0}{\strut writers.Any} \colorbox{red!0}{\strut opinions} \colorbox{red!0}{\strut ,} \colorbox{red!0}{\strut findings} \colorbox{red!0}{\strut ,} \colorbox{red!0}{\strut conclusions} \colorbox{red!0}{\strut or} \colorbox{red!0}{\strut recommendations} \colorbox{red!0}{\strut expressed} \colorbox{red!0}{\strut in} \colorbox{red!0}{\strut this} \colorbox{red!0}{\strut material} \colorbox{red!0}{\strut are} \colorbox{red!0}{\strut those} \colorbox{red!0}{\strut of} \colorbox{red!0}{\strut the} \colorbox{red!0}{\strut authors} \colorbox{red!0}{\strut and} \colorbox{red!0}{\strut do} \colorbox{red!0}{\strut not} \colorbox{red!0}{\strut necessarily} \colorbox{red!0}{\strut reflect} \colorbox{red!0}{\strut the} \colorbox{red!0}{\strut views} \colorbox{red!0}{\strut of} \colorbox{red!0}{\strut UK} \colorbox{red!0}{\strut Essays.Overhead} \colorbox{red!6}{\strut cost} \colorbox{red!0}{\strut is} \colorbox{red!0}{\strut an} \colorbox{red!0}{\strut ongoing} \colorbox{red!1}{\strut expense} \colorbox{red!0}{\strut of} \colorbox{red!0}{\strut operating} \colorbox{red!0}{\strut a} \colorbox{red!0}{\strut business} \colorbox{red!0}{\strut and} \colorbox{red!0}{\strut is} \colorbox{red!0}{\strut usually} \colorbox{red!0}{\strut used} \colorbox{red!0}{\strut to} \colorbox{red!0}{\strut group} \colorbox{red!0}{\strut expenses} \colorbox{red!0}{\strut that} \colorbox{red!0}{\strut are} \colorbox{red!0}{\strut necessary} \colorbox{red!0}{\strut to} \colorbox{red!0}{\strut the} \colorbox{red!0}{\strut continued} \colorbox{red!0}{\strut functioning} \colorbox{red!0}{\strut of} \colorbox{red!0}{\strut the} \colorbox{red!0}{\strut business} \colorbox{red!0}{\strut ,} \colorbox{red!0}{\strut but} \colorbox{red!0}{\strut can} \colorbox{red!0}{\strut not} \colorbox{red!0}{\strut be} \colorbox{red!0}{\strut immediately} \colorbox{red!0}{\strut associated} \colorbox{red!0}{\strut with} \colorbox{red!0}{\strut the} \colorbox{red!0}{\strut productsservices} \colorbox{red!0}{\strut being} \colorbox{red!0}{\strut offered} \colorbox{red!0}{\strut as} \colorbox{red!0}{\strut in} \colorbox{red!0}{\strut the} \colorbox{red!6}{\strut costs} \colorbox{red!0}{\strut do} \colorbox{red!0}{\strut not} \colorbox{red!0}{\strut directly} \colorbox{red!0}{\strut generate} \colorbox{red!0}{\strut profits.Overhead} \colorbox{red!6}{\strut cost} \colorbox{red!0}{\strut includes} \colorbox{red!0}{\strut indirect} \colorbox{red!1}{\strut product} \colorbox{red!6}{\strut cost} \colorbox{red!0}{\strut or} \colorbox{red!0}{\strut indirect} \colorbox{red!6}{\strut cost} \colorbox{red!0}{\strut of} \colorbox{red!0}{\strut responsibility} \colorbox{red!0}{\strut centre} \colorbox{red!0}{\strut .} \colorbox{red!0}{\strut Indirect} \colorbox{red!1}{\strut product} \colorbox{red!6}{\strut cost} \colorbox{red!0}{\strut is} \colorbox{red!0}{\strut known} \colorbox{red!0}{\strut as} \colorbox{red!1}{\strut manufacturing} \colorbox{red!7}{\strut overhead} \colorbox{red!0}{\strut whereas} \colorbox{red!0}{\strut indirect} \colorbox{red!6}{\strut cost} \colorbox{red!0}{\strut of} \colorbox{red!0}{\strut responsibility} \colorbox{red!0}{\strut centre} \colorbox{red!0}{\strut is} \colorbox{red!0}{\strut known} \colorbox{red!0}{\strut as} \colorbox{red!0}{\strut non-manufacturing} \colorbox{red!6}{\strut cost} \colorbox{red!0}{\strut .} \colorbox{red!1}{\strut Manufacturing} \colorbox{red!7}{\strut overhead} \colorbox{red!0}{\strut is} \colorbox{red!0}{\strut those} \colorbox{red!1}{\strut manufacturing} \colorbox{red!6}{\strut costs} \colorbox{red!0}{\strut that} \colorbox{red!0}{\strut are} \colorbox{red!0}{\strut incurred} \colorbox{red!0}{\strut to} \colorbox{red!0}{\strut a} \colorbox{red!0}{\strut variety} \colorbox{red!0}{\strut of} \colorbox{red!1}{\strut products} \colorbox{red!0}{\strut .} \colorbox{red!0}{\strut It} \colorbox{red!0}{\strut can} \colorbox{red!0}{\strut not} \colorbox{red!0}{\strut be} \colorbox{red!0}{\strut traced} \colorbox{red!0}{\strut to} \colorbox{red!0}{\strut individual} \colorbox{red!1}{\strut products} \colorbox{red!0}{\strut like} \colorbox{red!0}{\strut depreciation} \colorbox{red!0}{\strut and} \colorbox{red!0}{\strut insurance} \colorbox{red!0}{\strut of} \colorbox{red!1}{\strut manufacturing} \colorbox{red!0}{\strut equipment} \colorbox{red!0}{\strut ,} \colorbox{red!6}{\strut cost} \colorbox{red!0}{\strut of} \colorbox{red!0}{\strut occupying} \colorbox{red!0}{\strut ,} \colorbox{red!0}{\strut managing} \colorbox{red!0}{\strut and} \colorbox{red!0}{\strut maintaining} \colorbox{red!0}{\strut a} \colorbox{red!1}{\strut production} \colorbox{red!0}{\strut facility} \colorbox{red!0}{\strut .} \colorbox{red!1}{\strut Manufacturing} \colorbox{red!7}{\strut overhead} \colorbox{red!0}{\strut is} \colorbox{red!0}{\strut the} \colorbox{red!6}{\strut cost} \colorbox{red!0}{\strut that} \colorbox{red!0}{\strut could} \colorbox{red!0}{\strut be} \colorbox{red!0}{\strut traced} \colorbox{red!0}{\strut to} \colorbox{red!0}{\strut individual} \colorbox{red!1}{\strut product} \colorbox{red!0}{\strut but} \colorbox{red!0}{\strut it} \colorbox{red!0}{\strut is} \colorbox{red!0}{\strut not} \colorbox{red!0}{\strut worth} \colorbox{red!0}{\strut the} \colorbox{red!0}{\strut trouble} \colorbox{red!0}{\strut to} \colorbox{red!0}{\strut like} \colorbox{red!6}{\strut cost} \colorbox{red!0}{\strut of} \colorbox{red!0}{\strut lubricants} \colorbox{red!0}{\strut and} \colorbox{red!0}{\strut glue} \colorbox{red!0}{\strut used} \colorbox{red!0}{\strut .} \colorbox{red!1}{\strut Manufacturing} \colorbox{red!7}{\strut overhead} \colorbox{red!0}{\strut also} \colorbox{red!0}{\strut include} \colorbox{red!6}{\strut cost} \colorbox{red!0}{\strut that} \colorbox{red!0}{\strut is} \colorbox{red!0}{\strut more} \colorbox{red!0}{\strut appropriately} \colorbox{red!0}{\strut to} \colorbox{red!0}{\strut be} \colorbox{red!0}{\strut treated} \colorbox{red!0}{\strut as} \colorbox{red!6}{\strut cost} \colorbox{red!0}{\strut of} \colorbox{red!0}{\strut all} \colorbox{red!0}{\strut outputs} \colorbox{red!0}{\strut like} \colorbox{red!0}{\strut overtime} \colorbox{red!0}{\strut premium} \colorbox{red!0}{\strut ,} \colorbox{red!6}{\strut cost} \colorbox{red!0}{\strut of} \colorbox{red!0}{\strut idle} \colorbox{red!0}{\strut time} \colorbox{red!0}{\strut ,} \colorbox{red!0}{\strut utilities} \colorbox{red!0}{\strut cost.Non-manufacturing} \colorbox{red!6}{\strut cost} \colorbox{red!0}{\strut includes} \colorbox{red!0}{\strut customer} \colorbox{red!0}{\strut service} \colorbox{red!0}{\strut ,} \colorbox{red!0}{\strut marketing} \colorbox{red!0}{\strut and} \colorbox{red!0}{\strut research} \colorbox{red!0}{\strut .} \colorbox{red!0}{\strut development} \colorbox{red!0}{\strut cost.ALLOCATING} \colorbox{red!7}{\strut OVERHEAD} \colorbox{red!0}{\strut COSTSNormally} \colorbox{red!0}{\strut ,} \colorbox{red!0}{\strut only} \colorbox{red!1}{\strut manufacturing} \colorbox{red!7}{\strut overhead} \colorbox{red!0}{\strut is} \colorbox{red!0}{\strut allocated} \colorbox{red!0}{\strut to} \colorbox{red!1}{\strut products} \colorbox{red!0}{\strut .} \colorbox{red!0}{\strut However} \colorbox{red!0}{\strut ,} \colorbox{red!0}{\strut depending} \colorbox{red!0}{\strut on} \colorbox{red!0}{\strut the} \colorbox{red!0}{\strut industry} \colorbox{red!0}{\strut the} \colorbox{red!0}{\strut business} \colorbox{red!0}{\strut is} \colorbox{red!0}{\strut in} \colorbox{red!0}{\strut and} \colorbox{red!0}{\strut to} \colorbox{red!0}{\strut obtain} \colorbox{red!0}{\strut more} \colorbox{red!0}{\strut comprehensive} \colorbox{red!0}{\strut estimates} \colorbox{red!0}{\strut of} \colorbox{red!1}{\strut product} \colorbox{red!6}{\strut cost} \colorbox{red!0}{\strut ,} \colorbox{red!0}{\strut management} \colorbox{red!0}{\strut accountant} \colorbox{red!0}{\strut may} \colorbox{red!3}{\strut allocate} \colorbox{red!0}{\strut non-manufacturing} \colorbox{red!6}{\strut cost} \colorbox{red!0}{\strut to} \colorbox{red!1}{\strut products} \colorbox{red!0}{\strut .} \colorbox{red!0}{\strut One} \colorbox{red!0}{\strut example} \colorbox{red!0}{\strut is} 
}}}
\end{CJK*}

\begin{CJK*}{UTF8}{gbsn}
{\setlength{\fboxsep}{0pt}\colorbox{white!0}{\parbox{0.9\textwidth}{
\colorbox{red!7}{\strut Reciprocal} \colorbox{red!6}{\strut Method} \colorbox{red!0}{\strut of} \colorbox{red!5}{\strut Cost} \colorbox{red!1}{\strut Allocation} \colorbox{red!0}{\strut .} \colorbox{red!1}{\strut Service} \colorbox{red!1}{\strut Department} \colorbox{red!0}{\strut Costing} \colorbox{red!7}{\strut Reciprocal} \colorbox{red!6}{\strut Method} \colorbox{red!0}{\strut of} \colorbox{red!5}{\strut Cost} \colorbox{red!1}{\strut Allocation} \colorbox{red!0}{\strut .} \colorbox{red!1}{\strut Service} \colorbox{red!1}{\strut Department} \colorbox{red!0}{\strut CostingDefinition} \colorbox{red!0}{\strut .} \colorbox{red!7}{\strut Reciprocal} \colorbox{red!6}{\strut method} \colorbox{red!0}{\strut is} \colorbox{red!0}{\strut a} \colorbox{red!6}{\strut method} \colorbox{red!0}{\strut of} \colorbox{red!2}{\strut allocating} \colorbox{red!1}{\strut service} \colorbox{red!1}{\strut department} \colorbox{red!4}{\strut costs} \colorbox{red!0}{\strut to} \colorbox{red!0}{\strut other} \colorbox{red!1}{\strut departments} \colorbox{red!0}{\strut that} \colorbox{red!0}{\strut gives} \colorbox{red!0}{\strut full} \colorbox{red!0}{\strut recognition} \colorbox{red!0}{\strut to} \colorbox{red!0}{\strut interdepartmental} \colorbox{red!0}{\strut services.Explanation} \colorbox{red!0}{\strut .} \colorbox{red!0}{\strut The} \colorbox{red!7}{\strut reciprocal} \colorbox{red!6}{\strut method} \colorbox{red!0}{\strut gives} \colorbox{red!0}{\strut full} \colorbox{red!0}{\strut recognition} \colorbox{red!0}{\strut to} \colorbox{red!0}{\strut interdepartmental} \colorbox{red!1}{\strut services} \colorbox{red!0}{\strut .} \colorbox{red!0}{\strut Under} \colorbox{red!0}{\strut the} \colorbox{red!0}{\strut step} \colorbox{red!6}{\strut method} \colorbox{red!0}{\strut ,} \colorbox{red!0}{\strut only} \colorbox{red!0}{\strut partial} \colorbox{red!0}{\strut recognition} \colorbox{red!0}{\strut of} \colorbox{red!0}{\strut interdepartmental} \colorbox{red!1}{\strut services} \colorbox{red!0}{\strut is} \colorbox{red!0}{\strut possible} \colorbox{red!0}{\strut .} \colorbox{red!0}{\strut The} \colorbox{red!0}{\strut step} \colorbox{red!6}{\strut method} \colorbox{red!0}{\strut always} \colorbox{red!1}{\strut allocates} \colorbox{red!4}{\strut costs} \colorbox{red!0}{\strut forward} \colorbox{red!0}{\strut never} \colorbox{red!0}{\strut backward} \colorbox{red!0}{\strut .} \colorbox{red!0}{\strut The} \colorbox{red!7}{\strut reciprocal} \colorbox{red!6}{\strut method} \colorbox{red!0}{\strut ,} \colorbox{red!0}{\strut by} \colorbox{red!0}{\strut contrast} \colorbox{red!0}{\strut ,} \colorbox{red!1}{\strut allocates} \colorbox{red!1}{\strut service} \colorbox{red!1}{\strut department} \colorbox{red!4}{\strut costs} \colorbox{red!0}{\strut in} \colorbox{red!0}{\strut both} \colorbox{red!0}{\strut directions} \colorbox{red!0}{\strut .} \colorbox{red!0}{\strut The} \colorbox{red!7}{\strut reciprocal} \colorbox{red!1}{\strut allocation} \colorbox{red!0}{\strut requires} \colorbox{red!0}{\strut the} \colorbox{red!0}{\strut use} \colorbox{red!0}{\strut of} \colorbox{red!0}{\strut simultaneous} \colorbox{red!1}{\strut equations} \colorbox{red!0}{\strut .} \colorbox{red!0}{\strut This} \colorbox{red!6}{\strut method} \colorbox{red!0}{\strut is} \colorbox{red!0}{\strut also} \colorbox{red!0}{\strut known} \colorbox{red!0}{\strut as} \colorbox{red!0}{\strut algebraic} \colorbox{red!6}{\strut method} \colorbox{red!0}{\strut and} \colorbox{red!0}{\strut simultaneous} \colorbox{red!1}{\strut equations} \colorbox{red!0}{\strut method.Under} \colorbox{red!0}{\strut this} \colorbox{red!6}{\strut method} \colorbox{red!0}{\strut the} \colorbox{red!0}{\strut true} \colorbox{red!5}{\strut cost} \colorbox{red!0}{\strut of} \colorbox{red!0}{\strut the} \colorbox{red!1}{\strut service} \colorbox{red!1}{\strut departments} \colorbox{red!0}{\strut are} \colorbox{red!0}{\strut computed} \colorbox{red!0}{\strut first} \colorbox{red!0}{\strut with} \colorbox{red!0}{\strut the} \colorbox{red!0}{\strut help} \colorbox{red!0}{\strut of} \colorbox{red!0}{\strut simultaneous} \colorbox{red!1}{\strut equations} \colorbox{red!0}{\strut and} \colorbox{red!0}{\strut these} \colorbox{red!0}{\strut are} \colorbox{red!0}{\strut then} \colorbox{red!0}{\strut distributed} \colorbox{red!0}{\strut to} \colorbox{red!0}{\strut producing} \colorbox{red!1}{\strut departments} \colorbox{red!0}{\strut on} \colorbox{red!0}{\strut the} \colorbox{red!0}{\strut basis} \colorbox{red!0}{\strut of} \colorbox{red!0}{\strut given} \colorbox{red!0}{\strut percentage} \colorbox{red!0}{\strut or} \colorbox{red!0}{\strut ratio} \colorbox{red!0}{\strut .} \colorbox{red!0}{\strut Remember} \colorbox{red!0}{\strut that} \colorbox{red!0}{\strut true} \colorbox{red!5}{\strut cost} \colorbox{red!0}{\strut of} \colorbox{red!0}{\strut the} \colorbox{red!1}{\strut service} \colorbox{red!1}{\strut department} \colorbox{red!0}{\strut means} \colorbox{red!0}{\strut the} \colorbox{red!5}{\strut cost} \colorbox{red!0}{\strut of} \colorbox{red!0}{\strut the} \colorbox{red!1}{\strut service} \colorbox{red!1}{\strut department} \colorbox{red!0}{\strut which} \colorbox{red!0}{\strut includes} \colorbox{red!0}{\strut original} \colorbox{red!5}{\strut cost} \colorbox{red!0}{\strut of} \colorbox{red!0}{\strut the} \colorbox{red!1}{\strut department} \colorbox{red!0}{\strut plus} \colorbox{red!0}{\strut the} \colorbox{red!0}{\strut share} \colorbox{red!0}{\strut of} \colorbox{red!0}{\strut the} \colorbox{red!0}{\strut other} \colorbox{red!1}{\strut service} \colorbox{red!1}{\strut department} \colorbox{red!0}{\strut .} \colorbox{red!0}{\strut The} \colorbox{red!0}{\strut main} \colorbox{red!0}{\strut advantage} \colorbox{red!0}{\strut of} \colorbox{red!0}{\strut this} \colorbox{red!6}{\strut method} \colorbox{red!0}{\strut is} \colorbox{red!0}{\strut to} \colorbox{red!0}{\strut have} \colorbox{red!0}{\strut an} \colorbox{red!0}{\strut accurate} \colorbox{red!1}{\strut distribution} \colorbox{red!0}{\strut in} \colorbox{red!0}{\strut a} \colorbox{red!0}{\strut single} \colorbox{red!0}{\strut step} \colorbox{red!0}{\strut in} \colorbox{red!0}{\strut the} \colorbox{red!1}{\strut distribution} \colorbox{red!0}{\strut summary} \colorbox{red!0}{\strut .} \colorbox{red!0}{\strut .} \colorbox{red!0}{\strut Example} \colorbox{red!0}{\strut .} \colorbox{red!0}{\strut A} \colorbox{red!0}{\strut company} \colorbox{red!0}{\strut has} \colorbox{red!0}{\strut two} \colorbox{red!1}{\strut service} \colorbox{red!0}{\strut and} \colorbox{red!0}{\strut two} \colorbox{red!0}{\strut producing} \colorbox{red!1}{\strut departments} \colorbox{red!0}{\strut .} \colorbox{red!0}{\strut The} \colorbox{red!0}{\strut two} \colorbox{red!1}{\strut service} \colorbox{red!1}{\strut departments} \colorbox{red!0}{\strut serve} \colorbox{red!0}{\strut not} \colorbox{red!0}{\strut only} \colorbox{red!0}{\strut to} \colorbox{red!0}{\strut producing} \colorbox{red!1}{\strut departments} \colorbox{red!0}{\strut but} \colorbox{red!0}{\strut also} \colorbox{red!0}{\strut to} \colorbox{red!0}{\strut each} \colorbox{red!0}{\strut other} \colorbox{red!0}{\strut .} \colorbox{red!0}{\strut The} \colorbox{red!0}{\strut departmental} \colorbox{red!0}{\strut estimates} \colorbox{red!0}{\strut for} \colorbox{red!0}{\strut the} \colorbox{red!0}{\strut next} \colorbox{red!0}{\strut year} \colorbox{red!0}{\strut are} \colorbox{red!0}{\strut as} \colorbox{red!0}{\strut follows.Producing} \colorbox{red!1}{\strut departments} \colorbox{red!0}{\strut .} \colorbox{red!0}{\strut A} \colorbox{red!0}{\strut B} \colorbox{red!1}{\strut Service} \colorbox{red!1}{\strut departments} \colorbox{red!0}{\strut .} \colorbox{red!0}{\strut X} \colorbox{red!0}{\strut Y} \colorbox{red!0}{\strut 50,000} \colorbox{red!0}{\strut 40,000} \colorbox{red!0}{\strut 10,000} \colorbox{red!0}{\strut 8,800The} \colorbox{red!1}{\strut service} \colorbox{red!1}{\strut departments} \colorbox{red!4}{\strut costs} \colorbox{red!0}{\strut are} \colorbox{red!0}{\strut to} \colorbox{red!0}{\strut be} \colorbox{red!0}{\strut distributed} \colorbox{red!0}{\strut as} \colorbox{red!0}{\strut under} \colorbox{red!0}{\strut .} \colorbox{red!5}{\strut Cost} \colorbox{red!0}{\strut of} \colorbox{red!0}{\strut X} \colorbox{red!0}{\strut .} \colorbox{red!0}{\strut 50} \colorbox{red!0}{\strut .} \colorbox{red!0}{\strut to} \colorbox{red!0}{\strut A} \colorbox{red!0}{\strut ,} \colorbox{red!0}{\strut 40} \colorbox{red!0}{\strut .} \colorbox{red!0}{\strut to} \colorbox{red!0}{\strut B} \colorbox{red!0}{\strut ,} \colorbox{red!0}{\strut and} \colorbox{red!0}{\strut 10} \colorbox{red!0}{\strut .} \colorbox{red!0}{\strut to} \colorbox{red!0}{\strut Y} \colorbox{red!5}{\strut Cost} \colorbox{red!0}{\strut of} \colorbox{red!0}{\strut Y} \colorbox{red!0}{\strut .} \colorbox{red!0}{\strut 40} \colorbox{red!0}{\strut .} \colorbox{red!0}{\strut to} \colorbox{red!0}{\strut A} \colorbox{red!0}{\strut ,} \colorbox{red!0}{\strut 40} \colorbox{red!0}{\strut .} \colorbox{red!0}{\strut to} \colorbox{red!0}{\strut B} \colorbox{red!0}{\strut ,} \colorbox{red!0}{\strut and} \colorbox{red!0}{\strut 20} \colorbox{red!0}{\strut .} \colorbox{red!0}{\strut to} \colorbox{red!0}{\strut XRequired} \colorbox{red!0}{\strut .} \colorbox{red!0}{\strut Transfer} 
}}}
\end{CJK*}

query: define user maintenance

\begin{CJK*}{UTF8}{gbsn}
{\setlength{\fboxsep}{0pt}\colorbox{white!0}{\parbox{0.9\textwidth}{
\colorbox{red!9}{\strut Automatic} \colorbox{red!11}{\strut Maintenance} \colorbox{red!9}{\strut Automatic} \colorbox{red!0}{\strut MaintenanceMaintenance} \colorbox{red!0}{\strut activity} \colorbox{red!0}{\strut refers} \colorbox{red!0}{\strut to} \colorbox{red!0}{\strut an} \colorbox{red!0}{\strut application} \colorbox{red!0}{\strut or} \colorbox{red!0}{\strut process} \colorbox{red!0}{\strut that} \colorbox{red!0}{\strut helps} \colorbox{red!0}{\strut maintain} \colorbox{red!0}{\strut the} \colorbox{red!0}{\strut health} \colorbox{red!0}{\strut and} \colorbox{red!0}{\strut performance} \colorbox{red!0}{\strut of} \colorbox{red!0}{\strut a} \colorbox{red!1}{\strut Windows} \colorbox{red!1}{\strut PC} \colorbox{red!0}{\strut .} \colorbox{red!11}{\strut Maintenance} \colorbox{red!0}{\strut includes} \colorbox{red!0}{\strut keeping} \colorbox{red!1}{\strut Windows} \colorbox{red!0}{\strut and} \colorbox{red!0}{\strut applications} \colorbox{red!0}{\strut up-to-date} \colorbox{red!0}{\strut ,} \colorbox{red!0}{\strut checking} \colorbox{red!0}{\strut security} \colorbox{red!0}{\strut ,} \colorbox{red!0}{\strut and} \colorbox{red!0}{\strut running} \colorbox{red!0}{\strut scans} \colorbox{red!0}{\strut for} \colorbox{red!0}{\strut malware} \colorbox{red!0}{\strut .} \colorbox{red!1}{\strut Windows} \colorbox{red!9}{\strut Automatic} \colorbox{red!1}{\strut Management} \colorbox{red!0}{\strut .} \colorbox{red!1}{\strut WAM} \colorbox{red!0}{\strut .} \colorbox{red!0}{\strut is} \colorbox{red!0}{\strut a} \colorbox{red!0}{\strut set} \colorbox{red!0}{\strut of} \colorbox{red!0}{\strut enhancements} \colorbox{red!0}{\strut to} \colorbox{red!0}{\strut the} \colorbox{red!1}{\strut Task} \colorbox{red!1}{\strut Scheduler} \colorbox{red!0}{\strut API} \colorbox{red!0}{\strut you} \colorbox{red!0}{\strut can} \colorbox{red!0}{\strut use} \colorbox{red!0}{\strut to} \colorbox{red!0}{\strut link} \colorbox{red!0}{\strut your} \colorbox{red!0}{\strut applications} \colorbox{red!0}{\strut into} \colorbox{red!0}{\strut the} \colorbox{red!1}{\strut Windows} \colorbox{red!11}{\strut maintenance} \colorbox{red!1}{\strut schedule} \colorbox{red!0}{\strut .} \colorbox{red!0}{\strut Specifically} \colorbox{red!0}{\strut ,} \colorbox{red!1}{\strut WAM} \colorbox{red!0}{\strut allows} \colorbox{red!0}{\strut you} \colorbox{red!0}{\strut to} \colorbox{red!0}{\strut add} \colorbox{red!0}{\strut activities} \colorbox{red!0}{\strut that} \colorbox{red!0}{\strut require} \colorbox{red!0}{\strut regular} \colorbox{red!1}{\strut scheduling} \colorbox{red!0}{\strut ,} \colorbox{red!0}{\strut but} \colorbox{red!0}{\strut do} \colorbox{red!0}{\strut not} \colorbox{red!0}{\strut have} \colorbox{red!0}{\strut exact} \colorbox{red!0}{\strut time} \colorbox{red!0}{\strut requirements} \colorbox{red!0}{\strut .} \colorbox{red!0}{\strut Instead} \colorbox{red!0}{\strut ,} \colorbox{red!1}{\strut WAM} \colorbox{red!0}{\strut relies} \colorbox{red!0}{\strut on} \colorbox{red!0}{\strut the} \colorbox{red!0}{\strut operating} \colorbox{red!1}{\strut system} \colorbox{red!0}{\strut to} \colorbox{red!0}{\strut choose} \colorbox{red!0}{\strut the} \colorbox{red!0}{\strut appropriate} \colorbox{red!0}{\strut time} \colorbox{red!0}{\strut to} \colorbox{red!0}{\strut activate} \colorbox{red!0}{\strut the} \colorbox{red!1}{\strut task} \colorbox{red!0}{\strut throughout} \colorbox{red!0}{\strut the} \colorbox{red!0}{\strut day} \colorbox{red!0}{\strut .} \colorbox{red!0}{\strut The} \colorbox{red!1}{\strut system} \colorbox{red!0}{\strut chooses} \colorbox{red!0}{\strut those} \colorbox{red!0}{\strut times} \colorbox{red!0}{\strut based} \colorbox{red!0}{\strut on} \colorbox{red!0}{\strut minimal} \colorbox{red!0}{\strut impact} \colorbox{red!0}{\strut to} \colorbox{red!0}{\strut the} \colorbox{red!0}{\strut user} \colorbox{red!0}{\strut ,} \colorbox{red!1}{\strut PC} \colorbox{red!0}{\strut performance} \colorbox{red!0}{\strut ,} \colorbox{red!0}{\strut and} \colorbox{red!0}{\strut energy} \colorbox{red!0}{\strut efficiency.How} \colorbox{red!1}{\strut Scheduled} \colorbox{red!11}{\strut Maintenance} \colorbox{red!0}{\strut WorksWindows} \colorbox{red!9}{\strut Automatic} \colorbox{red!11}{\strut Maintenance} \colorbox{red!0}{\strut minimizes} \colorbox{red!0}{\strut impact} \colorbox{red!0}{\strut to} \colorbox{red!0}{\strut the} \colorbox{red!1}{\strut PC} \colorbox{red!0}{\strut by} \colorbox{red!1}{\strut scheduling} \colorbox{red!11}{\strut maintenance} \colorbox{red!0}{\strut only} \colorbox{red!0}{\strut when} \colorbox{red!0}{\strut the} \colorbox{red!1}{\strut PC} \colorbox{red!0}{\strut is} \colorbox{red!0}{\strut on} \colorbox{red!0}{\strut and} \colorbox{red!0}{\strut idle} \colorbox{red!0}{\strut .} \colorbox{red!0}{\strut By} \colorbox{red!0}{\strut default} \colorbox{red!0}{\strut ,} \colorbox{red!0}{\strut the} \colorbox{red!1}{\strut system} \colorbox{red!0}{\strut performs} \colorbox{red!11}{\strut maintenance} \colorbox{red!0}{\strut daily} \colorbox{red!0}{\strut ,} \colorbox{red!0}{\strut starting} \colorbox{red!0}{\strut at} \colorbox{red!0}{\strut 3} \colorbox{red!0}{\strut AM} \colorbox{red!0}{\strut .} \colorbox{red!0}{\strut .} \colorbox{red!0}{\strut Note} \colorbox{red!0}{\strut that} \colorbox{red!0}{\strut the} \colorbox{red!0}{\strut user} \colorbox{red!0}{\strut may} \colorbox{red!0}{\strut re-schedule} \colorbox{red!0}{\strut when} \colorbox{red!0}{\strut the} \colorbox{red!11}{\strut maintenance} \colorbox{red!0}{\strut occurs} \colorbox{red!0}{\strut .} \colorbox{red!0}{\strut .} \colorbox{red!0}{\strut This} \colorbox{red!0}{\strut daily} \colorbox{red!0}{\strut session} \colorbox{red!0}{\strut is} \colorbox{red!0}{\strut limited} \colorbox{red!0}{\strut to} \colorbox{red!0}{\strut a} \colorbox{red!0}{\strut maximum} \colorbox{red!0}{\strut duration} \colorbox{red!0}{\strut of} \colorbox{red!0}{\strut 1} \colorbox{red!0}{\strut hour} \colorbox{red!0}{\strut per} \colorbox{red!0}{\strut attempt} \colorbox{red!0}{\strut .} \colorbox{red!0}{\strut If} \colorbox{red!0}{\strut the} \colorbox{red!0}{\strut user} \colorbox{red!0}{\strut is} \colorbox{red!0}{\strut actively} \colorbox{red!0}{\strut using} \colorbox{red!0}{\strut the} \colorbox{red!0}{\strut machine} \colorbox{red!0}{\strut ,} \colorbox{red!0}{\strut the} \colorbox{red!1}{\strut system} \colorbox{red!0}{\strut defers} \colorbox{red!11}{\strut maintenance} \colorbox{red!0}{\strut until} \colorbox{red!0}{\strut a} \colorbox{red!0}{\strut later} \colorbox{red!0}{\strut time} \colorbox{red!0}{\strut .} \colorbox{red!0}{\strut The} \colorbox{red!1}{\strut system} \colorbox{red!0}{\strut also} \colorbox{red!0}{\strut suspends} \colorbox{red!0}{\strut any} \colorbox{red!0}{\strut executing} \colorbox{red!11}{\strut maintenance} \colorbox{red!1}{\strut task} \colorbox{red!0}{\strut if} \colorbox{red!0}{\strut the} \colorbox{red!0}{\strut user} \colorbox{red!0}{\strut returns} \colorbox{red!0}{\strut to} \colorbox{red!0}{\strut the} \colorbox{red!0}{\strut PC.The} \colorbox{red!1}{\strut system} \colorbox{red!0}{\strut restarts} \colorbox{red!0}{\strut a} \colorbox{red!0}{\strut suspended} \colorbox{red!11}{\strut maintenance} \colorbox{red!1}{\strut task} \colorbox{red!0}{\strut during} \colorbox{red!0}{\strut the} \colorbox{red!0}{\strut next} \colorbox{red!0}{\strut idle} \colorbox{red!0}{\strut period} \colorbox{red!0}{\strut .} \colorbox{red!0}{\strut however} \colorbox{red!0}{\strut ,} \colorbox{red!0}{\strut the} \colorbox{red!1}{\strut system} \colorbox{red!0}{\strut will} \colorbox{red!0}{\strut not} \colorbox{red!0}{\strut suspend} \colorbox{red!0}{\strut any} \colorbox{red!1}{\strut task} \colorbox{red!0}{\strut marked} \colorbox{red!0}{\strut as} \colorbox{red!0}{\strut critical} \colorbox{red!0}{\strut .} \colorbox{red!0}{\strut Instead} \colorbox{red!0}{\strut ,} \colorbox{red!0}{\strut the} \colorbox{red!1}{\strut system} \colorbox{red!0}{\strut allows} \colorbox{red!0}{\strut a} \colorbox{red!0}{\strut critical} \colorbox{red!1}{\strut task} \colorbox{red!0}{\strut to} \colorbox{red!0}{\strut complete} \colorbox{red!0}{\strut ,} \colorbox{red!0}{\strut regardless} \colorbox{red!0}{\strut of} \colorbox{red!0}{\strut user} \colorbox{red!0}{\strut action.Due} \colorbox{red!0}{\strut to} \colorbox{red!0}{\strut the} \colorbox{red!0}{\strut nature} \colorbox{red!0}{\strut of} \colorbox{red!1}{\strut scheduling} \colorbox{red!0}{\strut ,} \colorbox{red!0}{\strut some} \colorbox{red!1}{\strut scheduled} \colorbox{red!0}{\strut tasks} \colorbox{red!0}{\strut may} \colorbox{red!0}{\strut not} \colorbox{red!0}{\strut finish} \colorbox{red!0}{\strut .} \colorbox{red!0}{\strut perhaps} \colorbox{red!0}{\strut there} \colorbox{red!0}{\strut are} \colorbox{red!0}{\strut too} \colorbox{red!0}{\strut many} \colorbox{red!1}{\strut scheduled} \colorbox{red!0}{\strut events} \colorbox{red!0}{\strut to} \colorbox{red!0}{\strut fit} \colorbox{red!0}{\strut in} \colorbox{red!0}{\strut the} \colorbox{red!0}{\strut 1} \colorbox{red!0}{\strut hour} \colorbox{red!11}{\strut maintenance} \colorbox{red!1}{\strut window} \colorbox{red!0}{\strut ,} \colorbox{red!0}{\strut or} \colorbox{red!0}{\strut maybe} \colorbox{red!0}{\strut the} \colorbox{red!0}{\strut computer} 
}}}
\end{CJK*}

\begin{CJK*}{UTF8}{gbsn}
{\setlength{\fboxsep}{0pt}\colorbox{white!0}{\parbox{0.9\textwidth}{
\colorbox{red!0}{\strut User-defined} \colorbox{red!9}{\strut function} \colorbox{red!0}{\strut .} \colorbox{red!0}{\strut User-defined} \colorbox{red!0}{\strut functionFrom} \colorbox{red!0}{\strut Wikipedia} \colorbox{red!0}{\strut ,} \colorbox{red!0}{\strut the} \colorbox{red!0}{\strut free} \colorbox{red!0}{\strut encyclopedianavigation} \colorbox{red!0}{\strut searchA} \colorbox{red!0}{\strut user-defined} \colorbox{red!9}{\strut function} \colorbox{red!0}{\strut .} \colorbox{red!1}{\strut UDF} \colorbox{red!0}{\strut .} \colorbox{red!0}{\strut is} \colorbox{red!0}{\strut a} \colorbox{red!9}{\strut function} \colorbox{red!0}{\strut provided} \colorbox{red!0}{\strut by} \colorbox{red!0}{\strut the} \colorbox{red!8}{\strut user} \colorbox{red!0}{\strut of} \colorbox{red!0}{\strut a} \colorbox{red!1}{\strut program} \colorbox{red!0}{\strut or} \colorbox{red!0}{\strut environment} \colorbox{red!0}{\strut ,} \colorbox{red!0}{\strut in} \colorbox{red!0}{\strut a} \colorbox{red!0}{\strut context} \colorbox{red!1}{\strut where} \colorbox{red!0}{\strut the} \colorbox{red!0}{\strut usual} \colorbox{red!0}{\strut assumption} \colorbox{red!0}{\strut is} \colorbox{red!0}{\strut that} \colorbox{red!9}{\strut functions} \colorbox{red!0}{\strut are} \colorbox{red!0}{\strut built} \colorbox{red!0}{\strut into} \colorbox{red!0}{\strut the} \colorbox{red!1}{\strut program} \colorbox{red!0}{\strut or} \colorbox{red!0}{\strut environment.Contents} \colorbox{red!0}{\strut .} \colorbox{red!0}{\strut hide} \colorbox{red!0}{\strut .} \colorbox{red!0}{\strut 1} \colorbox{red!0}{\strut BASIC} \colorbox{red!0}{\strut language2} \colorbox{red!0}{\strut Databases2.1} \colorbox{red!1}{\strut SQL} \colorbox{red!0}{\strut Server} \colorbox{red!0}{\strut 20002.2} \colorbox{red!0}{\strut Apache} \colorbox{red!0}{\strut Hive3} \colorbox{red!0}{\strut References4} \colorbox{red!0}{\strut External} \colorbox{red!0}{\strut linksBASIC} \colorbox{red!1}{\strut language} \colorbox{red!0}{\strut .} \colorbox{red!0}{\strut edit} \colorbox{red!0}{\strut .} \colorbox{red!0}{\strut In} \colorbox{red!0}{\strut some} \colorbox{red!0}{\strut old} \colorbox{red!0}{\strut implementations} \colorbox{red!0}{\strut of} \colorbox{red!0}{\strut the} \colorbox{red!0}{\strut BASIC} \colorbox{red!1}{\strut programming} \colorbox{red!1}{\strut language} \colorbox{red!0}{\strut ,} \colorbox{red!0}{\strut user-defined} \colorbox{red!9}{\strut functions} \colorbox{red!0}{\strut are} \colorbox{red!9}{\strut defined} \colorbox{red!0}{\strut using} \colorbox{red!0}{\strut the} \colorbox{red!0}{\strut .} \colorbox{red!0}{\strut .} \colorbox{red!0}{\strut DEF} \colorbox{red!0}{\strut FN} \colorbox{red!0}{\strut .} \colorbox{red!0}{\strut .} \colorbox{red!0}{\strut syntax} \colorbox{red!0}{\strut .} \colorbox{red!0}{\strut More} \colorbox{red!0}{\strut modern} \colorbox{red!0}{\strut dialects} \colorbox{red!0}{\strut of} \colorbox{red!0}{\strut BASIC} \colorbox{red!0}{\strut are} \colorbox{red!0}{\strut influenced} \colorbox{red!0}{\strut by} \colorbox{red!0}{\strut the} \colorbox{red!0}{\strut structured} \colorbox{red!1}{\strut programming} \colorbox{red!0}{\strut paradigm} \colorbox{red!0}{\strut ,} \colorbox{red!1}{\strut where} \colorbox{red!0}{\strut most} \colorbox{red!0}{\strut or} \colorbox{red!0}{\strut all} \colorbox{red!0}{\strut of} \colorbox{red!0}{\strut the} \colorbox{red!0}{\strut code} \colorbox{red!0}{\strut is} \colorbox{red!0}{\strut written} \colorbox{red!0}{\strut as} \colorbox{red!0}{\strut user-defined} \colorbox{red!9}{\strut functions} \colorbox{red!0}{\strut or} \colorbox{red!0}{\strut procedures} \colorbox{red!0}{\strut ,} \colorbox{red!0}{\strut and} \colorbox{red!0}{\strut the} \colorbox{red!0}{\strut concept} \colorbox{red!0}{\strut becomes} \colorbox{red!0}{\strut practically} \colorbox{red!0}{\strut redundant.Databases} \colorbox{red!0}{\strut .} \colorbox{red!0}{\strut edit} \colorbox{red!0}{\strut .} \colorbox{red!0}{\strut In} \colorbox{red!0}{\strut relational} \colorbox{red!1}{\strut database} \colorbox{red!0}{\strut management} \colorbox{red!0}{\strut systems} \colorbox{red!0}{\strut ,} \colorbox{red!0}{\strut a} \colorbox{red!0}{\strut user-defined} \colorbox{red!9}{\strut function} \colorbox{red!0}{\strut provides} \colorbox{red!0}{\strut a} \colorbox{red!0}{\strut mechanism} \colorbox{red!0}{\strut for} \colorbox{red!0}{\strut extending} \colorbox{red!0}{\strut the} \colorbox{red!9}{\strut functionality} \colorbox{red!0}{\strut of} \colorbox{red!0}{\strut the} \colorbox{red!1}{\strut database} \colorbox{red!0}{\strut server} \colorbox{red!0}{\strut by} \colorbox{red!0}{\strut adding} \colorbox{red!0}{\strut a} \colorbox{red!9}{\strut function} \colorbox{red!0}{\strut ,} \colorbox{red!0}{\strut that} \colorbox{red!0}{\strut can} \colorbox{red!0}{\strut be} \colorbox{red!0}{\strut evaluated} \colorbox{red!0}{\strut in} \colorbox{red!0}{\strut standard} \colorbox{red!0}{\strut query} \colorbox{red!1}{\strut language} \colorbox{red!0}{\strut .} \colorbox{red!0}{\strut usually} \colorbox{red!1}{\strut SQL} \colorbox{red!0}{\strut .} \colorbox{red!0}{\strut statements} \colorbox{red!0}{\strut .} \colorbox{red!0}{\strut The} \colorbox{red!1}{\strut SQL} \colorbox{red!0}{\strut standard} \colorbox{red!0}{\strut distinguishes} \colorbox{red!0}{\strut between} \colorbox{red!1}{\strut scalar} \colorbox{red!0}{\strut and} \colorbox{red!1}{\strut table} \colorbox{red!9}{\strut functions} \colorbox{red!0}{\strut .} \colorbox{red!0}{\strut A} \colorbox{red!1}{\strut scalar} \colorbox{red!9}{\strut function} \colorbox{red!0}{\strut returns} \colorbox{red!0}{\strut only} \colorbox{red!0}{\strut a} \colorbox{red!0}{\strut single} \colorbox{red!0}{\strut value} \colorbox{red!0}{\strut .} \colorbox{red!0}{\strut or} \colorbox{red!0}{\strut NULL} \colorbox{red!0}{\strut .} \colorbox{red!0}{\strut ,} \colorbox{red!0}{\strut whereas} \colorbox{red!0}{\strut a} \colorbox{red!1}{\strut table} \colorbox{red!9}{\strut function} \colorbox{red!0}{\strut returns} \colorbox{red!0}{\strut a} \colorbox{red!0}{\strut .} \colorbox{red!0}{\strut relational} \colorbox{red!0}{\strut .} \colorbox{red!1}{\strut table} \colorbox{red!0}{\strut comprising} \colorbox{red!0}{\strut zero} \colorbox{red!0}{\strut or} \colorbox{red!0}{\strut more} \colorbox{red!0}{\strut rows} \colorbox{red!0}{\strut ,} \colorbox{red!0}{\strut each} \colorbox{red!0}{\strut row} \colorbox{red!0}{\strut with} \colorbox{red!0}{\strut one} \colorbox{red!0}{\strut or} \colorbox{red!0}{\strut more} \colorbox{red!0}{\strut columns.User-defined} \colorbox{red!9}{\strut functions} \colorbox{red!0}{\strut in} \colorbox{red!1}{\strut SQL} \colorbox{red!0}{\strut are} \colorbox{red!0}{\strut declared} \colorbox{red!0}{\strut using} \colorbox{red!0}{\strut the} \colorbox{red!1}{\strut CREATE} \colorbox{red!9}{\strut FUNCTION} \colorbox{red!0}{\strut statement} \colorbox{red!0}{\strut .} \colorbox{red!0}{\strut For} \colorbox{red!0}{\strut example} \colorbox{red!0}{\strut ,} \colorbox{red!0}{\strut a} \colorbox{red!9}{\strut function} \colorbox{red!0}{\strut that} \colorbox{red!0}{\strut converts} \colorbox{red!1}{\strut Celsius} \colorbox{red!0}{\strut to} \colorbox{red!0}{\strut Fahrenheit} \colorbox{red!0}{\strut might} \colorbox{red!0}{\strut be} \colorbox{red!0}{\strut declared} \colorbox{red!0}{\strut like} \colorbox{red!0}{\strut this} \colorbox{red!0}{\strut .} \colorbox{red!1}{\strut CREATE} \colorbox{red!9}{\strut FUNCTION} \colorbox{red!0}{\strut dbo} \colorbox{red!0}{\strut .} \colorbox{red!0}{\strut CtoF} \colorbox{red!0}{\strut .} \colorbox{red!1}{\strut Celsius} \colorbox{red!0}{\strut FLOAT} \colorbox{red!0}{\strut .} \colorbox{red!0}{\strut RETURNS} \colorbox{red!0}{\strut FLOATRETURN} \colorbox{red!0}{\strut .} \colorbox{red!1}{\strut Celsius} \colorbox{red!0}{\strut .} \colorbox{red!0}{\strut 1} \colorbox{red!0}{\strut .} \colorbox{red!0}{\strut 8} \colorbox{red!0}{\strut .} \colorbox{red!0}{\strut .} \colorbox{red!0}{\strut 32Once} \colorbox{red!0}{\strut created} \colorbox{red!0}{\strut ,} \colorbox{red!0}{\strut a} \colorbox{red!0}{\strut user-defined} \colorbox{red!9}{\strut function} \colorbox{red!0}{\strut may} \colorbox{red!0}{\strut be} \colorbox{red!0}{\strut used} \colorbox{red!0}{\strut in} \colorbox{red!0}{\strut expressions} \colorbox{red!0}{\strut in} \colorbox{red!1}{\strut SQL} \colorbox{red!0}{\strut statements} \colorbox{red!0}{\strut .} \colorbox{red!0}{\strut For} \colorbox{red!0}{\strut example} \colorbox{red!0}{\strut ,} \colorbox{red!0}{\strut it} \colorbox{red!0}{\strut can} \colorbox{red!0}{\strut be} \colorbox{red!0}{\strut invoked} \colorbox{red!1}{\strut where} \colorbox{red!0}{\strut most} \colorbox{red!0}{\strut other} \colorbox{red!0}{\strut intrinsic} \colorbox{red!9}{\strut functions} \colorbox{red!0}{\strut are} \colorbox{red!0}{\strut allowed} \colorbox{red!0}{\strut .} \colorbox{red!0}{\strut This} \colorbox{red!0}{\strut also} \colorbox{red!0}{\strut includes} \colorbox{red!0}{\strut SELECT} \colorbox{red!0}{\strut statements} \colorbox{red!0}{\strut ,} \colorbox{red!1}{\strut where} \colorbox{red!0}{\strut the} \colorbox{red!9}{\strut function} \colorbox{red!0}{\strut can} \colorbox{red!0}{\strut be} \colorbox{red!0}{\strut used} \colorbox{red!0}{\strut against} 
}}}
\end{CJK*}

query: mia nrt distance

\begin{CJK*}{UTF8}{gbsn}
{\setlength{\fboxsep}{0pt}\colorbox{white!0}{\parbox{0.9\textwidth}{
\colorbox{red!0}{\strut Distance} \colorbox{red!0}{\strut from} \colorbox{red!14}{\strut Miami} \colorbox{red!0}{\strut International} \colorbox{red!0}{\strut Airport} \colorbox{red!0}{\strut .} \colorbox{red!0}{\strut MIA} \colorbox{red!0}{\strut .} \colorbox{red!0}{\strut to} \colorbox{red!1}{\strut Narita} \colorbox{red!0}{\strut International} \colorbox{red!0}{\strut Airport} \colorbox{red!0}{\strut .} \colorbox{red!1}{\strut NRT} \colorbox{red!0}{\strut .} \colorbox{red!0}{\strut Distance} \colorbox{red!0}{\strut from} \colorbox{red!14}{\strut Miami} \colorbox{red!0}{\strut International} \colorbox{red!0}{\strut Airport} \colorbox{red!0}{\strut .} \colorbox{red!0}{\strut MIA} \colorbox{red!0}{\strut .} \colorbox{red!0}{\strut to} \colorbox{red!1}{\strut Narita} \colorbox{red!0}{\strut International} \colorbox{red!0}{\strut Airport} \colorbox{red!0}{\strut .} \colorbox{red!1}{\strut NRT} \colorbox{red!0}{\strut .} \colorbox{red!0}{\strut The} \colorbox{red!2}{\strut flight} \colorbox{red!0}{\strut distance} \colorbox{red!0}{\strut from} \colorbox{red!14}{\strut Miami} \colorbox{red!0}{\strut International} \colorbox{red!0}{\strut Airport} \colorbox{red!0}{\strut to} \colorbox{red!1}{\strut Narita} \colorbox{red!0}{\strut International} \colorbox{red!0}{\strut Airport} \colorbox{red!0}{\strut is} \colorbox{red!0}{\strut 7437} \colorbox{red!0}{\strut miles} \colorbox{red!0}{\strut .} \colorbox{red!0}{\strut 11968} \colorbox{red!0}{\strut kilometers} \colorbox{red!0}{\strut .} \colorbox{red!0}{\strut 6462} \colorbox{red!0}{\strut nautical} \colorbox{red!0}{\strut miles.Search} \colorbox{red!0}{\strut airportsSearch} \colorbox{red!0}{\strut by} \colorbox{red!0}{\strut airport} \colorbox{red!0}{\strut name} \colorbox{red!0}{\strut ,} \colorbox{red!0}{\strut city} \colorbox{red!0}{\strut or} \colorbox{red!0}{\strut IATA} \colorbox{red!0}{\strut airport} \colorbox{red!0}{\strut code.From} \colorbox{red!0}{\strut AirportTo} \colorbox{red!0}{\strut AirportMultiple} \colorbox{red!0}{\strut airportsAdd} \colorbox{red!0}{\strut AirportRemove} \colorbox{red!0}{\strut AirportDistanceFrom} \colorbox{red!0}{\strut -} \colorbox{red!0}{\strut ToMiami} \colorbox{red!0}{\strut .} \colorbox{red!0}{\strut MIA} \colorbox{red!0}{\strut .} \colorbox{red!0}{\strut -} \colorbox{red!15}{\strut Tokyo} \colorbox{red!0}{\strut .} \colorbox{red!1}{\strut NRT} \colorbox{red!0}{\strut .} \colorbox{red!0}{\strut mi7437km11968NM6462MapABFlight} \colorbox{red!0}{\strut durationEstimated} \colorbox{red!2}{\strut flight} \colorbox{red!14}{\strut time} \colorbox{red!0}{\strut from} \colorbox{red!14}{\strut Miami} \colorbox{red!0}{\strut International} \colorbox{red!0}{\strut Airport} \colorbox{red!0}{\strut .} \colorbox{red!0}{\strut MIA} \colorbox{red!0}{\strut .} \colorbox{red!0}{\strut to} \colorbox{red!1}{\strut Narita} \colorbox{red!0}{\strut International} \colorbox{red!0}{\strut Airport} \colorbox{red!0}{\strut .} \colorbox{red!1}{\strut NRT} \colorbox{red!0}{\strut .} \colorbox{red!0}{\strut is} \colorbox{red!0}{\strut 14} \colorbox{red!0}{\strut hours} \colorbox{red!0}{\strut 34} \colorbox{red!0}{\strut minutes.Time} \colorbox{red!13}{\strut difference} \colorbox{red!0}{\strut and} \colorbox{red!0}{\strut current} \colorbox{red!0}{\strut local} \colorbox{red!0}{\strut timesThe} \colorbox{red!14}{\strut time} \colorbox{red!13}{\strut difference} \colorbox{red!0}{\strut between} \colorbox{red!14}{\strut Miami} \colorbox{red!0}{\strut and} \colorbox{red!15}{\strut Tokyo} \colorbox{red!0}{\strut is} \colorbox{red!0}{\strut 13} \colorbox{red!0}{\strut hours} \colorbox{red!0}{\strut .} \colorbox{red!15}{\strut Tokyo} \colorbox{red!0}{\strut is} \colorbox{red!0}{\strut 13} \colorbox{red!0}{\strut hours} \colorbox{red!0}{\strut ahead} \colorbox{red!0}{\strut of} \colorbox{red!0}{\strut Miami.Time} \colorbox{red!0}{\strut DifferenceMiamiTokyoMiami205308} \colorbox{red!0}{\strut EDTFriday} \colorbox{red!0}{\strut ,} \colorbox{red!0}{\strut April} \colorbox{red!0}{\strut 6th} \colorbox{red!0}{\strut 2018Tokyo095308} \colorbox{red!0}{\strut JSTSaturday} \colorbox{red!0}{\strut ,} \colorbox{red!0}{\strut April} \colorbox{red!0}{\strut 7th} \colorbox{red!0}{\strut 2018Airport} \colorbox{red!0}{\strut informationA} \colorbox{red!14}{\strut Miami} \colorbox{red!0}{\strut International} \colorbox{red!0}{\strut AirportCity} \colorbox{red!0}{\strut .} \colorbox{red!0}{\strut MiamiCountry} \colorbox{red!0}{\strut .} \colorbox{red!0}{\strut United} \colorbox{red!0}{\strut StatesIATA} \colorbox{red!0}{\strut Code} \colorbox{red!0}{\strut .} \colorbox{red!0}{\strut MIAICAO} \colorbox{red!0}{\strut Code} \colorbox{red!0}{\strut .} \colorbox{red!0}{\strut KMIACoordinates} \colorbox{red!0}{\strut .} \colorbox{red!0}{\strut 254735N} \colorbox{red!0}{\strut ,} \colorbox{red!0}{\strut 801726WB} \colorbox{red!1}{\strut Narita} \colorbox{red!0}{\strut International} \colorbox{red!0}{\strut AirportCity} \colorbox{red!0}{\strut .} \colorbox{red!0}{\strut TokyoCountry} \colorbox{red!0}{\strut .} \colorbox{red!0}{\strut JapanIATA} \colorbox{red!0}{\strut Code} \colorbox{red!0}{\strut .} \colorbox{red!0}{\strut NRTICAO} \colorbox{red!0}{\strut Code} \colorbox{red!0}{\strut .} \colorbox{red!0}{\strut RJAACoordinates} \colorbox{red!0}{\strut .} \colorbox{red!0}{\strut 354552N} \colorbox{red!0}{\strut ,} \colorbox{red!0}{\strut 140239EFrequent} \colorbox{red!0}{\strut Flyer} \colorbox{red!0}{\strut Miles} \colorbox{red!0}{\strut Calculator} \colorbox{red!0}{\strut ,} \colorbox{red!0}{\strut MIA} \colorbox{red!0}{\strut -} \colorbox{red!0}{\strut NRTElite} \colorbox{red!0}{\strut level} \colorbox{red!0}{\strut bonus} \colorbox{red!0}{\strut .} \colorbox{red!0}{\strut .} \colorbox{red!0}{\strut .} \colorbox{red!0}{\strut .} \colorbox{red!0}{\strut Booking} \colorbox{red!0}{\strut class} \colorbox{red!0}{\strut bonus} \colorbox{red!0}{\strut .} \colorbox{red!0}{\strut .} \colorbox{red!0}{\strut .} \colorbox{red!0}{\strut .} \colorbox{red!0}{\strut Air} \colorbox{red!0}{\strut miles7437Elite} \colorbox{red!0}{\strut level} \colorbox{red!0}{\strut bonus0Booking} \colorbox{red!0}{\strut class} \colorbox{red!0}{\strut bonus0In} \colorbox{red!0}{\strut totalTotal} \colorbox{red!0}{\strut frequent} \colorbox{red!0}{\strut flyer} \colorbox{red!0}{\strut miles7437CalculateRound} \colorbox{red!0}{\strut trip} \colorbox{red!0}{\strut ?} \colorbox{red!0}{\strut No} 
}}}
\end{CJK*}

\begin{CJK*}{UTF8}{gbsn}
{\setlength{\fboxsep}{0pt}\colorbox{white!0}{\parbox{0.9\textwidth}{
\colorbox{red!0}{\strut The} \colorbox{red!1}{\strut driving} \colorbox{red!4}{\strut distance} \colorbox{red!0}{\strut from} \colorbox{red!1}{\strut Fort} \colorbox{red!0}{\strut Lauderdale-Hollywood} \colorbox{red!1}{\strut International} \colorbox{red!2}{\strut Airport} \colorbox{red!0}{\strut to} \colorbox{red!9}{\strut Miami} \colorbox{red!1}{\strut International} \colorbox{red!2}{\strut Airport} \colorbox{red!0}{\strut is} \colorbox{red!0}{\strut .} \colorbox{red!0}{\strut The} \colorbox{red!1}{\strut driving} \colorbox{red!4}{\strut distance} \colorbox{red!0}{\strut from} \colorbox{red!1}{\strut Fort} \colorbox{red!0}{\strut Lauderdale-Hollywood} \colorbox{red!1}{\strut International} \colorbox{red!2}{\strut Airport} \colorbox{red!0}{\strut to} \colorbox{red!9}{\strut Miami} \colorbox{red!1}{\strut International} \colorbox{red!2}{\strut Airport} \colorbox{red!0}{\strut is32} \colorbox{red!1}{\strut miles} \colorbox{red!0}{\strut 51} \colorbox{red!0}{\strut kmCity} \colorbox{red!0}{\strut .} \colorbox{red!0}{\strut Check-in} \colorbox{red!0}{\strut .} \colorbox{red!0}{\strut Check-out} \colorbox{red!0}{\strut .} \colorbox{red!0}{\strut Rooms} \colorbox{red!0}{\strut .} \colorbox{red!0}{\strut Travelers} \colorbox{red!0}{\strut .} \colorbox{red!0}{\strut Get} \colorbox{red!0}{\strut .} \colorbox{red!0}{\strut Get} \colorbox{red!0}{\strut .} \colorbox{red!0}{\strut From} \colorbox{red!0}{\strut .} \colorbox{red!0}{\strut To} \colorbox{red!0}{\strut .} \colorbox{red!1}{\strut Fort} \colorbox{red!10}{\strut Lauderdale} \colorbox{red!0}{\strut to} \colorbox{red!9}{\strut Miami} \colorbox{red!0}{\strut road} \colorbox{red!0}{\strut tripMap} \colorbox{red!0}{\strut of} \colorbox{red!1}{\strut driving} \colorbox{red!1}{\strut directions} \colorbox{red!0}{\strut from} \colorbox{red!10}{\strut FLL} \colorbox{red!0}{\strut to} \colorbox{red!0}{\strut MIAClick} \colorbox{red!0}{\strut here} \colorbox{red!0}{\strut to} \colorbox{red!0}{\strut show} \colorbox{red!0}{\strut mapDrag} \colorbox{red!0}{\strut the} \colorbox{red!0}{\strut line} \colorbox{red!0}{\strut on} \colorbox{red!0}{\strut the} \colorbox{red!0}{\strut map} \colorbox{red!0}{\strut to} \colorbox{red!0}{\strut calculate} \colorbox{red!0}{\strut the} \colorbox{red!1}{\strut driving} \colorbox{red!4}{\strut distance} \colorbox{red!0}{\strut for} \colorbox{red!0}{\strut a} \colorbox{red!0}{\strut different} \colorbox{red!0}{\strut route.If} \colorbox{red!0}{\strut you} \colorbox{red!0}{\strut want} \colorbox{red!0}{\strut to} \colorbox{red!0}{\strut verify} \colorbox{red!0}{\strut these} \colorbox{red!1}{\strut driving} \colorbox{red!1}{\strut directions} \colorbox{red!0}{\strut or} \colorbox{red!0}{\strut look} \colorbox{red!0}{\strut for} \colorbox{red!0}{\strut another} \colorbox{red!0}{\strut possible} \colorbox{red!0}{\strut route} \colorbox{red!0}{\strut ,} \colorbox{red!0}{\strut you} \colorbox{red!0}{\strut can} \colorbox{red!0}{\strut try} \colorbox{red!0}{\strut Google} \colorbox{red!0}{\strut Maps} \colorbox{red!0}{\strut ,} \colorbox{red!0}{\strut Bing} \colorbox{red!0}{\strut Maps} \colorbox{red!0}{\strut ,} \colorbox{red!0}{\strut or} \colorbox{red!0}{\strut MapQuest.More} \colorbox{red!0}{\strut trip} \colorbox{red!0}{\strut calculationsdriving} \colorbox{red!0}{\strut time} \colorbox{red!0}{\strut from} \colorbox{red!10}{\strut FLL} \colorbox{red!0}{\strut to} \colorbox{red!0}{\strut MIAcost} \colorbox{red!0}{\strut of} \colorbox{red!1}{\strut driving} \colorbox{red!0}{\strut from} \colorbox{red!10}{\strut FLL} \colorbox{red!0}{\strut to} \colorbox{red!0}{\strut MIAreverse} \colorbox{red!1}{\strut drive} \colorbox{red!4}{\strut distance} \colorbox{red!0}{\strut from} \colorbox{red!10}{\strut MIA} \colorbox{red!0}{\strut to} \colorbox{red!0}{\strut FLLhalfway} \colorbox{red!0}{\strut between} \colorbox{red!10}{\strut FLL} \colorbox{red!0}{\strut and} \colorbox{red!0}{\strut MIAstopping} \colorbox{red!0}{\strut points} \colorbox{red!0}{\strut from} \colorbox{red!10}{\strut FLL} \colorbox{red!0}{\strut to} \colorbox{red!0}{\strut MIAhotels} \colorbox{red!0}{\strut near} \colorbox{red!0}{\strut MIAflight} \colorbox{red!4}{\strut distance} \colorbox{red!0}{\strut from} \colorbox{red!10}{\strut FLL} \colorbox{red!0}{\strut to} \colorbox{red!0}{\strut MIAflight} \colorbox{red!0}{\strut time} \colorbox{red!0}{\strut from} \colorbox{red!10}{\strut FLL} \colorbox{red!0}{\strut to} \colorbox{red!0}{\strut MIAfly} \colorbox{red!0}{\strut or} \colorbox{red!1}{\strut drive} \colorbox{red!0}{\strut from} \colorbox{red!10}{\strut FLL} \colorbox{red!0}{\strut to} \colorbox{red!0}{\strut MIAairports} \colorbox{red!0}{\strut near} \colorbox{red!0}{\strut MIAairlines} \colorbox{red!1}{\strut flying} \colorbox{red!0}{\strut to} \colorbox{red!0}{\strut MIAnonstop} \colorbox{red!1}{\strut flights} \colorbox{red!0}{\strut from} \colorbox{red!10}{\strut FLL} \colorbox{red!0}{\strut to} \colorbox{red!0}{\strut MIAtime} \colorbox{red!1}{\strut difference} \colorbox{red!0}{\strut between} \colorbox{red!10}{\strut FLL} \colorbox{red!0}{\strut and} \colorbox{red!10}{\strut MIA} 
}}}
\end{CJK*}

query: how many 1000 in 1 million

\begin{CJK*}{UTF8}{gbsn}
{\setlength{\fboxsep}{0pt}\colorbox{white!0}{\parbox{0.9\textwidth}{
\colorbox{red!4}{\strut How} \colorbox{red!0}{\strut many} \colorbox{red!5}{\strut thousands} \colorbox{red!0}{\strut are} \colorbox{red!0}{\strut in} \colorbox{red!0}{\strut a} \colorbox{red!5}{\strut million} \colorbox{red!0}{\strut ?} \colorbox{red!0}{\strut Answers.com} \colorbox{red!0}{\strut .} \colorbox{red!0}{\strut WikiAnswers} \colorbox{red!0}{\strut .} \colorbox{red!0}{\strut Categories} \colorbox{red!0}{\strut Science} \colorbox{red!0}{\strut Math} \colorbox{red!0}{\strut and} \colorbox{red!0}{\strut Arithmetic} \colorbox{red!0}{\strut Mathematical} \colorbox{red!0}{\strut Analysis} \colorbox{red!4}{\strut How} \colorbox{red!0}{\strut many} \colorbox{red!5}{\strut thousands} \colorbox{red!0}{\strut are} \colorbox{red!0}{\strut in} \colorbox{red!0}{\strut a} \colorbox{red!5}{\strut million} \colorbox{red!0}{\strut ?} \colorbox{red!0}{\strut FlagHow} \colorbox{red!0}{\strut many} \colorbox{red!5}{\strut thousands} \colorbox{red!0}{\strut are} \colorbox{red!0}{\strut in} \colorbox{red!0}{\strut a} \colorbox{red!5}{\strut million} \colorbox{red!0}{\strut ?} \colorbox{red!0}{\strut Answer} \colorbox{red!0}{\strut by} \colorbox{red!0}{\strut Rob} \colorbox{red!0}{\strut Flanders} \colorbox{red!0}{\strut Confidence} \colorbox{red!0}{\strut votes} \colorbox{red!0}{\strut 31.2KANSWER} \colorbox{red!0}{\strut .} \colorbox{red!0}{\strut 1000} \colorbox{red!5}{\strut thousands} \colorbox{red!0}{\strut .} \colorbox{red!0}{\strut 1} \colorbox{red!5}{\strut million} \colorbox{red!0}{\strut ,} \colorbox{red!0}{\strut 1} \colorbox{red!0}{\strut ,} \colorbox{red!0}{\strut 000} \colorbox{red!0}{\strut ,} \colorbox{red!0}{\strut 000} \colorbox{red!0}{\strut 1000} \colorbox{red!4}{\strut millions} \colorbox{red!0}{\strut .} \colorbox{red!0}{\strut 1} \colorbox{red!0}{\strut billion} \colorbox{red!0}{\strut ,} \colorbox{red!0}{\strut 1,000,000,000} \colorbox{red!0}{\strut 1000} \colorbox{red!0}{\strut billions} \colorbox{red!0}{\strut .} \colorbox{red!0}{\strut 1} \colorbox{red!0}{\strut trillion} \colorbox{red!0}{\strut ,} \colorbox{red!0}{\strut 1,000,000,000,000} \colorbox{red!0}{\strut There} \colorbox{red!0}{\strut are} \colorbox{red!0}{\strut a} \colorbox{red!5}{\strut thousand} \colorbox{red!5}{\strut thousands} \colorbox{red!0}{\strut in} \colorbox{red!0}{\strut one} \colorbox{red!5}{\strut million} \colorbox{red!0}{\strut 1000} \colorbox{red!0}{\strut Proof} \colorbox{red!0}{\strut is} \colorbox{red!0}{\strut seen} \colorbox{red!0}{\strut when} \colorbox{red!0}{\strut multiplied} \colorbox{red!0}{\strut together} \colorbox{red!0}{\strut ,} \colorbox{red!0}{\strut 1000} \colorbox{red!0}{\strut .} \colorbox{red!0}{\strut 1000} \colorbox{red!0}{\strut .} \colorbox{red!0}{\strut 1,000,000} \colorbox{red!0}{\strut .} \colorbox{red!0}{\strut one} \colorbox{red!5}{\strut million} \colorbox{red!0}{\strut .} \colorbox{red!0}{\strut .} \colorbox{red!0}{\strut There} \colorbox{red!0}{\strut are} \colorbox{red!0}{\strut .} \colorbox{red!0}{\strut 1,0001,000} \colorbox{red!0}{\strut .} \colorbox{red!0}{\strut 1,000,00067} \colorbox{red!0}{\strut people} \colorbox{red!0}{\strut found} \colorbox{red!0}{\strut this} \colorbox{red!0}{\strut usefulWas} \colorbox{red!0}{\strut this} \colorbox{red!0}{\strut answer} \colorbox{red!0}{\strut useful} \colorbox{red!0}{\strut ?} \colorbox{red!0}{\strut YesSomewhatNoUser00987} \colorbox{red!0}{\strut 126,341} \colorbox{red!0}{\strut ContributionsHow} \colorbox{red!0}{\strut many} \colorbox{red!5}{\strut thousands} \colorbox{red!0}{\strut makes} \colorbox{red!0}{\strut a} \colorbox{red!5}{\strut million} \colorbox{red!0}{\strut ?} \colorbox{red!0}{\strut A} \colorbox{red!5}{\strut thousand} \colorbox{red!5}{\strut thousand} \colorbox{red!0}{\strut is} \colorbox{red!0}{\strut a} \colorbox{red!5}{\strut million} \colorbox{red!0}{\strut 1000} \colorbox{red!0}{\strut x} \colorbox{red!0}{\strut 1000} \colorbox{red!0}{\strut .} \colorbox{red!0}{\strut 1,000,000Matthew} \colorbox{red!0}{\strut Burgess} \colorbox{red!0}{\strut 396,785} \colorbox{red!0}{\strut ContributionsA} \colorbox{red!5}{\strut million} \colorbox{red!0}{\strut equals} \colorbox{red!4}{\strut how} \colorbox{red!0}{\strut many} \colorbox{red!5}{\strut thousand} \colorbox{red!0}{\strut ?} \colorbox{red!0}{\strut One} \colorbox{red!5}{\strut million} \colorbox{red!0}{\strut is} \colorbox{red!0}{\strut equal} \colorbox{red!0}{\strut to} \colorbox{red!0}{\strut 1000} \colorbox{red!0}{\strut thousands.Anand} \colorbox{red!0}{\strut Vijayakumar} \colorbox{red!0}{\strut 363,997} \colorbox{red!0}{\strut ContributionsHow} \colorbox{red!0}{\strut many} \colorbox{red!5}{\strut thousands} \colorbox{red!0}{\strut is} \colorbox{red!0}{\strut in} \colorbox{red!5}{\strut million} \colorbox{red!0}{\strut dollars} \colorbox{red!0}{\strut ?} \colorbox{red!0}{\strut 1000000} \colorbox{red!0}{\strut .} \colorbox{red!0}{\strut 1000} \colorbox{red!0}{\strut .} \colorbox{red!0}{\strut 1000} \colorbox{red!0}{\strut A} \colorbox{red!5}{\strut thousand} \colorbox{red!5}{\strut thousands} \colorbox{red!0}{\strut is} \colorbox{red!0}{\strut called} \colorbox{red!0}{\strut a} \colorbox{red!5}{\strut million} \colorbox{red!0}{\strut dollars.Anand} \colorbox{red!0}{\strut Mehta} \colorbox{red!0}{\strut 278,423} \colorbox{red!0}{\strut Contributionsmehtamatics} \colorbox{red!0}{\strut .} \colorbox{red!0}{\strut mathematics} \colorbox{red!0}{\strut with} \colorbox{red!0}{\strut a} \colorbox{red!0}{\strut differenceHow} \colorbox{red!0}{\strut many} \colorbox{red!5}{\strut thousands} \colorbox{red!0}{\strut in} \colorbox{red!0}{\strut 31.92} \colorbox{red!5}{\strut million} \colorbox{red!0}{\strut ?} \colorbox{red!0}{\strut 319204} \colorbox{red!0}{\strut JAYS} \colorbox{red!0}{\strut 2,010,442} \colorbox{red!0}{\strut ContributionsMathematics} \colorbox{red!0}{\strut ,} \colorbox{red!0}{\strut facts} \colorbox{red!0}{\strut ,} \colorbox{red!0}{\strut figures} \colorbox{red!0}{\strut ,} \colorbox{red!0}{\strut definitions} \colorbox{red!0}{\strut ,} \colorbox{red!0}{\strut conversions} \colorbox{red!0}{\strut and} \colorbox{red!0}{\strut physics} \colorbox{red!0}{\strut are} \colorbox{red!0}{\strut my} \colorbox{red!0}{\strut interests} \colorbox{red!0}{\strut on} \colorbox{red!0}{\strut Answers.comHow} \colorbox{red!0}{\strut many} \colorbox{red!5}{\strut thousands} \colorbox{red!0}{\strut in} \colorbox{red!0}{\strut a} \colorbox{red!0}{\strut one} \colorbox{red!5}{\strut million} \colorbox{red!0}{\strut ?} \colorbox{red!0}{\strut There} \colorbox{red!0}{\strut are} \colorbox{red!0}{\strut 1,000} \colorbox{red!5}{\strut thousands} \colorbox{red!0}{\strut in} \colorbox{red!0}{\strut one} \colorbox{red!0}{\strut million.Anand} \colorbox{red!0}{\strut Mehta} \colorbox{red!0}{\strut 278,423} \colorbox{red!0}{\strut Contributionsmehtamatics} \colorbox{red!0}{\strut .} \colorbox{red!0}{\strut mathematics} \colorbox{red!0}{\strut with} \colorbox{red!0}{\strut a} \colorbox{red!0}{\strut differenceHow} \colorbox{red!0}{\strut many} \colorbox{red!5}{\strut thousands} \colorbox{red!0}{\strut in} \colorbox{red!0}{\strut 17.5} \colorbox{red!5}{\strut million} \colorbox{red!0}{\strut ?} \colorbox{red!0}{\strut 17500How} \colorbox{red!0}{\strut many} \colorbox{red!0}{\strut hundred} \colorbox{red!5}{\strut thousands} \colorbox{red!0}{\strut are} \colorbox{red!0}{\strut in} \colorbox{red!0}{\strut a} \colorbox{red!5}{\strut million} \colorbox{red!0}{\strut and} \colorbox{red!0}{\strut why} \colorbox{red!0}{\strut ?} \colorbox{red!0}{\strut 10} \colorbox{red!0}{\strut .} \colorbox{red!0}{\strut Because} \colorbox{red!0}{\strut 100,000} \colorbox{red!0}{\strut x} \colorbox{red!0}{\strut 10} \colorbox{red!0}{\strut .} \colorbox{red!0}{\strut 1,000,000Sandalian} \colorbox{red!0}{\strut 919} \colorbox{red!0}{\strut ContributionsHow} \colorbox{red!0}{\strut many} \colorbox{red!0}{\strut 10} \colorbox{red!5}{\strut thousands} \colorbox{red!0}{\strut are} \colorbox{red!0}{\strut in} \colorbox{red!0}{\strut a} \colorbox{red!5}{\strut million} \colorbox{red!0}{\strut ?} \colorbox{red!0}{\strut There} \colorbox{red!0}{\strut are} \colorbox{red!0}{\strut 100} \colorbox{red!0}{\strut ten} \colorbox{red!5}{\strut thousands} \colorbox{red!0}{\strut in} \colorbox{red!0}{\strut a} \colorbox{red!0}{\strut million.4} \colorbox{red!0}{\strut JAYS} \colorbox{red!0}{\strut 2,010,442} \colorbox{red!0}{\strut ContributionsMathematics} \colorbox{red!0}{\strut ,} \colorbox{red!0}{\strut facts} \colorbox{red!0}{\strut ,} \colorbox{red!0}{\strut figures} \colorbox{red!0}{\strut ,} \colorbox{red!0}{\strut definitions} \colorbox{red!0}{\strut ,} \colorbox{red!0}{\strut conversions} \colorbox{red!0}{\strut and} \colorbox{red!0}{\strut physics} \colorbox{red!0}{\strut are} \colorbox{red!0}{\strut my} \colorbox{red!0}{\strut interests} \colorbox{red!0}{\strut on} \colorbox{red!0}{\strut Answers.comHow} \colorbox{red!0}{\strut many} \colorbox{red!5}{\strut thousand} \colorbox{red!0}{\strut is} \colorbox{red!0}{\strut 0.3} \colorbox{red!5}{\strut million} \colorbox{red!0}{\strut ?} \colorbox{red!0}{\strut 0.3} \colorbox{red!0}{\strut trillion} \colorbox{red!0}{\strut equals} \colorbox{red!0}{\strut 300} \colorbox{red!5}{\strut million} \colorbox{red!0}{\strut thousands.4} \colorbox{red!0}{\strut JAYS} \colorbox{red!0}{\strut 2,010,442} \colorbox{red!0}{\strut ContributionsMathematics} \colorbox{red!0}{\strut ,} \colorbox{red!0}{\strut facts} 
}}}
\end{CJK*}

\begin{CJK*}{UTF8}{gbsn}
{\setlength{\fboxsep}{0pt}\colorbox{white!0}{\parbox{0.9\textwidth}{
\colorbox{red!1}{\strut What} \colorbox{red!0}{\strut does} \colorbox{red!4}{\strut trillion} \colorbox{red!1}{\strut equal} \colorbox{red!0}{\strut ?} \colorbox{red!0}{\strut Nasiruddin} \colorbox{red!0}{\strut 5} \colorbox{red!0}{\strut ContributionsWhat} \colorbox{red!0}{\strut does} \colorbox{red!4}{\strut trillion} \colorbox{red!1}{\strut equal} \colorbox{red!0}{\strut ?} \colorbox{red!0}{\strut 1,000,000,000,000What} \colorbox{red!0}{\strut is} \colorbox{red!3}{\strut 1000} \colorbox{red!4}{\strut trillion} \colorbox{red!0}{\strut ?} \colorbox{red!0}{\strut A} \colorbox{red!0}{\strut thousand} \colorbox{red!4}{\strut trillion} \colorbox{red!0}{\strut is} \colorbox{red!0}{\strut one} \colorbox{red!0}{\strut quadrillion} \colorbox{red!0}{\strut .} \colorbox{red!0}{\strut You} \colorbox{red!0}{\strut can} \colorbox{red!0}{\strut figure} \colorbox{red!0}{\strut this} \colorbox{red!0}{\strut out} \colorbox{red!0}{\strut byknowing} \colorbox{red!0}{\strut the} \colorbox{red!0}{\strut numbers} \colorbox{red!0}{\strut of} \colorbox{red!0}{\strut zeroes} \colorbox{red!0}{\strut are} \colorbox{red!0}{\strut in} \colorbox{red!0}{\strut a} \colorbox{red!4}{\strut trillion} \colorbox{red!0}{\strut ,} \colorbox{red!0}{\strut which} \colorbox{red!0}{\strut are} \colorbox{red!0}{\strut 12.Since} \colorbox{red!3}{\strut 1000} \colorbox{red!0}{\strut has} \colorbox{red!0}{\strut three} \colorbox{red!0}{\strut zeroes} \colorbox{red!0}{\strut ,} \colorbox{red!3}{\strut 1000} \colorbox{red!4}{\strut trillion} \colorbox{red!0}{\strut is} \colorbox{red!1}{\strut 1} \colorbox{red!0}{\strut What} \colorbox{red!0}{\strut is} \colorbox{red!3}{\strut 1000} \colorbox{red!0}{\strut times} \colorbox{red!0}{\strut a} \colorbox{red!4}{\strut trillion} \colorbox{red!1}{\strut million} \colorbox{red!0}{\strut ?} \colorbox{red!0}{\strut quatrillionAnna} \colorbox{red!0}{\strut Rino} \colorbox{red!0}{\strut 36,058} \colorbox{red!0}{\strut ContributionsHow} \colorbox{red!0}{\strut many} \colorbox{red!3}{\strut 1000} \colorbox{red!0}{\strut in} \colorbox{red!0}{\strut a} \colorbox{red!4}{\strut trillion} \colorbox{red!0}{\strut ?} \colorbox{red!0}{\strut Number} \colorbox{red!0}{\strut of} \colorbox{red!3}{\strut 1000} \colorbox{red!0}{\strut in} \colorbox{red!0}{\strut a} \colorbox{red!4}{\strut trillion} \colorbox{red!0}{\strut .} \colorbox{red!1}{\strut 1} \colorbox{red!0}{\strut billionWhat} \colorbox{red!0}{\strut is} \colorbox{red!3}{\strut 1000} \colorbox{red!1}{\strut million} \colorbox{red!0}{\strut in} \colorbox{red!0}{\strut billions} \colorbox{red!0}{\strut or} \colorbox{red!4}{\strut trillions} \colorbox{red!0}{\strut ?} \colorbox{red!3}{\strut 1000} \colorbox{red!1}{\strut million} \colorbox{red!1}{\strut equals} \colorbox{red!1}{\strut 1} \colorbox{red!4}{\strut billion} \colorbox{red!0}{\strut 1,000,000,000} \colorbox{red!3}{\strut 1000} \colorbox{red!4}{\strut billion} \colorbox{red!1}{\strut equals} \colorbox{red!1}{\strut 1} \colorbox{red!4}{\strut trillion} \colorbox{red!0}{\strut 1,000,000,000,000Al} \colorbox{red!0}{\strut Cohen} \colorbox{red!0}{\strut 126,337} \colorbox{red!0}{\strut ContributionsSenior} \colorbox{red!0}{\strut Fellow} \colorbox{red!0}{\strut in} \colorbox{red!0}{\strut Electrical} \colorbox{red!0}{\strut EngineeringDoes} \colorbox{red!3}{\strut 1000} \colorbox{red!1}{\strut million} \colorbox{red!1}{\strut equal} \colorbox{red!1}{\strut 1} \colorbox{red!4}{\strut trillion} \colorbox{red!0}{\strut ?} \colorbox{red!0}{\strut No} \colorbox{red!0}{\strut .} \colorbox{red!0}{\strut 1,000} \colorbox{red!1}{\strut million} \colorbox{red!0}{\strut .} \colorbox{red!1}{\strut 1} \colorbox{red!4}{\strut billion} \colorbox{red!0}{\strut 1,000} \colorbox{red!4}{\strut billion} \colorbox{red!0}{\strut .} \colorbox{red!1}{\strut 1} \colorbox{red!0}{\strut trillionWhat} \colorbox{red!0}{\strut is} \colorbox{red!0}{\strut the} \colorbox{red!0}{\strut value} \colorbox{red!0}{\strut of} \colorbox{red!3}{\strut 1000} \colorbox{red!4}{\strut trillion} \colorbox{red!0}{\strut ?} \colorbox{red!0}{\strut 1000,000,00,00,000,001000} \colorbox{red!4}{\strut trillion} \colorbox{red!1}{\strut equal} \colorbox{red!0}{\strut to} \colorbox{red!1}{\strut how} \colorbox{red!0}{\strut much} \colorbox{red!0}{\strut Indian} \colorbox{red!0}{\strut rupees} \colorbox{red!0}{\strut ?} \colorbox{red!3}{\strut 1000} \colorbox{red!4}{\strut trillion} \colorbox{red!0}{\strut indian1000} \colorbox{red!4}{\strut trillion} \colorbox{red!0}{\strut is} \colorbox{red!1}{\strut equal} \colorbox{red!0}{\strut to} \colorbox{red!1}{\strut what} \colorbox{red!0}{\strut ?} \colorbox{red!1}{\strut 1} \colorbox{red!0}{\strut quadrillion} \colorbox{red!0}{\strut exactly} \colorbox{red!0}{\strut .} \colorbox{red!0}{\strut Pcig} \colorbox{red!0}{\strut morfil} \colorbox{red!0}{\strut 39,268} \colorbox{red!0}{\strut ContributionsWhat} \colorbox{red!0}{\strut is} \colorbox{red!0}{\strut a} \colorbox{red!4}{\strut trillion} \colorbox{red!0}{\strut times} \colorbox{red!3}{\strut 1000} \colorbox{red!0}{\strut ?} \colorbox{red!0}{\strut On} \colorbox{red!0}{\strut the} \colorbox{red!0}{\strut short} \colorbox{red!0}{\strut scale} \colorbox{red!0}{\strut .} \colorbox{red!0}{\strut as} \colorbox{red!0}{\strut used} \colorbox{red!0}{\strut in} \colorbox{red!0}{\strut the} \colorbox{red!0}{\strut US} \colorbox{red!0}{\strut .} \colorbox{red!0}{\strut .} \colorbox{red!1}{\strut 1} \colorbox{red!4}{\strut trillion} \colorbox{red!0}{\strut .} \colorbox{red!0}{\strut 10} \colorbox{red!0}{\strut 12} \colorbox{red!0}{\strut .} \colorbox{red!0}{\strut x} \colorbox{red!3}{\strut 1000} \colorbox{red!0}{\strut .} \colorbox{red!1}{\strut 1} \colorbox{red!0}{\strut quadrillion} \colorbox{red!0}{\strut .} \colorbox{red!0}{\strut 10} \colorbox{red!0}{\strut 15} \colorbox{red!0}{\strut .} \colorbox{red!0}{\strut On} \colorbox{red!0}{\strut the} \colorbox{red!0}{\strut long} \colorbox{red!0}{\strut scales} \colorbox{red!0}{\strut .} \colorbox{red!0}{\strut as} \colorbox{red!0}{\strut used} \colorbox{red!0}{\strut in} \colorbox{red!0}{\strut Europe} \colorbox{red!0}{\strut .} \colorbox{red!0}{\strut .} \colorbox{red!1}{\strut 1} \colorbox{red!4}{\strut trillion} \colorbox{red!0}{\strut .} \colorbox{red!0}{\strut 10} \colorbox{red!0}{\strut 18} \colorbox{red!0}{\strut .} \colorbox{red!0}{\strut x} \colorbox{red!3}{\strut 1000} \colorbox{red!0}{\strut .} \colorbox{red!1}{\strut 1} \colorbox{red!0}{\strut thousand} \colorbox{red!0}{\strut Prasang} \colorbox{red!0}{\strut ghanshyam} \colorbox{red!0}{\strut 348} \colorbox{red!0}{\strut ContributionsHow} \colorbox{red!0}{\strut much} \colorbox{red!0}{\strut is} \colorbox{red!3}{\strut 1000} \colorbox{red!4}{\strut trillion} \colorbox{red!1}{\strut equal} \colorbox{red!0}{\strut ?} \colorbox{red!0}{\strut 10} \colorbox{red!0}{\strut crore} \colorbox{red!0}{\strut crores4} \colorbox{red!0}{\strut JAYS} \colorbox{red!0}{\strut 2,010,442} \colorbox{red!0}{\strut ContributionsMathematics} \colorbox{red!0}{\strut ,} \colorbox{red!0}{\strut facts} \colorbox{red!0}{\strut ,} \colorbox{red!0}{\strut figures} \colorbox{red!0}{\strut ,} \colorbox{red!0}{\strut definitions} \colorbox{red!0}{\strut ,} \colorbox{red!0}{\strut conversions} \colorbox{red!0}{\strut and} \colorbox{red!0}{\strut physics} \colorbox{red!0}{\strut are} \colorbox{red!0}{\strut my} \colorbox{red!0}{\strut interests} \colorbox{red!0}{\strut on} \colorbox{red!0}{\strut Answers.comWhat} \colorbox{red!0}{\strut is} \colorbox{red!0}{\strut the} \colorbox{red!0}{\strut number} \colorbox{red!3}{\strut 1000} \colorbox{red!4}{\strut trillion} \colorbox{red!0}{\strut in} \colorbox{red!0}{\strut words} \colorbox{red!0}{\strut ?} \colorbox{red!0}{\strut One} \colorbox{red!0}{\strut thousand} \colorbox{red!4}{\strut trillion} \colorbox{red!0}{\strut .} 
}}}
\end{CJK*}

query: what is the voltage in israel

\begin{CJK*}{UTF8}{gbsn}
{\setlength{\fboxsep}{0pt}\colorbox{white!0}{\parbox{0.9\textwidth}{
\colorbox{red!0}{\strut Aliyah} \colorbox{red!0}{\strut .} \colorbox{red!13}{\strut Electrical} \colorbox{red!0}{\strut .} \colorbox{red!0}{\strut FAQ} \colorbox{red!0}{\strut .} \colorbox{red!0}{\strut .} \colorbox{red!0}{\strut Aliyah} \colorbox{red!0}{\strut .} \colorbox{red!13}{\strut Electrical} \colorbox{red!0}{\strut .} \colorbox{red!0}{\strut FAQ} \colorbox{red!0}{\strut .} \colorbox{red!0}{\strut LAST} \colorbox{red!0}{\strut UPDATED} \colorbox{red!0}{\strut May} \colorbox{red!0}{\strut 21,2006} \colorbox{red!0}{\strut .} \colorbox{red!0}{\strut CLICK} \colorbox{red!0}{\strut ON} \colorbox{red!0}{\strut QUESTION} \colorbox{red!0}{\strut TO} \colorbox{red!0}{\strut GO} \colorbox{red!0}{\strut TO} \colorbox{red!0}{\strut ANSWER} \colorbox{red!0}{\strut .} \colorbox{red!0}{\strut 1} \colorbox{red!0}{\strut .} \colorbox{red!11}{\strut What} \colorbox{red!0}{\strut are} \colorbox{red!0}{\strut the} \colorbox{red!0}{\strut main} \colorbox{red!6}{\strut differences} \colorbox{red!0}{\strut between} \colorbox{red!0}{\strut the} \colorbox{red!13}{\strut electrical} \colorbox{red!5}{\strut power} \colorbox{red!2}{\strut supplied} \colorbox{red!0}{\strut in} \colorbox{red!0}{\strut the} \colorbox{red!0}{\strut US} \colorbox{red!0}{\strut and} \colorbox{red!0}{\strut the} \colorbox{red!5}{\strut power} \colorbox{red!2}{\strut supplied} \colorbox{red!0}{\strut in} \colorbox{red!3}{\strut Israel} \colorbox{red!0}{\strut ?} \colorbox{red!0}{\strut 2} \colorbox{red!0}{\strut .} \colorbox{red!0}{\strut Can} \colorbox{red!0}{\strut I} \colorbox{red!0}{\strut use} \colorbox{red!0}{\strut my} \colorbox{red!1}{\strut 110V} \colorbox{red!0}{\strut refrigerator} \colorbox{red!0}{\strut in} \colorbox{red!3}{\strut Israel} \colorbox{red!0}{\strut ?} \colorbox{red!0}{\strut 3} \colorbox{red!0}{\strut .} \colorbox{red!11}{\strut What} \colorbox{red!0}{\strut about} \colorbox{red!0}{\strut buying} \colorbox{red!0}{\strut a} \colorbox{red!1}{\strut 110V} \colorbox{red!1}{\strut washer} \colorbox{red!0}{\strut andor} \colorbox{red!1}{\strut dryer} \colorbox{red!0}{\strut ,} \colorbox{red!0}{\strut can} \colorbox{red!0}{\strut I} \colorbox{red!0}{\strut use} \colorbox{red!0}{\strut them} \colorbox{red!0}{\strut in} \colorbox{red!3}{\strut Israel} \colorbox{red!0}{\strut ?} \colorbox{red!0}{\strut 4} \colorbox{red!0}{\strut .} \colorbox{red!0}{\strut Can} \colorbox{red!0}{\strut I} \colorbox{red!0}{\strut use} \colorbox{red!0}{\strut my} \colorbox{red!1}{\strut 110v} \colorbox{red!0}{\strut small} \colorbox{red!1}{\strut appliances} \colorbox{red!0}{\strut in} \colorbox{red!3}{\strut Israel} \colorbox{red!0}{\strut with} \colorbox{red!0}{\strut a} \colorbox{red!2}{\strut transformer} \colorbox{red!0}{\strut ?} \colorbox{red!0}{\strut 5} \colorbox{red!0}{\strut .} \colorbox{red!11}{\strut What} \colorbox{red!0}{\strut is} \colorbox{red!0}{\strut the} \colorbox{red!6}{\strut difference} \colorbox{red!0}{\strut between} \colorbox{red!0}{\strut a} \colorbox{red!2}{\strut transformer} \colorbox{red!0}{\strut ,} \colorbox{red!2}{\strut converter} \colorbox{red!0}{\strut ,} \colorbox{red!0}{\strut and} \colorbox{red!5}{\strut power} \colorbox{red!1}{\strut supply} \colorbox{red!0}{\strut ?} \colorbox{red!0}{\strut 6} \colorbox{red!0}{\strut .} \colorbox{red!0}{\strut Do} \colorbox{red!0}{\strut I} \colorbox{red!0}{\strut need} \colorbox{red!0}{\strut anything} \colorbox{red!0}{\strut special} \colorbox{red!0}{\strut to} \colorbox{red!1}{\strut convert} \colorbox{red!0}{\strut the} \colorbox{red!1}{\strut voltage} \colorbox{red!0}{\strut in} \colorbox{red!0}{\strut my} \colorbox{red!1}{\strut computer} \colorbox{red!0}{\strut if} \colorbox{red!0}{\strut I} \colorbox{red!1}{\strut bring} \colorbox{red!0}{\strut it} \colorbox{red!0}{\strut from} \colorbox{red!0}{\strut the} \colorbox{red!0}{\strut US} \colorbox{red!0}{\strut to} \colorbox{red!3}{\strut Israel} \colorbox{red!0}{\strut ?} \colorbox{red!0}{\strut 7} \colorbox{red!0}{\strut .} \colorbox{red!0}{\strut Can} \colorbox{red!0}{\strut I} \colorbox{red!0}{\strut use} \colorbox{red!0}{\strut my} \colorbox{red!0}{\strut lighting} \colorbox{red!0}{\strut fixtures} \colorbox{red!0}{\strut from} \colorbox{red!0}{\strut the} \colorbox{red!0}{\strut US} \colorbox{red!0}{\strut in} \colorbox{red!3}{\strut Israel} \colorbox{red!0}{\strut ?} \colorbox{red!0}{\strut 8} \colorbox{red!0}{\strut .} \colorbox{red!0}{\strut If} \colorbox{red!0}{\strut I} \colorbox{red!0}{\strut purchase} \colorbox{red!0}{\strut a} \colorbox{red!0}{\strut 12VDC} \colorbox{red!0}{\strut -} \colorbox{red!0}{\strut .} \colorbox{red!1}{\strut 110VAC} \colorbox{red!1}{\strut inverter} \colorbox{red!0}{\strut ,} \colorbox{red!0}{\strut could} \colorbox{red!0}{\strut I} \colorbox{red!0}{\strut then} \colorbox{red!0}{\strut use} \colorbox{red!0}{\strut a} \colorbox{red!0}{\strut 220VAC} \colorbox{red!0}{\strut -} \colorbox{red!0}{\strut .} \colorbox{red!0}{\strut 12VDC} \colorbox{red!5}{\strut power} \colorbox{red!0}{\strut pack} \colorbox{red!0}{\strut to} \colorbox{red!1}{\strut supply} \colorbox{red!0}{\strut it} \colorbox{red!0}{\strut with} \colorbox{red!0}{\strut DC} \colorbox{red!1}{\strut voltage} \colorbox{red!0}{\strut to} \colorbox{red!0}{\strut run} \colorbox{red!0}{\strut my} \colorbox{red!0}{\strut stereo} \colorbox{red!1}{\strut system} \colorbox{red!0}{\strut with} \colorbox{red!0}{\strut 60Hz} \colorbox{red!14}{\strut electricity} \colorbox{red!0}{\strut ?} \colorbox{red!0}{\strut 9} \colorbox{red!0}{\strut .} \colorbox{red!0}{\strut I} \colorbox{red!0}{\strut am} \colorbox{red!0}{\strut planning} \colorbox{red!0}{\strut to} \colorbox{red!1}{\strut bring} \colorbox{red!0}{\strut with} \colorbox{red!0}{\strut me} \colorbox{red!0}{\strut ,} \colorbox{red!0}{\strut to} \colorbox{red!3}{\strut Israel} \colorbox{red!0}{\strut ,} \colorbox{red!0}{\strut some} \colorbox{red!0}{\strut equipment} \colorbox{red!1}{\strut which} \colorbox{red!1}{\strut uses} \colorbox{red!1}{\strut 110V} \colorbox{red!0}{\strut 60Hz} \colorbox{red!1}{\strut motors} \colorbox{red!0}{\strut .} \colorbox{red!0}{\strut I} \colorbox{red!0}{\strut would} \colorbox{red!0}{\strut like} \colorbox{red!0}{\strut to} \colorbox{red!0}{\strut have} \colorbox{red!0}{\strut the} \colorbox{red!1}{\strut motors} \colorbox{red!1}{\strut converted} \colorbox{red!0}{\strut in} \colorbox{red!3}{\strut Israel} \colorbox{red!0}{\strut to} \colorbox{red!0}{\strut 220V} \colorbox{red!0}{\strut 50Hz} \colorbox{red!0}{\strut .} \colorbox{red!0}{\strut Can} \colorbox{red!0}{\strut I} \colorbox{red!0}{\strut have} \colorbox{red!0}{\strut this} \colorbox{red!0}{\strut done} \colorbox{red!0}{\strut ,} \colorbox{red!0}{\strut and} \colorbox{red!0}{\strut would} \colorbox{red!0}{\strut it} \colorbox{red!0}{\strut be} \colorbox{red!0}{\strut costly} \colorbox{red!0}{\strut ?} \colorbox{red!0}{\strut 10} \colorbox{red!0}{\strut .} \colorbox{red!0}{\strut Can} \colorbox{red!0}{\strut my} \colorbox{red!1}{\strut 110V} \colorbox{red!1}{\strut computer} \colorbox{red!0}{\strut monitor} \colorbox{red!0}{\strut work} \colorbox{red!0}{\strut in} \colorbox{red!3}{\strut Israel} \colorbox{red!0}{\strut ?} \colorbox{red!11}{\strut What} \colorbox{red!0}{\strut about} \colorbox{red!0}{\strut my} \colorbox{red!0}{\strut printer} \colorbox{red!0}{\strut ?} \colorbox{red!0}{\strut 11} \colorbox{red!0}{\strut .} \colorbox{red!0}{\strut I} \colorbox{red!0}{\strut came} \colorbox{red!0}{\strut to} \colorbox{red!3}{\strut Israel} \colorbox{red!0}{\strut with} \colorbox{red!0}{\strut a} \colorbox{red!0}{\strut stacked} \colorbox{red!0}{\strut Maytag} \colorbox{red!0}{\strut washerdryer} \colorbox{red!0}{\strut ,} \colorbox{red!1}{\strut which} \colorbox{red!0}{\strut I} \colorbox{red!0}{\strut was} \colorbox{red!0}{\strut told} \colorbox{red!0}{\strut needs} \colorbox{red!0}{\strut a} \colorbox{red!0}{\strut 30A} \colorbox{red!0}{\strut line} \colorbox{red!0}{\strut .} \colorbox{red!0}{\strut The} \colorbox{red!0}{\strut electrician} \colorbox{red!0}{\strut told} \colorbox{red!0}{\strut me} \colorbox{red!0}{\strut that} \colorbox{red!0}{\strut I} \colorbox{red!0}{\strut need} \colorbox{red!0}{\strut this} \colorbox{red!0}{\strut big} \colorbox{red!0}{\strut .} \colorbox{red!0}{\strut huge} \colorbox{red!0}{\strut .} \colorbox{red!0}{\strut outlet} \colorbox{red!0}{\strut ,} \colorbox{red!0}{\strut while} \colorbox{red!0}{\strut the} \colorbox{red!0}{\strut company} \colorbox{red!0}{\strut that} \colorbox{red!0}{\strut will} \colorbox{red!0}{\strut be} \colorbox{red!0}{\strut installing} \colorbox{red!0}{\strut the} \colorbox{red!0}{\strut appliance} \colorbox{red!0}{\strut said} \colorbox{red!0}{\strut that} \colorbox{red!0}{\strut they} \colorbox{red!0}{\strut will} \colorbox{red!0}{\strut install} \colorbox{red!0}{\strut a} \colorbox{red!0}{\strut .} \colorbox{red!0}{\strut .} \colorbox{red!0}{\strut sheka} 
}}}
\end{CJK*}

\begin{CJK*}{UTF8}{gbsn}
{\setlength{\fboxsep}{0pt}\colorbox{white!0}{\parbox{0.9\textwidth}{
\colorbox{red!0}{\strut Search} \colorbox{red!0}{\strut results} \colorbox{red!0}{\strut Ceptics} \colorbox{red!1}{\strut 2} \colorbox{red!4}{\strut USB} \colorbox{red!4}{\strut Israel} \colorbox{red!3}{\strut Travel} \colorbox{red!4}{\strut Adapter} \colorbox{red!0}{\strut 4} \colorbox{red!0}{\strut in} \colorbox{red!0}{\strut 1} \colorbox{red!2}{\strut Power} \colorbox{red!3}{\strut Plug} \colorbox{red!0}{\strut .} \colorbox{red!3}{\strut Type} \colorbox{red!1}{\strut H} \colorbox{red!0}{\strut .} \colorbox{red!0}{\strut -} \colorbox{red!2}{\strut Universal} \colorbox{red!0}{\strut Socketby} \colorbox{red!0}{\strut Ceptics} \colorbox{red!0}{\strut .} \colorbox{red!0}{\strut 12.99} \colorbox{red!0}{\strut .} \colorbox{red!0}{\strut 12} \colorbox{red!0}{\strut 99FREE} \colorbox{red!1}{\strut Shipping} \colorbox{red!0}{\strut on} \colorbox{red!1}{\strut eligible} \colorbox{red!0}{\strut orders} \colorbox{red!0}{\strut and} \colorbox{red!0}{\strut 1} \colorbox{red!0}{\strut more} \colorbox{red!0}{\strut promotion4.4} \colorbox{red!0}{\strut out} \colorbox{red!0}{\strut of} \colorbox{red!0}{\strut 5} \colorbox{red!1}{\strut stars} \colorbox{red!0}{\strut 509OREI} \colorbox{red!4}{\strut Israel} \colorbox{red!0}{\strut ,} \colorbox{red!2}{\strut Palestine} \colorbox{red!3}{\strut Travel} \colorbox{red!3}{\strut Plug} \colorbox{red!4}{\strut Adapter} \colorbox{red!0}{\strut -} \colorbox{red!1}{\strut Dual} \colorbox{red!4}{\strut USB} \colorbox{red!0}{\strut -} \colorbox{red!2}{\strut Surge} \colorbox{red!1}{\strut Protection} \colorbox{red!0}{\strut -} \colorbox{red!3}{\strut Type} \colorbox{red!1}{\strut H} \colorbox{red!0}{\strut .} \colorbox{red!0}{\strut U2U-14} \colorbox{red!0}{\strut .} \colorbox{red!0}{\strut -} \colorbox{red!1}{\strut Does} \colorbox{red!0}{\strut Not} \colorbox{red!3}{\strut Convert} \colorbox{red!0}{\strut Voltageby} \colorbox{red!0}{\strut Orei} \colorbox{red!0}{\strut .} \colorbox{red!0}{\strut 19.99} \colorbox{red!0}{\strut .} \colorbox{red!0}{\strut 19} \colorbox{red!0}{\strut 99Only} \colorbox{red!0}{\strut 18} \colorbox{red!0}{\strut left} \colorbox{red!0}{\strut in} \colorbox{red!0}{\strut stock} \colorbox{red!0}{\strut -} \colorbox{red!1}{\strut order} \colorbox{red!0}{\strut soon.FREE} \colorbox{red!1}{\strut Shipping} \colorbox{red!0}{\strut on} \colorbox{red!1}{\strut eligible} \colorbox{red!0}{\strut orders4.4} \colorbox{red!0}{\strut out} \colorbox{red!0}{\strut of} \colorbox{red!0}{\strut 5} \colorbox{red!1}{\strut stars} \colorbox{red!0}{\strut 257Amazon} \colorbox{red!0}{\strut s} \colorbox{red!0}{\strut ChoiceCeptics} \colorbox{red!0}{\strut CT-14} \colorbox{red!2}{\strut USA} \colorbox{red!0}{\strut to} \colorbox{red!4}{\strut Israel} \colorbox{red!0}{\strut ,} \colorbox{red!2}{\strut Palestine} \colorbox{red!3}{\strut Travel} \colorbox{red!4}{\strut Adapter} \colorbox{red!3}{\strut Plug} \colorbox{red!0}{\strut -} \colorbox{red!3}{\strut Type} \colorbox{red!1}{\strut H} \colorbox{red!0}{\strut .} \colorbox{red!0}{\strut 3} \colorbox{red!0}{\strut Pack} \colorbox{red!0}{\strut .} \colorbox{red!0}{\strut -} \colorbox{red!1}{\strut Dual} \colorbox{red!0}{\strut Inputs} \colorbox{red!0}{\strut -} \colorbox{red!1}{\strut Ultra} \colorbox{red!1}{\strut Compact} \colorbox{red!0}{\strut .} \colorbox{red!1}{\strut Does} \colorbox{red!0}{\strut Not} \colorbox{red!3}{\strut Convert} \colorbox{red!2}{\strut Voltage} \colorbox{red!0}{\strut .} \colorbox{red!0}{\strut by} \colorbox{red!0}{\strut Ceptics} \colorbox{red!0}{\strut .} \colorbox{red!0}{\strut 9.99} \colorbox{red!0}{\strut .} \colorbox{red!0}{\strut 9} \colorbox{red!0}{\strut 99More} \colorbox{red!0}{\strut Buying} \colorbox{red!0}{\strut Choices} \colorbox{red!0}{\strut .} \colorbox{red!0}{\strut 8.24} \colorbox{red!0}{\strut .} \colorbox{red!0}{\strut 5} \colorbox{red!0}{\strut used} \colorbox{red!0}{\strut .} \colorbox{red!0}{\strut new} \colorbox{red!0}{\strut offers} \colorbox{red!0}{\strut .} \colorbox{red!0}{\strut FREE} \colorbox{red!1}{\strut Shipping} \colorbox{red!0}{\strut on} \colorbox{red!1}{\strut eligible} \colorbox{red!0}{\strut orders} \colorbox{red!0}{\strut and} \colorbox{red!0}{\strut 1} \colorbox{red!0}{\strut more} \colorbox{red!0}{\strut promotion4.8} \colorbox{red!0}{\strut out} \colorbox{red!0}{\strut of} \colorbox{red!0}{\strut 5} \colorbox{red!1}{\strut stars} \colorbox{red!0}{\strut 3,746Ceptics} \colorbox{red!0}{\strut CTU-14} \colorbox{red!2}{\strut USA} \colorbox{red!0}{\strut to} \colorbox{red!4}{\strut Israel} \colorbox{red!0}{\strut ,} \colorbox{red!2}{\strut Palestine} \colorbox{red!3}{\strut Travel} \colorbox{red!4}{\strut Adapter} \colorbox{red!3}{\strut Plug} \colorbox{red!0}{\strut With} \colorbox{red!1}{\strut Dual} \colorbox{red!4}{\strut USB} \colorbox{red!0}{\strut -} \colorbox{red!3}{\strut Type} \colorbox{red!1}{\strut H} \colorbox{red!0}{\strut -} \colorbox{red!1}{\strut Ultra} \colorbox{red!0}{\strut Compactby} \colorbox{red!0}{\strut Ceptics} \colorbox{red!0}{\strut .} \colorbox{red!0}{\strut 12.99} \colorbox{red!0}{\strut .} \colorbox{red!0}{\strut 12} \colorbox{red!0}{\strut 99} \colorbox{red!0}{\strut .} \colorbox{red!0}{\strut 14.99More} \colorbox{red!0}{\strut Buying} \colorbox{red!0}{\strut Choices} \colorbox{red!0}{\strut .} \colorbox{red!0}{\strut 11.37} \colorbox{red!0}{\strut .} \colorbox{red!0}{\strut 4} \colorbox{red!0}{\strut used} \colorbox{red!0}{\strut .} \colorbox{red!0}{\strut new} \colorbox{red!0}{\strut offers} \colorbox{red!0}{\strut .} \colorbox{red!0}{\strut FREE} \colorbox{red!1}{\strut Shipping} \colorbox{red!0}{\strut on} \colorbox{red!1}{\strut eligible} \colorbox{red!0}{\strut orders4.7} \colorbox{red!0}{\strut out} \colorbox{red!0}{\strut of} \colorbox{red!0}{\strut 5} \colorbox{red!1}{\strut stars} \colorbox{red!0}{\strut 2,193VCT} \colorbox{red!0}{\strut VP-5} \colorbox{red!4}{\strut Israel} \colorbox{red!4}{\strut Adapter} \colorbox{red!3}{\strut Plug} \colorbox{red!3}{\strut Converts} \colorbox{red!2}{\strut USA} \colorbox{red!3}{\strut Plug} \colorbox{red!0}{\strut to} \colorbox{red!4}{\strut Israel} \colorbox{red!0}{\strut Plugby} \colorbox{red!0}{\strut VCT} \colorbox{red!0}{\strut .} \colorbox{red!0}{\strut 6.50} \colorbox{red!0}{\strut .} \colorbox{red!0}{\strut 6} \colorbox{red!0}{\strut 50More} \colorbox{red!0}{\strut Buying} \colorbox{red!0}{\strut Choices} \colorbox{red!0}{\strut .} \colorbox{red!0}{\strut 4.50} \colorbox{red!0}{\strut .} \colorbox{red!0}{\strut 3} \colorbox{red!0}{\strut new} \colorbox{red!0}{\strut offers} \colorbox{red!0}{\strut .} \colorbox{red!0}{\strut FREE} \colorbox{red!1}{\strut Shipping} \colorbox{red!0}{\strut on} \colorbox{red!1}{\strut eligible} \colorbox{red!0}{\strut orders3.9} \colorbox{red!0}{\strut out} \colorbox{red!0}{\strut of} \colorbox{red!0}{\strut 5} \colorbox{red!1}{\strut stars} \colorbox{red!0}{\strut 94Ceptics} \colorbox{red!4}{\strut Israel} \colorbox{red!3}{\strut Travel} \colorbox{red!3}{\strut Plug} \colorbox{red!4}{\strut Adapter} \colorbox{red!0}{\strut .} \colorbox{red!3}{\strut Type} \colorbox{red!1}{\strut H} \colorbox{red!0}{\strut .} \colorbox{red!0}{\strut -} \colorbox{red!0}{\strut 3} \colorbox{red!0}{\strut Pack} \colorbox{red!0}{\strut .} \colorbox{red!0}{\strut Grounded} \colorbox{red!0}{\strut .} \colorbox{red!2}{\strut Universal} \colorbox{red!0}{\strut .} \colorbox{red!0}{\strut .} \colorbox{red!0}{\strut GP-14-3PK} \colorbox{red!0}{\strut .} \colorbox{red!0}{\strut by} \colorbox{red!0}{\strut Ceptics} \colorbox{red!0}{\strut .} \colorbox{red!0}{\strut 7.99} \colorbox{red!0}{\strut .} \colorbox{red!0}{\strut 7} \colorbox{red!0}{\strut 99FREE} \colorbox{red!1}{\strut Shipping} \colorbox{red!0}{\strut on} \colorbox{red!1}{\strut eligible} \colorbox{red!0}{\strut orders} \colorbox{red!0}{\strut and} \colorbox{red!0}{\strut 1} \colorbox{red!0}{\strut more} \colorbox{red!0}{\strut promotion4.5} \colorbox{red!0}{\strut out} \colorbox{red!0}{\strut of} \colorbox{red!0}{\strut 5} \colorbox{red!1}{\strut stars} \colorbox{red!0}{\strut 7,042Orei} \colorbox{red!4}{\strut Israel} \colorbox{red!1}{\strut 2} \colorbox{red!4}{\strut USB} \colorbox{red!0}{\strut .} \colorbox{red!0}{\strut 3.4A17W} \colorbox{red!0}{\strut .} \colorbox{red!3}{\strut Travel} \colorbox{red!0}{\strut Charger} \colorbox{red!0}{\strut for} \colorbox{red!0}{\strut all} \colorbox{red!0}{\strut iPhone} \colorbox{red!0}{\strut ,} \colorbox{red!0}{\strut iPad} \colorbox{red!0}{\strut ,} \colorbox{red!0}{\strut Samsung} \colorbox{red!0}{\strut Galaxy} \colorbox{red!0}{\strut ,} \colorbox{red!0}{\strut Android} \colorbox{red!0}{\strut ,} \colorbox{red!1}{\strut HTC} \colorbox{red!0}{\strut One} \colorbox{red!0}{\strut ,} \colorbox{red!1}{\strut Motorola} \colorbox{red!0}{\strut ,} \colorbox{red!0}{\strut LG} \colorbox{red!0}{\strut .} \colorbox{red!0}{\strut W2U-H} \colorbox{red!0}{\strut .} \colorbox{red!0}{\strut by} \colorbox{red!0}{\strut Orei} \colorbox{red!0}{\strut .} \colorbox{red!0}{\strut 11.99} \colorbox{red!0}{\strut .} 
}}}
\end{CJK*}

query: what is the butler's name in the addams family

\begin{CJK*}{UTF8}{gbsn}
{\setlength{\fboxsep}{0pt}\colorbox{white!0}{\parbox{0.9\textwidth}{
\colorbox{red!23}{\strut Lurch} \colorbox{red!0}{\strut .} \colorbox{red!0}{\strut The} \colorbox{red!2}{\strut Addams} \colorbox{red!1}{\strut Family} \colorbox{red!0}{\strut .} \colorbox{red!0}{\strut .} \colorbox{red!0}{\strut From} \colorbox{red!0}{\strut Wikipedia} \colorbox{red!0}{\strut ,} \colorbox{red!0}{\strut the} \colorbox{red!0}{\strut free} \colorbox{red!0}{\strut encyclopedianavigation} \colorbox{red!0}{\strut search} \colorbox{red!0}{\strut .} \colorbox{red!0}{\strut hide} \colorbox{red!0}{\strut .} \colorbox{red!0}{\strut This} \colorbox{red!0}{\strut article} \colorbox{red!0}{\strut has} \colorbox{red!0}{\strut multiple} \colorbox{red!0}{\strut issues} \colorbox{red!0}{\strut .} \colorbox{red!0}{\strut Please} \colorbox{red!0}{\strut help} \colorbox{red!0}{\strut improve} \colorbox{red!0}{\strut it} \colorbox{red!0}{\strut or} \colorbox{red!0}{\strut discuss} \colorbox{red!0}{\strut these} \colorbox{red!0}{\strut issues} \colorbox{red!0}{\strut on} \colorbox{red!0}{\strut the} \colorbox{red!0}{\strut talk} \colorbox{red!0}{\strut page} \colorbox{red!0}{\strut .} \colorbox{red!0}{\strut .} \colorbox{red!0}{\strut Learn} \colorbox{red!1}{\strut how} \colorbox{red!0}{\strut and} \colorbox{red!0}{\strut when} \colorbox{red!0}{\strut to} \colorbox{red!0}{\strut remove} \colorbox{red!0}{\strut these} \colorbox{red!0}{\strut template} \colorbox{red!0}{\strut messages} \colorbox{red!0}{\strut .} \colorbox{red!0}{\strut This} \colorbox{red!0}{\strut article} \colorbox{red!0}{\strut needs} \colorbox{red!0}{\strut additional} \colorbox{red!0}{\strut citations} \colorbox{red!0}{\strut for} \colorbox{red!0}{\strut verification} \colorbox{red!0}{\strut .} \colorbox{red!0}{\strut .} \colorbox{red!0}{\strut January} \colorbox{red!0}{\strut 2008} \colorbox{red!0}{\strut .} \colorbox{red!0}{\strut This} \colorbox{red!0}{\strut article} \colorbox{red!0}{\strut possibly} \colorbox{red!0}{\strut contains} \colorbox{red!1}{\strut original} \colorbox{red!0}{\strut research} \colorbox{red!0}{\strut .} \colorbox{red!0}{\strut .} \colorbox{red!0}{\strut December} \colorbox{red!0}{\strut 2012} \colorbox{red!0}{\strut .} \colorbox{red!4}{\strut LurchTed} \colorbox{red!1}{\strut Cassidy} \colorbox{red!0}{\strut .} \colorbox{red!0}{\strut on} \colorbox{red!0}{\strut right} \colorbox{red!0}{\strut .} \colorbox{red!0}{\strut as} \colorbox{red!23}{\strut Lurch} \colorbox{red!0}{\strut with} \colorbox{red!0}{\strut Jackie} \colorbox{red!0}{\strut Coogan} \colorbox{red!0}{\strut as} \colorbox{red!1}{\strut Uncle} \colorbox{red!1}{\strut Fester} \colorbox{red!0}{\strut .} \colorbox{red!0}{\strut left} \colorbox{red!0}{\strut .} \colorbox{red!0}{\strut .First} \colorbox{red!1}{\strut appearance} \colorbox{red!0}{\strut The} \colorbox{red!1}{\strut New} \colorbox{red!0}{\strut Yorker} \colorbox{red!2}{\strut cartoon} \colorbox{red!0}{\strut ,} \colorbox{red!0}{\strut .} \colorbox{red!0}{\strut 1938} \colorbox{red!0}{\strut .} \colorbox{red!1}{\strut Created} \colorbox{red!0}{\strut by} \colorbox{red!1}{\strut Charles} \colorbox{red!0}{\strut AddamsPortrayed} \colorbox{red!0}{\strut by} \colorbox{red!1}{\strut Ted} \colorbox{red!0}{\strut CassidyJim} \colorbox{red!0}{\strut CummingsCarel} \colorbox{red!0}{\strut StruyckenJohn} \colorbox{red!0}{\strut DeSantisRyan} \colorbox{red!0}{\strut Jacob} \colorbox{red!0}{\strut WoodInformationGender} \colorbox{red!0}{\strut MaleOccupation} \colorbox{red!0}{\strut ServantNationality} \colorbox{red!0}{\strut AmericanLurch} \colorbox{red!0}{\strut .} \colorbox{red!0}{\strut whose} \colorbox{red!0}{\strut first} \colorbox{red!1}{\strut name} \colorbox{red!0}{\strut is} \colorbox{red!0}{\strut unknown} \colorbox{red!0}{\strut .} \colorbox{red!0}{\strut is} \colorbox{red!0}{\strut a} \colorbox{red!0}{\strut fictional} \colorbox{red!1}{\strut character} \colorbox{red!1}{\strut created} \colorbox{red!0}{\strut by} \colorbox{red!0}{\strut American} \colorbox{red!0}{\strut cartoonist} \colorbox{red!1}{\strut Charles} \colorbox{red!2}{\strut Addams} \colorbox{red!0}{\strut as} \colorbox{red!0}{\strut a} \colorbox{red!1}{\strut manservant} \colorbox{red!0}{\strut to} \colorbox{red!0}{\strut The} \colorbox{red!2}{\strut Addams} \colorbox{red!1}{\strut Family} \colorbox{red!0}{\strut .} \colorbox{red!0}{\strut In} \colorbox{red!0}{\strut the} \colorbox{red!1}{\strut original} \colorbox{red!0}{\strut television} \colorbox{red!1}{\strut series} \colorbox{red!0}{\strut ,} \colorbox{red!23}{\strut Lurch} \colorbox{red!0}{\strut was} \colorbox{red!6}{\strut played} \colorbox{red!0}{\strut by} \colorbox{red!1}{\strut Ted} \colorbox{red!1}{\strut Cassidy} \colorbox{red!0}{\strut ,} \colorbox{red!18}{\strut who} \colorbox{red!0}{\strut used} \colorbox{red!0}{\strut the} \colorbox{red!0}{\strut famous} \colorbox{red!0}{\strut catchphrase} \colorbox{red!0}{\strut ,} \colorbox{red!0}{\strut .} \colorbox{red!0}{\strut .} \colorbox{red!0}{\strut You} \colorbox{red!0}{\strut rang} \colorbox{red!0}{\strut ?} \colorbox{red!0}{\strut .} \colorbox{red!0}{\strut .} \colorbox{red!0}{\strut .} \colorbox{red!0}{\strut a} \colorbox{red!0}{\strut similar} \colorbox{red!0}{\strut phrase} \colorbox{red!0}{\strut was} \colorbox{red!0}{\strut the} \colorbox{red!0}{\strut trademark} \colorbox{red!0}{\strut of} \colorbox{red!0}{\strut the} \colorbox{red!1}{\strut character} \colorbox{red!0}{\strut Maynard} \colorbox{red!0}{\strut G.} \colorbox{red!1}{\strut Krebs} \colorbox{red!0}{\strut in} \colorbox{red!0}{\strut The} \colorbox{red!0}{\strut Many} \colorbox{red!0}{\strut Loves} \colorbox{red!0}{\strut of} \colorbox{red!0}{\strut Dobie} \colorbox{red!0}{\strut Gillis} \colorbox{red!0}{\strut .} \colorbox{red!0}{\strut .Contents} \colorbox{red!0}{\strut .} \colorbox{red!0}{\strut hide} \colorbox{red!0}{\strut .} \colorbox{red!0}{\strut 1} \colorbox{red!0}{\strut Cartoons2} \colorbox{red!0}{\strut Characterization3} \colorbox{red!0}{\strut Backstory4} \colorbox{red!0}{\strut Influence5} \colorbox{red!0}{\strut ReferencesCartoons} \colorbox{red!0}{\strut .} \colorbox{red!0}{\strut edit} \colorbox{red!0}{\strut .} \colorbox{red!0}{\strut In} \colorbox{red!1}{\strut Charles} \colorbox{red!2}{\strut Addams} \colorbox{red!0}{\strut s} \colorbox{red!1}{\strut original} \colorbox{red!2}{\strut cartoons} \colorbox{red!0}{\strut ,} \colorbox{red!23}{\strut Lurch} \colorbox{red!0}{\strut is} \colorbox{red!0}{\strut often} \colorbox{red!0}{\strut seen} \colorbox{red!0}{\strut accompanying} \colorbox{red!0}{\strut the} \colorbox{red!0}{\strut rest} \colorbox{red!0}{\strut of} \colorbox{red!0}{\strut the} \colorbox{red!1}{\strut Family} \colorbox{red!0}{\strut ,} \colorbox{red!0}{\strut sometimes} \colorbox{red!0}{\strut carrying} \colorbox{red!0}{\strut a} \colorbox{red!0}{\strut feather-duster} \colorbox{red!0}{\strut .} \colorbox{red!0}{\strut In} \colorbox{red!0}{\strut a} \colorbox{red!0}{\strut couple} \colorbox{red!0}{\strut of} \colorbox{red!0}{\strut illustrations} \colorbox{red!0}{\strut ,} \colorbox{red!0}{\strut the} \colorbox{red!1}{\strut Family} \colorbox{red!0}{\strut is} \colorbox{red!0}{\strut seen} \colorbox{red!0}{\strut decorating} \colorbox{red!23}{\strut Lurch} \colorbox{red!0}{\strut like} \colorbox{red!0}{\strut they} \colorbox{red!0}{\strut would} \colorbox{red!0}{\strut a} \colorbox{red!0}{\strut Christmas} \colorbox{red!0}{\strut tree.Characterization} \colorbox{red!0}{\strut .} \colorbox{red!0}{\strut edit} \colorbox{red!0}{\strut .} \colorbox{red!0}{\strut This} \colorbox{red!0}{\strut section} \colorbox{red!0}{\strut is} \colorbox{red!0}{\strut written} \colorbox{red!0}{\strut like} \colorbox{red!0}{\strut a} \colorbox{red!0}{\strut personal} \colorbox{red!0}{\strut reflection} \colorbox{red!0}{\strut or} \colorbox{red!0}{\strut opinion} \colorbox{red!0}{\strut essay} \colorbox{red!0}{\strut that} \colorbox{red!0}{\strut states} \colorbox{red!0}{\strut a} \colorbox{red!0}{\strut Wikipedia} \colorbox{red!0}{\strut editor} \colorbox{red!0}{\strut s} \colorbox{red!0}{\strut personal} \colorbox{red!0}{\strut feelings} \colorbox{red!0}{\strut about} \colorbox{red!0}{\strut a} \colorbox{red!0}{\strut topic} \colorbox{red!0}{\strut .} \colorbox{red!0}{\strut Please} \colorbox{red!0}{\strut help} \colorbox{red!0}{\strut improve} \colorbox{red!0}{\strut it} \colorbox{red!0}{\strut by} \colorbox{red!0}{\strut rewriting} \colorbox{red!0}{\strut it} \colorbox{red!0}{\strut in} \colorbox{red!0}{\strut an} \colorbox{red!0}{\strut encyclopedic} \colorbox{red!0}{\strut style} \colorbox{red!0}{\strut .} \colorbox{red!0}{\strut .} \colorbox{red!0}{\strut April} \colorbox{red!0}{\strut 2014} \colorbox{red!0}{\strut .} \colorbox{red!0}{\strut .} \colorbox{red!0}{\strut Learn} \colorbox{red!1}{\strut how} \colorbox{red!0}{\strut and} \colorbox{red!0}{\strut when} \colorbox{red!0}{\strut to} \colorbox{red!0}{\strut remove} \colorbox{red!0}{\strut this} \colorbox{red!0}{\strut template} \colorbox{red!0}{\strut message} \colorbox{red!0}{\strut .} \colorbox{red!23}{\strut Lurch} \colorbox{red!0}{\strut is} \colorbox{red!0}{\strut a} \colorbox{red!0}{\strut 6} \colorbox{red!0}{\strut ft} \colorbox{red!0}{\strut 9} \colorbox{red!0}{\strut in} \colorbox{red!0}{\strut .} \colorbox{red!0}{\strut 2.05} 
}}}
\end{CJK*}

\begin{CJK*}{UTF8}{gbsn}
{\setlength{\fboxsep}{0pt}\colorbox{white!0}{\parbox{0.9\textwidth}{
\colorbox{red!0}{\strut The} \colorbox{red!11}{\strut Addams} \colorbox{red!10}{\strut Family} \colorbox{red!0}{\strut .} \colorbox{red!0}{\strut 1964} \colorbox{red!0}{\strut publicity} \colorbox{red!0}{\strut photo} \colorbox{red!0}{\strut for} \colorbox{red!0}{\strut the} \colorbox{red!1}{\strut TV} \colorbox{red!1}{\strut series} \colorbox{red!0}{\strut .} \colorbox{red!0}{\strut From} \colorbox{red!0}{\strut the} \colorbox{red!0}{\strut left} \colorbox{red!0}{\strut .} \colorbox{red!0}{\strut Lisa} \colorbox{red!0}{\strut Loring} \colorbox{red!0}{\strut as} \colorbox{red!1}{\strut Wednesday} \colorbox{red!0}{\strut ,} \colorbox{red!0}{\strut John} \colorbox{red!0}{\strut Astin} \colorbox{red!0}{\strut as} \colorbox{red!1}{\strut Gomez} \colorbox{red!0}{\strut ,} \colorbox{red!0}{\strut Ted} \colorbox{red!0}{\strut Cassidy} \colorbox{red!0}{\strut as} \colorbox{red!1}{\strut Lurch} \colorbox{red!0}{\strut ,} \colorbox{red!0}{\strut Carolyn} \colorbox{red!0}{\strut Jones} \colorbox{red!0}{\strut as} \colorbox{red!1}{\strut Morticia} \colorbox{red!0}{\strut and} \colorbox{red!0}{\strut Ken} \colorbox{red!0}{\strut Weatherwax} \colorbox{red!0}{\strut as} \colorbox{red!0}{\strut Pugsley.The} \colorbox{red!11}{\strut Addams} \colorbox{red!10}{\strut Family} \colorbox{red!0}{\strut are} \colorbox{red!0}{\strut an} \colorbox{red!0}{\strut eccentric} \colorbox{red!0}{\strut and} \colorbox{red!0}{\strut rather} \colorbox{red!0}{\strut macabre} \colorbox{red!0}{\strut fictional} \colorbox{red!10}{\strut family} \colorbox{red!0}{\strut .} \colorbox{red!0}{\strut They} \colorbox{red!0}{\strut were} \colorbox{red!1}{\strut created} \colorbox{red!0}{\strut by} \colorbox{red!0}{\strut the} \colorbox{red!1}{\strut American} \colorbox{red!0}{\strut cartoonist} \colorbox{red!1}{\strut Charles} \colorbox{red!11}{\strut Addams} \colorbox{red!0}{\strut and} \colorbox{red!0}{\strut first} \colorbox{red!1}{\strut appeared} \colorbox{red!0}{\strut in} \colorbox{red!0}{\strut a} \colorbox{red!1}{\strut series} \colorbox{red!0}{\strut of} \colorbox{red!0}{\strut single-panel} \colorbox{red!2}{\strut cartoons} \colorbox{red!0}{\strut in} \colorbox{red!0}{\strut The} \colorbox{red!1}{\strut New} \colorbox{red!0}{\strut Yorker} \colorbox{red!1}{\strut magazine} \colorbox{red!0}{\strut in} \colorbox{red!0}{\strut 1938.The} \colorbox{red!0}{\strut extremely} \colorbox{red!0}{\strut wealthy} \colorbox{red!10}{\strut family} \colorbox{red!1}{\strut live} \colorbox{red!0}{\strut in} \colorbox{red!0}{\strut a} \colorbox{red!0}{\strut mansion} \colorbox{red!0}{\strut that} \colorbox{red!0}{\strut has} \colorbox{red!0}{\strut become} \colorbox{red!0}{\strut somewhat} \colorbox{red!0}{\strut run} \colorbox{red!0}{\strut down} \colorbox{red!0}{\strut ,} \colorbox{red!0}{\strut giving} \colorbox{red!0}{\strut it} \colorbox{red!0}{\strut the} \colorbox{red!0}{\strut appearance} \colorbox{red!0}{\strut of} \colorbox{red!0}{\strut a} \colorbox{red!0}{\strut typical} \colorbox{red!0}{\strut haunted} \colorbox{red!0}{\strut house} \colorbox{red!0}{\strut .} \colorbox{red!0}{\strut The} \colorbox{red!10}{\strut family} \colorbox{red!0}{\strut consists} \colorbox{red!0}{\strut of} \colorbox{red!0}{\strut a} \colorbox{red!1}{\strut husband} \colorbox{red!0}{\strut and} \colorbox{red!1}{\strut wife} \colorbox{red!0}{\strut ,} \colorbox{red!0}{\strut their} \colorbox{red!0}{\strut two} \colorbox{red!0}{\strut young} \colorbox{red!1}{\strut children} \colorbox{red!0}{\strut and} \colorbox{red!0}{\strut two} \colorbox{red!0}{\strut older} \colorbox{red!1}{\strut relatives} \colorbox{red!0}{\strut .} \colorbox{red!0}{\strut They} \colorbox{red!0}{\strut have} \colorbox{red!0}{\strut a} \colorbox{red!1}{\strut butler} \colorbox{red!3}{\strut who} \colorbox{red!0}{\strut resembles} \colorbox{red!1}{\strut Frankenstein} \colorbox{red!0}{\strut s} \colorbox{red!0}{\strut monster} \colorbox{red!0}{\strut .} \colorbox{red!0}{\strut as} \colorbox{red!1}{\strut played} \colorbox{red!0}{\strut by} \colorbox{red!0}{\strut Boris} \colorbox{red!0}{\strut Karloff} \colorbox{red!0}{\strut in} \colorbox{red!0}{\strut the} \colorbox{red!0}{\strut 1931} \colorbox{red!1}{\strut movie} \colorbox{red!1}{\strut Frankenstein} \colorbox{red!0}{\strut .} \colorbox{red!0}{\strut and} \colorbox{red!0}{\strut various} \colorbox{red!0}{\strut other} \colorbox{red!10}{\strut family} \colorbox{red!0}{\strut members} \colorbox{red!0}{\strut have} \colorbox{red!0}{\strut visited} \colorbox{red!0}{\strut them} \colorbox{red!0}{\strut from} \colorbox{red!0}{\strut time} \colorbox{red!0}{\strut to} \colorbox{red!0}{\strut time.The} \colorbox{red!1}{\strut characters} \colorbox{red!0}{\strut are} \colorbox{red!0}{\strut unnamed} \colorbox{red!0}{\strut in} \colorbox{red!1}{\strut Charles} \colorbox{red!11}{\strut Addams} \colorbox{red!0}{\strut .} \colorbox{red!2}{\strut cartoons} \colorbox{red!0}{\strut .} \colorbox{red!1}{\strut When} \colorbox{red!0}{\strut a} \colorbox{red!1}{\strut TV} \colorbox{red!0}{\strut comedy} \colorbox{red!1}{\strut series} \colorbox{red!1}{\strut based} \colorbox{red!0}{\strut on} \colorbox{red!0}{\strut the} \colorbox{red!1}{\strut characters} \colorbox{red!0}{\strut was} \colorbox{red!0}{\strut developed} \colorbox{red!0}{\strut in} \colorbox{red!0}{\strut 1964} \colorbox{red!0}{\strut ,} \colorbox{red!1}{\strut Charles} \colorbox{red!11}{\strut Addams} \colorbox{red!0}{\strut was} \colorbox{red!0}{\strut asked} \colorbox{red!0}{\strut to} \colorbox{red!0}{\strut provide} \colorbox{red!2}{\strut names} \colorbox{red!0}{\strut for} \colorbox{red!0}{\strut them} \colorbox{red!0}{\strut .} \colorbox{red!0}{\strut He} \colorbox{red!2}{\strut named} \colorbox{red!0}{\strut the} \colorbox{red!1}{\strut butler} \colorbox{red!0}{\strut .} \colorbox{red!0}{\strut .} \colorbox{red!1}{\strut Lurch} \colorbox{red!0}{\strut .} \colorbox{red!0}{\strut .} \colorbox{red!0}{\strut ,} \colorbox{red!0}{\strut the} \colorbox{red!1}{\strut husband} \colorbox{red!0}{\strut and} \colorbox{red!1}{\strut wife} \colorbox{red!0}{\strut .} \colorbox{red!0}{\strut .} \colorbox{red!1}{\strut Gomez} \colorbox{red!0}{\strut .} \colorbox{red!0}{\strut .} \colorbox{red!0}{\strut and} \colorbox{red!0}{\strut .} \colorbox{red!0}{\strut .} \colorbox{red!1}{\strut Morticia} \colorbox{red!0}{\strut .} \colorbox{red!0}{\strut .} \colorbox{red!0}{\strut ,} \colorbox{red!0}{\strut the} \colorbox{red!0}{\strut two} \colorbox{red!0}{\strut older} \colorbox{red!1}{\strut relatives} \colorbox{red!0}{\strut .} \colorbox{red!0}{\strut .} \colorbox{red!1}{\strut Uncle} \colorbox{red!1}{\strut Fester} \colorbox{red!0}{\strut .} \colorbox{red!0}{\strut .} \colorbox{red!0}{\strut and} \colorbox{red!0}{\strut .} \colorbox{red!0}{\strut .} \colorbox{red!1}{\strut Grandmama} \colorbox{red!1}{\strut Frump} \colorbox{red!0}{\strut .} \colorbox{red!0}{\strut .} \colorbox{red!0}{\strut and} \colorbox{red!0}{\strut the} \colorbox{red!1}{\strut children} \colorbox{red!0}{\strut .} \colorbox{red!0}{\strut .} \colorbox{red!1}{\strut Wednesday} \colorbox{red!0}{\strut .} \colorbox{red!0}{\strut .} \colorbox{red!0}{\strut and} \colorbox{red!0}{\strut .} \colorbox{red!0}{\strut .} \colorbox{red!0}{\strut Pubert} \colorbox{red!0}{\strut .} \colorbox{red!0}{\strut .} \colorbox{red!0}{\strut .} \colorbox{red!0}{\strut The} \colorbox{red!2}{\strut name} \colorbox{red!0}{\strut .} \colorbox{red!0}{\strut .} \colorbox{red!0}{\strut Pubert} \colorbox{red!0}{\strut .} \colorbox{red!0}{\strut .} \colorbox{red!0}{\strut was} \colorbox{red!0}{\strut rejected} \colorbox{red!0}{\strut by} \colorbox{red!0}{\strut the} \colorbox{red!1}{\strut show} \colorbox{red!0}{\strut s} \colorbox{red!0}{\strut producers} \colorbox{red!0}{\strut and} \colorbox{red!0}{\strut the} \colorbox{red!1}{\strut character} \colorbox{red!0}{\strut was} \colorbox{red!2}{\strut named} \colorbox{red!0}{\strut .} \colorbox{red!0}{\strut .} \colorbox{red!1}{\strut Pugsley} \colorbox{red!0}{\strut .} \colorbox{red!0}{\strut .} \colorbox{red!0}{\strut instead} \colorbox{red!0}{\strut .} \colorbox{red!0}{\strut The} \colorbox{red!2}{\strut name} \colorbox{red!0}{\strut .} \colorbox{red!0}{\strut .} \colorbox{red!0}{\strut Pubert} \colorbox{red!0}{\strut .} \colorbox{red!0}{\strut .} \colorbox{red!0}{\strut was} \colorbox{red!0}{\strut later} \colorbox{red!0}{\strut used} \colorbox{red!0}{\strut as} \colorbox{red!0}{\strut the} \colorbox{red!2}{\strut name} \colorbox{red!0}{\strut of} \colorbox{red!1}{\strut Gomez} \colorbox{red!0}{\strut and} \colorbox{red!1}{\strut Morticia} \colorbox{red!0}{\strut s} \colorbox{red!0}{\strut third} \colorbox{red!1}{\strut child} \colorbox{red!0}{\strut in} \colorbox{red!0}{\strut the} \colorbox{red!0}{\strut 1993} \colorbox{red!1}{\strut movie} \colorbox{red!0}{\strut The} \colorbox{red!11}{\strut Addams} \colorbox{red!10}{\strut Family} \colorbox{red!0}{\strut Values} \colorbox{red!0}{\strut .} \colorbox{red!0}{\strut .} \colorbox{red!0}{\strut .} \colorbox{red!1}{\strut Grandmama} 
}}}
\end{CJK*}

query: consolidate function

\begin{CJK*}{UTF8}{gbsn}
{\setlength{\fboxsep}{0pt}\colorbox{white!0}{\parbox{0.9\textwidth}{
\colorbox{red!10}{\strut Consolidate} \colorbox{red!6}{\strut data} \colorbox{red!0}{\strut in} \colorbox{red!0}{\strut multiple} \colorbox{red!2}{\strut worksheets} \colorbox{red!0}{\strut To} \colorbox{red!0}{\strut summarize} \colorbox{red!0}{\strut and} \colorbox{red!0}{\strut report} \colorbox{red!0}{\strut results} \colorbox{red!0}{\strut from} \colorbox{red!0}{\strut separate} \colorbox{red!2}{\strut worksheets} \colorbox{red!0}{\strut ,} \colorbox{red!0}{\strut you} \colorbox{red!0}{\strut can} \colorbox{red!10}{\strut consolidate} \colorbox{red!6}{\strut data} \colorbox{red!0}{\strut from} \colorbox{red!0}{\strut each} \colorbox{red!0}{\strut into} \colorbox{red!0}{\strut a} \colorbox{red!1}{\strut master} \colorbox{red!2}{\strut worksheet} \colorbox{red!0}{\strut .} \colorbox{red!0}{\strut The} \colorbox{red!2}{\strut worksheets} \colorbox{red!0}{\strut can} \colorbox{red!0}{\strut be} \colorbox{red!0}{\strut in} \colorbox{red!0}{\strut the} \colorbox{red!0}{\strut same} \colorbox{red!1}{\strut workbook} \colorbox{red!0}{\strut as} \colorbox{red!0}{\strut the} \colorbox{red!1}{\strut master} \colorbox{red!2}{\strut worksheet} \colorbox{red!0}{\strut or} \colorbox{red!0}{\strut in} \colorbox{red!0}{\strut other} \colorbox{red!1}{\strut workbooks} \colorbox{red!0}{\strut .} \colorbox{red!1}{\strut When} \colorbox{red!0}{\strut you} \colorbox{red!10}{\strut consolidate} \colorbox{red!6}{\strut data} \colorbox{red!0}{\strut ,} \colorbox{red!0}{\strut you} \colorbox{red!0}{\strut are} \colorbox{red!1}{\strut assembling} \colorbox{red!6}{\strut data} \colorbox{red!0}{\strut so} \colorbox{red!0}{\strut that} \colorbox{red!0}{\strut you} \colorbox{red!0}{\strut can} \colorbox{red!0}{\strut more} \colorbox{red!0}{\strut easily} \colorbox{red!0}{\strut update} \colorbox{red!0}{\strut and} \colorbox{red!0}{\strut aggregate} \colorbox{red!0}{\strut as} \colorbox{red!0}{\strut needed.For} \colorbox{red!0}{\strut example} \colorbox{red!0}{\strut ,} \colorbox{red!0}{\strut if} \colorbox{red!0}{\strut you} \colorbox{red!0}{\strut have} \colorbox{red!0}{\strut an} \colorbox{red!0}{\strut expense} \colorbox{red!2}{\strut worksheet} \colorbox{red!0}{\strut for} \colorbox{red!0}{\strut each} \colorbox{red!0}{\strut of} \colorbox{red!0}{\strut your} \colorbox{red!0}{\strut regional} \colorbox{red!0}{\strut offices} \colorbox{red!0}{\strut ,} \colorbox{red!0}{\strut you} \colorbox{red!0}{\strut might} \colorbox{red!0}{\strut use} \colorbox{red!10}{\strut consolidation} \colorbox{red!0}{\strut to} \colorbox{red!0}{\strut roll} \colorbox{red!0}{\strut these} \colorbox{red!0}{\strut figures} \colorbox{red!0}{\strut into} \colorbox{red!0}{\strut a} \colorbox{red!1}{\strut master} \colorbox{red!0}{\strut corporate} \colorbox{red!0}{\strut expense} \colorbox{red!2}{\strut worksheet} \colorbox{red!0}{\strut .} \colorbox{red!0}{\strut This} \colorbox{red!1}{\strut master} \colorbox{red!2}{\strut worksheet} \colorbox{red!0}{\strut might} \colorbox{red!0}{\strut also} \colorbox{red!0}{\strut contain} \colorbox{red!0}{\strut sales} \colorbox{red!0}{\strut totals} \colorbox{red!0}{\strut and} \colorbox{red!0}{\strut averages} \colorbox{red!0}{\strut ,} \colorbox{red!0}{\strut current} \colorbox{red!0}{\strut inventory} \colorbox{red!0}{\strut levels} \colorbox{red!0}{\strut ,} \colorbox{red!0}{\strut and} \colorbox{red!0}{\strut highest} \colorbox{red!0}{\strut selling} \colorbox{red!0}{\strut products} \colorbox{red!0}{\strut for} \colorbox{red!0}{\strut the} \colorbox{red!0}{\strut entire} \colorbox{red!0}{\strut enterprise.Tip} \colorbox{red!0}{\strut .} \colorbox{red!0}{\strut If} \colorbox{red!0}{\strut you} \colorbox{red!0}{\strut frequently} \colorbox{red!10}{\strut consolidate} \colorbox{red!6}{\strut data} \colorbox{red!0}{\strut ,} \colorbox{red!0}{\strut it} \colorbox{red!0}{\strut might} \colorbox{red!0}{\strut help} \colorbox{red!0}{\strut to} \colorbox{red!0}{\strut base} \colorbox{red!0}{\strut your} \colorbox{red!2}{\strut worksheets} \colorbox{red!0}{\strut on} \colorbox{red!0}{\strut a} \colorbox{red!2}{\strut worksheet} \colorbox{red!0}{\strut template} \colorbox{red!0}{\strut that} \colorbox{red!0}{\strut uses} \colorbox{red!0}{\strut a} \colorbox{red!0}{\strut consistent} \colorbox{red!0}{\strut layout} \colorbox{red!0}{\strut .} \colorbox{red!0}{\strut To} \colorbox{red!0}{\strut learn} \colorbox{red!0}{\strut more} \colorbox{red!0}{\strut about} \colorbox{red!0}{\strut Templates} \colorbox{red!0}{\strut ,} \colorbox{red!0}{\strut see} \colorbox{red!0}{\strut .} \colorbox{red!0}{\strut Create} \colorbox{red!0}{\strut a} \colorbox{red!0}{\strut template} \colorbox{red!0}{\strut .} \colorbox{red!0}{\strut This} \colorbox{red!0}{\strut is} \colorbox{red!0}{\strut also} \colorbox{red!0}{\strut an} \colorbox{red!0}{\strut ideal} \colorbox{red!0}{\strut time} \colorbox{red!0}{\strut to} \colorbox{red!0}{\strut set} \colorbox{red!0}{\strut up} \colorbox{red!0}{\strut your} \colorbox{red!0}{\strut template} \colorbox{red!0}{\strut with} \colorbox{red!3}{\strut Excel} \colorbox{red!0}{\strut tables.There} \colorbox{red!0}{\strut are} \colorbox{red!0}{\strut two} \colorbox{red!0}{\strut ways} \colorbox{red!0}{\strut to} \colorbox{red!10}{\strut consolidate} \colorbox{red!6}{\strut data} \colorbox{red!0}{\strut .} \colorbox{red!0}{\strut by} \colorbox{red!0}{\strut Category} \colorbox{red!0}{\strut or} \colorbox{red!0}{\strut by} \colorbox{red!0}{\strut Position.Consolidation} \colorbox{red!0}{\strut by} \colorbox{red!0}{\strut position} \colorbox{red!0}{\strut .} \colorbox{red!1}{\strut When} \colorbox{red!0}{\strut the} \colorbox{red!6}{\strut data} \colorbox{red!0}{\strut in} \colorbox{red!0}{\strut the} \colorbox{red!0}{\strut source} \colorbox{red!0}{\strut areas} \colorbox{red!0}{\strut is} \colorbox{red!0}{\strut arranged} \colorbox{red!0}{\strut in} \colorbox{red!0}{\strut the} \colorbox{red!0}{\strut same} \colorbox{red!0}{\strut order} \colorbox{red!0}{\strut and} \colorbox{red!0}{\strut uses} \colorbox{red!0}{\strut the} \colorbox{red!0}{\strut same} \colorbox{red!0}{\strut labels} \colorbox{red!0}{\strut .} \colorbox{red!0}{\strut Use} \colorbox{red!0}{\strut this} \colorbox{red!0}{\strut method} \colorbox{red!0}{\strut to} \colorbox{red!10}{\strut consolidate} \colorbox{red!6}{\strut data} \colorbox{red!0}{\strut from} \colorbox{red!0}{\strut a} \colorbox{red!0}{\strut series} \colorbox{red!0}{\strut of} \colorbox{red!2}{\strut worksheets} \colorbox{red!0}{\strut ,} \colorbox{red!0}{\strut such} \colorbox{red!0}{\strut as} \colorbox{red!0}{\strut departmental} \colorbox{red!0}{\strut budget} \colorbox{red!2}{\strut worksheets} \colorbox{red!0}{\strut that} \colorbox{red!0}{\strut have} \colorbox{red!0}{\strut been} \colorbox{red!0}{\strut created} \colorbox{red!0}{\strut from} \colorbox{red!0}{\strut the} \colorbox{red!0}{\strut same} \colorbox{red!0}{\strut template.Consolidation} \colorbox{red!0}{\strut by} \colorbox{red!0}{\strut category} \colorbox{red!0}{\strut .} \colorbox{red!1}{\strut When} \colorbox{red!0}{\strut the} \colorbox{red!6}{\strut data} \colorbox{red!0}{\strut in} \colorbox{red!0}{\strut the} \colorbox{red!0}{\strut source} \colorbox{red!0}{\strut areas} \colorbox{red!0}{\strut is} \colorbox{red!0}{\strut not} \colorbox{red!0}{\strut arranged} \colorbox{red!0}{\strut in} \colorbox{red!0}{\strut the} \colorbox{red!0}{\strut same} \colorbox{red!0}{\strut order} \colorbox{red!0}{\strut but} \colorbox{red!0}{\strut uses} \colorbox{red!0}{\strut the} \colorbox{red!0}{\strut same} \colorbox{red!0}{\strut labels} \colorbox{red!0}{\strut .} \colorbox{red!0}{\strut Use} \colorbox{red!0}{\strut this} \colorbox{red!0}{\strut method} \colorbox{red!0}{\strut to} \colorbox{red!10}{\strut consolidate} \colorbox{red!6}{\strut data} \colorbox{red!0}{\strut from} \colorbox{red!0}{\strut a} \colorbox{red!0}{\strut series} \colorbox{red!0}{\strut of} \colorbox{red!2}{\strut worksheets} \colorbox{red!0}{\strut that} \colorbox{red!0}{\strut have} \colorbox{red!0}{\strut different} \colorbox{red!0}{\strut layouts} \colorbox{red!0}{\strut but} \colorbox{red!0}{\strut have} \colorbox{red!0}{\strut the} \colorbox{red!0}{\strut same} \colorbox{red!6}{\strut data} \colorbox{red!0}{\strut labels.Consolidating} \colorbox{red!6}{\strut data} \colorbox{red!0}{\strut by} \colorbox{red!0}{\strut category} \colorbox{red!0}{\strut is} \colorbox{red!0}{\strut similar} \colorbox{red!0}{\strut to} \colorbox{red!0}{\strut creating} \colorbox{red!0}{\strut a} \colorbox{red!0}{\strut PivotTable} \colorbox{red!0}{\strut .} \colorbox{red!0}{\strut With} \colorbox{red!0}{\strut a} \colorbox{red!0}{\strut PivotTable} \colorbox{red!0}{\strut ,} \colorbox{red!0}{\strut however} \colorbox{red!0}{\strut ,} \colorbox{red!0}{\strut you} \colorbox{red!0}{\strut can} \colorbox{red!0}{\strut easily} \colorbox{red!0}{\strut reorganize} \colorbox{red!0}{\strut the} \colorbox{red!0}{\strut categories} \colorbox{red!0}{\strut .} \colorbox{red!0}{\strut If} \colorbox{red!0}{\strut you} \colorbox{red!0}{\strut want} \colorbox{red!0}{\strut a} \colorbox{red!0}{\strut more} \colorbox{red!0}{\strut flexible} \colorbox{red!10}{\strut consolidation} \colorbox{red!0}{\strut by} \colorbox{red!0}{\strut category} 
}}}
\end{CJK*}

\begin{CJK*}{UTF8}{gbsn}
{\setlength{\fboxsep}{0pt}\colorbox{white!0}{\parbox{0.9\textwidth}{
\colorbox{red!7}{\strut How} \colorbox{red!0}{\strut to} \colorbox{red!11}{\strut Consolidate} \colorbox{red!0}{\strut in} \colorbox{red!11}{\strut Excel} \colorbox{red!0}{\strut Edit} \colorbox{red!0}{\strut ArticleHow} \colorbox{red!0}{\strut to} \colorbox{red!11}{\strut Consolidate} \colorbox{red!0}{\strut in} \colorbox{red!0}{\strut ExcelFour} \colorbox{red!2}{\strut Methods} \colorbox{red!0}{\strut .} \colorbox{red!11}{\strut Consolidate} \colorbox{red!0}{\strut According} \colorbox{red!0}{\strut to} \colorbox{red!0}{\strut the} \colorbox{red!1}{\strut Position} \colorbox{red!0}{\strut in} \colorbox{red!0}{\strut an} \colorbox{red!11}{\strut Excel} \colorbox{red!0}{\strut WorksheetIdentify} \colorbox{red!0}{\strut Categories} \colorbox{red!0}{\strut to} \colorbox{red!11}{\strut Consolidate} \colorbox{red!11}{\strut Excel} \colorbox{red!1}{\strut Data} \colorbox{red!0}{\strut Use} \colorbox{red!1}{\strut Formulas} \colorbox{red!0}{\strut to} \colorbox{red!11}{\strut Consolidate} \colorbox{red!11}{\strut Excel} \colorbox{red!0}{\strut DataAccess} \colorbox{red!0}{\strut the} \colorbox{red!0}{\strut PivotTable} \colorbox{red!1}{\strut function} \colorbox{red!0}{\strut Community} \colorbox{red!0}{\strut Q} \colorbox{red!0}{\strut .} \colorbox{red!0}{\strut AMicrosoft} \colorbox{red!1}{\strut Office} \colorbox{red!11}{\strut Excel} \colorbox{red!0}{\strut comes} \colorbox{red!0}{\strut with} \colorbox{red!0}{\strut several} \colorbox{red!0}{\strut features} \colorbox{red!0}{\strut for} \colorbox{red!0}{\strut customizing} \colorbox{red!1}{\strut tables} \colorbox{red!0}{\strut and} \colorbox{red!0}{\strut charts} \colorbox{red!0}{\strut full} \colorbox{red!0}{\strut of} \colorbox{red!0}{\strut important} \colorbox{red!1}{\strut data} \colorbox{red!0}{\strut .} \colorbox{red!0}{\strut The} \colorbox{red!1}{\strut program} \colorbox{red!0}{\strut also} \colorbox{red!0}{\strut offers} \colorbox{red!1}{\strut efficient} \colorbox{red!1}{\strut ways} \colorbox{red!0}{\strut to} \colorbox{red!0}{\strut combine} \colorbox{red!0}{\strut and} \colorbox{red!0}{\strut summarize} \colorbox{red!1}{\strut data} \colorbox{red!0}{\strut from} \colorbox{red!0}{\strut multiple} \colorbox{red!1}{\strut files} \colorbox{red!0}{\strut ,} \colorbox{red!0}{\strut also} \colorbox{red!0}{\strut known} \colorbox{red!0}{\strut as} \colorbox{red!1}{\strut worksheets} \colorbox{red!0}{\strut .} \colorbox{red!1}{\strut Common} \colorbox{red!2}{\strut methods} \colorbox{red!0}{\strut to} \colorbox{red!11}{\strut consolidate} \colorbox{red!0}{\strut in} \colorbox{red!11}{\strut Excel} \colorbox{red!0}{\strut include} \colorbox{red!1}{\strut consolidating} \colorbox{red!0}{\strut by} \colorbox{red!1}{\strut position} \colorbox{red!0}{\strut ,} \colorbox{red!0}{\strut by} \colorbox{red!1}{\strut category} \colorbox{red!0}{\strut ,} \colorbox{red!0}{\strut by} \colorbox{red!1}{\strut formula} \colorbox{red!0}{\strut or} \colorbox{red!0}{\strut by} \colorbox{red!0}{\strut using} \colorbox{red!11}{\strut Excel} \colorbox{red!0}{\strut .} \colorbox{red!0}{\strut s} \colorbox{red!1}{\strut Pivot} \colorbox{red!1}{\strut Table} \colorbox{red!0}{\strut feature} \colorbox{red!0}{\strut .} \colorbox{red!0}{\strut Scroll} \colorbox{red!0}{\strut past} \colorbox{red!0}{\strut the} \colorbox{red!0}{\strut jump} \colorbox{red!0}{\strut to} \colorbox{red!0}{\strut learn} \colorbox{red!7}{\strut how} \colorbox{red!0}{\strut to} \colorbox{red!11}{\strut consolidate} \colorbox{red!0}{\strut in} \colorbox{red!11}{\strut Excel} \colorbox{red!0}{\strut so} \colorbox{red!0}{\strut that} \colorbox{red!0}{\strut your} \colorbox{red!0}{\strut information} \colorbox{red!0}{\strut appears} \colorbox{red!0}{\strut in} \colorbox{red!0}{\strut a} \colorbox{red!0}{\strut master} \colorbox{red!1}{\strut worksheet} \colorbox{red!0}{\strut as} \colorbox{red!0}{\strut a} \colorbox{red!0}{\strut reference} \colorbox{red!0}{\strut whenever} \colorbox{red!0}{\strut you} \colorbox{red!0}{\strut need} \colorbox{red!0}{\strut to} \colorbox{red!0}{\strut generate} \colorbox{red!0}{\strut reports} \colorbox{red!0}{\strut .} 
}}}
\end{CJK*}

query: what do partnerships file tax in michigan

\begin{CJK*}{UTF8}{gbsn}
{\setlength{\fboxsep}{0pt}\colorbox{white!0}{\parbox{0.9\textwidth}{
\colorbox{red!3}{\strut How} \colorbox{red!0}{\strut to} \colorbox{red!1}{\strut Pay} \colorbox{red!2}{\strut Taxes} \colorbox{red!0}{\strut for} \colorbox{red!0}{\strut a} \colorbox{red!1}{\strut Limited} \colorbox{red!1}{\strut Liability} \colorbox{red!1}{\strut Corporation} \colorbox{red!0}{\strut in} \colorbox{red!8}{\strut Michigan} \colorbox{red!0}{\strut As} \colorbox{red!0}{\strut a} \colorbox{red!1}{\strut limited} \colorbox{red!1}{\strut liability} \colorbox{red!1}{\strut company} \colorbox{red!0}{\strut in} \colorbox{red!8}{\strut Michigan} \colorbox{red!0}{\strut ,} \colorbox{red!0}{\strut you} \colorbox{red!0}{\strut have} \colorbox{red!2}{\strut tax} \colorbox{red!0}{\strut obligations} \colorbox{red!0}{\strut to} \colorbox{red!0}{\strut the} \colorbox{red!1}{\strut state} \colorbox{red!0}{\strut and} \colorbox{red!0}{\strut the} \colorbox{red!1}{\strut IRS} \colorbox{red!0}{\strut .} \colorbox{red!2}{\strut Tax} \colorbox{red!0}{\strut obligations} \colorbox{red!0}{\strut for} \colorbox{red!11}{\strut LLCs} \colorbox{red!0}{\strut vary} \colorbox{red!0}{\strut ,} \colorbox{red!0}{\strut depending} \colorbox{red!0}{\strut on} \colorbox{red!0}{\strut whether} \colorbox{red!0}{\strut you} \colorbox{red!0}{\strut sell} \colorbox{red!0}{\strut or} \colorbox{red!0}{\strut rent} \colorbox{red!0}{\strut goods} \colorbox{red!0}{\strut ,} \colorbox{red!0}{\strut or} \colorbox{red!0}{\strut have} \colorbox{red!0}{\strut employees} \colorbox{red!0}{\strut .} \colorbox{red!0}{\strut After} \colorbox{red!1}{\strut registering} \colorbox{red!0}{\strut to} \colorbox{red!1}{\strut pay} \colorbox{red!1}{\strut state} \colorbox{red!2}{\strut taxes} \colorbox{red!0}{\strut and} \colorbox{red!0}{\strut determining} \colorbox{red!0}{\strut the} \colorbox{red!2}{\strut taxes} \colorbox{red!0}{\strut for} \colorbox{red!0}{\strut which} \colorbox{red!0}{\strut your} \colorbox{red!11}{\strut LLC} \colorbox{red!0}{\strut is} \colorbox{red!0}{\strut responsible} \colorbox{red!0}{\strut ,} \colorbox{red!0}{\strut your} \colorbox{red!1}{\strut business} \colorbox{red!2}{\strut taxes} \colorbox{red!0}{\strut may} \colorbox{red!0}{\strut be} \colorbox{red!0}{\strut paid} \colorbox{red!0}{\strut online} \colorbox{red!0}{\strut via} \colorbox{red!0}{\strut the} \colorbox{red!8}{\strut Michigan} \colorbox{red!0}{\strut Department} \colorbox{red!0}{\strut of} \colorbox{red!0}{\strut Treasury} \colorbox{red!0}{\strut website} \colorbox{red!0}{\strut or} \colorbox{red!0}{\strut by} \colorbox{red!0}{\strut mail.Registration} \colorbox{red!0}{\strut for} \colorbox{red!8}{\strut Michigan} \colorbox{red!0}{\strut TaxesNew} \colorbox{red!1}{\strut businesses} \colorbox{red!0}{\strut in} \colorbox{red!8}{\strut Michigan} \colorbox{red!0}{\strut should} \colorbox{red!0}{\strut use} \colorbox{red!0}{\strut Form} \colorbox{red!0}{\strut 518} \colorbox{red!0}{\strut ,} \colorbox{red!0}{\strut Registration} \colorbox{red!0}{\strut for} \colorbox{red!8}{\strut Michigan} \colorbox{red!2}{\strut Taxes} \colorbox{red!0}{\strut ,} \colorbox{red!0}{\strut to} \colorbox{red!0}{\strut register} \colorbox{red!0}{\strut to} \colorbox{red!1}{\strut pay} \colorbox{red!2}{\strut taxes} \colorbox{red!0}{\strut .} \colorbox{red!0}{\strut Indicate} \colorbox{red!0}{\strut whether} \colorbox{red!0}{\strut you} \colorbox{red!0}{\strut sell} \colorbox{red!0}{\strut tangible} \colorbox{red!0}{\strut property} \colorbox{red!0}{\strut and} \colorbox{red!0}{\strut if} \colorbox{red!0}{\strut you} \colorbox{red!0}{\strut re} \colorbox{red!0}{\strut liable} \colorbox{red!0}{\strut for} \colorbox{red!1}{\strut sales} \colorbox{red!2}{\strut tax} \colorbox{red!0}{\strut or} \colorbox{red!0}{\strut if} \colorbox{red!0}{\strut you} \colorbox{red!0}{\strut lease} \colorbox{red!0}{\strut property} \colorbox{red!0}{\strut ,} \colorbox{red!0}{\strut which} \colorbox{red!1}{\strut requires} \colorbox{red!0}{\strut payment} \colorbox{red!0}{\strut of} \colorbox{red!0}{\strut a} \colorbox{red!0}{\strut use} \colorbox{red!2}{\strut tax} \colorbox{red!0}{\strut .} \colorbox{red!8}{\strut Michigan} \colorbox{red!0}{\strut also} \colorbox{red!2}{\strut taxes} \colorbox{red!0}{\strut tobacco} \colorbox{red!0}{\strut and} \colorbox{red!0}{\strut motor} \colorbox{red!0}{\strut fuels} \colorbox{red!0}{\strut .} \colorbox{red!0}{\strut if} \colorbox{red!0}{\strut your} \colorbox{red!1}{\strut business} \colorbox{red!0}{\strut sells} \colorbox{red!0}{\strut these} \colorbox{red!0}{\strut products} \colorbox{red!0}{\strut ,} \colorbox{red!0}{\strut the} \colorbox{red!0}{\strut Department} \colorbox{red!0}{\strut of} \colorbox{red!0}{\strut Treasury} \colorbox{red!0}{\strut suggests} \colorbox{red!0}{\strut you} \colorbox{red!0}{\strut register} \colorbox{red!0}{\strut to} \colorbox{red!1}{\strut pay} \colorbox{red!0}{\strut for} \colorbox{red!0}{\strut those} \colorbox{red!2}{\strut taxes} \colorbox{red!0}{\strut as} \colorbox{red!0}{\strut well} \colorbox{red!0}{\strut .} \colorbox{red!0}{\strut The} \colorbox{red!8}{\strut Michigan} \colorbox{red!0}{\strut Department} \colorbox{red!0}{\strut of} \colorbox{red!0}{\strut Treasury} \colorbox{red!0}{\strut recommends} \colorbox{red!0}{\strut Form} \colorbox{red!0}{\strut 518} \colorbox{red!0}{\strut to} \colorbox{red!0}{\strut be} \colorbox{red!0}{\strut mailed} \colorbox{red!0}{\strut at} \colorbox{red!0}{\strut least} \colorbox{red!0}{\strut six} \colorbox{red!0}{\strut weeks} \colorbox{red!0}{\strut before} \colorbox{red!0}{\strut you} \colorbox{red!0}{\strut begin} \colorbox{red!0}{\strut doing} \colorbox{red!1}{\strut business} \colorbox{red!0}{\strut in} \colorbox{red!0}{\strut the} \colorbox{red!0}{\strut state.Ready} \colorbox{red!0}{\strut to} \colorbox{red!1}{\strut start} \colorbox{red!0}{\strut your} \colorbox{red!11}{\strut LLC} \colorbox{red!0}{\strut ?} \colorbox{red!1}{\strut Start} \colorbox{red!0}{\strut an} \colorbox{red!11}{\strut LLC} \colorbox{red!0}{\strut Online} \colorbox{red!0}{\strut NowEmployer} \colorbox{red!0}{\strut ObligationsIf} \colorbox{red!0}{\strut your} \colorbox{red!11}{\strut LLC} \colorbox{red!0}{\strut employes} \colorbox{red!0}{\strut personnel} \colorbox{red!0}{\strut ,} \colorbox{red!0}{\strut register} \colorbox{red!0}{\strut to} \colorbox{red!1}{\strut pay} \colorbox{red!0}{\strut employer-related} \colorbox{red!2}{\strut taxes} \colorbox{red!0}{\strut ,} \colorbox{red!0}{\strut such} \colorbox{red!0}{\strut as} \colorbox{red!0}{\strut unemployment} \colorbox{red!0}{\strut insurance} \colorbox{red!0}{\strut .} \colorbox{red!0}{\strut You} \colorbox{red!0}{\strut may} \colorbox{red!0}{\strut also} \colorbox{red!0}{\strut be} \colorbox{red!0}{\strut required} \colorbox{red!0}{\strut to} \colorbox{red!0}{\strut withhold} \colorbox{red!0}{\strut both} \colorbox{red!0}{\strut federal} \colorbox{red!0}{\strut and} \colorbox{red!1}{\strut state} \colorbox{red!1}{\strut income} \colorbox{red!2}{\strut tax} \colorbox{red!0}{\strut from} \colorbox{red!0}{\strut their} \colorbox{red!1}{\strut pay} \colorbox{red!0}{\strut .} \colorbox{red!0}{\strut After} \colorbox{red!1}{\strut registering} \colorbox{red!0}{\strut to} \colorbox{red!1}{\strut pay} \colorbox{red!1}{\strut state} \colorbox{red!2}{\strut taxes} \colorbox{red!0}{\strut ,} \colorbox{red!0}{\strut the} \colorbox{red!1}{\strut state} \colorbox{red!0}{\strut will} \colorbox{red!0}{\strut send} \colorbox{red!0}{\strut you} \colorbox{red!0}{\strut personalized} \colorbox{red!2}{\strut tax} \colorbox{red!0}{\strut returns} \colorbox{red!0}{\strut to} \colorbox{red!0}{\strut report} \colorbox{red!0}{\strut any} \colorbox{red!0}{\strut withheld} \colorbox{red!1}{\strut income} \colorbox{red!0}{\strut .} \colorbox{red!0}{\strut At} \colorbox{red!0}{\strut the} \colorbox{red!0}{\strut end} \colorbox{red!0}{\strut of} \colorbox{red!0}{\strut the} \colorbox{red!0}{\strut year} \colorbox{red!0}{\strut ,} \colorbox{red!0}{\strut file} \colorbox{red!0}{\strut Form} \colorbox{red!0}{\strut 165} \colorbox{red!0}{\strut with} \colorbox{red!0}{\strut the} \colorbox{red!1}{\strut state} \colorbox{red!0}{\strut to} \colorbox{red!0}{\strut report} \colorbox{red!0}{\strut the} \colorbox{red!0}{\strut full} \colorbox{red!0}{\strut amount} \colorbox{red!0}{\strut withheld} \colorbox{red!0}{\strut ,} \colorbox{red!0}{\strut and} \colorbox{red!0}{\strut include} \colorbox{red!0}{\strut copies} \colorbox{red!0}{\strut of} \colorbox{red!0}{\strut the} \colorbox{red!0}{\strut W-2} \colorbox{red!0}{\strut forms} \colorbox{red!0}{\strut distributed} \colorbox{red!0}{\strut to} \colorbox{red!0}{\strut each} \colorbox{red!0}{\strut employee} \colorbox{red!0}{\strut and} \colorbox{red!0}{\strut IRS.Federal} \colorbox{red!0}{\strut TaxesMichigan} \colorbox{red!1}{\strut requires} \colorbox{red!1}{\strut businesses} \colorbox{red!0}{\strut to} \colorbox{red!0}{\strut complete} \colorbox{red!0}{\strut federal} \colorbox{red!2}{\strut tax} \colorbox{red!0}{\strut returns} \colorbox{red!0}{\strut before} \colorbox{red!1}{\strut state} \colorbox{red!0}{\strut returns} \colorbox{red!0}{\strut .} \colorbox{red!0}{\strut To} \colorbox{red!0}{\strut file} \colorbox{red!0}{\strut a} \colorbox{red!0}{\strut federal} 
}}}
\end{CJK*}

\begin{CJK*}{UTF8}{gbsn}
{\setlength{\fboxsep}{0pt}\colorbox{white!0}{\parbox{0.9\textwidth}{
\colorbox{red!0}{\strut 5} \colorbox{red!0}{\strut Steps} \colorbox{red!0}{\strut to} \colorbox{red!1}{\strut Filing} \colorbox{red!3}{\strut Partnership} \colorbox{red!6}{\strut Taxes} \colorbox{red!0}{\strut 5} \colorbox{red!0}{\strut Steps} \colorbox{red!0}{\strut to} \colorbox{red!1}{\strut Filing} \colorbox{red!3}{\strut Partnership} \colorbox{red!0}{\strut Taxesby} \colorbox{red!0}{\strut Jane} \colorbox{red!0}{\strut Haskins} \colorbox{red!0}{\strut ,} \colorbox{red!0}{\strut Esq} \colorbox{red!0}{\strut .} \colorbox{red!0}{\strut Freelance} \colorbox{red!0}{\strut writerPartnerships} \colorbox{red!0}{\strut don} \colorbox{red!0}{\strut .} \colorbox{red!0}{\strut t} \colorbox{red!1}{\strut pay} \colorbox{red!1}{\strut federal} \colorbox{red!1}{\strut income} \colorbox{red!6}{\strut tax} \colorbox{red!0}{\strut .} \colorbox{red!0}{\strut Instead} \colorbox{red!0}{\strut ,} \colorbox{red!0}{\strut the} \colorbox{red!3}{\strut partnership} \colorbox{red!0}{\strut .} \colorbox{red!0}{\strut s} \colorbox{red!1}{\strut income} \colorbox{red!0}{\strut ,} \colorbox{red!1}{\strut losses} \colorbox{red!0}{\strut ,} \colorbox{red!1}{\strut deductions} \colorbox{red!0}{\strut and} \colorbox{red!1}{\strut credits} \colorbox{red!0}{\strut pass} \colorbox{red!0}{\strut through} \colorbox{red!0}{\strut to} \colorbox{red!0}{\strut the} \colorbox{red!1}{\strut partners} \colorbox{red!0}{\strut themselves} \colorbox{red!0}{\strut ,} \colorbox{red!1}{\strut who} \colorbox{red!0}{\strut report} \colorbox{red!0}{\strut these} \colorbox{red!0}{\strut amountsand} \colorbox{red!1}{\strut pay} \colorbox{red!6}{\strut taxes} \colorbox{red!0}{\strut on} \colorbox{red!0}{\strut themas} \colorbox{red!0}{\strut part} \colorbox{red!0}{\strut of} \colorbox{red!0}{\strut their} \colorbox{red!0}{\strut personal} \colorbox{red!1}{\strut income} \colorbox{red!6}{\strut tax} \colorbox{red!0}{\strut returns.Even} \colorbox{red!0}{\strut though} \colorbox{red!5}{\strut partnerships} \colorbox{red!0}{\strut aren} \colorbox{red!0}{\strut .} \colorbox{red!0}{\strut t} \colorbox{red!6}{\strut taxed} \colorbox{red!0}{\strut ,} \colorbox{red!0}{\strut they} \colorbox{red!0}{\strut must} \colorbox{red!1}{\strut file} \colorbox{red!0}{\strut a} \colorbox{red!6}{\strut tax} \colorbox{red!2}{\strut return} \colorbox{red!0}{\strut each} \colorbox{red!0}{\strut year} \colorbox{red!0}{\strut unless} \colorbox{red!0}{\strut the} \colorbox{red!3}{\strut partnership} \colorbox{red!0}{\strut has} \colorbox{red!0}{\strut no} \colorbox{red!1}{\strut income} \colorbox{red!0}{\strut or} \colorbox{red!1}{\strut expenses} \colorbox{red!0}{\strut .} \colorbox{red!0}{\strut The} \colorbox{red!2}{\strut return} \colorbox{red!0}{\strut will} \colorbox{red!0}{\strut show} \colorbox{red!0}{\strut the} \colorbox{red!3}{\strut partnership} \colorbox{red!0}{\strut .} \colorbox{red!0}{\strut s} \colorbox{red!0}{\strut total} \colorbox{red!1}{\strut income} \colorbox{red!0}{\strut ,} \colorbox{red!1}{\strut deductions} \colorbox{red!0}{\strut and} \colorbox{red!1}{\strut credits} \colorbox{red!0}{\strut .} \colorbox{red!5}{\strut Partnerships} \colorbox{red!0}{\strut also} \colorbox{red!0}{\strut must} \colorbox{red!1}{\strut prepare} \colorbox{red!1}{\strut schedules} \colorbox{red!0}{\strut showing} \colorbox{red!0}{\strut each} \colorbox{red!1}{\strut partner} \colorbox{red!0}{\strut .} \colorbox{red!0}{\strut s} \colorbox{red!0}{\strut share} \colorbox{red!0}{\strut of} \colorbox{red!0}{\strut the} \colorbox{red!1}{\strut business} \colorbox{red!1}{\strut income} \colorbox{red!0}{\strut or} \colorbox{red!1}{\strut loss} \colorbox{red!0}{\strut .} \colorbox{red!0}{\strut They} \colorbox{red!0}{\strut may} \colorbox{red!0}{\strut also} \colorbox{red!0}{\strut have} \colorbox{red!0}{\strut to} \colorbox{red!1}{\strut file} \colorbox{red!1}{\strut state} \colorbox{red!6}{\strut tax} \colorbox{red!2}{\strut returns} \colorbox{red!0}{\strut and} \colorbox{red!1}{\strut pay} \colorbox{red!0}{\strut certain} \colorbox{red!1}{\strut state} \colorbox{red!0}{\strut taxes.Whether} \colorbox{red!0}{\strut you} \colorbox{red!0}{\strut operate} \colorbox{red!0}{\strut as} \colorbox{red!0}{\strut a} \colorbox{red!1}{\strut general} \colorbox{red!3}{\strut partnership} \colorbox{red!0}{\strut or} \colorbox{red!0}{\strut a} \colorbox{red!1}{\strut limited} \colorbox{red!3}{\strut partnership} \colorbox{red!0}{\strut ,} \colorbox{red!0}{\strut you} \colorbox{red!0}{\strut .} \colorbox{red!0}{\strut ll} \colorbox{red!0}{\strut follow} \colorbox{red!0}{\strut the} \colorbox{red!0}{\strut same} \colorbox{red!0}{\strut basic} \colorbox{red!0}{\strut procedure} \colorbox{red!0}{\strut for} \colorbox{red!1}{\strut filing} \colorbox{red!1}{\strut business} \colorbox{red!6}{\strut taxes} \colorbox{red!0}{\strut .} \colorbox{red!0}{\strut However} \colorbox{red!0}{\strut ,} \colorbox{red!1}{\strut limited} \colorbox{red!1}{\strut partners} \colorbox{red!0}{\strut are} \colorbox{red!0}{\strut subject} \colorbox{red!0}{\strut to} \colorbox{red!0}{\strut slightly} \colorbox{red!0}{\strut different} \colorbox{red!6}{\strut tax} \colorbox{red!0}{\strut treatment} \colorbox{red!0}{\strut than} \colorbox{red!1}{\strut general} \colorbox{red!0}{\strut partners.Here} \colorbox{red!0}{\strut are} \colorbox{red!0}{\strut the} \colorbox{red!0}{\strut five} \colorbox{red!0}{\strut steps} \colorbox{red!0}{\strut you} \colorbox{red!0}{\strut .} \colorbox{red!0}{\strut ll} \colorbox{red!0}{\strut need} \colorbox{red!0}{\strut to} \colorbox{red!0}{\strut follow} \colorbox{red!0}{\strut to} \colorbox{red!1}{\strut file} \colorbox{red!1}{\strut business} \colorbox{red!6}{\strut taxes} \colorbox{red!0}{\strut for} \colorbox{red!0}{\strut your} \colorbox{red!0}{\strut partnership.1} \colorbox{red!0}{\strut .} \colorbox{red!1}{\strut Prepare} \colorbox{red!1}{\strut Form} \colorbox{red!0}{\strut 1065} \colorbox{red!0}{\strut ,} \colorbox{red!0}{\strut U.S.} \colorbox{red!2}{\strut Return} \colorbox{red!0}{\strut of} \colorbox{red!3}{\strut Partnership} \colorbox{red!0}{\strut IncomeEvery} \colorbox{red!3}{\strut partnership} \colorbox{red!0}{\strut must} \colorbox{red!1}{\strut prepare} \colorbox{red!0}{\strut a} \colorbox{red!1}{\strut federal} \colorbox{red!3}{\strut partnership} \colorbox{red!6}{\strut tax} \colorbox{red!2}{\strut return} \colorbox{red!0}{\strut on} \colorbox{red!0}{\strut Internal} \colorbox{red!0}{\strut Revenue} \colorbox{red!0}{\strut Servicer} \colorbox{red!1}{\strut Form} \colorbox{red!0}{\strut 1065} \colorbox{red!0}{\strut .} \colorbox{red!0}{\strut On} \colorbox{red!0}{\strut this} \colorbox{red!1}{\strut form} \colorbox{red!0}{\strut ,} \colorbox{red!0}{\strut you} \colorbox{red!0}{\strut .} \colorbox{red!0}{\strut ll} \colorbox{red!0}{\strut be} \colorbox{red!0}{\strut asked} \colorbox{red!0}{\strut to} \colorbox{red!0}{\strut provide} \colorbox{red!0}{\strut the} \colorbox{red!3}{\strut partnership} \colorbox{red!0}{\strut .} \colorbox{red!0}{\strut s} \colorbox{red!0}{\strut total} \colorbox{red!1}{\strut income} \colorbox{red!0}{\strut or} \colorbox{red!1}{\strut loss} \colorbox{red!0}{\strut .} \colorbox{red!0}{\strut You} \colorbox{red!0}{\strut will} \colorbox{red!0}{\strut list} \colorbox{red!1}{\strut deductions} \colorbox{red!0}{\strut such} \colorbox{red!0}{\strut as} \colorbox{red!1}{\strut salaries} \colorbox{red!0}{\strut ,} \colorbox{red!0}{\strut guaranteed} \colorbox{red!0}{\strut payments} \colorbox{red!0}{\strut to} \colorbox{red!1}{\strut partners} \colorbox{red!0}{\strut ,} \colorbox{red!0}{\strut rent} \colorbox{red!0}{\strut ,} \colorbox{red!0}{\strut repairs} \colorbox{red!0}{\strut ,} \colorbox{red!6}{\strut taxes} \colorbox{red!0}{\strut ,} \colorbox{red!0}{\strut depreciation} \colorbox{red!0}{\strut and} \colorbox{red!0}{\strut employee} \colorbox{red!1}{\strut benefit} \colorbox{red!0}{\strut programs} \colorbox{red!0}{\strut .} \colorbox{red!0}{\strut Your} \colorbox{red!3}{\strut partnership} \colorbox{red!0}{\strut .} \colorbox{red!0}{\strut s} \colorbox{red!0}{\strut total} \colorbox{red!1}{\strut income} \colorbox{red!0}{\strut ,} \colorbox{red!0}{\strut less} \colorbox{red!0}{\strut its} \colorbox{red!1}{\strut deductions} \colorbox{red!0}{\strut ,} \colorbox{red!0}{\strut is} \colorbox{red!0}{\strut its} \colorbox{red!0}{\strut ordinary} \colorbox{red!1}{\strut business} \colorbox{red!0}{\strut income.You} \colorbox{red!0}{\strut .} \colorbox{red!0}{\strut ll} \colorbox{red!0}{\strut also} \colorbox{red!0}{\strut need} \colorbox{red!0}{\strut to} \colorbox{red!0}{\strut fill} \colorbox{red!0}{\strut out} \colorbox{red!0}{\strut several} \colorbox{red!1}{\strut Form} \colorbox{red!0}{\strut 1065} \colorbox{red!1}{\strut schedules} \colorbox{red!0}{\strut .} \colorbox{red!1}{\strut Schedule} \colorbox{red!0}{\strut B} \colorbox{red!0}{\strut includes} \colorbox{red!0}{\strut a} \colorbox{red!0}{\strut series} \colorbox{red!0}{\strut of} \colorbox{red!0}{\strut questions} \colorbox{red!0}{\strut about} \colorbox{red!0}{\strut your} \colorbox{red!0}{\strut partnershipfrom} \colorbox{red!0}{\strut the} \colorbox{red!0}{\strut types} \colorbox{red!0}{\strut of} \colorbox{red!1}{\strut partners} 
}}}
\end{CJK*}

query: against what part of the electromagnetic spectrum does sunscreen protect?

\begin{CJK*}{UTF8}{gbsn}
{\setlength{\fboxsep}{0pt}\colorbox{white!0}{\parbox{0.9\textwidth}{
\colorbox{red!8}{\strut Critical} \colorbox{red!8}{\strut Wavelength} \colorbox{red!0}{\strut .} \colorbox{red!0}{\strut Broad} \colorbox{red!1}{\strut Spectrum} \colorbox{red!1}{\strut UV} \colorbox{red!1}{\strut Protection} \colorbox{red!8}{\strut Critical} \colorbox{red!8}{\strut Wavelength} \colorbox{red!0}{\strut .} \colorbox{red!0}{\strut Broad} \colorbox{red!1}{\strut Spectrum} \colorbox{red!1}{\strut UV} \colorbox{red!1}{\strut Protection} \colorbox{red!0}{\strut .} \colorbox{red!0}{\strut .} \colorbox{red!0}{\strut one} \colorbox{red!0}{\strut of} \colorbox{red!0}{\strut the} \colorbox{red!0}{\strut best} \colorbox{red!0}{\strut informational} \colorbox{red!0}{\strut pages} \colorbox{red!0}{\strut on} \colorbox{red!3}{\strut sunscreens} \colorbox{red!0}{\strut and} \colorbox{red!8}{\strut critical} \colorbox{red!8}{\strut wavelength} \colorbox{red!0}{\strut I} \colorbox{red!0}{\strut have} \colorbox{red!0}{\strut seen} \colorbox{red!0}{\strut .} \colorbox{red!0}{\strut .} \colorbox{red!0}{\strut Karl} \colorbox{red!0}{\strut Gruber} \colorbox{red!0}{\strut MD} \colorbox{red!0}{\strut ,} \colorbox{red!0}{\strut Founder} \colorbox{red!0}{\strut of} \colorbox{red!0}{\strut LUCA} \colorbox{red!0}{\strut SunscreenWhat} \colorbox{red!0}{\strut Is} \colorbox{red!8}{\strut Critical} \colorbox{red!8}{\strut Wavelength} \colorbox{red!0}{\strut ?} \colorbox{red!0}{\strut .} \colorbox{red!5}{\strut What} \colorbox{red!0}{\strut is} \colorbox{red!8}{\strut critical} \colorbox{red!8}{\strut wavelength} \colorbox{red!0}{\strut and} \colorbox{red!0}{\strut why} \colorbox{red!0}{\strut is} \colorbox{red!0}{\strut it} \colorbox{red!0}{\strut so} \colorbox{red!0}{\strut important} \colorbox{red!0}{\strut ?} \colorbox{red!0}{\strut .} \colorbox{red!0}{\strut you} \colorbox{red!0}{\strut ask} \colorbox{red!0}{\strut .} \colorbox{red!8}{\strut Critical} \colorbox{red!8}{\strut wavelength} \colorbox{red!0}{\strut identifies} \colorbox{red!0}{\strut the} \colorbox{red!0}{\strut amount} \colorbox{red!0}{\strut of} \colorbox{red!0}{\strut UVA} \colorbox{red!1}{\strut protection} \colorbox{red!0}{\strut a} \colorbox{red!0}{\strut given} \colorbox{red!4}{\strut sunscreen} \colorbox{red!0}{\strut product} \colorbox{red!0}{\strut offers} \colorbox{red!0}{\strut ,} \colorbox{red!0}{\strut and} \colorbox{red!0}{\strut provides} \colorbox{red!0}{\strut a} \colorbox{red!0}{\strut way} \colorbox{red!0}{\strut to} \colorbox{red!0}{\strut define} \colorbox{red!0}{\strut true} \colorbox{red!0}{\strut .} \colorbox{red!0}{\strut broad} \colorbox{red!1}{\strut spectrum} \colorbox{red!0}{\strut .} \colorbox{red!1}{\strut protection} \colorbox{red!0}{\strut .} \colorbox{red!8}{\strut Critical} \colorbox{red!8}{\strut wavelength} \colorbox{red!1}{\strut measurements} \colorbox{red!0}{\strut are} \colorbox{red!0}{\strut therefore} \colorbox{red!0}{\strut extremely} \colorbox{red!0}{\strut beneficial} \colorbox{red!0}{\strut to} \colorbox{red!0}{\strut the} \colorbox{red!0}{\strut consumer} \colorbox{red!0}{\strut seeking} \colorbox{red!4}{\strut sunscreen} \colorbox{red!0}{\strut products} \colorbox{red!0}{\strut that} \colorbox{red!0}{\strut provide} \colorbox{red!0}{\strut maximum} \colorbox{red!1}{\strut protection} \colorbox{red!0}{\strut from} \colorbox{red!0}{\strut the} \colorbox{red!1}{\strut sun} \colorbox{red!0}{\strut .} \colorbox{red!0}{\strut s} \colorbox{red!0}{\strut harmful} \colorbox{red!0}{\strut rays} \colorbox{red!0}{\strut .} \colorbox{red!0}{\strut Here} \colorbox{red!0}{\strut .} \colorbox{red!0}{\strut s} \colorbox{red!0}{\strut how} \colorbox{red!0}{\strut it} \colorbox{red!0}{\strut all} \colorbox{red!0}{\strut worksMeasuring} \colorbox{red!1}{\strut UV} \colorbox{red!1}{\strut Absorbance} \colorbox{red!0}{\strut The} \colorbox{red!1}{\strut UV} \colorbox{red!1}{\strut absorbance} \colorbox{red!0}{\strut of} \colorbox{red!0}{\strut a} \colorbox{red!4}{\strut sunscreen} \colorbox{red!0}{\strut product} \colorbox{red!0}{\strut can} \colorbox{red!0}{\strut be} \colorbox{red!0}{\strut determined} \colorbox{red!0}{\strut in} \colorbox{red!0}{\strut vitro} \colorbox{red!0}{\strut over} \colorbox{red!0}{\strut the} \colorbox{red!0}{\strut entire} \colorbox{red!1}{\strut UV} \colorbox{red!1}{\strut spectrum} \colorbox{red!0}{\strut .} \colorbox{red!0}{\strut 290nm} \colorbox{red!0}{\strut .} \colorbox{red!0}{\strut 400nm} \colorbox{red!0}{\strut .} \colorbox{red!0}{\strut using} \colorbox{red!0}{\strut substrate} \colorbox{red!0}{\strut spectrophotometry} \colorbox{red!0}{\strut .} \colorbox{red!0}{\strut A} \colorbox{red!0}{\strut uniform} \colorbox{red!0}{\strut amount} \colorbox{red!0}{\strut and} \colorbox{red!0}{\strut thickness} \colorbox{red!0}{\strut of} \colorbox{red!4}{\strut sunscreen} \colorbox{red!0}{\strut is} \colorbox{red!0}{\strut applied} \colorbox{red!0}{\strut to} \colorbox{red!0}{\strut a} \colorbox{red!0}{\strut slide} \colorbox{red!0}{\strut and} \colorbox{red!0}{\strut exposed} \colorbox{red!0}{\strut to} \colorbox{red!1}{\strut UV} \colorbox{red!0}{\strut light} \colorbox{red!0}{\strut .} \colorbox{red!0}{\strut the} \colorbox{red!1}{\strut absorbance} \colorbox{red!0}{\strut of} \colorbox{red!0}{\strut that} \colorbox{red!1}{\strut UV} \colorbox{red!0}{\strut radiation} \colorbox{red!0}{\strut is} \colorbox{red!1}{\strut measured} \colorbox{red!0}{\strut .} \colorbox{red!0}{\strut The} \colorbox{red!0}{\strut graph} \colorbox{red!0}{\strut below} \colorbox{red!0}{\strut is} \colorbox{red!0}{\strut an} \colorbox{red!0}{\strut example} \colorbox{red!0}{\strut that} \colorbox{red!0}{\strut approximates} \colorbox{red!0}{\strut the} \colorbox{red!1}{\strut absorbance} \colorbox{red!0}{\strut curves} \colorbox{red!0}{\strut of} \colorbox{red!0}{\strut a} \colorbox{red!0}{\strut UVB} \colorbox{red!4}{\strut sunscreen} \colorbox{red!0}{\strut .} \colorbox{red!0}{\strut 2-EHMC} \colorbox{red!0}{\strut ,} \colorbox{red!0}{\strut 5} \colorbox{red!0}{\strut .} \colorbox{red!0}{\strut .} \colorbox{red!0}{\strut ,} \colorbox{red!0}{\strut a} \colorbox{red!0}{\strut UVA} \colorbox{red!4}{\strut sunscreen} \colorbox{red!0}{\strut .} \colorbox{red!0}{\strut TDSA} \colorbox{red!0}{\strut ,} \colorbox{red!0}{\strut 5} \colorbox{red!0}{\strut .} \colorbox{red!0}{\strut .} \colorbox{red!0}{\strut ,} \colorbox{red!0}{\strut and} \colorbox{red!0}{\strut a} \colorbox{red!0}{\strut broad} \colorbox{red!1}{\strut spectrum} \colorbox{red!4}{\strut sunscreen} \colorbox{red!0}{\strut such} \colorbox{red!0}{\strut as} \colorbox{red!0}{\strut Zinc} \colorbox{red!0}{\strut Oxide} \colorbox{red!0}{\strut .} \colorbox{red!0}{\strut 20} \colorbox{red!0}{\strut .} \colorbox{red!0}{\strut .} \colorbox{red!0}{\strut .The} \colorbox{red!0}{\strut shape} \colorbox{red!0}{\strut of} \colorbox{red!0}{\strut the} \colorbox{red!0}{\strut resultant} \colorbox{red!1}{\strut absorbance} \colorbox{red!0}{\strut curve} \colorbox{red!0}{\strut represents} \colorbox{red!0}{\strut the} \colorbox{red!0}{\strut efficiency} \colorbox{red!0}{\strut at} \colorbox{red!0}{\strut which} \colorbox{red!0}{\strut a} \colorbox{red!4}{\strut sunscreen} \colorbox{red!0}{\strut product} \colorbox{red!0}{\strut blocks} \colorbox{red!0}{\strut a} \colorbox{red!0}{\strut given} \colorbox{red!1}{\strut UV} \colorbox{red!8}{\strut wavelength} \colorbox{red!0}{\strut with} \colorbox{red!0}{\strut respect} \colorbox{red!0}{\strut to} \colorbox{red!0}{\strut another} \colorbox{red!0}{\strut .} \colorbox{red!0}{\strut This} \colorbox{red!1}{\strut UV} \colorbox{red!1}{\strut absorbance} \colorbox{red!0}{\strut curve} \colorbox{red!0}{\strut demonstrates} \colorbox{red!0}{\strut the} \colorbox{red!0}{\strut amplitude} \colorbox{red!0}{\strut and} \colorbox{red!0}{\strut breadth} \colorbox{red!0}{\strut of} \colorbox{red!1}{\strut protection} \colorbox{red!0}{\strut provided} \colorbox{red!0}{\strut .} \colorbox{red!0}{\strut from} \colorbox{red!0}{\strut 290nm} \colorbox{red!0}{\strut .} \colorbox{red!0}{\strut 400nm} \colorbox{red!0}{\strut .} \colorbox{red!0}{\strut across} \colorbox{red!0}{\strut the} \colorbox{red!1}{\strut UV} \colorbox{red!0}{\strut spectrum.Interpreting} \colorbox{red!0}{\strut the} \colorbox{red!1}{\strut Absorbance} \colorbox{red!0}{\strut Curve} \colorbox{red!0}{\strut The} \colorbox{red!0}{\strut .} \colorbox{red!0}{\strut amplitude} \colorbox{red!0}{\strut .} \colorbox{red!0}{\strut of} \colorbox{red!0}{\strut the} \colorbox{red!1}{\strut absorbance} \colorbox{red!0}{\strut curve} \colorbox{red!0}{\strut reflects} \colorbox{red!0}{\strut the} \colorbox{red!0}{\strut degree} \colorbox{red!0}{\strut of} \colorbox{red!1}{\strut protection} \colorbox{red!0}{\strut .} \colorbox{red!0}{\strut The} \colorbox{red!0}{\strut higher} \colorbox{red!0}{\strut the} \colorbox{red!0}{\strut amplitude} \colorbox{red!0}{\strut of} \colorbox{red!0}{\strut the} \colorbox{red!0}{\strut curve} \colorbox{red!0}{\strut ,} \colorbox{red!0}{\strut the} \colorbox{red!0}{\strut greater} \colorbox{red!0}{\strut the} \colorbox{red!1}{\strut absorbance} \colorbox{red!0}{\strut ,} \colorbox{red!0}{\strut and} \colorbox{red!0}{\strut the} \colorbox{red!0}{\strut more} \colorbox{red!1}{\strut protection} 
}}}
\end{CJK*}

\begin{CJK*}{UTF8}{gbsn}
{\setlength{\fboxsep}{0pt}\colorbox{white!0}{\parbox{0.9\textwidth}{
\colorbox{red!3}{\strut What} \colorbox{red!0}{\strut are} \colorbox{red!0}{\strut the} \colorbox{red!4}{\strut parts} \colorbox{red!0}{\strut of} \colorbox{red!0}{\strut the} \colorbox{red!4}{\strut electromagnetic} \colorbox{red!4}{\strut spectrum} \colorbox{red!0}{\strut ?} \colorbox{red!3}{\strut What} \colorbox{red!0}{\strut are} \colorbox{red!0}{\strut the} \colorbox{red!4}{\strut parts} \colorbox{red!0}{\strut of} \colorbox{red!0}{\strut the} \colorbox{red!4}{\strut electromagnetic} \colorbox{red!4}{\strut spectrum} \colorbox{red!0}{\strut ?} \colorbox{red!0}{\strut radio} \colorbox{red!0}{\strut wavesAshley} \colorbox{red!0}{\strut Holden} \colorbox{red!0}{\strut 9} \colorbox{red!0}{\strut ContributionsWhat} \colorbox{red!0}{\strut are} \colorbox{red!0}{\strut all} \colorbox{red!0}{\strut the} \colorbox{red!4}{\strut parts} \colorbox{red!0}{\strut of} \colorbox{red!0}{\strut the} \colorbox{red!4}{\strut electromagnetic} \colorbox{red!4}{\strut spectrum} \colorbox{red!0}{\strut ?} \colorbox{red!0}{\strut Radio} \colorbox{red!0}{\strut -} \colorbox{red!0}{\strut Microwave} \colorbox{red!0}{\strut -} \colorbox{red!0}{\strut Infrared} \colorbox{red!0}{\strut -} \colorbox{red!0}{\strut Visible} \colorbox{red!0}{\strut .} \colorbox{red!0}{\strut colours} \colorbox{red!0}{\strut .} \colorbox{red!0}{\strut -} \colorbox{red!0}{\strut Ultraviolet} \colorbox{red!0}{\strut -} \colorbox{red!0}{\strut X-ray} \colorbox{red!0}{\strut -} \colorbox{red!0}{\strut Gamma} \colorbox{red!0}{\strut The} \colorbox{red!0}{\strut best} \colorbox{red!0}{\strut way} \colorbox{red!0}{\strut to} \colorbox{red!0}{\strut remember} \colorbox{red!0}{\strut it} \colorbox{red!0}{\strut is} \colorbox{red!0}{\strut .} \colorbox{red!0}{\strut Rabbits} \colorbox{red!0}{\strut Mate} \colorbox{red!0}{\strut In} \colorbox{red!0}{\strut Very} \colorbox{red!0}{\strut Unusual} \colorbox{red!0}{\strut eXpens} \colorbox{red!0}{\strut What} \colorbox{red!0}{\strut are} \colorbox{red!0}{\strut the} \colorbox{red!4}{\strut parts} \colorbox{red!0}{\strut of} \colorbox{red!0}{\strut an} \colorbox{red!4}{\strut electromagnetic} \colorbox{red!4}{\strut spectrum} \colorbox{red!0}{\strut ?} \colorbox{red!0}{\strut The} \colorbox{red!4}{\strut electromagnetic} \colorbox{red!4}{\strut spectrum} \colorbox{red!0}{\strut consists} \colorbox{red!0}{\strut of} \colorbox{red!0}{\strut non-visible} \colorbox{red!0}{\strut radiation} \colorbox{red!0}{\strut ,} \colorbox{red!0}{\strut visible} \colorbox{red!0}{\strut light} \colorbox{red!0}{\strut ,} \colorbox{red!0}{\strut and} \colorbox{red!0}{\strut radio} \colorbox{red!0}{\strut waves} \colorbox{red!0}{\strut .} \colorbox{red!0}{\strut Some} \colorbox{red!0}{\strut examples} \colorbox{red!0}{\strut include} \colorbox{red!0}{\strut Gamma} \colorbox{red!0}{\strut rays} \colorbox{red!0}{\strut ,} \colorbox{red!0}{\strut x-rays} \colorbox{red!0}{\strut ,} \colorbox{red!0}{\strut ultraviolet} \colorbox{red!0}{\strut ,} \colorbox{red!0}{\strut UHF} \colorbox{red!0}{\strut and} \colorbox{red!0}{\strut VHF} \colorbox{red!0}{\strut bandwidt} \colorbox{red!0}{\strut John} \colorbox{red!0}{\strut Ellis} \colorbox{red!0}{\strut Hartford} \colorbox{red!0}{\strut 21,476} \colorbox{red!0}{\strut ContributionsWhat} \colorbox{red!0}{\strut is} \colorbox{red!4}{\strut part} \colorbox{red!0}{\strut of} \colorbox{red!0}{\strut the} \colorbox{red!4}{\strut electromagnetic} \colorbox{red!4}{\strut spectrum} \colorbox{red!0}{\strut ?} \colorbox{red!0}{\strut One} \colorbox{red!0}{\strut example} \colorbox{red!0}{\strut is} \colorbox{red!0}{\strut the} \colorbox{red!0}{\strut visible} \colorbox{red!4}{\strut spectrum} \colorbox{red!0}{\strut .} \colorbox{red!0}{\strut all} \colorbox{red!0}{\strut the} \colorbox{red!0}{\strut colors} \colorbox{red!0}{\strut that} \colorbox{red!0}{\strut you} \colorbox{red!0}{\strut can} \colorbox{red!0}{\strut see.Jack177} \colorbox{red!0}{\strut 784} \colorbox{red!0}{\strut ContributionsThe} \colorbox{red!4}{\strut part} \colorbox{red!0}{\strut of} \colorbox{red!0}{\strut the} \colorbox{red!4}{\strut electromagnetic} \colorbox{red!4}{\strut spectrum} \colorbox{red!0}{\strut that} \colorbox{red!0}{\strut you} \colorbox{red!0}{\strut can} \colorbox{red!0}{\strut see} \colorbox{red!0}{\strut ?} \colorbox{red!0}{\strut visible} \colorbox{red!0}{\strut light} \colorbox{red!0}{\strut 790-400} \colorbox{red!0}{\strut nmCommon} \colorbox{red!0}{\strut properties} \colorbox{red!0}{\strut for} \colorbox{red!0}{\strut the} \colorbox{red!4}{\strut electromagnetic} \colorbox{red!4}{\strut spectrum} \colorbox{red!0}{\strut ?} \colorbox{red!0}{\strut G} \colorbox{red!0}{\strut x} \colorbox{red!0}{\strut u} \colorbox{red!0}{\strut v} \colorbox{red!0}{\strut i} \colorbox{red!0}{\strut m} \colorbox{red!0}{\strut rPetethemeerkat} \colorbox{red!0}{\strut 1,289} \colorbox{red!0}{\strut ContributionsList} \colorbox{red!0}{\strut the} \colorbox{red!4}{\strut parts} \colorbox{red!0}{\strut of} \colorbox{red!0}{\strut the} \colorbox{red!4}{\strut electromagnetic} \colorbox{red!4}{\strut spectrum} \colorbox{red!0}{\strut ?} \colorbox{red!0}{\strut Radio} \colorbox{red!0}{\strut waves} \colorbox{red!0}{\strut Microwaves} \colorbox{red!0}{\strut Infrared} \colorbox{red!0}{\strut Visible} \colorbox{red!0}{\strut light} \colorbox{red!0}{\strut Ultraviolet} \colorbox{red!0}{\strut X} \colorbox{red!0}{\strut rays} \colorbox{red!0}{\strut Gamma} \colorbox{red!0}{\strut raysJohn} \colorbox{red!0}{\strut Ellis} \colorbox{red!0}{\strut Hartford} \colorbox{red!0}{\strut 21,476} \colorbox{red!0}{\strut ContributionsWhat} \colorbox{red!4}{\strut part} \colorbox{red!0}{\strut of} \colorbox{red!0}{\strut the} \colorbox{red!4}{\strut electromagnetic} \colorbox{red!4}{\strut spectrum} \colorbox{red!0}{\strut is} \colorbox{red!0}{\strut color} \colorbox{red!0}{\strut ?} \colorbox{red!0}{\strut The} \colorbox{red!0}{\strut so} \colorbox{red!0}{\strut called} \colorbox{red!0}{\strut visible} \colorbox{red!4}{\strut spectrum} \colorbox{red!0}{\strut .} \colorbox{red!0}{\strut .} \colorbox{red!0}{\strut from} \colorbox{red!0}{\strut red} \colorbox{red!0}{\strut .} \colorbox{red!0}{\strut low} \colorbox{red!0}{\strut frequency} \colorbox{red!0}{\strut .} \colorbox{red!0}{\strut to} \colorbox{red!0}{\strut violet} \colorbox{red!0}{\strut .} \colorbox{red!0}{\strut high} \colorbox{red!0}{\strut frequency} \colorbox{red!0}{\strut .} \colorbox{red!0}{\strut .Identify} \colorbox{red!0}{\strut the} \colorbox{red!4}{\strut parts} \colorbox{red!0}{\strut of} \colorbox{red!0}{\strut the} \colorbox{red!4}{\strut electromagnetic} \colorbox{red!4}{\strut spectrum} \colorbox{red!0}{\strut ?} \colorbox{red!0}{\strut go} \colorbox{red!0}{\strut to} \colorbox{red!0}{\strut school} \colorbox{red!0}{\strut and} \colorbox{red!0}{\strut find} \colorbox{red!0}{\strut outWhy} \colorbox{red!0}{\strut is} \colorbox{red!0}{\strut sound} \colorbox{red!0}{\strut not} \colorbox{red!4}{\strut part} \colorbox{red!0}{\strut of} \colorbox{red!0}{\strut the} \colorbox{red!4}{\strut electromagnetic} \colorbox{red!4}{\strut spectrum} \colorbox{red!0}{\strut ?} \colorbox{red!0}{\strut Sound} \colorbox{red!0}{\strut needs} \colorbox{red!0}{\strut a} \colorbox{red!0}{\strut medium} \colorbox{red!0}{\strut to} \colorbox{red!0}{\strut travel} \colorbox{red!0}{\strut and} \colorbox{red!0}{\strut thus} \colorbox{red!0}{\strut is} \colorbox{red!0}{\strut not} \colorbox{red!0}{\strut a} \colorbox{red!4}{\strut part} \colorbox{red!0}{\strut of} \colorbox{red!0}{\strut the} \colorbox{red!4}{\strut electromagnetic} \colorbox{red!4}{\strut spectrum} \colorbox{red!0}{\strut .} \colorbox{red!0}{\strut Usually} \colorbox{red!0}{\strut if} \colorbox{red!0}{\strut it} \colorbox{red!0}{\strut can} \colorbox{red!0}{\strut travel} \colorbox{red!0}{\strut through} \colorbox{red!0}{\strut a} \colorbox{red!0}{\strut vacuum} \colorbox{red!0}{\strut its} \colorbox{red!0}{\strut a} \colorbox{red!4}{\strut part} \colorbox{red!0}{\strut of} \colorbox{red!0}{\strut the} \colorbox{red!4}{\strut electromagnetic} \colorbox{red!0}{\strut spectrum.Kevinkendall} \colorbox{red!0}{\strut 2} \colorbox{red!0}{\strut ContributionsWhat} \colorbox{red!0}{\strut is} \colorbox{red!0}{\strut the} \colorbox{red!4}{\strut part} \colorbox{red!0}{\strut of} \colorbox{red!0}{\strut the} \colorbox{red!4}{\strut electromagnetic} \colorbox{red!4}{\strut spectrum} \colorbox{red!0}{\strut that} \colorbox{red!0}{\strut you} \colorbox{red!0}{\strut can} \colorbox{red!0}{\strut hear} \colorbox{red!0}{\strut ?} \colorbox{red!4}{\strut Electromagnetic} \colorbox{red!4}{\strut spectrum} \colorbox{red!0}{\strut consists} \colorbox{red!0}{\strut of} \colorbox{red!0}{\strut radiations} \colorbox{red!0}{\strut of} \colorbox{red!0}{\strut different} \colorbox{red!0}{\strut wavelengths} \colorbox{red!0}{\strut and} \colorbox{red!0}{\strut frequency} \colorbox{red!0}{\strut which} \colorbox{red!0}{\strut are} \colorbox{red!0}{\strut visible} \colorbox{red!0}{\strut sometimes} \colorbox{red!0}{\strut and} \colorbox{red!0}{\strut most} \colorbox{red!0}{\strut of} \colorbox{red!0}{\strut them} \colorbox{red!0}{\strut are} \colorbox{red!0}{\strut invisible} \colorbox{red!0}{\strut .} \colorbox{red!0}{\strut They} \colorbox{red!0}{\strut all} \colorbox{red!0}{\strut are} \colorbox{red!0}{\strut forms} 
}}}
\end{CJK*}

query: what is a buddy test

\begin{CJK*}{UTF8}{gbsn}
{\setlength{\fboxsep}{0pt}\colorbox{white!0}{\parbox{0.9\textwidth}{
\colorbox{red!0}{\strut See} \colorbox{red!4}{\strut What} \colorbox{red!0}{\strut Our} \colorbox{red!9}{\strut ACT} \colorbox{red!8}{\strut Test} \colorbox{red!5}{\strut Watch} \colorbox{red!0}{\strut Customers} \colorbox{red!0}{\strut Are} \colorbox{red!0}{\strut Saying} \colorbox{red!9}{\strut ACT} \colorbox{red!8}{\strut Test} \colorbox{red!0}{\strut WatchOur} \colorbox{red!0}{\strut revolutionary} \colorbox{red!0}{\strut timing} \colorbox{red!0}{\strut device} \colorbox{red!0}{\strut gives} \colorbox{red!0}{\strut students} \colorbox{red!0}{\strut an} \colorbox{red!0}{\strut effective} \colorbox{red!0}{\strut way} \colorbox{red!0}{\strut to} \colorbox{red!0}{\strut manage} \colorbox{red!0}{\strut time} \colorbox{red!0}{\strut while} \colorbox{red!0}{\strut taking} \colorbox{red!0}{\strut the} \colorbox{red!0}{\strut ACT.Order} \colorbox{red!0}{\strut NowQuestion} \colorbox{red!0}{\strut TrackingNotifies} \colorbox{red!0}{\strut students} \colorbox{red!0}{\strut exactly} \colorbox{red!4}{\strut what} \colorbox{red!0}{\strut question} \colorbox{red!0}{\strut they} \colorbox{red!0}{\strut should} \colorbox{red!0}{\strut be} \colorbox{red!0}{\strut on} \colorbox{red!0}{\strut to} \colorbox{red!0}{\strut remain} \colorbox{red!0}{\strut on} \colorbox{red!0}{\strut track.View} \colorbox{red!0}{\strut NowPre-ProgrammedOur} \colorbox{red!9}{\strut ACT} \colorbox{red!8}{\strut Test} \colorbox{red!5}{\strut watch} \colorbox{red!0}{\strut comes} \colorbox{red!0}{\strut pre-programmed} \colorbox{red!0}{\strut for} \colorbox{red!0}{\strut all} \colorbox{red!0}{\strut 5} \colorbox{red!0}{\strut sections} \colorbox{red!0}{\strut of} \colorbox{red!0}{\strut the} \colorbox{red!0}{\strut ACT.View} \colorbox{red!0}{\strut NowSection} \colorbox{red!0}{\strut TrackingQuickly} \colorbox{red!0}{\strut know} \colorbox{red!1}{\strut how} \colorbox{red!0}{\strut much} \colorbox{red!0}{\strut time} \colorbox{red!0}{\strut has} \colorbox{red!0}{\strut elapsed} \colorbox{red!0}{\strut and} \colorbox{red!0}{\strut remains} \colorbox{red!0}{\strut in} \colorbox{red!0}{\strut each} \colorbox{red!0}{\strut section.View} \colorbox{red!0}{\strut NowApproved} \colorbox{red!8}{\strut Test} \colorbox{red!0}{\strut Watch100} \colorbox{red!0}{\strut percent} \colorbox{red!0}{\strut legal} \colorbox{red!9}{\strut ACT} \colorbox{red!0}{\strut pacing} \colorbox{red!5}{\strut watch} \colorbox{red!0}{\strut used} \colorbox{red!0}{\strut for} \colorbox{red!0}{\strut practice} \colorbox{red!0}{\strut and} \colorbox{red!0}{\strut during} \colorbox{red!0}{\strut the} \colorbox{red!0}{\strut real} \colorbox{red!0}{\strut ACT.View} \colorbox{red!0}{\strut NowThe} \colorbox{red!8}{\strut Test} \colorbox{red!0}{\strut Buddy} \colorbox{red!9}{\strut ACT} \colorbox{red!8}{\strut Test} \colorbox{red!0}{\strut WatchThe} \colorbox{red!8}{\strut Test} \colorbox{red!1}{\strut Buddy} \colorbox{red!0}{\strut .} \colorbox{red!0}{\strut for} \colorbox{red!9}{\strut ACT} \colorbox{red!0}{\strut .} \colorbox{red!0}{\strut gives} \colorbox{red!0}{\strut students} \colorbox{red!0}{\strut the} \colorbox{red!0}{\strut ability} \colorbox{red!0}{\strut to} \colorbox{red!0}{\strut precisely} \colorbox{red!0}{\strut manage} \colorbox{red!0}{\strut time} \colorbox{red!0}{\strut on} \colorbox{red!0}{\strut the} \colorbox{red!9}{\strut ACT} \colorbox{red!0}{\strut .} \colorbox{red!0}{\strut The} \colorbox{red!0}{\strut device} \colorbox{red!0}{\strut has} \colorbox{red!0}{\strut five} \colorbox{red!0}{\strut preset} \colorbox{red!0}{\strut timing} \colorbox{red!0}{\strut functions} \colorbox{red!0}{\strut ,} \colorbox{red!0}{\strut one} \colorbox{red!0}{\strut for} \colorbox{red!0}{\strut each} \colorbox{red!0}{\strut section} \colorbox{red!0}{\strut of} \colorbox{red!0}{\strut the} \colorbox{red!8}{\strut test} \colorbox{red!0}{\strut .} \colorbox{red!0}{\strut all} \colorbox{red!0}{\strut of} \colorbox{red!0}{\strut which} \colorbox{red!0}{\strut include} \colorbox{red!0}{\strut a} \colorbox{red!0}{\strut revolutionary} \colorbox{red!0}{\strut questionpassage} \colorbox{red!0}{\strut tracking} \colorbox{red!0}{\strut feature} \colorbox{red!0}{\strut which} \colorbox{red!0}{\strut allows} \colorbox{red!0}{\strut students} \colorbox{red!0}{\strut to} \colorbox{red!0}{\strut see} \colorbox{red!0}{\strut which} \colorbox{red!0}{\strut question} \colorbox{red!0}{\strut or} \colorbox{red!0}{\strut passage} \colorbox{red!0}{\strut they} \colorbox{red!0}{\strut should} \colorbox{red!0}{\strut have} \colorbox{red!0}{\strut completed} \colorbox{red!0}{\strut ,} \colorbox{red!0}{\strut given} \colorbox{red!1}{\strut how} \colorbox{red!0}{\strut much} \colorbox{red!0}{\strut time} \colorbox{red!0}{\strut has} \colorbox{red!0}{\strut passed.The} \colorbox{red!8}{\strut Test} \colorbox{red!1}{\strut Buddy} \colorbox{red!0}{\strut Video} \colorbox{red!0}{\strut Your} \colorbox{red!0}{\strut browser} \colorbox{red!0}{\strut does} \colorbox{red!0}{\strut not} \colorbox{red!0}{\strut currently} \colorbox{red!0}{\strut recognize} \colorbox{red!0}{\strut any} \colorbox{red!0}{\strut of} \colorbox{red!0}{\strut the} \colorbox{red!0}{\strut video} \colorbox{red!0}{\strut formats} \colorbox{red!0}{\strut available} \colorbox{red!0}{\strut .} \colorbox{red!0}{\strut Click} \colorbox{red!0}{\strut here} \colorbox{red!0}{\strut to} \colorbox{red!0}{\strut visit} \colorbox{red!0}{\strut our} \colorbox{red!0}{\strut frequently} \colorbox{red!0}{\strut asked} \colorbox{red!0}{\strut questions} \colorbox{red!0}{\strut about} \colorbox{red!0}{\strut HTML5} \colorbox{red!0}{\strut video.Top} \colorbox{red!0}{\strut TimerMeasures} \colorbox{red!1}{\strut how} \colorbox{red!0}{\strut much} \colorbox{red!0}{\strut time} \colorbox{red!0}{\strut has} \colorbox{red!0}{\strut passed} \colorbox{red!0}{\strut in} \colorbox{red!0}{\strut the} \colorbox{red!0}{\strut particular} \colorbox{red!0}{\strut section.Bottom} \colorbox{red!0}{\strut TimerDenotes} \colorbox{red!0}{\strut the} \colorbox{red!0}{\strut total} \colorbox{red!0}{\strut amount} \colorbox{red!0}{\strut of} \colorbox{red!0}{\strut time} \colorbox{red!0}{\strut in} \colorbox{red!0}{\strut the} \colorbox{red!0}{\strut specific} \colorbox{red!0}{\strut section} \colorbox{red!0}{\strut of} \colorbox{red!0}{\strut the} \colorbox{red!0}{\strut test.Fraction} \colorbox{red!0}{\strut TimerFraction} \colorbox{red!0}{\strut timer} \colorbox{red!0}{\strut at} \colorbox{red!0}{\strut the} \colorbox{red!0}{\strut very} \colorbox{red!0}{\strut bottom} \colorbox{red!0}{\strut of} \colorbox{red!0}{\strut the} \colorbox{red!0}{\strut screen} \colorbox{red!0}{\strut displays} \colorbox{red!4}{\strut what} \colorbox{red!0}{\strut question} \colorbox{red!0}{\strut you} \colorbox{red!0}{\strut re} \colorbox{red!0}{\strut on} \colorbox{red!0}{\strut in} \colorbox{red!0}{\strut regards} \colorbox{red!0}{\strut to} \colorbox{red!0}{\strut the} \colorbox{red!0}{\strut total} \colorbox{red!0}{\strut amount} \colorbox{red!0}{\strut of} \colorbox{red!0}{\strut questions} \colorbox{red!0}{\strut within} \colorbox{red!0}{\strut each} \colorbox{red!0}{\strut section.Exam} \colorbox{red!0}{\strut SectionsThe} \colorbox{red!0}{\strut very} \colorbox{red!0}{\strut top} \colorbox{red!0}{\strut displays} \colorbox{red!0}{\strut each} \colorbox{red!0}{\strut section} \colorbox{red!0}{\strut ,} \colorbox{red!0}{\strut for} \colorbox{red!0}{\strut example} \colorbox{red!0}{\strut .} \colorbox{red!0}{\strut E} \colorbox{red!0}{\strut .} \colorbox{red!0}{\strut English} \colorbox{red!0}{\strut ,} \colorbox{red!0}{\strut M} \colorbox{red!0}{\strut .} \colorbox{red!0}{\strut Math} \colorbox{red!0}{\strut ,} \colorbox{red!0}{\strut R} \colorbox{red!0}{\strut .} \colorbox{red!0}{\strut Reading} \colorbox{red!0}{\strut ,} \colorbox{red!0}{\strut S} \colorbox{red!0}{\strut .} \colorbox{red!0}{\strut Science} \colorbox{red!0}{\strut .} \colorbox{red!0}{\strut W} \colorbox{red!0}{\strut .} \colorbox{red!0}{\strut WritingStart} \colorbox{red!0}{\strut .} \colorbox{red!0}{\strut Stop} \colorbox{red!0}{\strut ButtonAllows} \colorbox{red!0}{\strut you} \colorbox{red!0}{\strut to} \colorbox{red!0}{\strut start} \colorbox{red!0}{\strut and} \colorbox{red!0}{\strut stop} \colorbox{red!0}{\strut the} \colorbox{red!0}{\strut timer} \colorbox{red!0}{\strut for} \colorbox{red!0}{\strut the} \colorbox{red!0}{\strut respective} \colorbox{red!0}{\strut section} \colorbox{red!0}{\strut of} \colorbox{red!0}{\strut the} \colorbox{red!0}{\strut test.Mode} \colorbox{red!0}{\strut ButtonUsed} \colorbox{red!0}{\strut to} \colorbox{red!0}{\strut toggle} \colorbox{red!0}{\strut through} \colorbox{red!0}{\strut the} \colorbox{red!0}{\strut five} \colorbox{red!0}{\strut sections} \colorbox{red!0}{\strut of} \colorbox{red!0}{\strut the} \colorbox{red!9}{\strut ACT} \colorbox{red!0}{\strut .} \colorbox{red!0}{\strut English} \colorbox{red!0}{\strut ,} \colorbox{red!0}{\strut Math} \colorbox{red!0}{\strut ,} \colorbox{red!0}{\strut Reading} \colorbox{red!0}{\strut ,} \colorbox{red!0}{\strut Science} \colorbox{red!0}{\strut .} \colorbox{red!0}{\strut Writing.ACT} \colorbox{red!5}{\strut Watch} \colorbox{red!0}{\strut SolutionThe} \colorbox{red!8}{\strut Test} \colorbox{red!1}{\strut Buddy} \colorbox{red!0}{\strut Has} \colorbox{red!0}{\strut Been} 
}}}
\end{CJK*}

\begin{CJK*}{UTF8}{gbsn}
{\setlength{\fboxsep}{0pt}\colorbox{white!0}{\parbox{0.9\textwidth}{
\colorbox{red!4}{\strut What} \colorbox{red!0}{\strut s} \colorbox{red!0}{\strut an} \colorbox{red!7}{\strut Anchor} \colorbox{red!7}{\strut Buddy} \colorbox{red!0}{\strut ?} \colorbox{red!0}{\strut .} \colorbox{red!4}{\strut What} \colorbox{red!0}{\strut s} \colorbox{red!0}{\strut an} \colorbox{red!7}{\strut Anchor} \colorbox{red!7}{\strut Buddy} \colorbox{red!0}{\strut ?} \colorbox{red!1}{\strut When} \colorbox{red!7}{\strut anchoring} \colorbox{red!0}{\strut on} \colorbox{red!0}{\strut the} \colorbox{red!1}{\strut Columbia} \colorbox{red!0}{\strut I} \colorbox{red!0}{\strut always} \colorbox{red!0}{\strut use} \colorbox{red!0}{\strut my} \colorbox{red!7}{\strut Anchor} \colorbox{red!7}{\strut Buddy} \colorbox{red!0}{\strut .} \colorbox{red!0}{\strut The} \colorbox{red!7}{\strut Anchor} \colorbox{red!7}{\strut Buddy} \colorbox{red!0}{\strut is} \colorbox{red!0}{\strut a} \colorbox{red!0}{\strut .} \colorbox{red!0}{\strut 25} \colorbox{red!0}{\strut thingy} \colorbox{red!0}{\strut invented} \colorbox{red!0}{\strut in} \colorbox{red!0}{\strut Oregon} \colorbox{red!0}{\strut .} \colorbox{red!0}{\strut by} \colorbox{red!0}{\strut the} \colorbox{red!0}{\strut way} \colorbox{red!0}{\strut .} \colorbox{red!0}{\strut that} \colorbox{red!0}{\strut works} \colorbox{red!0}{\strut like} \colorbox{red!0}{\strut a} \colorbox{red!0}{\strut giant} \colorbox{red!0}{\strut bungee} \colorbox{red!0}{\strut cord} \colorbox{red!0}{\strut to} \colorbox{red!0}{\strut keep} \colorbox{red!0}{\strut your} \colorbox{red!1}{\strut boat} \colorbox{red!0}{\strut out} \colorbox{red!0}{\strut in} \colorbox{red!1}{\strut deep} \colorbox{red!1}{\strut water} \colorbox{red!0}{\strut and} \colorbox{red!0}{\strut keep} \colorbox{red!0}{\strut it} \colorbox{red!0}{\strut from} \colorbox{red!0}{\strut being} \colorbox{red!0}{\strut beached} \colorbox{red!0}{\strut by} \colorbox{red!0}{\strut tides} \colorbox{red!0}{\strut ,} \colorbox{red!0}{\strut yacht} \colorbox{red!0}{\strut and} \colorbox{red!1}{\strut ship} \colorbox{red!0}{\strut wakes} \colorbox{red!0}{\strut and} \colorbox{red!0}{\strut the} \colorbox{red!0}{\strut wind} \colorbox{red!0}{\strut .} \colorbox{red!0}{\strut Here} \colorbox{red!0}{\strut is} \colorbox{red!0}{\strut a} \colorbox{red!0}{\strut little} \colorbox{red!0}{\strut tutorial} \colorbox{red!0}{\strut on} \colorbox{red!0}{\strut using} \colorbox{red!0}{\strut an} \colorbox{red!7}{\strut Anchor} \colorbox{red!0}{\strut buddy.I} \colorbox{red!0}{\strut start} \colorbox{red!0}{\strut with} \colorbox{red!0}{\strut a} \colorbox{red!0}{\strut Danforth} \colorbox{red!0}{\strut like} \colorbox{red!0}{\strut this} \colorbox{red!0}{\strut Fortress} \colorbox{red!0}{\strut and} \colorbox{red!0}{\strut then} \colorbox{red!0}{\strut shackle} \colorbox{red!0}{\strut it} \colorbox{red!0}{\strut to} \colorbox{red!0}{\strut at} \colorbox{red!0}{\strut least} \colorbox{red!0}{\strut 3} \colorbox{red!1}{\strut feet} \colorbox{red!0}{\strut of} \colorbox{red!1}{\strut chain} \colorbox{red!0}{\strut .} \colorbox{red!1}{\strut Connect} \colorbox{red!0}{\strut one} \colorbox{red!0}{\strut end} \colorbox{red!0}{\strut of} \colorbox{red!0}{\strut the} \colorbox{red!7}{\strut Anchor} \colorbox{red!7}{\strut Buddy} \colorbox{red!0}{\strut .} \colorbox{red!0}{\strut the} \colorbox{red!0}{\strut blue} \colorbox{red!1}{\strut ropes} \colorbox{red!0}{\strut .} \colorbox{red!0}{\strut to} \colorbox{red!0}{\strut your} \colorbox{red!7}{\strut anchor} \colorbox{red!1}{\strut chain} \colorbox{red!0}{\strut .} \colorbox{red!0}{\strut I} \colorbox{red!0}{\strut like} \colorbox{red!0}{\strut connecting} \colorbox{red!0}{\strut two} \colorbox{red!7}{\strut Anchor} \colorbox{red!7}{\strut Buddies} \colorbox{red!0}{\strut in} \colorbox{red!0}{\strut .} \colorbox{red!0}{\strut .} \colorbox{red!0}{\strut series} \colorbox{red!0}{\strut .} \colorbox{red!0}{\strut .} \colorbox{red!0}{\strut to} \colorbox{red!0}{\strut keep} \colorbox{red!0}{\strut my} \colorbox{red!1}{\strut boat} \colorbox{red!0}{\strut further} \colorbox{red!0}{\strut out} \colorbox{red!0}{\strut .} \colorbox{red!0}{\strut Now} \colorbox{red!1}{\strut attach} \colorbox{red!0}{\strut 150} \colorbox{red!0}{\strut to} \colorbox{red!0}{\strut 200} \colorbox{red!1}{\strut feet} \colorbox{red!0}{\strut of} \colorbox{red!0}{\strut 38} \colorbox{red!0}{\strut .} \colorbox{red!0}{\strut .} \colorbox{red!0}{\strut or} \colorbox{red!0}{\strut 516} \colorbox{red!0}{\strut .} \colorbox{red!0}{\strut .} \colorbox{red!0}{\strut nylon} \colorbox{red!1}{\strut rope} \colorbox{red!0}{\strut to} \colorbox{red!0}{\strut the} \colorbox{red!0}{\strut other} \colorbox{red!0}{\strut end} \colorbox{red!0}{\strut of} \colorbox{red!0}{\strut the} \colorbox{red!7}{\strut Anchor} \colorbox{red!7}{\strut Buddy} \colorbox{red!0}{\strut ,} \colorbox{red!0}{\strut and} \colorbox{red!0}{\strut finally} \colorbox{red!0}{\strut buy} \colorbox{red!0}{\strut a} \colorbox{red!0}{\strut helix} \colorbox{red!7}{\strut anchor} \colorbox{red!0}{\strut ,} \colorbox{red!0}{\strut or} \colorbox{red!0}{\strut some} \colorbox{red!0}{\strut other} \colorbox{red!0}{\strut form} \colorbox{red!0}{\strut of} \colorbox{red!0}{\strut ground} \colorbox{red!7}{\strut anchor} \colorbox{red!0}{\strut and} \colorbox{red!1}{\strut attach} \colorbox{red!0}{\strut that} \colorbox{red!0}{\strut to} \colorbox{red!0}{\strut the} \colorbox{red!0}{\strut end} \colorbox{red!0}{\strut of} \colorbox{red!0}{\strut the} \colorbox{red!0}{\strut rope.Now} \colorbox{red!0}{\strut ,} \colorbox{red!0}{\strut as} \colorbox{red!0}{\strut you} \colorbox{red!0}{\strut get} \colorbox{red!0}{\strut within} \colorbox{red!0}{\strut ,} \colorbox{red!0}{\strut say} \colorbox{red!0}{\strut 50-100} \colorbox{red!1}{\strut feet} \colorbox{red!0}{\strut from} \colorbox{red!0}{\strut shore} \colorbox{red!0}{\strut chuck} \colorbox{red!0}{\strut your} \colorbox{red!7}{\strut anchor} \colorbox{red!0}{\strut into} \colorbox{red!0}{\strut the} \colorbox{red!0}{\strut drink} \colorbox{red!0}{\strut .} \colorbox{red!0}{\strut Slowly} \colorbox{red!0}{\strut motor} \colorbox{red!0}{\strut to} \colorbox{red!0}{\strut shore} \colorbox{red!0}{\strut ,} \colorbox{red!0}{\strut being} \colorbox{red!0}{\strut sure} \colorbox{red!0}{\strut that} \colorbox{red!0}{\strut the} \colorbox{red!7}{\strut Anchor} \colorbox{red!7}{\strut Buddy} \colorbox{red!0}{\strut and} \colorbox{red!1}{\strut rope} \colorbox{red!0}{\strut do} \colorbox{red!0}{\strut nt} \colorbox{red!0}{\strut get} \colorbox{red!0}{\strut sucked} \colorbox{red!0}{\strut into} \colorbox{red!0}{\strut the} \colorbox{red!0}{\strut prop} \colorbox{red!0}{\strut .} \colorbox{red!1}{\strut When} \colorbox{red!0}{\strut you} \colorbox{red!0}{\strut get} \colorbox{red!0}{\strut to} \colorbox{red!0}{\strut shore} \colorbox{red!0}{\strut ,} \colorbox{red!0}{\strut toss} \colorbox{red!0}{\strut the} \colorbox{red!0}{\strut rest} \colorbox{red!0}{\strut of} \colorbox{red!0}{\strut the} \colorbox{red!1}{\strut rope} \colorbox{red!0}{\strut and} \colorbox{red!0}{\strut your} \colorbox{red!0}{\strut ground} \colorbox{red!7}{\strut anchor} \colorbox{red!0}{\strut on} \colorbox{red!0}{\strut the} \colorbox{red!0}{\strut beach.Now} \colorbox{red!0}{\strut ,} \colorbox{red!0}{\strut grab} \colorbox{red!0}{\strut the} \colorbox{red!1}{\strut rope} \colorbox{red!0}{\strut and} \colorbox{red!0}{\strut start} \colorbox{red!1}{\strut pulling} \colorbox{red!0}{\strut on} \colorbox{red!0}{\strut the} \colorbox{red!0}{\strut part} \colorbox{red!0}{\strut that} \colorbox{red!0}{\strut goes} \colorbox{red!0}{\strut out} \colorbox{red!0}{\strut to} \colorbox{red!0}{\strut the} \colorbox{red!7}{\strut anchor} \colorbox{red!0}{\strut ,} \colorbox{red!1}{\strut pull} \colorbox{red!0}{\strut it} \colorbox{red!0}{\strut in} \colorbox{red!0}{\strut as} \colorbox{red!0}{\strut tight} \colorbox{red!0}{\strut as} \colorbox{red!0}{\strut you} \colorbox{red!0}{\strut can} \colorbox{red!0}{\strut ,} \colorbox{red!0}{\strut then} \colorbox{red!1}{\strut attach} \colorbox{red!0}{\strut it} \colorbox{red!0}{\strut to} \colorbox{red!0}{\strut the} \colorbox{red!0}{\strut bow} \colorbox{red!0}{\strut cleat} \colorbox{red!0}{\strut with} \colorbox{red!0}{\strut several} \colorbox{red!0}{\strut half} \colorbox{red!0}{\strut hitches.It} \colorbox{red!0}{\strut should} \colorbox{red!0}{\strut now} \colorbox{red!0}{\strut look} \colorbox{red!0}{\strut like} \colorbox{red!0}{\strut this.Note} \colorbox{red!0}{\strut that} \colorbox{red!0}{\strut in} \colorbox{red!0}{\strut order} \colorbox{red!0}{\strut to} \colorbox{red!0}{\strut take} \colorbox{red!0}{\strut this} \colorbox{red!0}{\strut picture} \colorbox{red!0}{\strut I} \colorbox{red!0}{\strut had} \colorbox{red!0}{\strut to} \colorbox{red!0}{\strut have} \colorbox{red!0}{\strut my} \colorbox{red!0}{\strut foot} \colorbox{red!0}{\strut firmly} 
}}}
\end{CJK*}

query: is the louisiana sales tax 4.75

\begin{CJK*}{UTF8}{gbsn}
{\setlength{\fboxsep}{0pt}\colorbox{white!0}{\parbox{0.9\textwidth}{
\colorbox{red!0}{\strut 2017} \colorbox{red!3}{\strut Jefferson} \colorbox{red!3}{\strut Parish} \colorbox{red!0}{\strut ,} \colorbox{red!0}{\strut Louisiana} \colorbox{red!2}{\strut Sales} \colorbox{red!3}{\strut Tax} \colorbox{red!0}{\strut Louisiana} \colorbox{red!0}{\strut Income} \colorbox{red!3}{\strut Tax} \colorbox{red!0}{\strut .} \colorbox{red!0}{\strut Louisiana} \colorbox{red!2}{\strut Sales} \colorbox{red!3}{\strut Tax} \colorbox{red!0}{\strut .} \colorbox{red!0}{\strut Louisiana} \colorbox{red!0}{\strut Property} \colorbox{red!3}{\strut Tax} \colorbox{red!0}{\strut .} \colorbox{red!0}{\strut Louisiana} \colorbox{red!0}{\strut Corporate} \colorbox{red!0}{\strut Tax2017} \colorbox{red!3}{\strut Jefferson} \colorbox{red!3}{\strut Parish} \colorbox{red!0}{\strut ,} \colorbox{red!0}{\strut Louisiana} \colorbox{red!2}{\strut Sales} \colorbox{red!0}{\strut TaxLocal} \colorbox{red!2}{\strut Sales} \colorbox{red!3}{\strut Tax} \colorbox{red!0}{\strut -} \colorbox{red!3}{\strut Jefferson} \colorbox{red!0}{\strut Parish9.75} \colorbox{red!0}{\strut .} \colorbox{red!0}{\strut 2017} \colorbox{red!3}{\strut Jefferson} \colorbox{red!3}{\strut Parish} \colorbox{red!2}{\strut sales} \colorbox{red!0}{\strut taxExact} \colorbox{red!3}{\strut tax} \colorbox{red!0}{\strut amount} \colorbox{red!0}{\strut may} \colorbox{red!0}{\strut vary} \colorbox{red!0}{\strut for} \colorbox{red!0}{\strut different} \colorbox{red!0}{\strut itemsTax} \colorbox{red!0}{\strut Jurisdiction} \colorbox{red!2}{\strut Sales} \colorbox{red!0}{\strut TaxLouisiana} \colorbox{red!0}{\strut State} \colorbox{red!2}{\strut Sales} \colorbox{red!3}{\strut Tax} \colorbox{red!0}{\strut 5.00} \colorbox{red!0}{\strut .} \colorbox{red!0}{\strut County} \colorbox{red!2}{\strut Sales} \colorbox{red!3}{\strut Tax} \colorbox{red!0}{\strut 4.75} \colorbox{red!0}{\strut .} \colorbox{red!0}{\strut City} \colorbox{red!2}{\strut Sales} \colorbox{red!3}{\strut Tax} \colorbox{red!0}{\strut NASpecial} \colorbox{red!2}{\strut Sales} \colorbox{red!3}{\strut Tax} \colorbox{red!0}{\strut NACombined} \colorbox{red!2}{\strut Sales} \colorbox{red!3}{\strut Tax} \colorbox{red!0}{\strut 9.75} \colorbox{red!0}{\strut .} \colorbox{red!0}{\strut .} \colorbox{red!0}{\strut Is} \colorbox{red!0}{\strut this} \colorbox{red!0}{\strut data} \colorbox{red!0}{\strut incorrect} \colorbox{red!0}{\strut ?} \colorbox{red!0}{\strut .} \colorbox{red!0}{\strut Download} \colorbox{red!0}{\strut all} \colorbox{red!0}{\strut Louisiana} \colorbox{red!2}{\strut sales} \colorbox{red!3}{\strut tax} \colorbox{red!1}{\strut rates} \colorbox{red!0}{\strut by} \colorbox{red!0}{\strut zip} \colorbox{red!0}{\strut codeThe} \colorbox{red!3}{\strut Jefferson} \colorbox{red!3}{\strut Parish} \colorbox{red!0}{\strut ,} \colorbox{red!0}{\strut Louisiana} \colorbox{red!2}{\strut sales} \colorbox{red!3}{\strut tax} \colorbox{red!0}{\strut is} \colorbox{red!0}{\strut 9.75} \colorbox{red!0}{\strut .} \colorbox{red!0}{\strut ,} \colorbox{red!0}{\strut consisting} \colorbox{red!0}{\strut of} \colorbox{red!0}{\strut 5.00} \colorbox{red!0}{\strut .} \colorbox{red!0}{\strut Louisiana} \colorbox{red!0}{\strut state} \colorbox{red!2}{\strut sales} \colorbox{red!3}{\strut tax} \colorbox{red!0}{\strut and} \colorbox{red!0}{\strut 4.75} \colorbox{red!0}{\strut .} \colorbox{red!3}{\strut Jefferson} \colorbox{red!3}{\strut Parish} \colorbox{red!0}{\strut local} \colorbox{red!2}{\strut sales} \colorbox{red!0}{\strut taxes.The} \colorbox{red!0}{\strut local} \colorbox{red!2}{\strut sales} \colorbox{red!3}{\strut tax} \colorbox{red!0}{\strut consists} \colorbox{red!0}{\strut of} \colorbox{red!0}{\strut a} \colorbox{red!0}{\strut 4.75} \colorbox{red!0}{\strut .} \colorbox{red!0}{\strut county} \colorbox{red!2}{\strut sales} \colorbox{red!0}{\strut tax.The} \colorbox{red!3}{\strut Jefferson} \colorbox{red!3}{\strut Parish} \colorbox{red!2}{\strut Sales} \colorbox{red!3}{\strut Tax} \colorbox{red!0}{\strut is} \colorbox{red!0}{\strut collected} \colorbox{red!0}{\strut by} \colorbox{red!0}{\strut the} \colorbox{red!0}{\strut merchant} \colorbox{red!0}{\strut on} \colorbox{red!0}{\strut all} \colorbox{red!0}{\strut qualifying} \colorbox{red!2}{\strut sales} \colorbox{red!0}{\strut made} \colorbox{red!0}{\strut within} \colorbox{red!3}{\strut Jefferson} \colorbox{red!0}{\strut ParishGroceries} \colorbox{red!0}{\strut are} \colorbox{red!0}{\strut exempt} \colorbox{red!0}{\strut from} \colorbox{red!0}{\strut the} \colorbox{red!3}{\strut Jefferson} \colorbox{red!3}{\strut Parish} \colorbox{red!0}{\strut and} \colorbox{red!0}{\strut Louisiana} \colorbox{red!0}{\strut state} \colorbox{red!2}{\strut sales} \colorbox{red!0}{\strut taxesJefferson} \colorbox{red!3}{\strut Parish} \colorbox{red!0}{\strut collects} \colorbox{red!0}{\strut a} \colorbox{red!0}{\strut 4.75} \colorbox{red!0}{\strut .} \colorbox{red!0}{\strut local} \colorbox{red!2}{\strut sales} \colorbox{red!3}{\strut tax} \colorbox{red!0}{\strut ,} \colorbox{red!0}{\strut the} \colorbox{red!0}{\strut maximum} \colorbox{red!0}{\strut local} \colorbox{red!2}{\strut sales} \colorbox{red!3}{\strut tax} \colorbox{red!0}{\strut allowed} \colorbox{red!0}{\strut under} \colorbox{red!0}{\strut Louisiana} \colorbox{red!0}{\strut lawJefferson} \colorbox{red!3}{\strut Parish} \colorbox{red!0}{\strut has} \colorbox{red!0}{\strut a} \colorbox{red!0}{\strut lower} \colorbox{red!2}{\strut sales} \colorbox{red!3}{\strut tax} \colorbox{red!0}{\strut than} \colorbox{red!0}{\strut 59.6} \colorbox{red!0}{\strut .} \colorbox{red!0}{\strut of} \colorbox{red!0}{\strut Louisiana} \colorbox{red!0}{\strut s} \colorbox{red!0}{\strut other} \colorbox{red!0}{\strut cities} \colorbox{red!0}{\strut and} \colorbox{red!0}{\strut countiesJefferson} \colorbox{red!3}{\strut Parish} \colorbox{red!0}{\strut Louisiana} \colorbox{red!2}{\strut Sales} \colorbox{red!3}{\strut Tax} \colorbox{red!0}{\strut ExemptionsIn} \colorbox{red!0}{\strut most} \colorbox{red!0}{\strut states} \colorbox{red!0}{\strut ,} \colorbox{red!0}{\strut essential} \colorbox{red!0}{\strut purchases} \colorbox{red!0}{\strut like} \colorbox{red!0}{\strut medicine} \colorbox{red!0}{\strut and} \colorbox{red!0}{\strut groceries} \colorbox{red!0}{\strut are} \colorbox{red!0}{\strut exempted} \colorbox{red!0}{\strut from} \colorbox{red!0}{\strut the} \colorbox{red!2}{\strut sales} \colorbox{red!3}{\strut tax} \colorbox{red!0}{\strut or} \colorbox{red!0}{\strut eligible} \colorbox{red!0}{\strut for} \colorbox{red!0}{\strut a} \colorbox{red!0}{\strut lower} \colorbox{red!2}{\strut sales} \colorbox{red!3}{\strut tax} \colorbox{red!1}{\strut rate} \colorbox{red!0}{\strut .} \colorbox{red!3}{\strut Jefferson} \colorbox{red!3}{\strut Parish} \colorbox{red!0}{\strut does} \colorbox{red!0}{\strut nt} \colorbox{red!0}{\strut collect} \colorbox{red!2}{\strut sales} \colorbox{red!3}{\strut tax} \colorbox{red!0}{\strut on} \colorbox{red!0}{\strut purchases} \colorbox{red!0}{\strut of} \colorbox{red!0}{\strut most} \colorbox{red!0}{\strut groceries} \colorbox{red!0}{\strut .} \colorbox{red!0}{\strut Certain} \colorbox{red!0}{\strut purchases} \colorbox{red!0}{\strut ,} \colorbox{red!0}{\strut including} \colorbox{red!0}{\strut alcohol} \colorbox{red!0}{\strut ,} \colorbox{red!0}{\strut cigarettes} \colorbox{red!0}{\strut ,} \colorbox{red!0}{\strut and} \colorbox{red!0}{\strut gasoline} \colorbox{red!0}{\strut ,} \colorbox{red!0}{\strut may} \colorbox{red!0}{\strut be} \colorbox{red!0}{\strut subject} \colorbox{red!0}{\strut to} \colorbox{red!0}{\strut additional} \colorbox{red!0}{\strut Louisiana} \colorbox{red!0}{\strut state} \colorbox{red!0}{\strut excise} \colorbox{red!3}{\strut taxes} \colorbox{red!0}{\strut in} \colorbox{red!0}{\strut addition} \colorbox{red!0}{\strut to} \colorbox{red!0}{\strut the} \colorbox{red!2}{\strut sales} \colorbox{red!0}{\strut tax.Note} \colorbox{red!0}{\strut that} \colorbox{red!0}{\strut in} \colorbox{red!0}{\strut some} \colorbox{red!0}{\strut areas} \colorbox{red!0}{\strut ,} \colorbox{red!0}{\strut items} \colorbox{red!0}{\strut like} \colorbox{red!0}{\strut alcohol} \colorbox{red!0}{\strut and} \colorbox{red!0}{\strut prepared} \colorbox{red!0}{\strut food} \colorbox{red!0}{\strut .} \colorbox{red!0}{\strut including} \colorbox{red!0}{\strut restaurant} \colorbox{red!0}{\strut meals} \colorbox{red!0}{\strut and} \colorbox{red!0}{\strut some} \colorbox{red!0}{\strut premade} \colorbox{red!0}{\strut supermarket} \colorbox{red!0}{\strut items} \colorbox{red!0}{\strut .} \colorbox{red!0}{\strut are} \colorbox{red!0}{\strut charged} \colorbox{red!0}{\strut at} \colorbox{red!0}{\strut a} \colorbox{red!0}{\strut higher} \colorbox{red!2}{\strut sales} \colorbox{red!3}{\strut tax} \colorbox{red!1}{\strut rate} \colorbox{red!0}{\strut than} \colorbox{red!0}{\strut general} \colorbox{red!0}{\strut purchases} \colorbox{red!0}{\strut .} \colorbox{red!0}{\strut Louisiana} \colorbox{red!0}{\strut s} \colorbox{red!2}{\strut sales} \colorbox{red!3}{\strut tax} \colorbox{red!1}{\strut rates} \colorbox{red!0}{\strut for} \colorbox{red!0}{\strut commonly} \colorbox{red!0}{\strut exempted} \colorbox{red!0}{\strut categories} \colorbox{red!0}{\strut are} \colorbox{red!0}{\strut listed} \colorbox{red!0}{\strut below} \colorbox{red!0}{\strut .} \colorbox{red!0}{\strut Some} 
}}}
\end{CJK*}

\begin{CJK*}{UTF8}{gbsn}
{\setlength{\fboxsep}{0pt}\colorbox{white!0}{\parbox{0.9\textwidth}{
\colorbox{red!5}{\strut Louisiana} \colorbox{red!4}{\strut Sales} \colorbox{red!5}{\strut Tax} \colorbox{red!2}{\strut Holidays} \colorbox{red!0}{\strut in} \colorbox{red!0}{\strut 2013} \colorbox{red!5}{\strut Louisiana} \colorbox{red!5}{\strut Taxes} \colorbox{red!0}{\strut .} \colorbox{red!0}{\strut Income} \colorbox{red!5}{\strut Tax} \colorbox{red!0}{\strut .} \colorbox{red!4}{\strut Sales} \colorbox{red!5}{\strut Tax} \colorbox{red!0}{\strut .} \colorbox{red!0}{\strut Property} \colorbox{red!5}{\strut Tax} \colorbox{red!0}{\strut .} \colorbox{red!0}{\strut Corporate} \colorbox{red!5}{\strut Tax} \colorbox{red!0}{\strut .} \colorbox{red!0}{\strut Excise} \colorbox{red!0}{\strut TaxesLouisiana} \colorbox{red!4}{\strut Sales} \colorbox{red!5}{\strut Tax} \colorbox{red!2}{\strut Holidays} \colorbox{red!0}{\strut in} \colorbox{red!0}{\strut 2013A} \colorbox{red!4}{\strut sales} \colorbox{red!5}{\strut tax} \colorbox{red!2}{\strut holiday} \colorbox{red!0}{\strut is} \colorbox{red!0}{\strut a} \colorbox{red!0}{\strut special} \colorbox{red!1}{\strut time} \colorbox{red!0}{\strut period} \colorbox{red!0}{\strut in} \colorbox{red!0}{\strut which} \colorbox{red!0}{\strut you} \colorbox{red!0}{\strut are} \colorbox{red!0}{\strut allowed} \colorbox{red!0}{\strut to} \colorbox{red!0}{\strut purchase} \colorbox{red!0}{\strut certain} \colorbox{red!0}{\strut items} \colorbox{red!0}{\strut without} \colorbox{red!0}{\strut having} \colorbox{red!0}{\strut to} \colorbox{red!1}{\strut pay} \colorbox{red!0}{\strut the} \colorbox{red!5}{\strut Louisiana} \colorbox{red!4}{\strut sales} \colorbox{red!5}{\strut tax} \colorbox{red!0}{\strut .} \colorbox{red!0}{\strut The} \colorbox{red!5}{\strut Louisiana} \colorbox{red!4}{\strut sales} \colorbox{red!5}{\strut tax} \colorbox{red!0}{\strut is} \colorbox{red!0}{\strut 4} \colorbox{red!0}{\strut .} \colorbox{red!0}{\strut ,} \colorbox{red!0}{\strut so} \colorbox{red!0}{\strut taking} \colorbox{red!0}{\strut advantage} \colorbox{red!0}{\strut of} \colorbox{red!0}{\strut a} \colorbox{red!5}{\strut Louisiana} \colorbox{red!4}{\strut sales} \colorbox{red!5}{\strut tax} \colorbox{red!2}{\strut holiday} \colorbox{red!0}{\strut to} \colorbox{red!0}{\strut buy} \colorbox{red!0}{\strut .} \colorbox{red!0}{\strut 500.00} \colorbox{red!0}{\strut worth} \colorbox{red!0}{\strut of} \colorbox{red!0}{\strut goods} \colorbox{red!0}{\strut would} \colorbox{red!0}{\strut save} \colorbox{red!0}{\strut you} \colorbox{red!0}{\strut a} \colorbox{red!0}{\strut total} \colorbox{red!0}{\strut of} \colorbox{red!0}{\strut .} \colorbox{red!0}{\strut 20.00.Louisiana} \colorbox{red!0}{\strut has} \colorbox{red!0}{\strut five} \colorbox{red!4}{\strut sales} \colorbox{red!5}{\strut tax} \colorbox{red!2}{\strut holidays} \colorbox{red!0}{\strut throughout} \colorbox{red!0}{\strut the} \colorbox{red!0}{\strut year} \colorbox{red!0}{\strut on} \colorbox{red!0}{\strut a} \colorbox{red!0}{\strut variety} \colorbox{red!0}{\strut of} \colorbox{red!0}{\strut goods} \colorbox{red!0}{\strut .} \colorbox{red!0}{\strut The} \colorbox{red!4}{\strut sales} \colorbox{red!5}{\strut tax} \colorbox{red!2}{\strut holiday} \colorbox{red!0}{\strut calendar} \colorbox{red!0}{\strut below} \colorbox{red!0}{\strut lists} \colorbox{red!0}{\strut all} \colorbox{red!0}{\strut of} \colorbox{red!0}{\strut the} \colorbox{red!0}{\strut major} \colorbox{red!5}{\strut Louisiana} \colorbox{red!4}{\strut sales} \colorbox{red!5}{\strut tax} \colorbox{red!2}{\strut holidays} \colorbox{red!0}{\strut ,} \colorbox{red!0}{\strut the} \colorbox{red!0}{\strut item} \colorbox{red!0}{\strut the} \colorbox{red!2}{\strut holiday} \colorbox{red!0}{\strut applies} \colorbox{red!0}{\strut to} \colorbox{red!0}{\strut ,} \colorbox{red!0}{\strut and} \colorbox{red!0}{\strut the} \colorbox{red!0}{\strut total} \colorbox{red!0}{\strut purchase} \colorbox{red!0}{\strut amount} \colorbox{red!0}{\strut for} \colorbox{red!0}{\strut which} \colorbox{red!0}{\strut the} \colorbox{red!2}{\strut holiday} \colorbox{red!0}{\strut can} \colorbox{red!0}{\strut be} \colorbox{red!0}{\strut used} \colorbox{red!0}{\strut .} \colorbox{red!0}{\strut per} \colorbox{red!0}{\strut person} \colorbox{red!0}{\strut .} \colorbox{red!0}{\strut .Sale} \colorbox{red!0}{\strut Dates} \colorbox{red!2}{\strut Sale} \colorbox{red!0}{\strut Item} \colorbox{red!2}{\strut Sale} \colorbox{red!0}{\strut Maximum} \colorbox{red!0}{\strut Cost} \colorbox{red!2}{\strut Sale} \colorbox{red!0}{\strut Start} \colorbox{red!0}{\strut YearSeptember} \colorbox{red!0}{\strut 6th} \colorbox{red!0}{\strut -} \colorbox{red!0}{\strut September} \colorbox{red!0}{\strut 8th} \colorbox{red!0}{\strut Ammunition} \colorbox{red!0}{\strut NO} \colorbox{red!0}{\strut LIMIT} \colorbox{red!0}{\strut 2009} \colorbox{red!0}{\strut .} \colorbox{red!0}{\strut last} \colorbox{red!0}{\strut 9} \colorbox{red!0}{\strut years} \colorbox{red!0}{\strut .} \colorbox{red!0}{\strut September} \colorbox{red!0}{\strut 6th} \colorbox{red!0}{\strut -} \colorbox{red!0}{\strut September} \colorbox{red!0}{\strut 8th} \colorbox{red!0}{\strut Firearms} \colorbox{red!0}{\strut NO} \colorbox{red!0}{\strut LIMIT} \colorbox{red!0}{\strut 2009} \colorbox{red!0}{\strut .} \colorbox{red!0}{\strut last} \colorbox{red!0}{\strut 9} \colorbox{red!0}{\strut years} \colorbox{red!0}{\strut .} \colorbox{red!0}{\strut September} \colorbox{red!0}{\strut 6th} \colorbox{red!0}{\strut -} \colorbox{red!0}{\strut September} \colorbox{red!0}{\strut 8th} \colorbox{red!0}{\strut Hunting} \colorbox{red!0}{\strut Supplies} \colorbox{red!0}{\strut NO} \colorbox{red!0}{\strut LIMIT} \colorbox{red!0}{\strut 2009} \colorbox{red!0}{\strut .} \colorbox{red!0}{\strut last} \colorbox{red!0}{\strut 9} \colorbox{red!0}{\strut years} \colorbox{red!0}{\strut .} \colorbox{red!0}{\strut May} \colorbox{red!0}{\strut 25th} \colorbox{red!0}{\strut -} \colorbox{red!0}{\strut May} \colorbox{red!0}{\strut 26th} \colorbox{red!0}{\strut Hurricane} \colorbox{red!0}{\strut Preparedness} \colorbox{red!0}{\strut Items} \colorbox{red!0}{\strut .} \colorbox{red!0}{\strut 1,500.00} \colorbox{red!0}{\strut 2008} \colorbox{red!0}{\strut .} \colorbox{red!0}{\strut last} \colorbox{red!0}{\strut 10} \colorbox{red!0}{\strut years} \colorbox{red!0}{\strut .} \colorbox{red!0}{\strut August} \colorbox{red!0}{\strut 2nd} \colorbox{red!0}{\strut -} \colorbox{red!0}{\strut August} \colorbox{red!0}{\strut 3rd} \colorbox{red!0}{\strut TPP} \colorbox{red!0}{\strut .} \colorbox{red!0}{\strut 2,500.00} \colorbox{red!0}{\strut 2007} \colorbox{red!0}{\strut .} \colorbox{red!0}{\strut last} \colorbox{red!0}{\strut 11} \colorbox{red!0}{\strut years} \colorbox{red!0}{\strut .} \colorbox{red!0}{\strut Why} \colorbox{red!0}{\strut do} \colorbox{red!0}{\strut states} \colorbox{red!0}{\strut have} \colorbox{red!4}{\strut sales} \colorbox{red!5}{\strut tax} \colorbox{red!2}{\strut holidays} \colorbox{red!0}{\strut ?} \colorbox{red!0}{\strut Over} \colorbox{red!0}{\strut a} \colorbox{red!0}{\strut dozen} \colorbox{red!0}{\strut states} \colorbox{red!0}{\strut have} \colorbox{red!0}{\strut various} \colorbox{red!0}{\strut types} \colorbox{red!0}{\strut of} \colorbox{red!4}{\strut sales} \colorbox{red!5}{\strut tax} \colorbox{red!2}{\strut holidays} \colorbox{red!0}{\strut throughout} \colorbox{red!0}{\strut the} \colorbox{red!0}{\strut year} \colorbox{red!0}{\strut .} \colorbox{red!0}{\strut Most} \colorbox{red!0}{\strut of} \colorbox{red!0}{\strut the} \colorbox{red!1}{\strut time} \colorbox{red!0}{\strut ,} \colorbox{red!0}{\strut these} \colorbox{red!2}{\strut holidays} \colorbox{red!0}{\strut are} \colorbox{red!0}{\strut special} \colorbox{red!0}{\strut promotions} \colorbox{red!0}{\strut designed} \colorbox{red!0}{\strut to} \colorbox{red!0}{\strut promote} \colorbox{red!0}{\strut desirable} \colorbox{red!0}{\strut purchases} \colorbox{red!0}{\strut of} \colorbox{red!0}{\strut items} \colorbox{red!0}{\strut such} \colorbox{red!0}{\strut as} \colorbox{red!0}{\strut energy-star} \colorbox{red!0}{\strut rated} \colorbox{red!0}{\strut products} \colorbox{red!0}{\strut ,} \colorbox{red!0}{\strut emergency} \colorbox{red!0}{\strut preparedness} \colorbox{red!0}{\strut supplies} \colorbox{red!0}{\strut ,} \colorbox{red!0}{\strut etc} \colorbox{red!0}{\strut .} \colorbox{red!0}{\strut Many} \colorbox{red!0}{\strut states} \colorbox{red!0}{\strut also} \colorbox{red!0}{\strut hold} \colorbox{red!4}{\strut sales} \colorbox{red!5}{\strut tax} \colorbox{red!2}{\strut holidays} \colorbox{red!0}{\strut to} \colorbox{red!0}{\strut correspond} \colorbox{red!0}{\strut with} \colorbox{red!0}{\strut the} \colorbox{red!0}{\strut back-to-school} \colorbox{red!0}{\strut shopping} \colorbox{red!0}{\strut season} \colorbox{red!0}{\strut for} \colorbox{red!0}{\strut items} \colorbox{red!0}{\strut like} \colorbox{red!0}{\strut books} \colorbox{red!0}{\strut ,} \colorbox{red!0}{\strut clothing} \colorbox{red!0}{\strut ,} \colorbox{red!0}{\strut and} \colorbox{red!0}{\strut school} \colorbox{red!0}{\strut supplies.In} \colorbox{red!0}{\strut some} \colorbox{red!0}{\strut cases} \colorbox{red!0}{\strut ,} 
}}}
\end{CJK*}
